# Supplementary material for: Generalisation of automatic tumour segmentation in histopathological whole-slide images across multiple cancer types
Source: arXiv:2510.11182 source file (2025-10-13)
Supplement: Supplementary file 1 [file appendix.pdf]

## **Supplementary appendix**

## Contents

|          |                                                                                |           |
|----------|--------------------------------------------------------------------------------|-----------|
| <b>1</b> | <b>Results from pre-planned analyses</b>                                       | <b>1</b>  |
| 1.1      | Primary model performance in Aperio AT2 (study protocol section 3.1 and 3.2.1) | 1         |
| 1.2      | Primary model performance in NanoZoomer XR (study protocol section 3.2.2)      | 3         |
| 1.3      | Cancer type-specialised models performance (study protocol section 3.2.3)      | 5         |
| 1.3.1    | Colorectal carcinoma                                                           | 5         |
| 1.3.2    | Endometrial carcinoma                                                          | 7         |
| 1.3.3    | Lung carcinoma                                                                 | 9         |
| 1.3.4    | Prostate carcinoma                                                             | 11        |
| 1.4      | Primary model replication performance (study protocol section 3.2.4)           | 13        |
| 1.4.1    | Replication 1                                                                  | 13        |
| 1.4.2    | Replication 2                                                                  | 15        |
| <b>2</b> | <b>Results from exploratory analyses</b>                                       | <b>17</b> |
| 2.1      | Association analyses in primary model                                          | 17        |
| 2.2      | Per-scan comparison                                                            | 25        |
| 2.3      | Region areas                                                                   | 26        |
| 2.4      | Intra- and inter-observer variability                                          | 29        |
| 2.5      | Performance evaluation in five different scanners                              | 30        |
| 2.6      | Comparison with MedSAM                                                         | 32        |
| <b>3</b> | <b>Segmentation network optimisation</b>                                       | <b>34</b> |
| <b>4</b> | <b>TCGA cohorts</b>                                                            | <b>35</b> |
| 4.1      | Included scans                                                                 | 35        |
| 4.2      | Baseline characteristics                                                       | 37        |
| <b>5</b> | <b>Protocol amendment</b>                                                      | <b>39</b> |
| 5.1      | Protocol section 1.1.4 DEn1 — Endometrial carcinoma                            | 39        |
| 5.2      | Protocol section 1.2.8 VUr1 — Urothelial carcinoma                             | 39        |
| 5.3      | Protocol Table 5 and protocol Fig. 18                                          | 39        |
| 5.4      | Protocol Figs. 27, 28, 29, 30                                                  | 40        |
| <b>6</b> | <b>Study protocol</b>                                                          | <b>46</b> |

## List of Figures

|     |                                                                        |    |
|-----|------------------------------------------------------------------------|----|
| S1  | Primary model performance on Aperio AT2 scans . . . . .                | 2  |
| S2  | Primary model performance on NanoZoomer XR scans . . . . .             | 4  |
| S3  | Colorectal model performance on Aperio AT2 scans . . . . .             | 6  |
| S4  | Endometrial model performance on Aperio AT2 scans . . . . .            | 8  |
| S5  | Lung model performance on Aperio AT2 scans . . . . .                   | 10 |
| S6  | Prostate model performance on Aperio AT2 scans . . . . .               | 12 |
| S7  | First primary model replica performance on Aperio AT2 scans . . . . .  | 14 |
| S8  | Second primary model replica performance on Aperio AT2 scans . . . . . | 16 |
| S9  | Associations VCo1 . . . . .                                            | 17 |
| S10 | Associations VEn1 . . . . .                                            | 18 |
| S11 | Associations VEn2 . . . . .                                            | 19 |
| S12 | Associations VLu1 . . . . .                                            | 20 |
| S13 | Associations VPr1 . . . . .                                            | 21 |
| S14 | Associations VBr1 . . . . .                                            | 22 |
| S15 | Associations VBr2 . . . . .                                            | 23 |
| S16 | Associations VUr1 . . . . .                                            | 24 |
| S17 | Per scan comparison . . . . .                                          | 25 |
| S18 | Region areas . . . . .                                                 | 27 |
| S19 | Intra- and inter-observer variability in VBr2 . . . . .                | 29 |
| S20 | Original vs restained mean difference . . . . .                        | 30 |
| S21 | Scanner vs scanner mean difference . . . . .                           | 31 |
| S22 | MedSAM performance in validation datasets . . . . .                    | 33 |
| S23 | Segmentation network optimisation loss curve . . . . .                 | 34 |
| S24 | Acquisition overview LUAD . . . . .                                    | 35 |
| S25 | Acquisition overview LUSC . . . . .                                    | 35 |
| S26 | Acquisition overview PRAD . . . . .                                    | 36 |
| S27 | Acquisition overview BLCA . . . . .                                    | 36 |
| S28 | Kaplan-Meier analysis in materials from TCGA lung carcinoma . . . . .  | 38 |
| S29 | Kaplan-Meier analysis in materials from lung carcinoma . . . . .       | 39 |
| S30 | Scan area Aperio AT2 . . . . .                                         | 41 |
| S31 | Scan area NanoZoomer XR . . . . .                                      | 42 |
| S32 | Scan content prevalence Aperio AT2 . . . . .                           | 43 |
| S33 | Scan content prevalence NanoZoomer XR . . . . .                        | 44 |

## List of Tables

|     |                                                                        |    |
|-----|------------------------------------------------------------------------|----|
| S1  | Primary model performance on Aperio AT2 scans . . . . .                | 1  |
| S2  | Primary model performance on NanoZoomer XR scans . . . . .             | 3  |
| S3  | Colorectal model performance on Aperio AT2 scans . . . . .             | 5  |
| S4  | Endometrial model performance on Aperio AT2 scans . . . . .            | 7  |
| S5  | Lung model performance on Aperio AT2 scans . . . . .                   | 9  |
| S6  | Prostate model performance on Aperio AT2 scans . . . . .               | 11 |
| S7  | First primary model replica performance on Aperio AT2 scans . . . . .  | 13 |
| S8  | Second primary model replica performance on Aperio AT2 scans . . . . . | 15 |
| S9  | Performance in true positive regions . . . . .                         | 26 |
| S10 | Subgroup analyses in bladder cohorts . . . . .                         | 28 |
| S11 | Intra- and inter-observer variability in VBr2 . . . . .                | 29 |
| S12 | Primary model performance on five different scanners . . . . .         | 30 |
| S13 | MedSAM performance in validation datasets . . . . .                    | 32 |
| S14 | Baseline characteristics in materials from TCGA . . . . .              | 37 |
| S15 | Baseline characteristics in materials from lung carcinoma . . . . .    | 40 |

# 1 Results from pre-planned analyses

## 1.1 Primary model performance in Aperio AT2 (study protocol section 3.1 and 3.2.1)

**Table S1: Primary model performance on Aperio AT2 scans**  
Data entries show mean value (95% CI)

| Cohort | Prevalence                | Bias                      |
|--------|---------------------------|---------------------------|
| VCo1   | 0.3410 (0.3315 – 0.3505)  | 0.3682 (0.3583 – 0.3781)  |
| VEn1   | 0.4924 (0.4363 – 0.5485)  | 0.4912 (0.4362 – 0.5462)  |
| VEn2   | 0.3970 (0.3611 – 0.4328)  | 0.4065 (0.3708 – 0.4422)  |
| VLu1   | 0.3380 (0.3208 – 0.3552)  | 0.3891 (0.3703 – 0.4079)  |
| VPr1   | 0.1777 (0.1671 – 0.1882)  | 0.1775 (0.1670 – 0.1881)  |
| VBr1   | 0.2278 (0.2089 – 0.2467)  | 0.2114 (0.1933 – 0.2295)  |
| VBr2   | 0.3081 (0.2808 – 0.3355)  | 0.2938 (0.2674 – 0.3201)  |
| VUr1   | 0.5304 (0.5004 – 0.5603)  | 0.2843 (0.2533 – 0.3154)  |
| Cohort | True positive rate        | False negative rate       |
| VCo1   | 0.8928 (0.8852 – 0.9004)  | 0.1072 (0.0996 – 0.1148)  |
| VEn1   | 0.9568 (0.9460 – 0.9677)  | 0.0432 (0.0323 – 0.0540)  |
| VEn2   | 0.9553 (0.9490 – 0.9616)  | 0.0447 (0.0384 – 0.0510)  |
| VLu1   | 0.9060 (0.8895 – 0.9224)  | 0.0940 (0.0776 – 0.1105)  |
| VPr1   | 0.8530 (0.8420 – 0.8640)  | 0.1470 (0.1360 – 0.1580)  |
| VBr1   | 0.8249 (0.8005 – 0.8494)  | 0.1751 (0.1506 – 0.1995)  |
| VBr2   | 0.8779 (0.8609 – 0.8950)  | 0.1221 (0.1050 – 0.1391)  |
| VUr1   | 0.4405 (0.4016 – 0.4794)  | 0.5595 (0.5206 – 0.5984)  |
| Cohort | True negative rate        | False positive rate       |
| VCo1   | 0.8935 (0.8883 – 0.8987)  | 0.1065 (0.1013 – 0.1117)  |
| VEn1   | 0.9187 (0.8887 – 0.9486)  | 0.0813 (0.0514 – 0.1113)  |
| VEn2   | 0.9286 (0.9099 – 0.9473)  | 0.0714 (0.0527 – 0.0901)  |
| VLu1   | 0.8760 (0.8660 – 0.8859)  | 0.1240 (0.1141 – 0.1340)  |
| VPr1   | 0.9722 (0.9693 – 0.9750)  | 0.0278 (0.0250 – 0.0307)  |
| VBr1   | 0.9741 (0.9689 – 0.9793)  | 0.0259 (0.0207 – 0.0311)  |
| VBr2   | 0.9610 (0.9531 – 0.9690)  | 0.0390 (0.0310 – 0.0469)  |
| VUr1   | 0.9443 (0.9340 – 0.9546)  | 0.0557 (0.0454 – 0.0660)  |
| Cohort | Positive predictive value | Negative predictive value |
| VCo1   | 0.8138 (0.8062 – 0.8213)  | 0.9380 (0.9336 – 0.9423)  |
| VEn1   | 0.9523 (0.9374 – 0.9672)  | 0.9132 (0.8783 – 0.9480)  |
| VEn2   | 0.9211 (0.9055 – 0.9366)  | 0.9504 (0.9367 – 0.9641)  |
| VLu1   | 0.7686 (0.7508 – 0.7864)  | 0.9640 (0.9597 – 0.9684)  |
| VPr1   | 0.8492 (0.8382 – 0.8601)  | 0.9721 (0.9691 – 0.9750)  |
| VBr1   | 0.8627 (0.8374 – 0.8880)  | 0.9523 (0.9442 – 0.9604)  |
| VBr2   | 0.9018 (0.8845 – 0.9191)  | 0.9324 (0.9192 – 0.9456)  |
| VUr1   | 0.6280 (0.5800 – 0.6759)  | 0.6139 (0.5860 – 0.6419)  |
| Cohort | Informedness              | Markedness                |
| VCo1   | 0.7863 (0.7780 – 0.7947)  | 0.7517 (0.7432 – 0.7603)  |
| VEn1   | 0.8755 (0.8441 – 0.9070)  | 0.8655 (0.8297 – 0.9013)  |
| VEn2   | 0.8839 (0.8653 – 0.9026)  | 0.8715 (0.8528 – 0.8902)  |
| VLu1   | 0.7819 (0.7653 – 0.7985)  | 0.7327 (0.7142 – 0.7511)  |
| VPr1   | 0.8252 (0.8144 – 0.8360)  | 0.8212 (0.8104 – 0.8320)  |
| VBr1   | 0.7990 (0.7745 – 0.8236)  | 0.8150 (0.7871 – 0.8429)  |
| VBr2   | 0.8390 (0.8214 – 0.8566)  | 0.8342 (0.8120 – 0.8564)  |
| VUr1   | 0.3848 (0.3508 – 0.4189)  | 0.2419 (0.1855 – 0.2983)  |
| Cohort | Matthews corr. coeff.     | Dice similarity coeff.    |
| VCo1   | 0.7683 (0.7605 – 0.7761)  | 0.8454 (0.8386 – 0.8523)  |
| VEn1   | 0.8686 (0.8349 – 0.9022)  | 0.9528 (0.9420 – 0.9636)  |
| VEn2   | 0.8753 (0.8576 – 0.8930)  | 0.9340 (0.9231 – 0.9449)  |
| VLu1   | 0.7551 (0.7387 – 0.7714)  | 0.8222 (0.8054 – 0.8391)  |
| VPr1   | 0.8203 (0.8103 – 0.8304)  | 0.8436 (0.8333 – 0.8538)  |
| VBr1   | 0.8021 (0.7782 – 0.8260)  | 0.8240 (0.7994 – 0.8486)  |
| VBr2   | 0.8351 (0.8176 – 0.8526)  | 0.8816 (0.8652 – 0.8980)  |
| VUr1   | 0.3691 (0.3369 – 0.4014)  | 0.4977 (0.4564 – 0.5390)  |

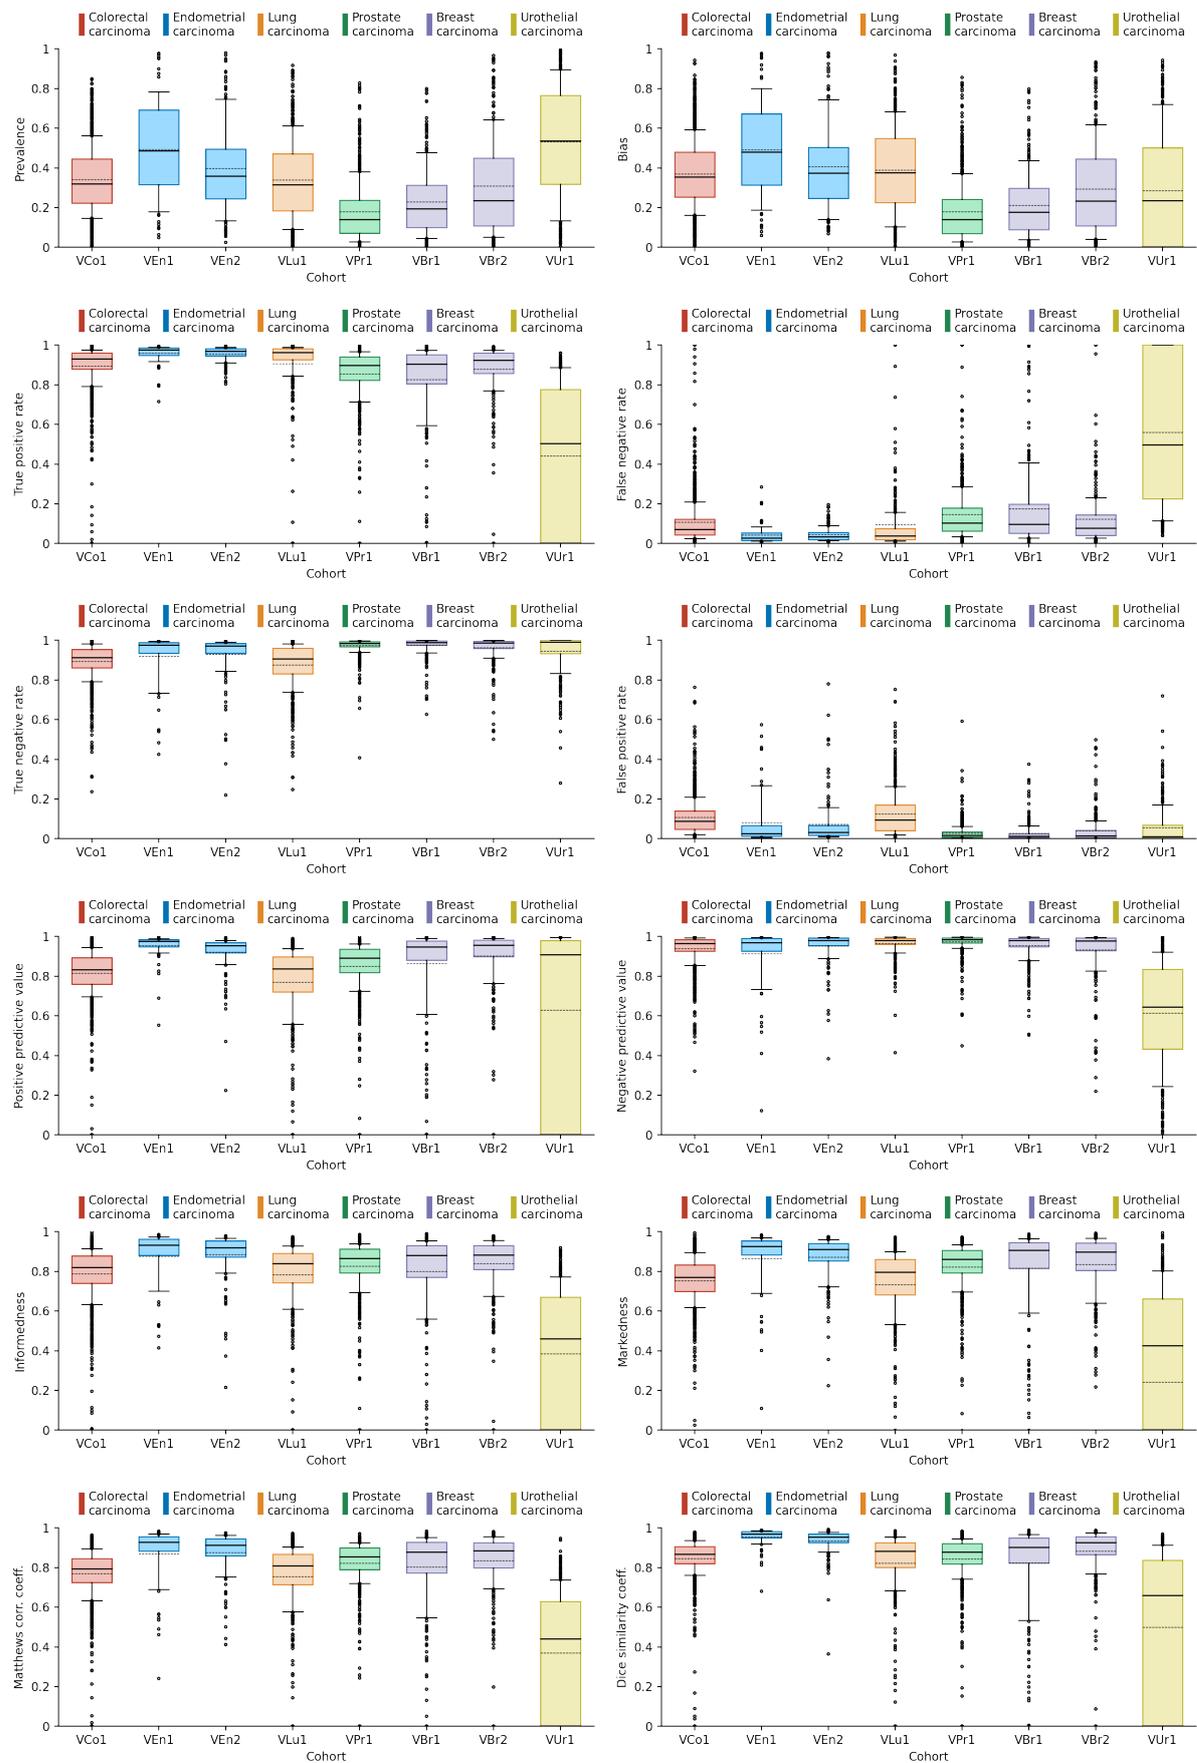

**Figure S1: Primary model performance on Aperio AT2 scans**

For each cohort, the plot displays the interquartile range (coloured box), mean value (perforated horizontal line), median value (solid horizontal line), the 10th and 90th percentile (whiskers), and outliers (black circles).

## 1.2 Primary model performance in NanoZoomer XR (study protocol section 3.2.2)

**Table S2: Primary model performance on NanoZoomer XR scans**  
Data entries show mean value (95% CI)

| Cohort | Prevalence                | Bias                      |
|--------|---------------------------|---------------------------|
| VCo1   | 0.3411 (0.3316 – 0.3505)  | 0.3695 (0.3596 – 0.3794)  |
| VEn1   | 0.4887 (0.4328 – 0.5447)  | 0.4924 (0.4367 – 0.5481)  |
| VEn2   | 0.3950 (0.3593 – 0.4307)  | 0.4044 (0.3691 – 0.4398)  |
| VLu1   | 0.3363 (0.3192 – 0.3534)  | 0.3841 (0.3655 – 0.4026)  |
| VPr1   | 0.1763 (0.1658 – 0.1868)  | 0.1791 (0.1686 – 0.1897)  |
| VBr1   | 0.2421 (0.2229 – 0.2614)  | 0.2232 (0.2043 – 0.2420)  |
| VBr2   | 0.3262 (0.2989 – 0.3534)  | 0.3126 (0.2862 – 0.3390)  |
| VUr1   | 0.5292 (0.4994 – 0.5590)  | 0.2423 (0.2134 – 0.2712)  |
| Cohort | True positive rate        | False negative rate       |
| VCo1   | 0.8894 (0.8815 – 0.8974)  | 0.1097 (0.1019 – 0.1175)  |
| VEn1   | 0.9625 (0.9534 – 0.9716)  | 0.0375 (0.0284 – 0.0466)  |
| VEn2   | 0.9555 (0.9491 – 0.9619)  | 0.0445 (0.0381 – 0.0509)  |
| VLu1   | 0.9016 (0.8854 – 0.9179)  | 0.0984 (0.0821 – 0.1146)  |
| VPr1   | 0.8568 (0.8454 – 0.8682)  | 0.1432 (0.1318 – 0.1546)  |
| VBr1   | 0.8117 (0.7849 – 0.8385)  | 0.1883 (0.1615 – 0.2151)  |
| VBr2   | 0.8696 (0.8497 – 0.8895)  | 0.1304 (0.1105 – 0.1503)  |
| VUr1   | 0.3806 (0.3433 – 0.4178)  | 0.6194 (0.5822 – 0.6567)  |
| Cohort | True negative rate        | False positive rate       |
| VCo1   | 0.8913 (0.8861 – 0.8965)  | 0.1087 (0.1035 – 0.1139)  |
| VEn1   | 0.9131 (0.8817 – 0.9445)  | 0.0869 (0.0555 – 0.1183)  |
| VEn2   | 0.9301 (0.9117 – 0.9484)  | 0.0699 (0.0516 – 0.0883)  |
| VLu1   | 0.8809 (0.8715 – 0.8903)  | 0.1191 (0.1097 – 0.1285)  |
| VPr1   | 0.9698 (0.9668 – 0.9728)  | 0.0302 (0.0272 – 0.0332)  |
| VBr1   | 0.9712 (0.9654 – 0.9770)  | 0.0288 (0.0230 – 0.0346)  |
| VBr2   | 0.9563 (0.9486 – 0.9640)  | 0.0437 (0.0360 – 0.0514)  |
| VUr1   | 0.9597 (0.9511 – 0.9683)  | 0.0403 (0.0317 – 0.0489)  |
| Cohort | Positive predictive value | Negative predictive value |
| VCo1   | 0.8101 (0.8025 – 0.8178)  | 0.9380 (0.9337 – 0.9423)  |
| VEn1   | 0.9484 (0.9329 – 0.9639)  | 0.9208 (0.8894 – 0.9523)  |
| VEn2   | 0.9183 (0.9015 – 0.9350)  | 0.9504 (0.9366 – 0.9641)  |
| VLu1   | 0.7716 (0.7541 – 0.7891)  | 0.9624 (0.9579 – 0.9668)  |
| VPr1   | 0.8369 (0.8252 – 0.8486)  | 0.9736 (0.9707 – 0.9764)  |
| VBr1   | 0.8474 (0.8191 – 0.8756)  | 0.9467 (0.9380 – 0.9554)  |
| VBr2   | 0.8885 (0.8682 – 0.9088)  | 0.9282 (0.9150 – 0.9414)  |
| VUr1   | 0.6099 (0.5606 – 0.6593)  | 0.5905 (0.5622 – 0.6188)  |
| Cohort | Informedness              | Markedness                |
| VCo1   | 0.7807 (0.7721 – 0.7893)  | 0.7481 (0.7395 – 0.7567)  |
| VEn1   | 0.8756 (0.8433 – 0.9079)  | 0.8692 (0.8361 – 0.9023)  |
| VEn2   | 0.8855 (0.8671 – 0.9039)  | 0.8686 (0.8491 – 0.8882)  |
| VLu1   | 0.7825 (0.7663 – 0.7987)  | 0.7340 (0.7159 – 0.7521)  |
| VPr1   | 0.8266 (0.8154 – 0.8378)  | 0.8105 (0.7989 – 0.8221)  |
| VBr1   | 0.7829 (0.7561 – 0.8097)  | 0.7941 (0.7625 – 0.8257)  |
| VBr2   | 0.8259 (0.8060 – 0.8457)  | 0.8167 (0.7924 – 0.8411)  |
| VUr1   | 0.3403 (0.3070 – 0.3735)  | 0.2004 (0.1433 – 0.2575)  |
| Cohort | Matthews corr. coeff.     | Dice similarity coeff.    |
| VCo1   | 0.7637 (0.7558 – 0.7715)  | 0.8417 (0.8346 – 0.8488)  |
| VEn1   | 0.8707 (0.8386 – 0.9028)  | 0.9535 (0.9430 – 0.9640)  |
| VEn2   | 0.8743 (0.8564 – 0.8922)  | 0.9320 (0.9203 – 0.9437)  |
| VLu1   | 0.7559 (0.7399 – 0.7719)  | 0.8216 (0.8050 – 0.8382)  |
| VPr1   | 0.8152 (0.8045 – 0.8259)  | 0.8382 (0.8272 – 0.8492)  |
| VBr1   | 0.7855 (0.7589 – 0.8121)  | 0.8101 (0.7828 – 0.8373)  |
| VBr2   | 0.8201 (0.8004 – 0.8398)  | 0.8700 (0.8507 – 0.8892)  |
| VUr1   | 0.3328 (0.3012 – 0.3644)  | 0.4453 (0.4048 – 0.4858)  |

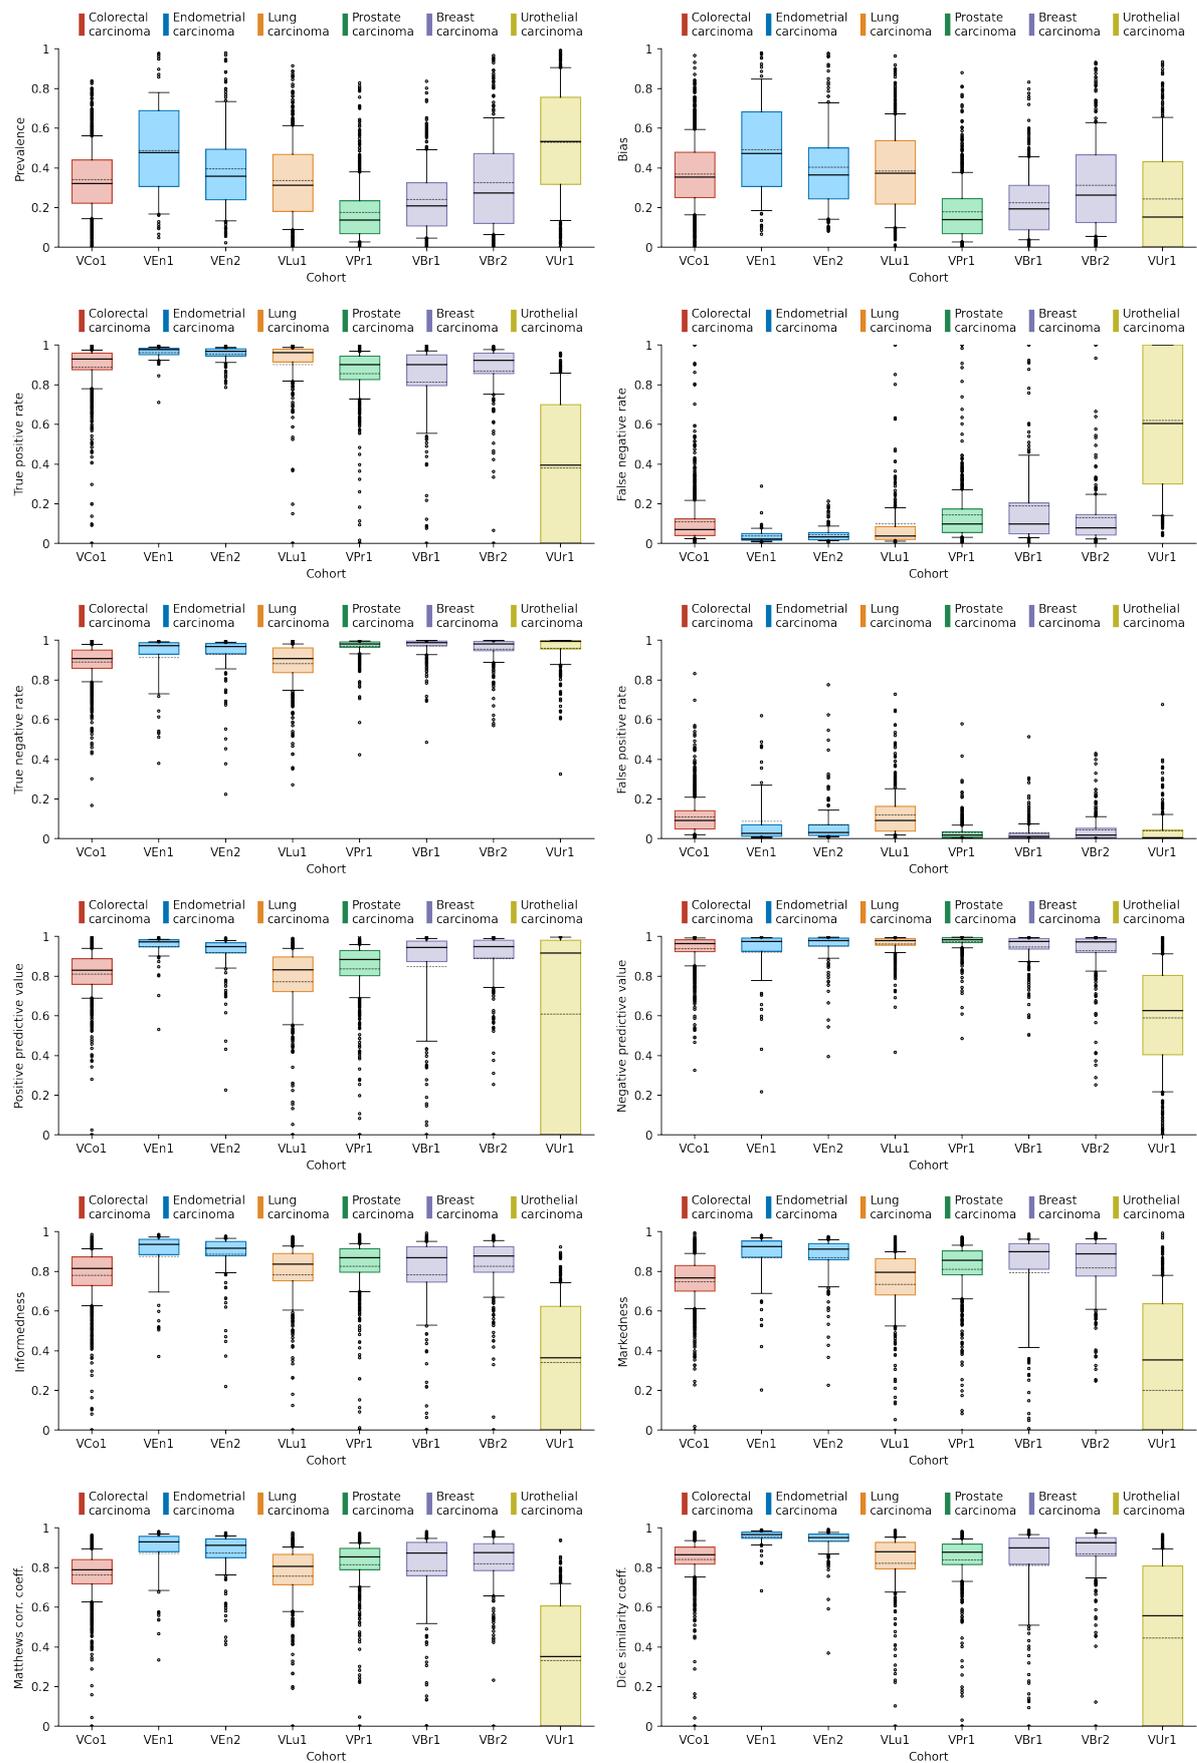

**Figure S2: Primary model performance on NanoZoomer XR scans**

For each cohort, the plot displays the interquartile range (coloured box), mean value (perforated horizontal line), median value (solid horizontal line), the 10th and 90th percentile (whiskers), and outliers (black circles).

### 1.3 Cancer type-specialised models performance (study protocol section 3.2.3)

#### 1.3.1 Colorectal carcinoma

**Table S3: Colorectal model performance on Aperio AT2 scans**  
Data entries show mean value (95% CI)

| Cohort | Prevalence                | Bias                        |
|--------|---------------------------|-----------------------------|
| VCo1   | 0.3410 (0.3315 – 0.3505)  | 0.3691 (0.3585 – 0.3796)    |
| VEn1   | 0.4924 (0.4363 – 0.5485)  | 0.4511 (0.3949 – 0.5073)    |
| VEn2   | 0.3970 (0.3611 – 0.4328)  | 0.4097 (0.3737 – 0.4457)    |
| VLu1   | 0.3380 (0.3208 – 0.3552)  | 0.3908 (0.3666 – 0.4149)    |
| VPr1   | 0.1777 (0.1671 – 0.1882)  | 0.5939 (0.5818 – 0.6060)    |
| VBr1   | 0.2278 (0.2089 – 0.2467)  | 0.1952 (0.1752 – 0.2151)    |
| VBr2   | 0.3081 (0.2808 – 0.3355)  | 0.2917 (0.2643 – 0.3191)    |
| VUr1   | 0.5304 (0.5004 – 0.5603)  | 0.0408 (0.0260 – 0.0557)    |
| Cohort | True positive rate        | False negative rate         |
| VCo1   | 0.8856 (0.8755 – 0.8958)  | 0.1144 (0.1042 – 0.1245)    |
| VEn1   | 0.8684 (0.8206 – 0.9162)  | 0.1316 (0.0838 – 0.1794)    |
| VEn2   | 0.8841 (0.8529 – 0.9153)  | 0.1159 (0.0847 – 0.1471)    |
| VLu1   | 0.7058 (0.6734 – 0.7381)  | 0.2942 (0.2619 – 0.3266)    |
| VPr1   | 0.9179 (0.9069 – 0.9290)  | 0.0821 (0.0710 – 0.0931)    |
| VBr1   | 0.6776 (0.6362 – 0.7191)  | 0.3224 (0.2809 – 0.3638)    |
| VBr2   | 0.7946 (0.7607 – 0.8285)  | 0.2054 (0.1715 – 0.2393)    |
| VUr1   | 0.0551 (0.0368 – 0.0735)  | 0.9449 (0.9265 – 0.9632)    |
| Cohort | True negative rate        | False positive rate         |
| VCo1   | 0.8932 (0.8876 – 0.8988)  | 0.1068 (0.1012 – 0.1124)    |
| VEn1   | 0.9135 (0.8817 – 0.9454)  | 0.0865 (0.0546 – 0.1183)    |
| VEn2   | 0.9070 (0.8897 – 0.9243)  | 0.0930 (0.0757 – 0.1103)    |
| VLu1   | 0.7958 (0.7781 – 0.8134)  | 0.2042 (0.1866 – 0.2219)    |
| VPr1   | 0.4906 (0.4759 – 0.5053)  | 0.5094 (0.4947 – 0.5241)    |
| VBr1   | 0.9595 (0.9518 – 0.9672)  | 0.0405 (0.0328 – 0.0482)    |
| VBr2   | 0.9312 (0.9189 – 0.9435)  | 0.0688 (0.0565 – 0.0811)    |
| VUr1   | 0.9929 (0.9874 – 0.9983)  | 0.0071 (0.0017 – 0.0126)    |
| Cohort | Positive predictive value | Negative predictive value   |
| VCo1   | 0.8095 (0.8005 – 0.8186)  | 0.9440 (0.9397 – 0.9482)    |
| VEn1   | 0.8940 (0.8482 – 0.9398)  | 0.8496 (0.8034 – 0.8957)    |
| VEn2   | 0.8239 (0.7862 – 0.8616)  | 0.9215 (0.9023 – 0.9407)    |
| VLu1   | 0.5768 (0.5491 – 0.6044)  | 0.9058 (0.8969 – 0.9147)    |
| VPr1   | 0.2881 (0.2712 – 0.3050)  | 0.9696 (0.9651 – 0.9741)    |
| VBr1   | 0.6811 (0.6393 – 0.7228)  | 0.9261 (0.9140 – 0.9382)    |
| VBr2   | 0.7703 (0.7364 – 0.8041)  | 0.9141 (0.8966 – 0.9316)    |
| VUr1   | 0.1184 (0.0843 – 0.1526)  | 0.4836 (0.4540 – 0.5132)    |
| Cohort | Informedness              | Markedness                  |
| VCo1   | 0.7788 (0.7688 – 0.7889)  | 0.7535 (0.7434 – 0.7636)    |
| VEn1   | 0.7819 (0.7296 – 0.8343)  | 0.7435 (0.6723 – 0.8147)    |
| VEn2   | 0.7911 (0.7590 – 0.8232)  | 0.7454 (0.7030 – 0.7878)    |
| VLu1   | 0.5015 (0.4751 – 0.5279)  | 0.4825 (0.4525 – 0.5126)    |
| VPr1   | 0.4086 (0.3929 – 0.4243)  | 0.2577 (0.2418 – 0.2736)    |
| VBr1   | 0.6371 (0.5967 – 0.6775)  | 0.6072 (0.5592 – 0.6551)    |
| VBr2   | 0.7258 (0.6931 – 0.7585)  | 0.6844 (0.6439 – 0.7249)    |
| VUr1   | 0.0480 (0.0318 – 0.0642)  | -0.3979 (-0.4420 – -0.3539) |
| Cohort | Matthews corr. coeff.     | Dice similarity coeff.      |
| VCo1   | 0.7659 (0.7566 – 0.7751)  | 0.8387 (0.8297 – 0.8477)    |
| VEn1   | 0.7672 (0.7147 – 0.8197)  | 0.8630 (0.8153 – 0.9107)    |
| VEn2   | 0.7674 (0.7335 – 0.8013)  | 0.8413 (0.8071 – 0.8755)    |
| VLu1   | 0.5010 (0.4760 – 0.5260)  | 0.6150 (0.5865 – 0.6435)    |
| VPr1   | 0.3094 (0.2944 – 0.3244)  | 0.3903 (0.3726 – 0.4080)    |
| VBr1   | 0.6292 (0.5896 – 0.6688)  | 0.6543 (0.6139 – 0.6948)    |
| VBr2   | 0.7092 (0.6770 – 0.7415)  | 0.7637 (0.7307 – 0.7967)    |
| VUr1   | 0.0452 (0.0306 – 0.0598)  | 0.0705 (0.0484 – 0.0927)    |

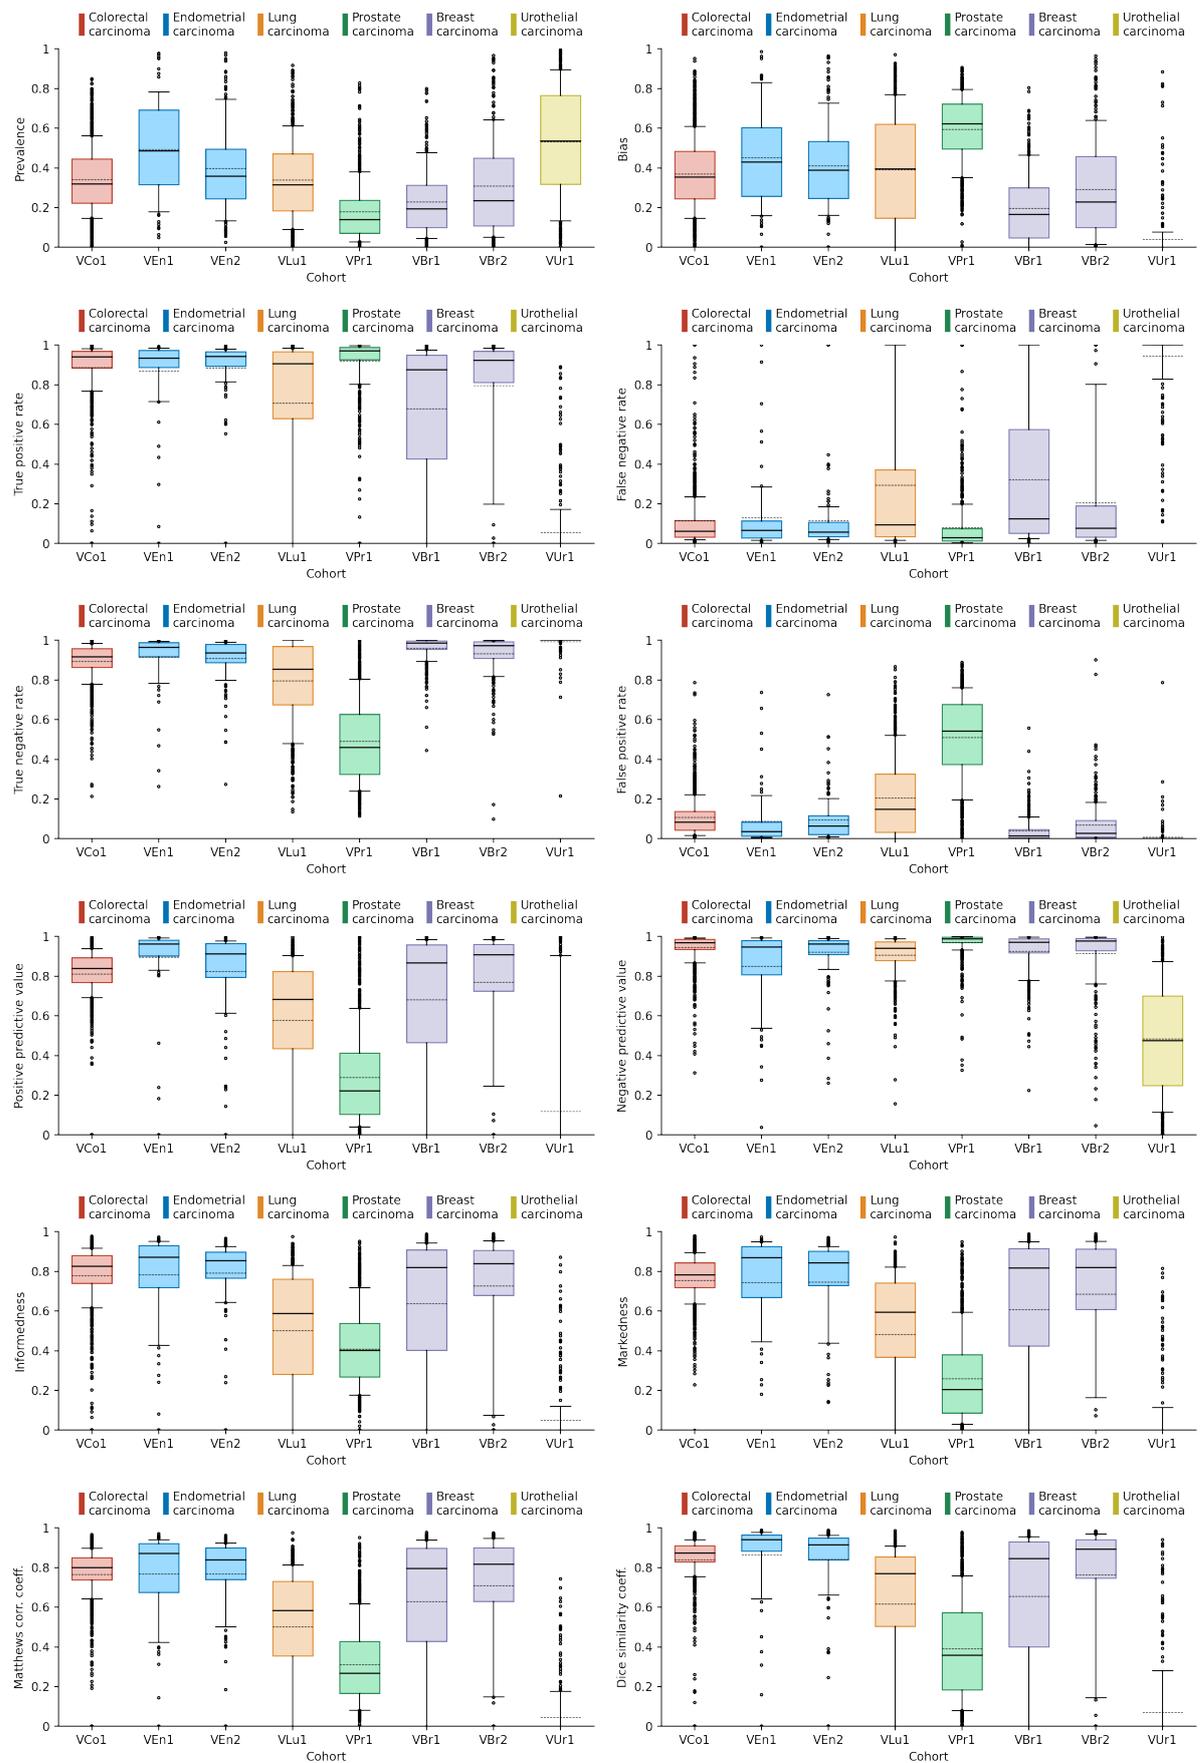

**Figure S3: Colorectal model performance on Aperio AT2 scans**

For each cohort, the plot displays the interquartile range (coloured box), mean value (perforated horizontal line), median value (solid horizontal line), the 10th and 90th percentile (whiskers), and outliers (black circles).

### 1.3.2 Endometrial carcinoma

**Table S4: Endometrial model performance on Aperio AT2 scans**  
Data entries show mean value (95% CI)

| Cohort | Prevalence                | Bias                      |
|--------|---------------------------|---------------------------|
| VCo1   | 0.3410 (0.3315 – 0.3505)  | 0.4541 (0.4431 – 0.4651)  |
| VEn1   | 0.4924 (0.4363 – 0.5485)  | 0.5023 (0.4465 – 0.5582)  |
| VEn2   | 0.3970 (0.3611 – 0.4328)  | 0.4146 (0.3788 – 0.4503)  |
| VLu1   | 0.3380 (0.3208 – 0.3552)  | 0.6098 (0.5891 – 0.6305)  |
| VPr1   | 0.1777 (0.1671 – 0.1882)  | 0.6396 (0.6279 – 0.6513)  |
| VBr1   | 0.2278 (0.2089 – 0.2467)  | 0.2583 (0.2359 – 0.2806)  |
| VBr2   | 0.3081 (0.2808 – 0.3355)  | 0.3690 (0.3395 – 0.3985)  |
| VUr1   | 0.5304 (0.5004 – 0.5603)  | 0.3003 (0.2642 – 0.3364)  |
| Cohort | True positive rate        | False negative rate       |
| VCo1   | 0.9342 (0.9261 – 0.9423)  | 0.0658 (0.0577 – 0.0739)  |
| VEn1   | 0.9689 (0.9605 – 0.9773)  | 0.0311 (0.0227 – 0.0395)  |
| VEn2   | 0.9676 (0.9631 – 0.9721)  | 0.0324 (0.0279 – 0.0369)  |
| VLu1   | 0.9545 (0.9410 – 0.9681)  | 0.0455 (0.0319 – 0.0590)  |
| VPr1   | 0.9703 (0.9639 – 0.9767)  | 0.0297 (0.0233 – 0.0361)  |
| VBr1   | 0.8265 (0.7909 – 0.8620)  | 0.1735 (0.1380 – 0.2091)  |
| VBr2   | 0.9221 (0.8991 – 0.9450)  | 0.0779 (0.0550 – 0.1009)  |
| VUr1   | 0.4105 (0.3669 – 0.4541)  | 0.5895 (0.5459 – 0.6331)  |
| Cohort | True negative rate        | False positive rate       |
| VCo1   | 0.7784 (0.7696 – 0.7871)  | 0.2216 (0.2129 – 0.2304)  |
| VEn1   | 0.9015 (0.8666 – 0.9364)  | 0.0985 (0.0636 – 0.1334)  |
| VEn2   | 0.9208 (0.9011 – 0.9405)  | 0.0792 (0.0595 – 0.0989)  |
| VLu1   | 0.5569 (0.5352 – 0.5786)  | 0.4431 (0.4214 – 0.4648)  |
| VPr1   | 0.4419 (0.4279 – 0.4560)  | 0.5581 (0.5440 – 0.5721)  |
| VBr1   | 0.9080 (0.8941 – 0.9220)  | 0.0920 (0.0780 – 0.1059)  |
| VBr2   | 0.8537 (0.8339 – 0.8735)  | 0.1463 (0.1265 – 0.1661)  |
| VUr1   | 0.8594 (0.8371 – 0.8816)  | 0.1406 (0.1184 – 0.1629)  |
| Cohort | Positive predictive value | Negative predictive value |
| VCo1   | 0.6883 (0.6786 – 0.6980)  | 0.9608 (0.9567 – 0.9650)  |
| VEn1   | 0.9426 (0.9263 – 0.9589)  | 0.9250 (0.8912 – 0.9587)  |
| VEn2   | 0.9109 (0.8949 – 0.9268)  | 0.9572 (0.9442 – 0.9702)  |
| VLu1   | 0.5264 (0.5065 – 0.5463)  | 0.9761 (0.9731 – 0.9791)  |
| VPr1   | 0.2769 (0.2612 – 0.2926)  | 0.9873 (0.9849 – 0.9897)  |
| VBr1   | 0.6715 (0.6373 – 0.7057)  | 0.9586 (0.9474 – 0.9697)  |
| VBr2   | 0.7220 (0.6938 – 0.7502)  | 0.9528 (0.9399 – 0.9656)  |
| VUr1   | 0.4894 (0.4428 – 0.5360)  | 0.6085 (0.5789 – 0.6381)  |
| Cohort | Informedness              | Markedness                |
| VCo1   | 0.7126 (0.7023 – 0.7228)  | 0.6491 (0.6387 – 0.6596)  |
| VEn1   | 0.8704 (0.8351 – 0.9058)  | 0.8676 (0.8326 – 0.9026)  |
| VEn2   | 0.8884 (0.8688 – 0.9079)  | 0.8680 (0.8496 – 0.8865)  |
| VLu1   | 0.5114 (0.4897 – 0.5332)  | 0.5025 (0.4830 – 0.5220)  |
| VPr1   | 0.4122 (0.3985 – 0.4259)  | 0.2642 (0.2493 – 0.2792)  |
| VBr1   | 0.7345 (0.6997 – 0.7693)  | 0.6301 (0.5903 – 0.6699)  |
| VBr2   | 0.7758 (0.7488 – 0.8027)  | 0.6748 (0.6439 – 0.7056)  |
| VUr1   | 0.2699 (0.2392 – 0.3006)  | 0.0979 (0.0421 – 0.1537)  |
| Cohort | Matthews corr. coeff.     | Dice similarity coeff.    |
| VCo1   | 0.6762 (0.6670 – 0.6854)  | 0.7800 (0.7712 – 0.7888)  |
| VEn1   | 0.8661 (0.8314 – 0.9008)  | 0.9534 (0.9432 – 0.9637)  |
| VEn2   | 0.8754 (0.8575 – 0.8934)  | 0.9345 (0.9235 – 0.9454)  |
| VLu1   | 0.4915 (0.4729 – 0.5100)  | 0.6513 (0.6320 – 0.6706)  |
| VPr1   | 0.3116 (0.2980 – 0.3251)  | 0.3884 (0.3712 – 0.4055)  |
| VBr1   | 0.6826 (0.6492 – 0.7161)  | 0.7160 (0.6818 – 0.7502)  |
| VBr2   | 0.7201 (0.6941 – 0.7462)  | 0.7917 (0.7661 – 0.8172)  |
| VUr1   | 0.2651 (0.2356 – 0.2946)  | 0.4216 (0.3791 – 0.4641)  |

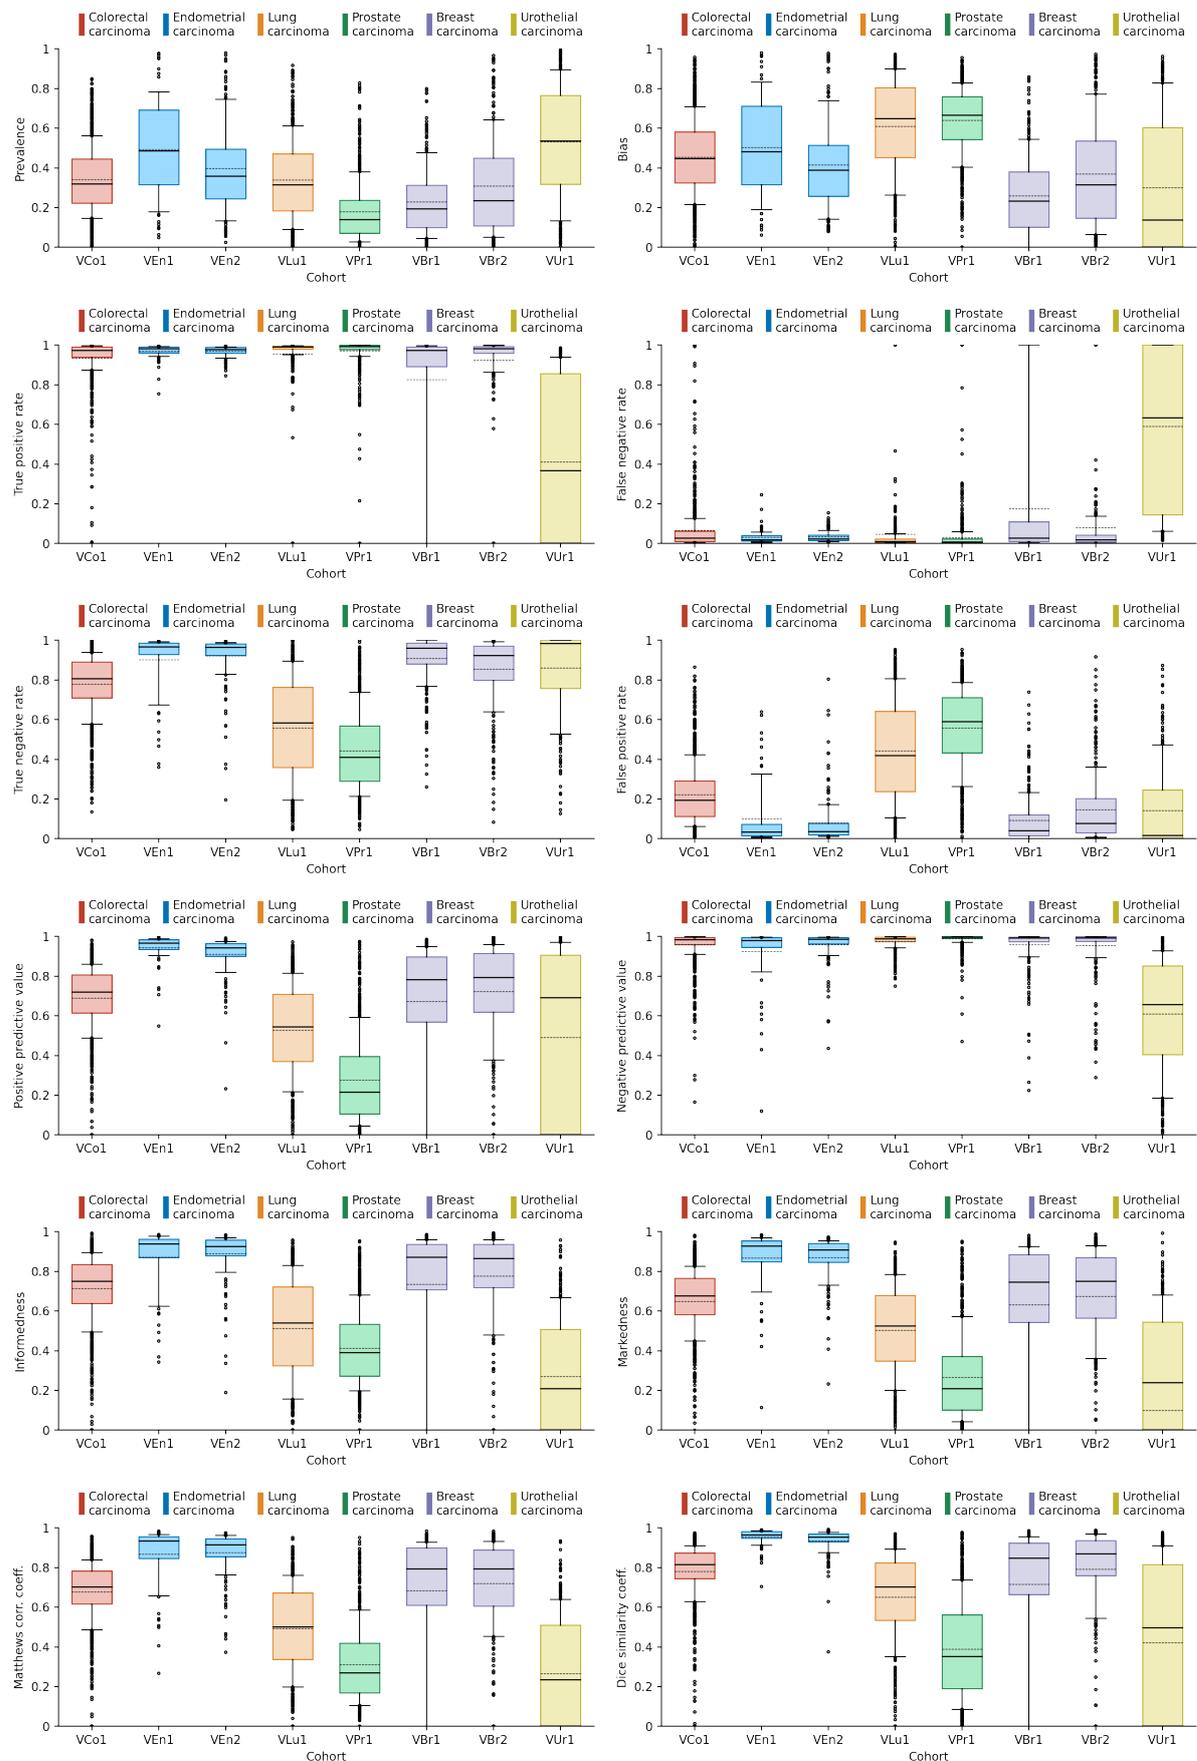

**Figure S4: Endometrial model performance on Aperio AT2 scans**

For each cohort, the plot displays the interquartile range (coloured box), mean value (perforated horizontal line), median value (solid horizontal line), the 10th and 90th percentile (whiskers), and outliers (black circles).

### 1.3.3 Lung carcinoma

**Table S5: Lung model performance on Aperio AT2 scans**  
Data entries show mean value (95% CI)

| Cohort | Prevalence                | Bias                      |
|--------|---------------------------|---------------------------|
| VCo1   | 0.3410 (0.3315 – 0.3505)  | 0.3841 (0.3742 – 0.3940)  |
| VEn1   | 0.4924 (0.4363 – 0.5485)  | 0.4945 (0.4405 – 0.5484)  |
| VEn2   | 0.3970 (0.3611 – 0.4328)  | 0.4451 (0.4110 – 0.4792)  |
| VLu1   | 0.3380 (0.3208 – 0.3552)  | 0.3904 (0.3718 – 0.4091)  |
| VPr1   | 0.1777 (0.1671 – 0.1882)  | 0.2360 (0.2226 – 0.2494)  |
| VBr1   | 0.2278 (0.2089 – 0.2467)  | 0.1989 (0.1796 – 0.2183)  |
| VBr2   | 0.3081 (0.2808 – 0.3355)  | 0.2808 (0.2544 – 0.3071)  |
| VUr1   | 0.5304 (0.5004 – 0.5603)  | 0.3643 (0.3339 – 0.3948)  |
| Cohort | True positive rate        | False negative rate       |
| VCo1   | 0.8697 (0.8602 – 0.8792)  | 0.1303 (0.1208 – 0.1398)  |
| VEn1   | 0.9470 (0.9290 – 0.9650)  | 0.0530 (0.0350 – 0.0710)  |
| VEn2   | 0.9536 (0.9454 – 0.9618)  | 0.0464 (0.0382 – 0.0546)  |
| VLu1   | 0.9171 (0.9017 – 0.9324)  | 0.0829 (0.0676 – 0.0983)  |
| VPr1   | 0.6463 (0.6198 – 0.6729)  | 0.3537 (0.3271 – 0.3802)  |
| VBr1   | 0.7130 (0.6793 – 0.7468)  | 0.2870 (0.2532 – 0.3207)  |
| VBr2   | 0.8023 (0.7750 – 0.8296)  | 0.1977 (0.1704 – 0.2250)  |
| VUr1   | 0.5804 (0.5442 – 0.6166)  | 0.4196 (0.3834 – 0.4558)  |
| Cohort | True negative rate        | False positive rate       |
| VCo1   | 0.8591 (0.8527 – 0.8655)  | 0.1409 (0.1345 – 0.1473)  |
| VEn1   | 0.9073 (0.8799 – 0.9348)  | 0.0927 (0.0652 – 0.1201)  |
| VEn2   | 0.8807 (0.8565 – 0.9049)  | 0.1193 (0.0951 – 0.1435)  |
| VLu1   | 0.8758 (0.8661 – 0.8856)  | 0.1242 (0.1144 – 0.1339)  |
| VPr1   | 0.8675 (0.8571 – 0.8779)  | 0.1325 (0.1221 – 0.1429)  |
| VBr1   | 0.9664 (0.9569 – 0.9759)  | 0.0336 (0.0241 – 0.0431)  |
| VBr2   | 0.9558 (0.9453 – 0.9663)  | 0.0442 (0.0337 – 0.0547)  |
| VUr1   | 0.9320 (0.9219 – 0.9420)  | 0.0680 (0.0580 – 0.0781)  |
| Cohort | Positive predictive value | Negative predictive value |
| VCo1   | 0.7603 (0.7509 – 0.7697)  | 0.9254 (0.9200 – 0.9309)  |
| VEn1   | 0.9246 (0.8976 – 0.9516)  | 0.9058 (0.8694 – 0.9421)  |
| VEn2   | 0.8478 (0.8175 – 0.8780)  | 0.9520 (0.9382 – 0.9657)  |
| VLu1   | 0.7706 (0.7537 – 0.7875)  | 0.9666 (0.9623 – 0.9709)  |
| VPr1   | 0.4593 (0.4351 – 0.4835)  | 0.9379 (0.9314 – 0.9445)  |
| VBr1   | 0.7981 (0.7631 – 0.8332)  | 0.9311 (0.9208 – 0.9413)  |
| VBr2   | 0.8640 (0.8364 – 0.8915)  | 0.9114 (0.8958 – 0.9271)  |
| VUr1   | 0.7497 (0.7092 – 0.7903)  | 0.6697 (0.6426 – 0.6968)  |
| Cohort | Informedness              | Markedness                |
| VCo1   | 0.7288 (0.7185 – 0.7391)  | 0.6857 (0.6757 – 0.6956)  |
| VEn1   | 0.8544 (0.8212 – 0.8875)  | 0.8304 (0.7886 – 0.8721)  |
| VEn2   | 0.8343 (0.8102 – 0.8584)  | 0.7997 (0.7697 – 0.8298)  |
| VLu1   | 0.7929 (0.7770 – 0.8088)  | 0.7372 (0.7196 – 0.7547)  |
| VPr1   | 0.5139 (0.4901 – 0.5376)  | 0.3972 (0.3724 – 0.4221)  |
| VBr1   | 0.6794 (0.6459 – 0.7130)  | 0.7292 (0.6913 – 0.7672)  |
| VBr2   | 0.7581 (0.7305 – 0.7857)  | 0.7754 (0.7425 – 0.8082)  |
| VUr1   | 0.5124 (0.4800 – 0.5447)  | 0.4194 (0.3714 – 0.4674)  |
| Cohort | Matthews corr. coeff.     | Dice similarity coeff.    |
| VCo1   | 0.7048 (0.6955 – 0.7141)  | 0.7972 (0.7885 – 0.8058)  |
| VEn1   | 0.8386 (0.8013 – 0.8759)  | 0.9287 (0.9061 – 0.9512)  |
| VEn2   | 0.8126 (0.7858 – 0.8394)  | 0.8809 (0.8560 – 0.9058)  |
| VLu1   | 0.7620 (0.7466 – 0.7774)  | 0.8278 (0.8120 – 0.8436)  |
| VPr1   | 0.4483 (0.4260 – 0.4706)  | 0.4906 (0.4673 – 0.5139)  |
| VBr1   | 0.7021 (0.6695 – 0.7348)  | 0.7281 (0.6949 – 0.7614)  |
| VBr2   | 0.7645 (0.7373 – 0.7917)  | 0.8126 (0.7853 – 0.8400)  |
| VUr1   | 0.4869 (0.4555 – 0.5182)  | 0.6380 (0.6009 – 0.6752)  |

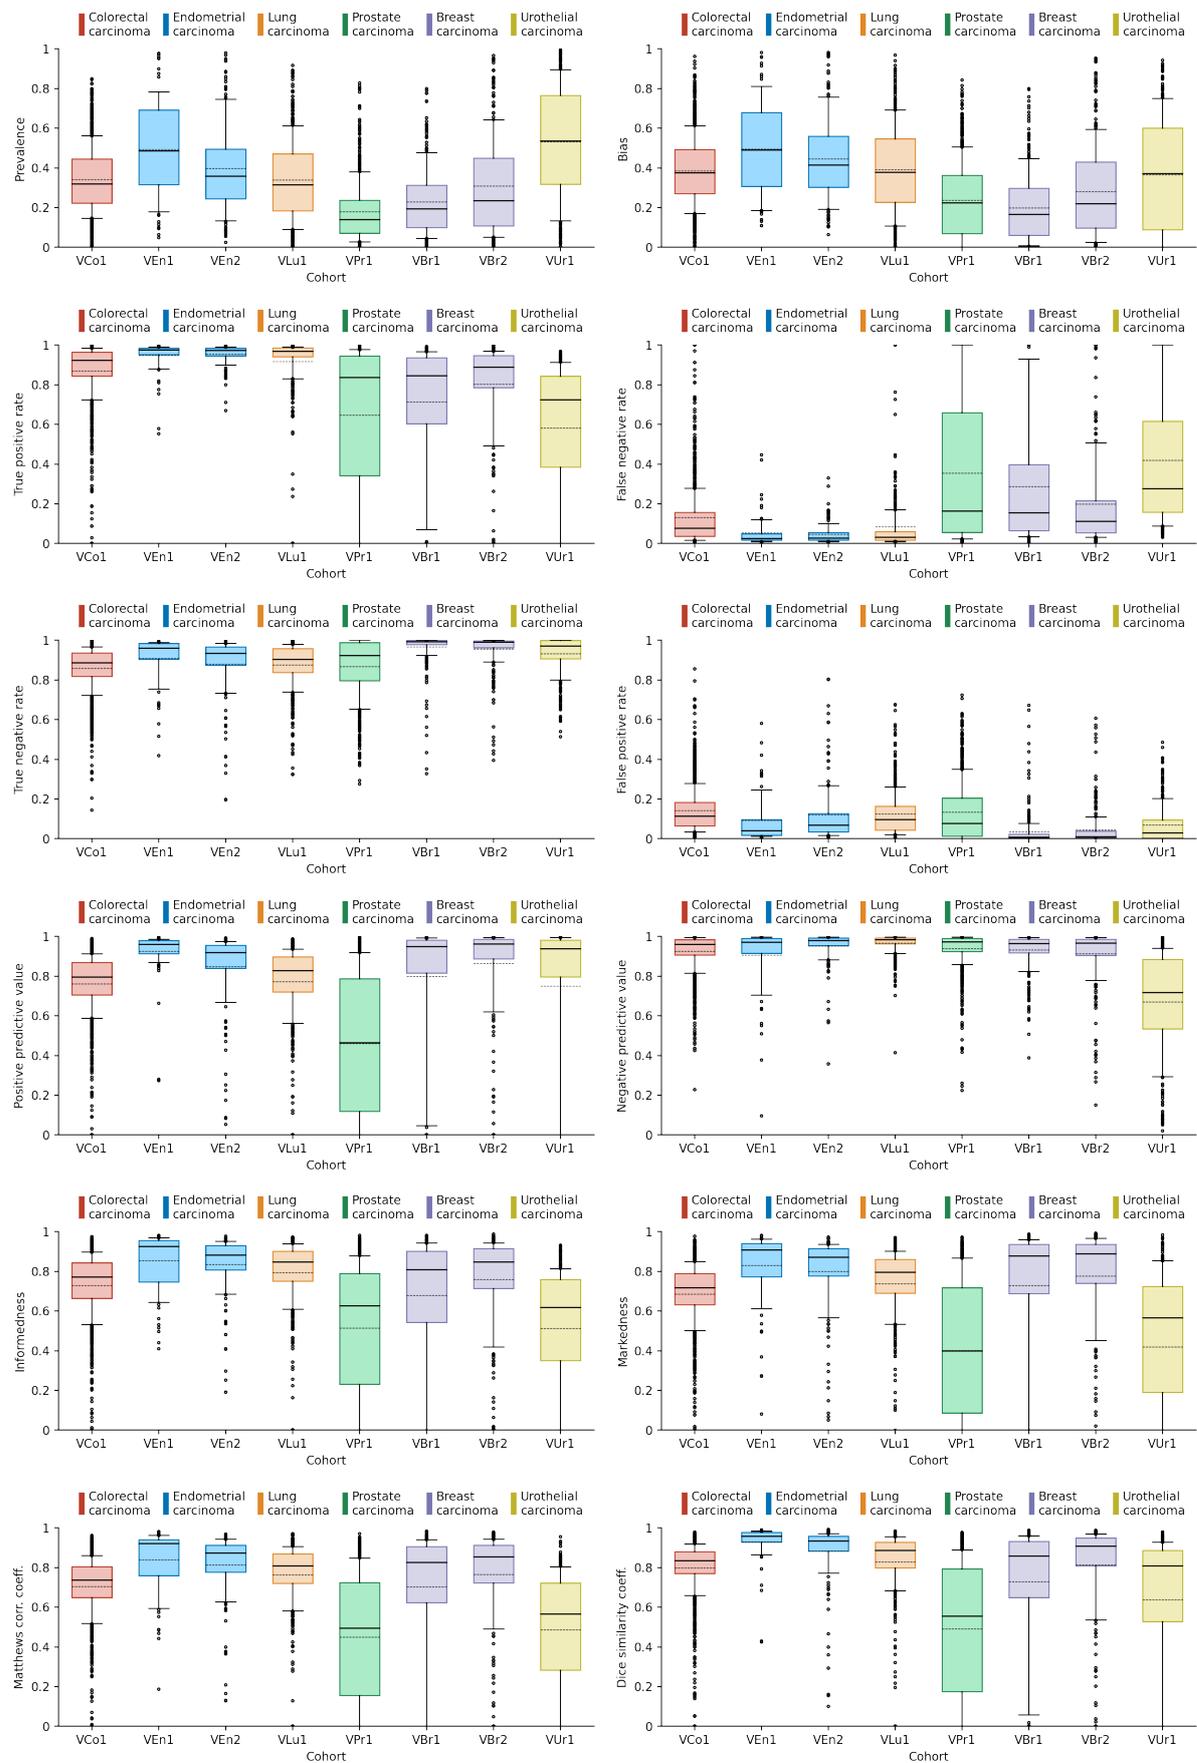

**Figure S5: Lung model performance on Aperio AT2 scans**

For each cohort, the plot displays the interquartile range (coloured box), mean value (perforated horizontal line), median value (solid horizontal line), the 10th and 90th percentile (whiskers), and outliers (black circles).

### 1.3.4 Prostate carcinoma

**Table S6: Prostate model performance on Aperio AT2 scans**  
Data entries show mean value (95% CI)

| Cohort | Prevalence                | Bias                        |
|--------|---------------------------|-----------------------------|
| VCo1   | 0.3410 (0.3315 – 0.3505)  | 0.3655 (0.3537 – 0.3773)    |
| VEn1   | 0.4924 (0.4363 – 0.5485)  | 0.5333 (0.4816 – 0.5850)    |
| VEn2   | 0.3970 (0.3611 – 0.4328)  | 0.4953 (0.4540 – 0.5366)    |
| VLu1   | 0.3380 (0.3208 – 0.3552)  | 0.4121 (0.3875 – 0.4366)    |
| VPr1   | 0.1777 (0.1671 – 0.1882)  | 0.1732 (0.1627 – 0.1838)    |
| VBr1   | 0.2278 (0.2089 – 0.2467)  | 0.2004 (0.1816 – 0.2191)    |
| VBr2   | 0.3081 (0.2808 – 0.3355)  | 0.2837 (0.2573 – 0.3101)    |
| VUr1   | 0.5304 (0.5004 – 0.5603)  | 0.0809 (0.0623 – 0.0995)    |
| Cohort | True positive rate        | False negative rate         |
| VCo1   | 0.7686 (0.7506 – 0.7866)  | 0.2314 (0.2134 – 0.2494)    |
| VEn1   | 0.8834 (0.8402 – 0.9266)  | 0.1166 (0.0734 – 0.1598)    |
| VEn2   | 0.8232 (0.7767 – 0.8697)  | 0.1768 (0.1303 – 0.2233)    |
| VLu1   | 0.6955 (0.6646 – 0.7264)  | 0.3045 (0.2736 – 0.3354)    |
| VPr1   | 0.8434 (0.8336 – 0.8531)  | 0.1566 (0.1469 – 0.1664)    |
| VBr1   | 0.7669 (0.7326 – 0.8012)  | 0.2331 (0.1988 – 0.2674)    |
| VBr2   | 0.8401 (0.8133 – 0.8669)  | 0.1599 (0.1331 – 0.1867)    |
| VUr1   | 0.1288 (0.1031 – 0.1546)  | 0.8712 (0.8454 – 0.8969)    |
| Cohort | True negative rate        | False positive rate         |
| VCo1   | 0.8313 (0.8238 – 0.8388)  | 0.1687 (0.1612 – 0.1762)    |
| VEn1   | 0.8011 (0.7482 – 0.8539)  | 0.1989 (0.1461 – 0.2518)    |
| VEn2   | 0.7338 (0.6966 – 0.7711)  | 0.2662 (0.2289 – 0.3034)    |
| VLu1   | 0.7514 (0.7313 – 0.7715)  | 0.2486 (0.2285 – 0.2687)    |
| VPr1   | 0.9753 (0.9725 – 0.9781)  | 0.0247 (0.0219 – 0.0275)    |
| VBr1   | 0.9701 (0.9649 – 0.9754)  | 0.0299 (0.0246 – 0.0351)    |
| VBr2   | 0.9523 (0.9427 – 0.9619)  | 0.0477 (0.0381 – 0.0573)    |
| VUr1   | 0.9871 (0.9817 – 0.9925)  | 0.0129 (0.0075 – 0.0183)    |
| Cohort | Positive predictive value | Negative predictive value   |
| VCo1   | 0.6430 (0.6287 – 0.6573)  | 0.8909 (0.8824 – 0.8994)    |
| VEn1   | 0.8126 (0.7535 – 0.8716)  | 0.8578 (0.8086 – 0.9070)    |
| VEn2   | 0.6367 (0.5877 – 0.6857)  | 0.8885 (0.8635 – 0.9135)    |
| VLu1   | 0.5504 (0.5241 – 0.5767)  | 0.8887 (0.8782 – 0.8993)    |
| VPr1   | 0.8717 (0.8626 – 0.8808)  | 0.9703 (0.9677 – 0.9730)    |
| VBr1   | 0.7956 (0.7624 – 0.8288)  | 0.9407 (0.9293 – 0.9521)    |
| VBr2   | 0.8525 (0.8274 – 0.8776)  | 0.9202 (0.9039 – 0.9365)    |
| VUr1   | 0.3673 (0.3164 – 0.4182)  | 0.5071 (0.4771 – 0.5371)    |
| Cohort | Informedness              | Markedness                  |
| VCo1   | 0.5999 (0.5843 – 0.6156)  | 0.5339 (0.5156 – 0.5522)    |
| VEn1   | 0.6845 (0.6257 – 0.7433)  | 0.6703 (0.6063 – 0.7343)    |
| VEn2   | 0.5571 (0.5110 – 0.6031)  | 0.5252 (0.4696 – 0.5809)    |
| VLu1   | 0.4469 (0.4219 – 0.4720)  | 0.4391 (0.4098 – 0.4684)    |
| VPr1   | 0.8187 (0.8091 – 0.8283)  | 0.8420 (0.8330 – 0.8510)    |
| VBr1   | 0.7370 (0.7036 – 0.7705)  | 0.7363 (0.6975 – 0.7752)    |
| VBr2   | 0.7924 (0.7658 – 0.8191)  | 0.7727 (0.7399 – 0.8055)    |
| VUr1   | 0.1159 (0.0931 – 0.1387)  | -0.1256 (-0.1844 – -0.0668) |
| Cohort | Matthews corr. coeff.     | Dice similarity coeff.      |
| VCo1   | 0.5739 (0.5594 – 0.5884)  | 0.6767 (0.6615 – 0.6920)    |
| VEn1   | 0.6719 (0.6112 – 0.7327)  | 0.8084 (0.7570 – 0.8599)    |
| VEn2   | 0.5454 (0.5001 – 0.5907)  | 0.6864 (0.6405 – 0.7323)    |
| VLu1   | 0.4475 (0.4237 – 0.4713)  | 0.5794 (0.5527 – 0.6060)    |
| VPr1   | 0.8273 (0.8188 – 0.8357)  | 0.8498 (0.8412 – 0.8585)    |
| VBr1   | 0.7381 (0.7060 – 0.7702)  | 0.7589 (0.7259 – 0.7919)    |
| VBr2   | 0.7828 (0.7571 – 0.8086)  | 0.8306 (0.8049 – 0.8563)    |
| VUr1   | 0.1307 (0.1073 – 0.1540)  | 0.1665 (0.1365 – 0.1965)    |

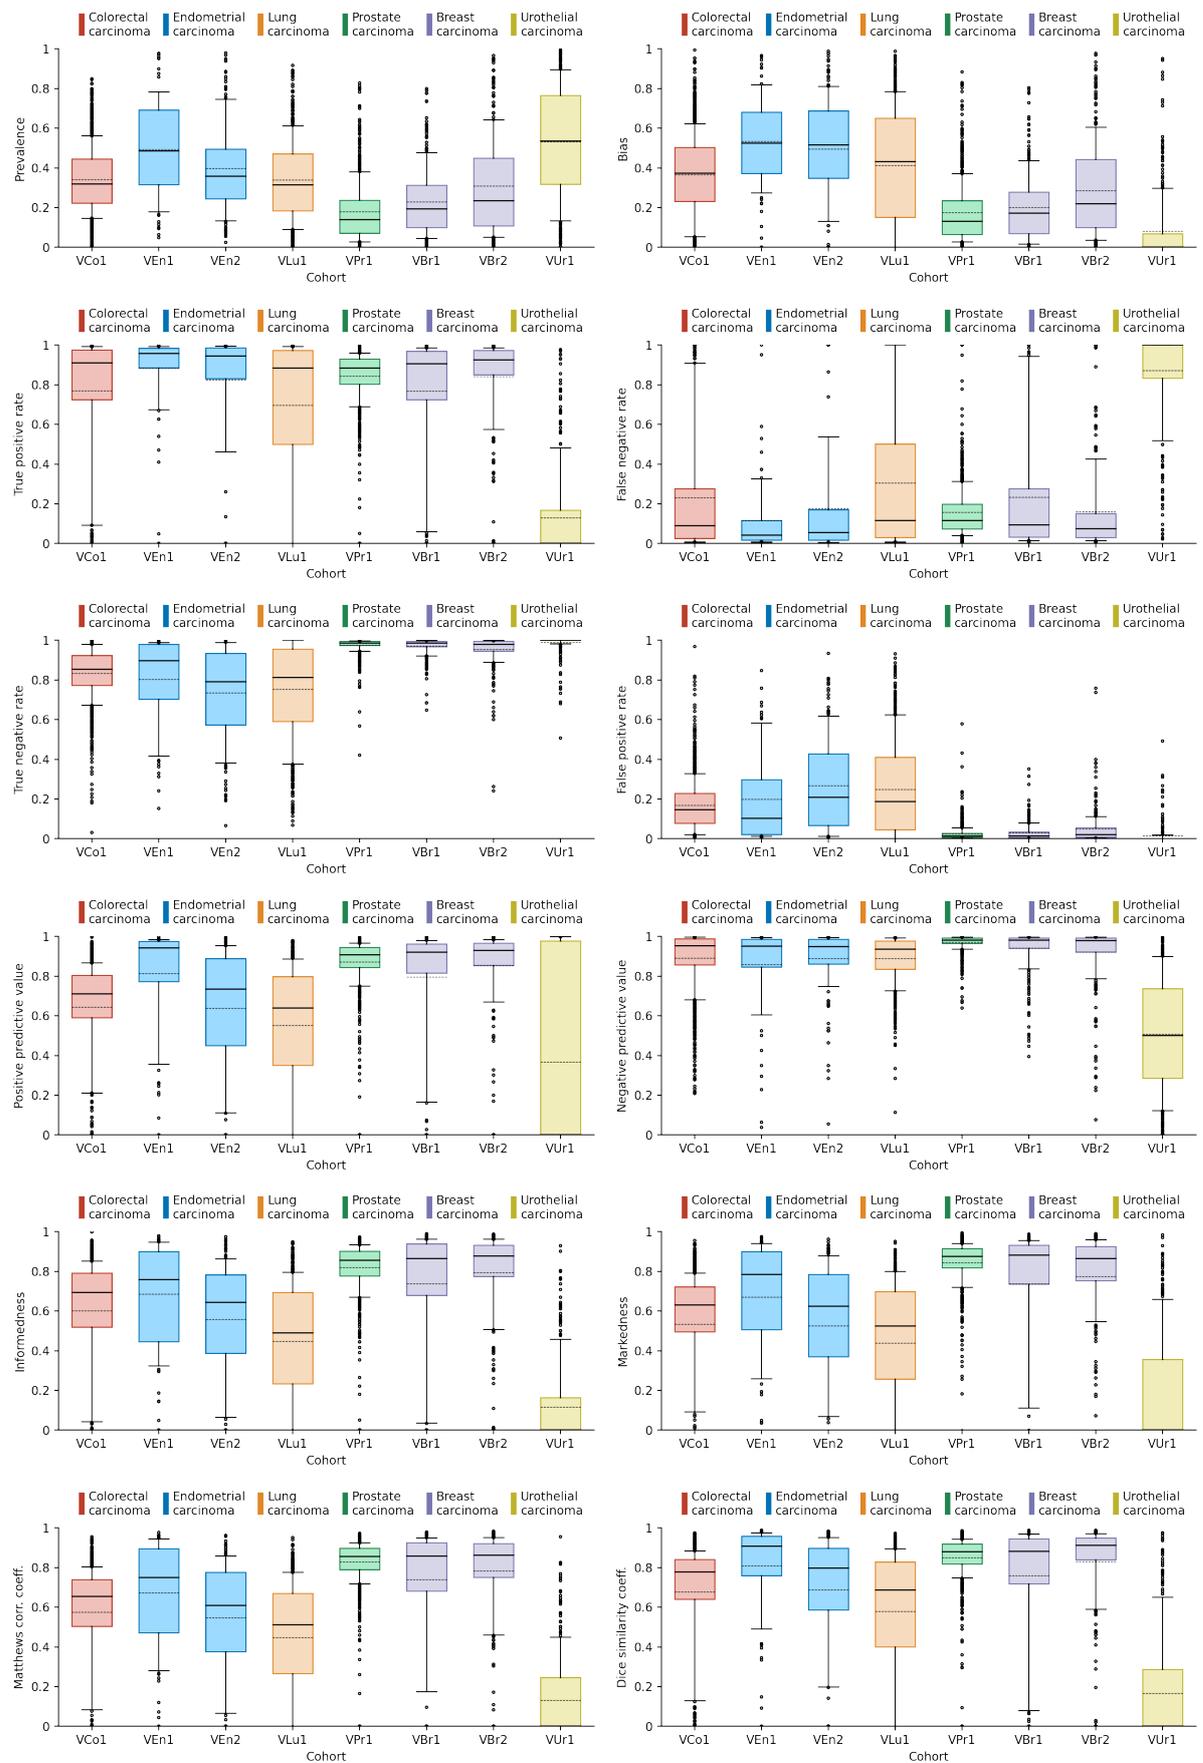

**Figure S6: Prostate model performance on Aperio AT2 scans**

For each cohort, the plot displays the interquartile range (coloured box), mean value (perforated horizontal line), median value (solid horizontal line), the 10th and 90th percentile (whiskers), and outliers (black circles).

## 1.4 Primary model replication performance (study protocol section 3.2.4)

### 1.4.1 Replication 1

**Table S7: First primary model replica performance on Aperio AT2 scans**  
Data entries show mean value (95% CI)

| Cohort | Prevalence                | Bias                      |
|--------|---------------------------|---------------------------|
| VCo1   | 0.3410 (0.3315 – 0.3505)  | 0.3746 (0.3647 – 0.3845)  |
| VEn1   | 0.4924 (0.4363 – 0.5485)  | 0.4993 (0.4432 – 0.5553)  |
| VEn2   | 0.3970 (0.3611 – 0.4328)  | 0.4141 (0.3782 – 0.4500)  |
| VLu1   | 0.3380 (0.3208 – 0.3552)  | 0.3967 (0.3777 – 0.4156)  |
| VPr1   | 0.1777 (0.1671 – 0.1882)  | 0.1820 (0.1713 – 0.1926)  |
| VBr1   | 0.2278 (0.2089 – 0.2467)  | 0.2139 (0.1958 – 0.2320)  |
| VBr2   | 0.3081 (0.2808 – 0.3355)  | 0.2974 (0.2709 – 0.3240)  |
| VUr1   | 0.5304 (0.5004 – 0.5603)  | 0.2726 (0.2416 – 0.3036)  |
| Cohort | True positive rate        | False negative rate       |
| VCo1   | 0.9015 (0.8942 – 0.9088)  | 0.0985 (0.0912 – 0.1058)  |
| VEn1   | 0.9662 (0.9579 – 0.9745)  | 0.0338 (0.0255 – 0.0421)  |
| VEn2   | 0.9647 (0.9595 – 0.9698)  | 0.0353 (0.0302 – 0.0405)  |
| VLu1   | 0.9062 (0.8892 – 0.9232)  | 0.0938 (0.0768 – 0.1108)  |
| VPr1   | 0.8673 (0.8564 – 0.8781)  | 0.1327 (0.1219 – 0.1436)  |
| VBr1   | 0.8344 (0.8091 – 0.8597)  | 0.1656 (0.1403 – 0.1909)  |
| VBr2   | 0.8892 (0.8721 – 0.9064)  | 0.1108 (0.0936 – 0.1279)  |
| VUr1   | 0.4238 (0.3845 – 0.4630)  | 0.5762 (0.5370 – 0.6155)  |
| Cohort | True negative rate        | False positive rate       |
| VCo1   | 0.8872 (0.8819 – 0.8924)  | 0.1128 (0.1076 – 0.1181)  |
| VEn1   | 0.9102 (0.8782 – 0.9422)  | 0.0898 (0.0578 – 0.1218)  |
| VEn2   | 0.9201 (0.9010 – 0.9391)  | 0.0799 (0.0609 – 0.0990)  |
| VLu1   | 0.8645 (0.8538 – 0.8752)  | 0.1355 (0.1248 – 0.1462)  |
| VPr1   | 0.9686 (0.9656 – 0.9716)  | 0.0314 (0.0284 – 0.0344)  |
| VBr1   | 0.9715 (0.9658 – 0.9772)  | 0.0285 (0.0228 – 0.0342)  |
| VBr2   | 0.9587 (0.9510 – 0.9665)  | 0.0413 (0.0335 – 0.0490)  |
| VUr1   | 0.9402 (0.9285 – 0.9520)  | 0.0598 (0.0480 – 0.0715)  |
| Cohort | Positive predictive value | Negative predictive value |
| VCo1   | 0.8061 (0.7986 – 0.8135)  | 0.9413 (0.9369 – 0.9456)  |
| VEn1   | 0.9474 (0.9318 – 0.9630)  | 0.9265 (0.8960 – 0.9569)  |
| VEn2   | 0.9112 (0.8952 – 0.9272)  | 0.9573 (0.9446 – 0.9701)  |
| VLu1   | 0.7552 (0.7372 – 0.7733)  | 0.9661 (0.9620 – 0.9701)  |
| VPr1   | 0.8354 (0.8246 – 0.8463)  | 0.9744 (0.9716 – 0.9772)  |
| VBr1   | 0.8471 (0.8206 – 0.8736)  | 0.9532 (0.9445 – 0.9619)  |
| VBr2   | 0.8896 (0.8709 – 0.9082)  | 0.9352 (0.9223 – 0.9481)  |
| VUr1   | 0.6053 (0.5570 – 0.6536)  | 0.6065 (0.5779 – 0.6351)  |
| Cohort | Informedness              | Markedness                |
| VCo1   | 0.7887 (0.7805 – 0.7968)  | 0.7474 (0.7390 – 0.7557)  |
| VEn1   | 0.8765 (0.8437 – 0.9092)  | 0.8739 (0.8414 – 0.9063)  |
| VEn2   | 0.8848 (0.8658 – 0.9037)  | 0.8685 (0.8501 – 0.8869)  |
| VLu1   | 0.7707 (0.7533 – 0.7881)  | 0.7213 (0.7025 – 0.7401)  |
| VPr1   | 0.8359 (0.8252 – 0.8466)  | 0.8099 (0.7991 – 0.8207)  |
| VBr1   | 0.8059 (0.7807 – 0.8312)  | 0.8003 (0.7706 – 0.8299)  |
| VBr2   | 0.8480 (0.8303 – 0.8657)  | 0.8248 (0.8011 – 0.8485)  |
| VUr1   | 0.3640 (0.3302 – 0.3978)  | 0.2117 (0.1538 – 0.2697)  |
| Cohort | Matthews corr. coeff.     | Dice similarity coeff.    |
| VCo1   | 0.7670 (0.7595 – 0.7746)  | 0.8453 (0.8387 – 0.8519)  |
| VEn1   | 0.8735 (0.8416 – 0.9055)  | 0.9552 (0.9444 – 0.9660)  |
| VEn2   | 0.8740 (0.8563 – 0.8917)  | 0.9332 (0.9221 – 0.9443)  |
| VLu1   | 0.7432 (0.7264 – 0.7601)  | 0.8137 (0.7963 – 0.8310)  |
| VPr1   | 0.8195 (0.8095 – 0.8296)  | 0.8429 (0.8326 – 0.8532)  |
| VBr1   | 0.7994 (0.7745 – 0.8243)  | 0.8213 (0.7956 – 0.8470)  |
| VBr2   | 0.8361 (0.8183 – 0.8538)  | 0.8814 (0.8645 – 0.8984)  |
| VUr1   | 0.3520 (0.3200 – 0.3840)  | 0.4766 (0.4352 – 0.5179)  |

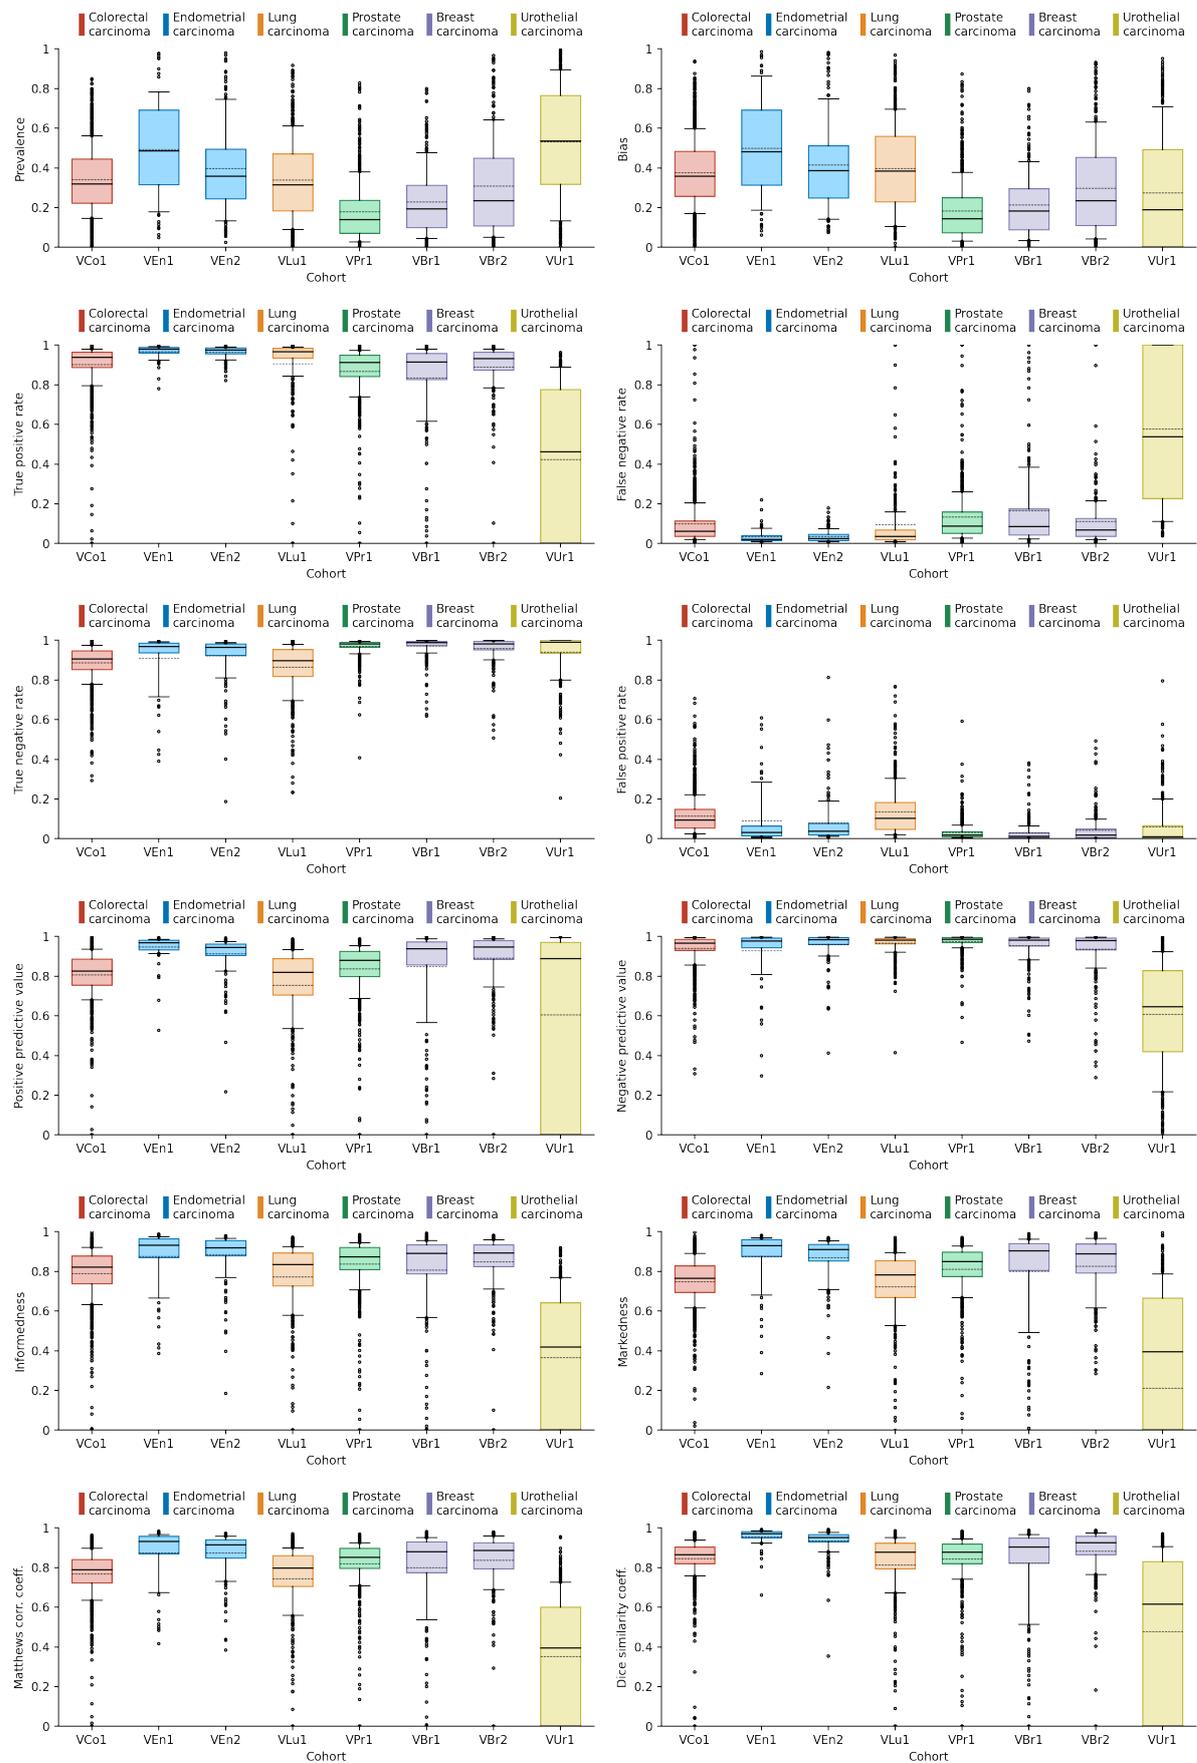

**Figure S7: First primary model replica performance on Aperio AT2 scans**

For each cohort, the plot displays the interquartile range (coloured box), mean value (perforated horizontal line), median value (solid horizontal line), the 10th and 90th percentile (whiskers), and outliers (black circles).

## 1.4.2 Replication 2

**Table S8: Second primary model replica performance on Aperio AT2 scans**  
Data entries show mean value (95% CI)

| Cohort | Prevalence                | Bias                      |
|--------|---------------------------|---------------------------|
| VCo1   | 0.3410 (0.3315 – 0.3505)  | 0.3744 (0.3644 – 0.3845)  |
| VEn1   | 0.4924 (0.4363 – 0.5485)  | 0.5010 (0.4448 – 0.5573)  |
| VEn2   | 0.3970 (0.3611 – 0.4328)  | 0.4162 (0.3800 – 0.4524)  |
| VLu1   | 0.3380 (0.3208 – 0.3552)  | 0.4058 (0.3865 – 0.4251)  |
| VPr1   | 0.1777 (0.1671 – 0.1882)  | 0.1803 (0.1695 – 0.1911)  |
| VBr1   | 0.2278 (0.2089 – 0.2467)  | 0.2136 (0.1951 – 0.2320)  |
| VBr2   | 0.3081 (0.2808 – 0.3355)  | 0.2977 (0.2708 – 0.3245)  |
| VUr1   | 0.5304 (0.5004 – 0.5603)  | 0.2337 (0.2026 – 0.2648)  |
| Cohort | True positive rate        | False negative rate       |
| VCo1   | 0.8970 (0.8886 – 0.9054)  | 0.1030 (0.0946 – 0.1114)  |
| VEn1   | 0.9668 (0.9585 – 0.9750)  | 0.0332 (0.0250 – 0.0415)  |
| VEn2   | 0.9665 (0.9616 – 0.9714)  | 0.0335 (0.0286 – 0.0384)  |
| VLu1   | 0.9130 (0.8960 – 0.9301)  | 0.0870 (0.0699 – 0.1040)  |
| VPr1   | 0.8536 (0.8414 – 0.8657)  | 0.1464 (0.1343 – 0.1586)  |
| VBr1   | 0.8232 (0.7973 – 0.8491)  | 0.1768 (0.1509 – 0.2027)  |
| VBr2   | 0.8825 (0.8651 – 0.9000)  | 0.1175 (0.1000 – 0.1349)  |
| VUr1   | 0.3435 (0.3039 – 0.3832)  | 0.6565 (0.6168 – 0.6961)  |
| Cohort | True negative rate        | False positive rate       |
| VCo1   | 0.8870 (0.8816 – 0.8924)  | 0.1130 (0.1076 – 0.1184)  |
| VEn1   | 0.9028 (0.8675 – 0.9380)  | 0.0972 (0.0620 – 0.1325)  |
| VEn2   | 0.9152 (0.8944 – 0.9360)  | 0.0848 (0.0640 – 0.1056)  |
| VLu1   | 0.8518 (0.8402 – 0.8634)  | 0.1482 (0.1366 – 0.1598)  |
| VPr1   | 0.9698 (0.9666 – 0.9730)  | 0.0302 (0.0270 – 0.0334)  |
| VBr1   | 0.9719 (0.9660 – 0.9778)  | 0.0281 (0.0222 – 0.0340)  |
| VBr2   | 0.9568 (0.9482 – 0.9654)  | 0.0432 (0.0346 – 0.0518)  |
| VUr1   | 0.9428 (0.9307 – 0.9548)  | 0.0572 (0.0452 – 0.0693)  |
| Cohort | Positive predictive value | Negative predictive value |
| VCo1   | 0.8022 (0.7940 – 0.8105)  | 0.9421 (0.9378 – 0.9464)  |
| VEn1   | 0.9454 (0.9301 – 0.9607)  | 0.9269 (0.8959 – 0.9580)  |
| VEn2   | 0.9097 (0.8936 – 0.9257)  | 0.9597 (0.9480 – 0.9714)  |
| VLu1   | 0.7448 (0.7266 – 0.7630)  | 0.9700 (0.9660 – 0.9739)  |
| VPr1   | 0.8402 (0.8285 – 0.8519)  | 0.9745 (0.9720 – 0.9771)  |
| VBr1   | 0.8519 (0.8251 – 0.8788)  | 0.9538 (0.9458 – 0.9617)  |
| VBr2   | 0.8970 (0.8791 – 0.9149)  | 0.9375 (0.9256 – 0.9494)  |
| VUr1   | 0.5032 (0.4531 – 0.5534)  | 0.5826 (0.5540 – 0.6111)  |
| Cohort | Informedness              | Markedness                |
| VCo1   | 0.7840 (0.7751 – 0.7930)  | 0.7444 (0.7351 – 0.7536)  |
| VEn1   | 0.8695 (0.8338 – 0.9052)  | 0.8723 (0.8396 – 0.9051)  |
| VEn2   | 0.8817 (0.8613 – 0.9021)  | 0.8694 (0.8514 – 0.8874)  |
| VLu1   | 0.7648 (0.7472 – 0.7825)  | 0.7148 (0.6959 – 0.7337)  |
| VPr1   | 0.8234 (0.8115 – 0.8352)  | 0.8148 (0.8032 – 0.8264)  |
| VBr1   | 0.7951 (0.7694 – 0.8208)  | 0.8057 (0.7767 – 0.8347)  |
| VBr2   | 0.8394 (0.8213 – 0.8574)  | 0.8345 (0.8125 – 0.8565)  |
| VUr1   | 0.2863 (0.2529 – 0.3198)  | 0.0858 (0.0278 – 0.1438)  |
| Cohort | Matthews corr. coeff.     | Dice similarity coeff.    |
| VCo1   | 0.7637 (0.7554 – 0.7720)  | 0.8411 (0.8335 – 0.8487)  |
| VEn1   | 0.8692 (0.8355 – 0.9029)  | 0.9545 (0.9441 – 0.9649)  |
| VEn2   | 0.8728 (0.8546 – 0.8911)  | 0.9333 (0.9221 – 0.9445)  |
| VLu1   | 0.7366 (0.7197 – 0.7536)  | 0.8095 (0.7920 – 0.8269)  |
| VPr1   | 0.8160 (0.8050 – 0.8270)  | 0.8388 (0.8275 – 0.8501)  |
| VBr1   | 0.7969 (0.7715 – 0.8223)  | 0.8202 (0.7943 – 0.8461)  |
| VBr2   | 0.8352 (0.8176 – 0.8528)  | 0.8804 (0.8635 – 0.8973)  |
| VUr1   | 0.2751 (0.2439 – 0.3063)  | 0.3875 (0.3454 – 0.4295)  |

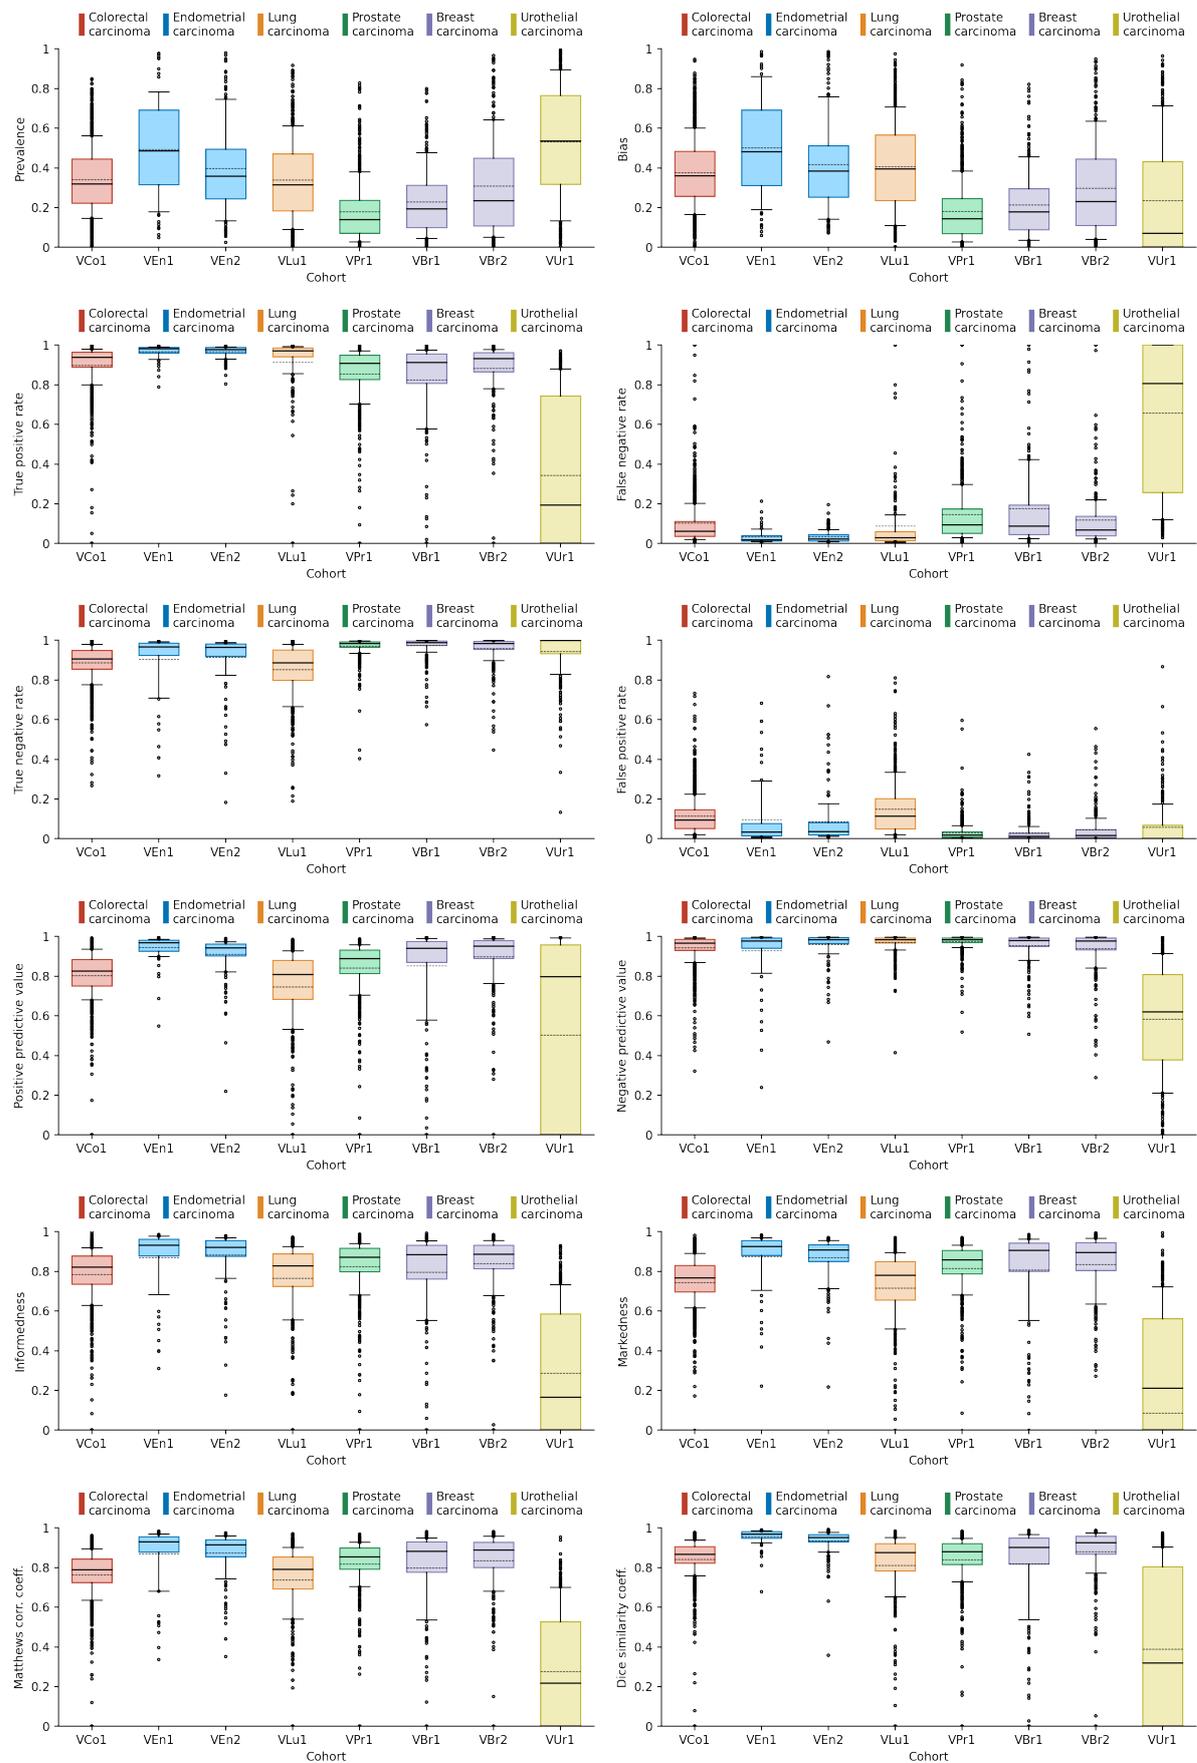

**Figure S8: Second primary model replica performance on Aperio AT2 scans**

For each cohort, the plot displays the interquartile range (coloured box), mean value (perforated horizontal line), median value (solid horizontal line), the 10th and 90th percentile (whiskers), and outliers (black circles).

## 2 Results from exploratory analyses

### 2.1 Association analyses in primary model

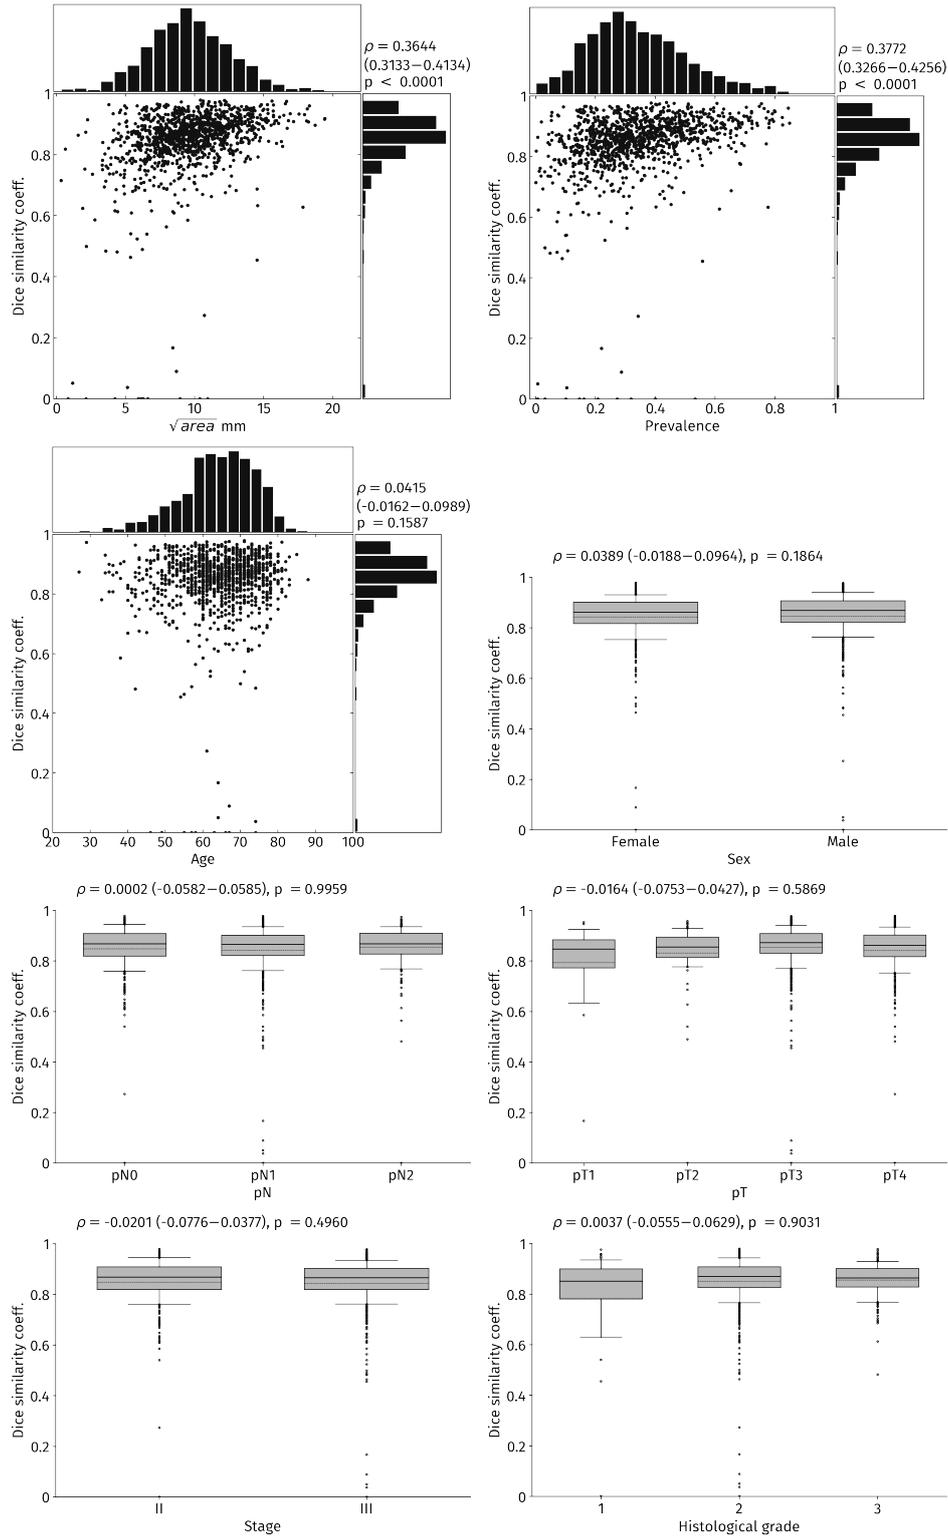

Figure S9: Associations of primary analysis result in VCo1

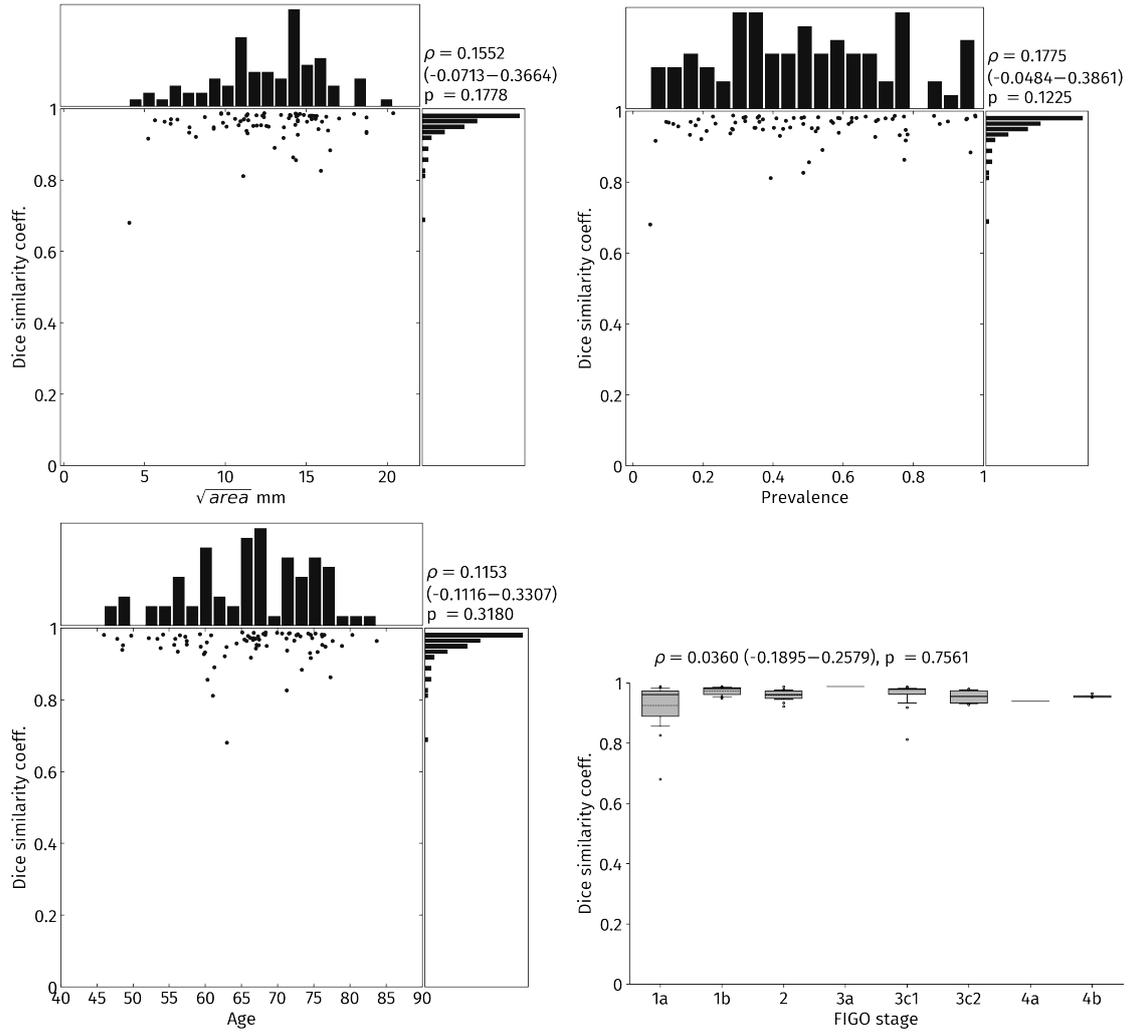

**Figure S10: Associations of primary analysis result in VEN1**

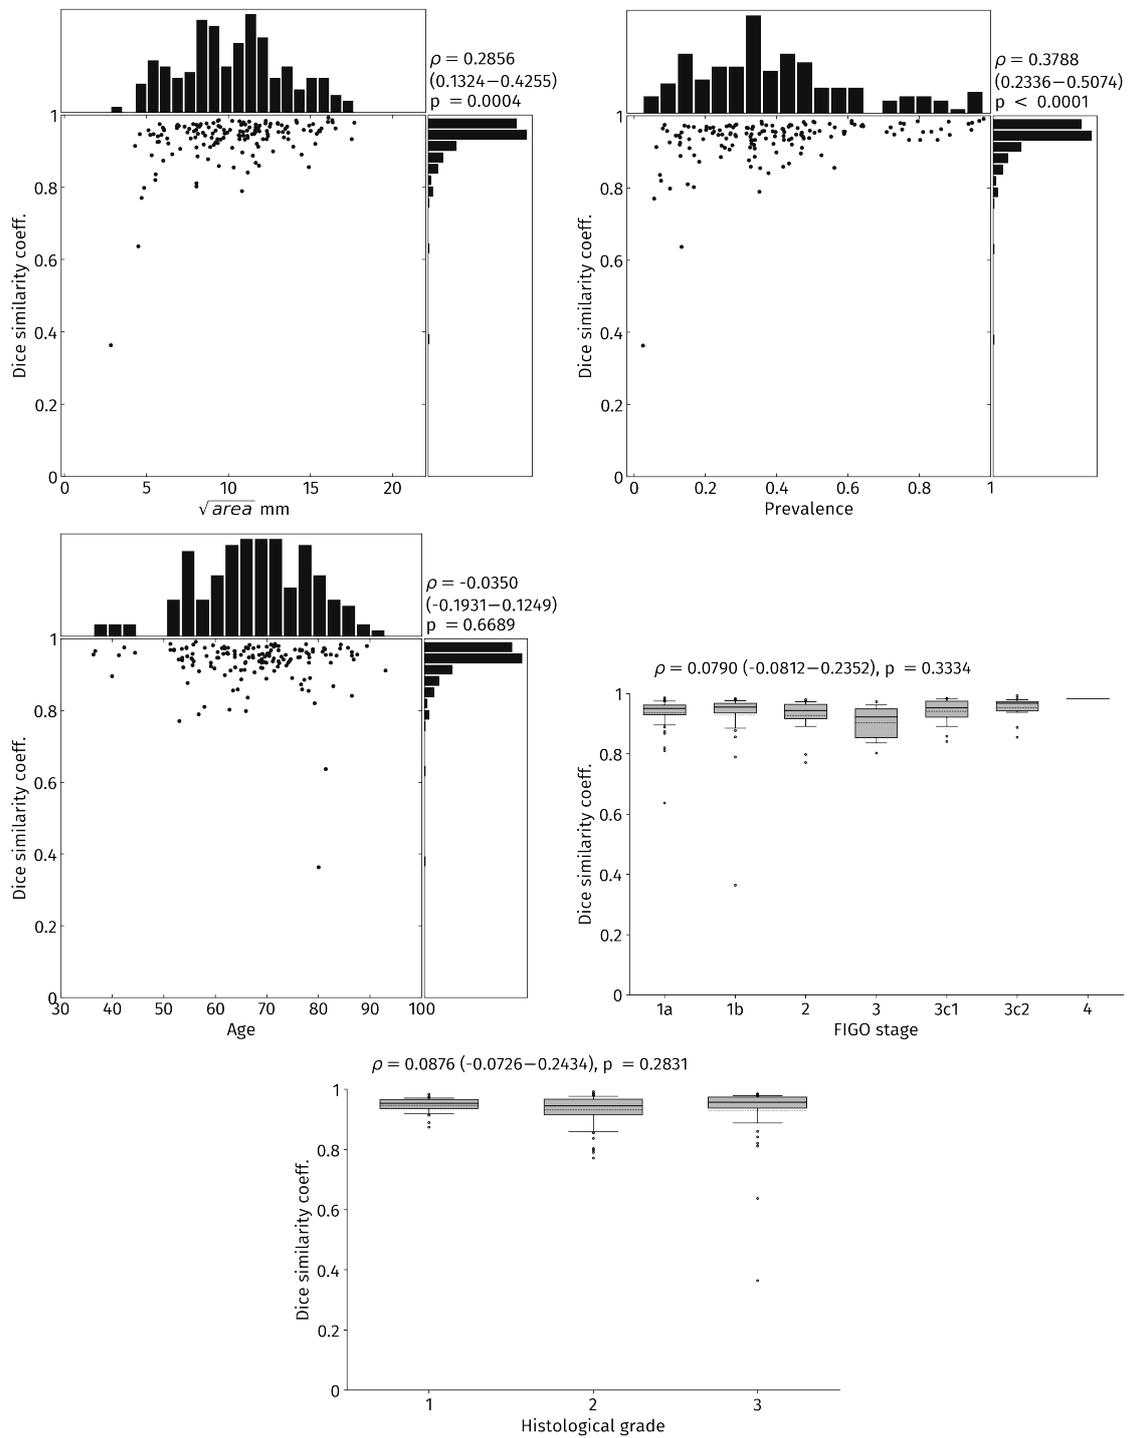

**Figure S11: Associations of primary analysis result in VEN2**

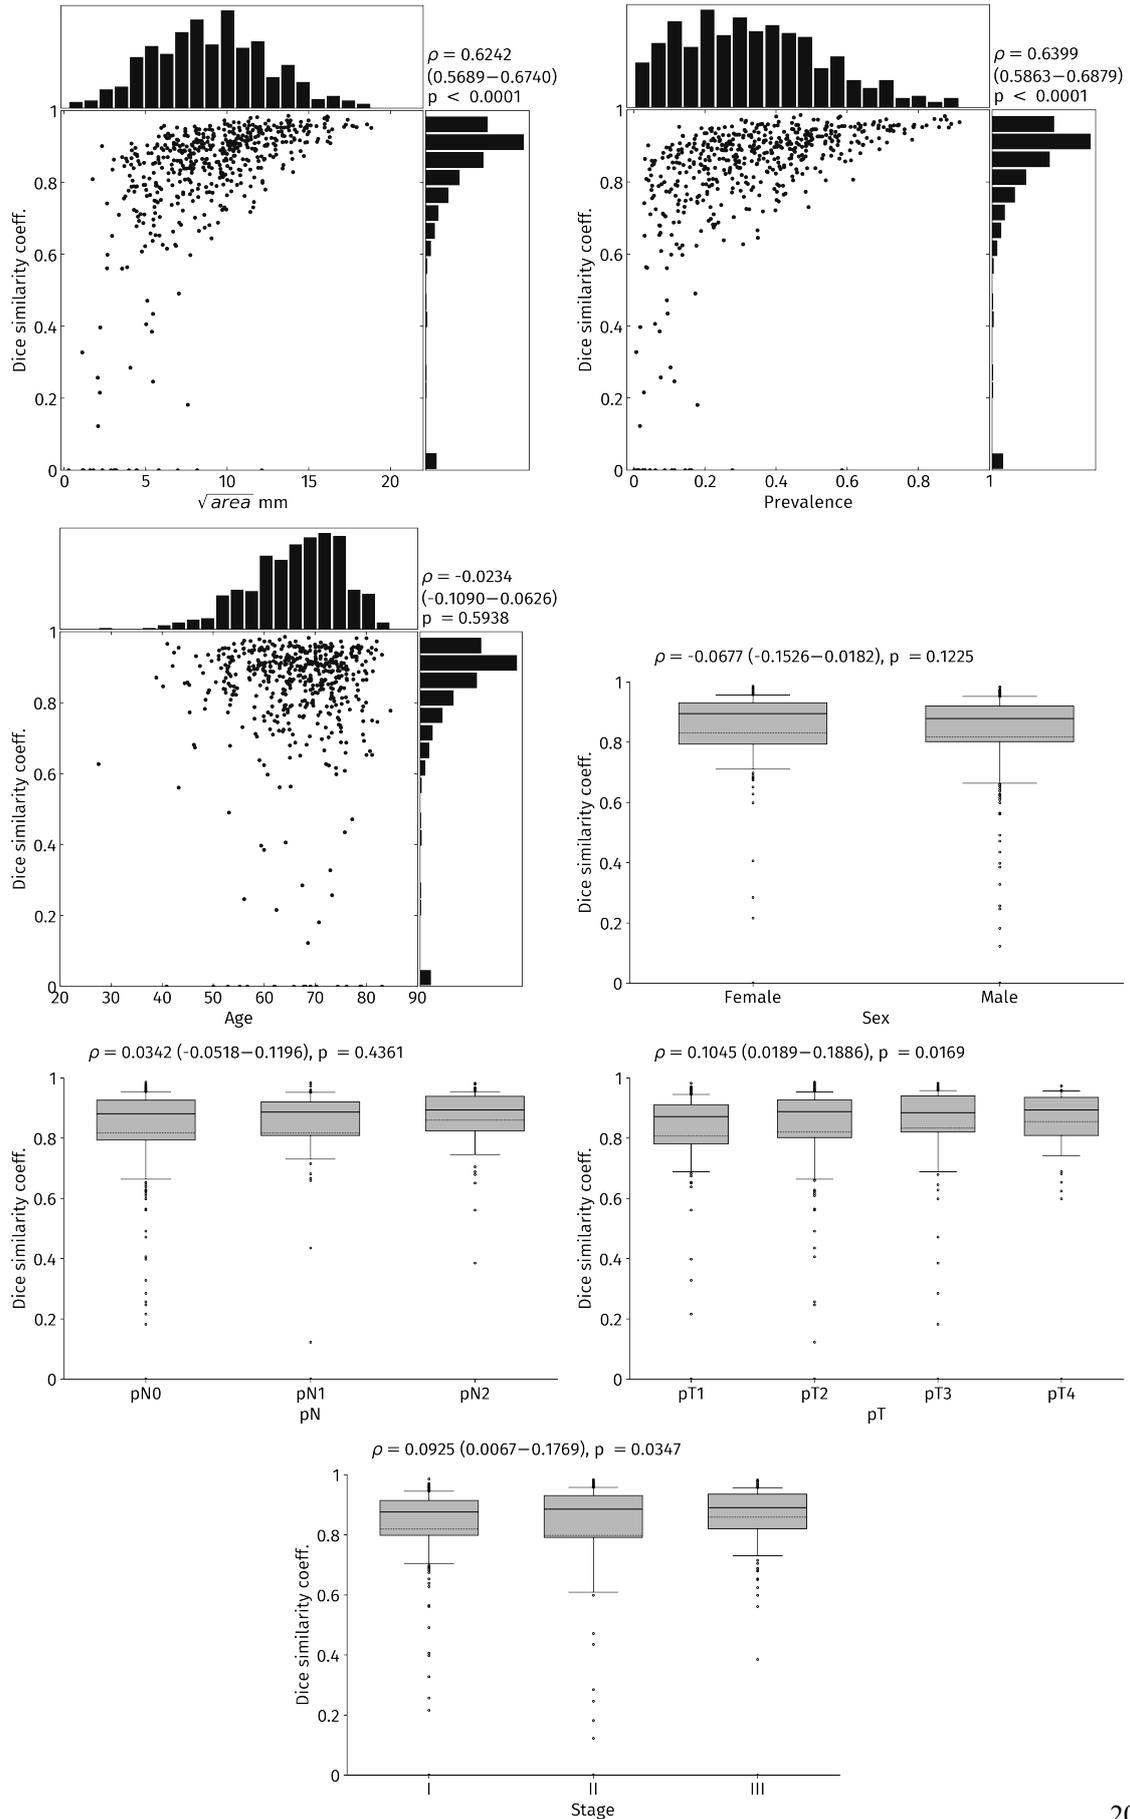

Figure S12: Associations of primary analysis result in VLu1

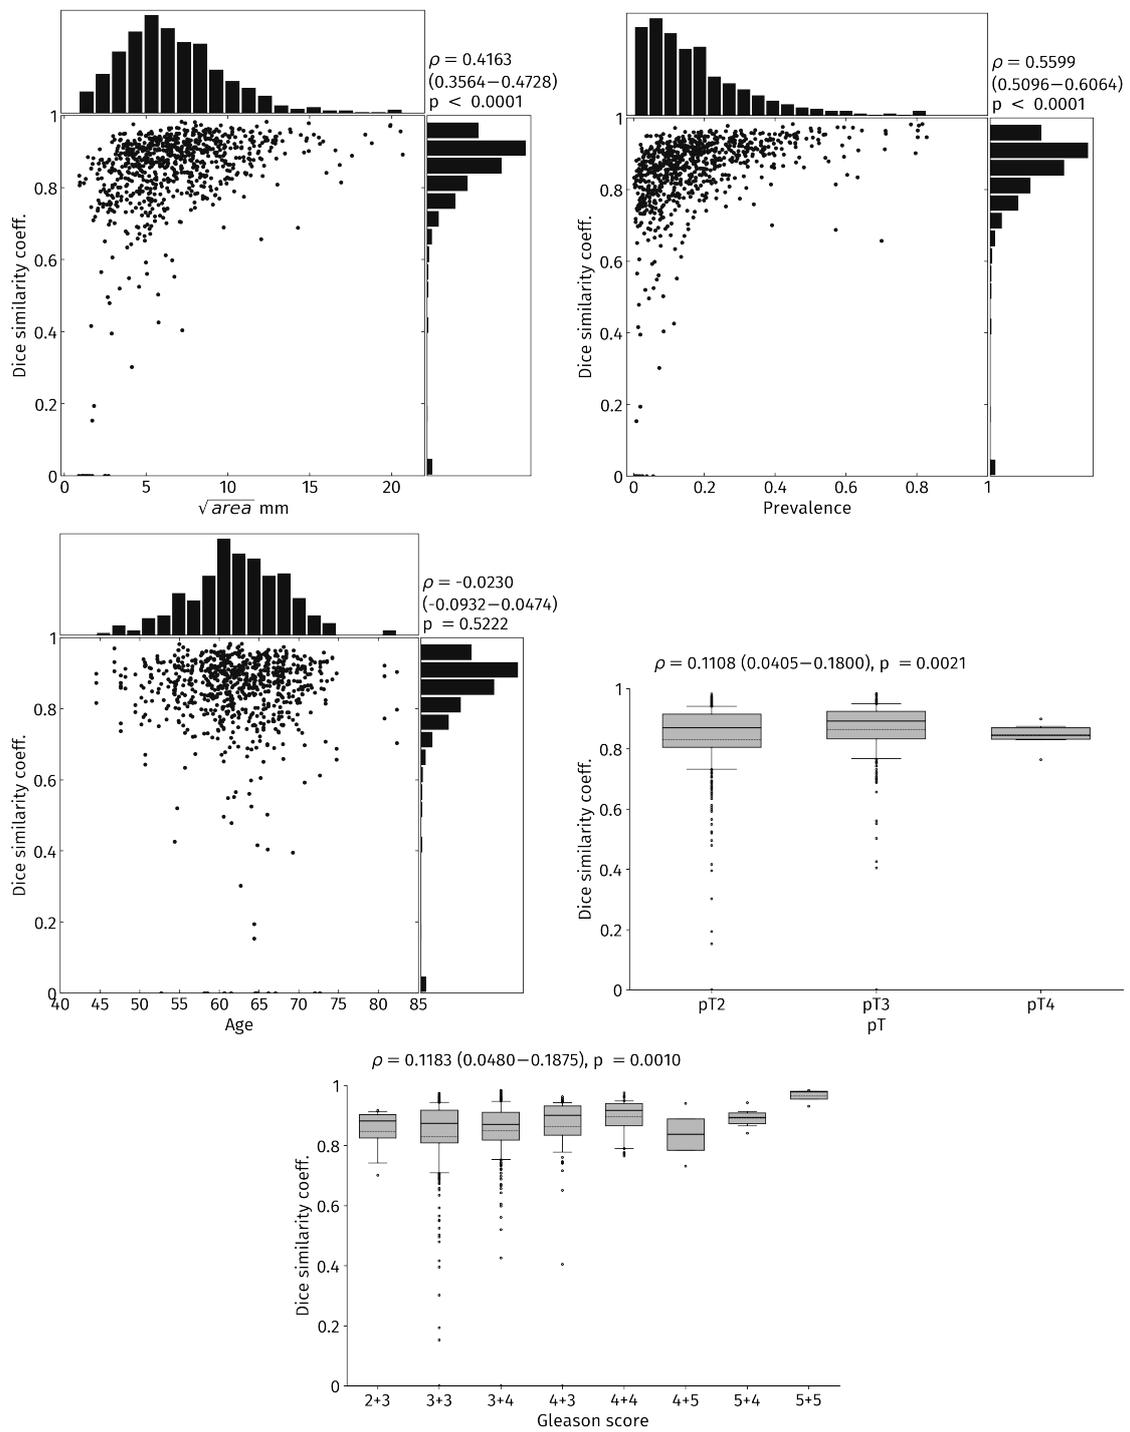

**Figure S13: Associations of primary analysis result in VPr1**

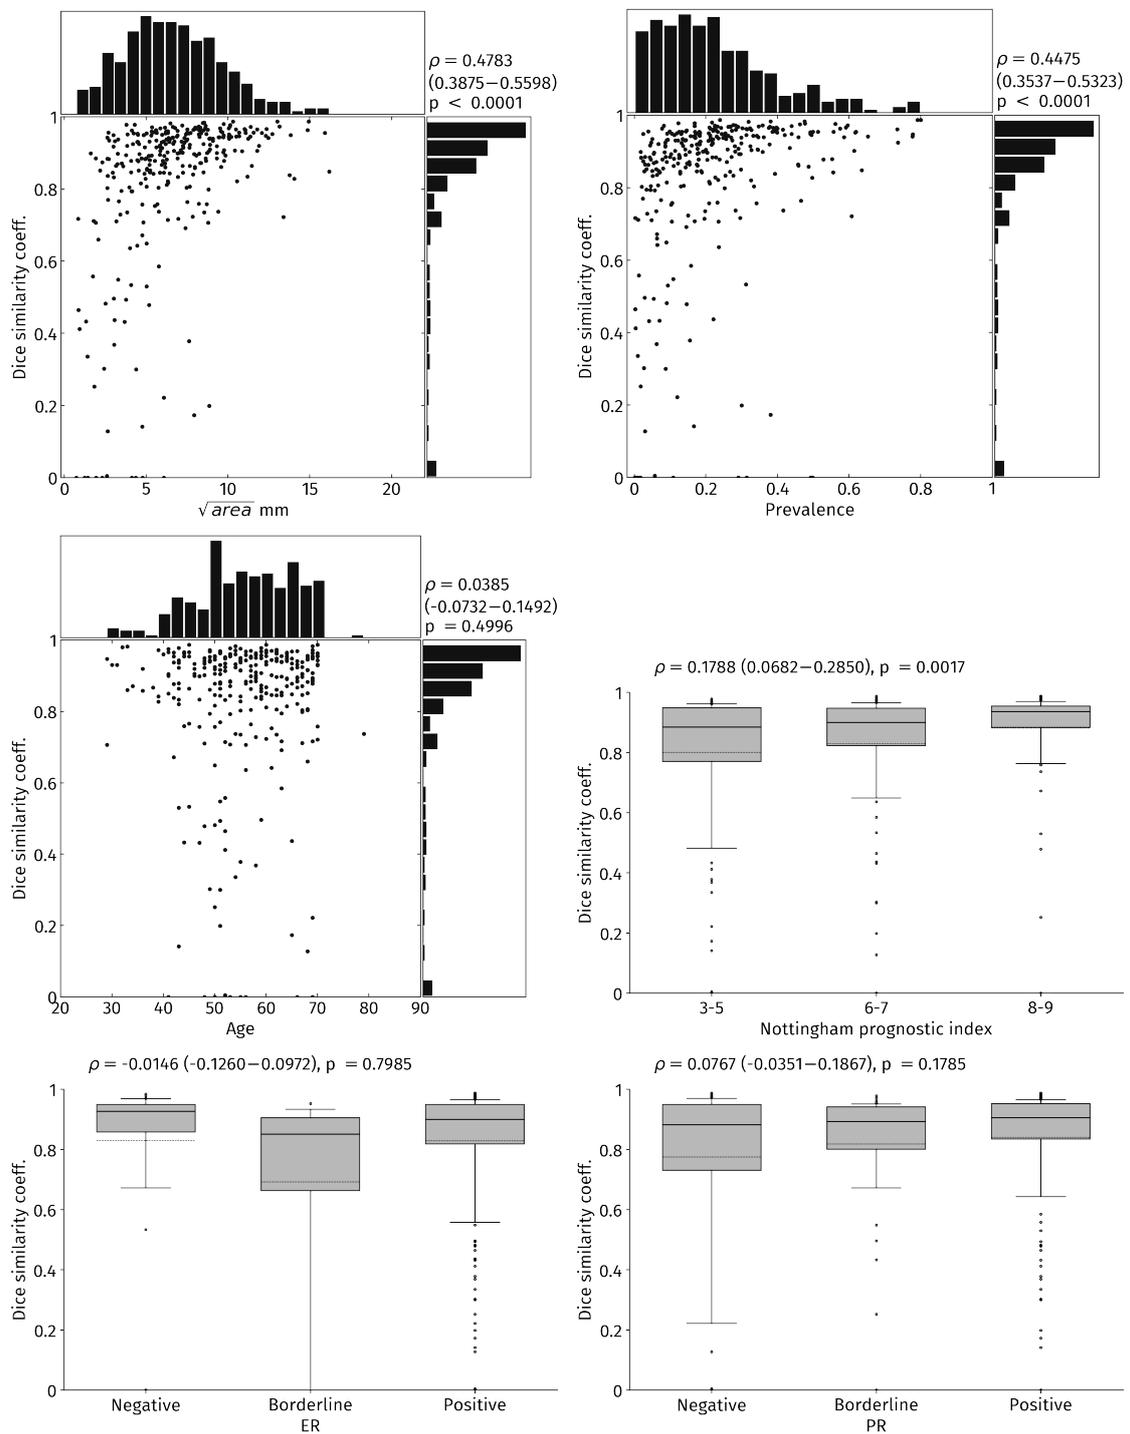

**Figure S14: Associations of primary analysis result in VBr1**

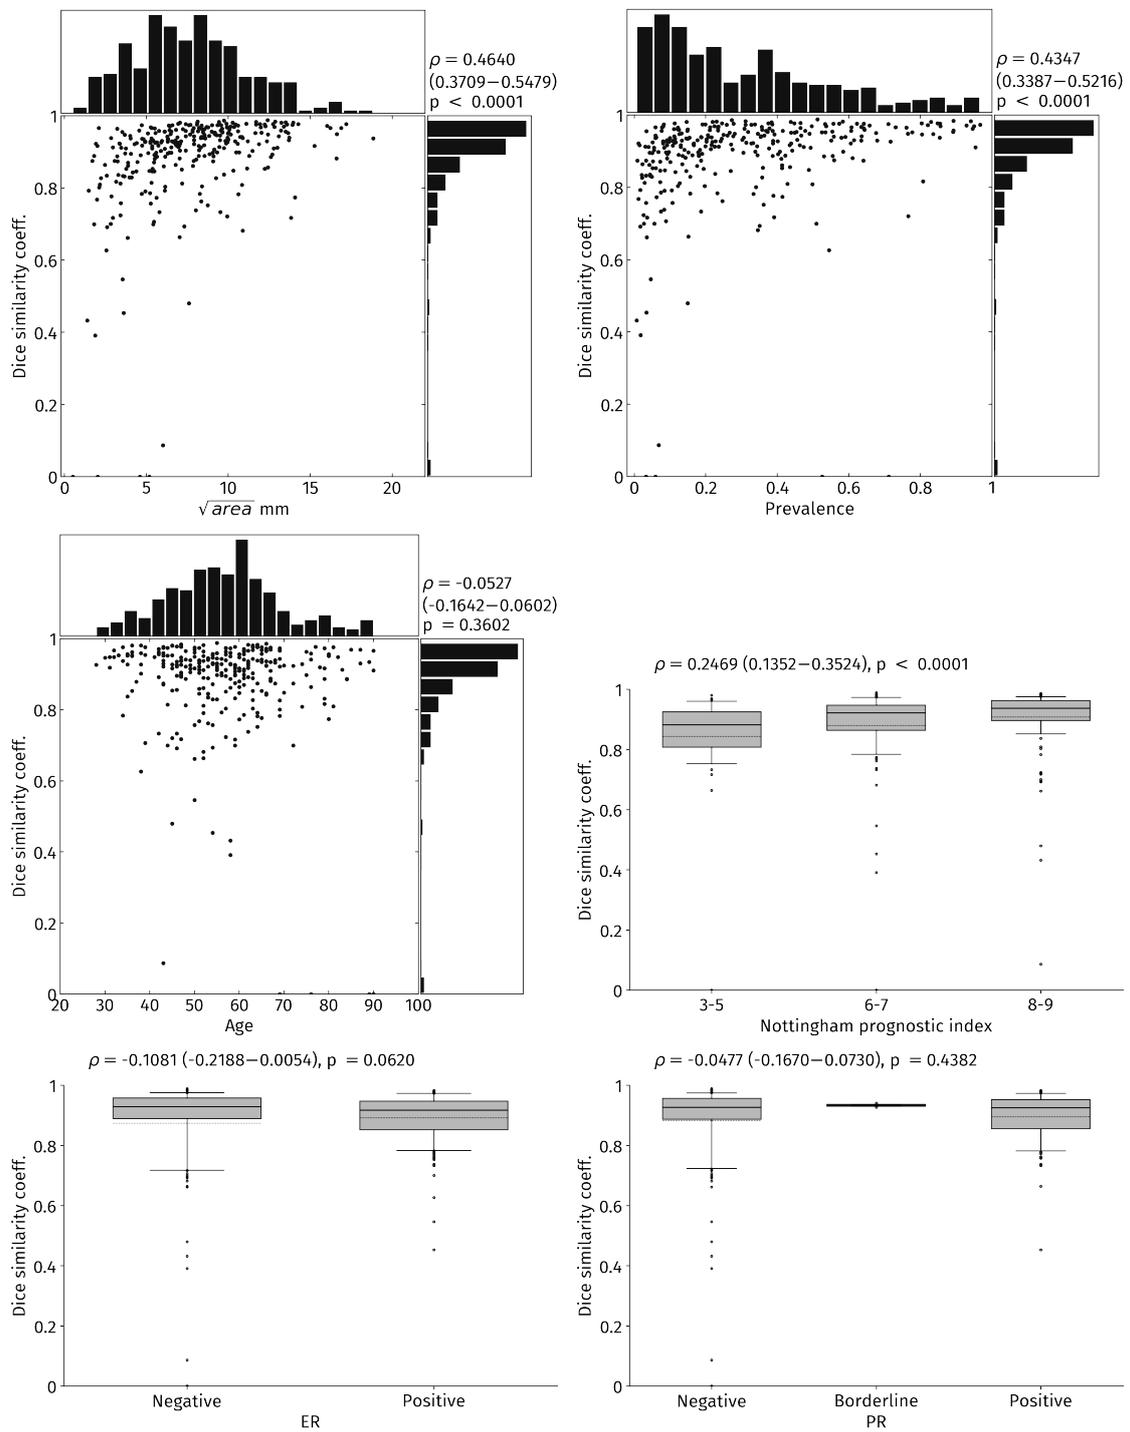

**Figure S15: Associations of primary analysis result in VBr2**

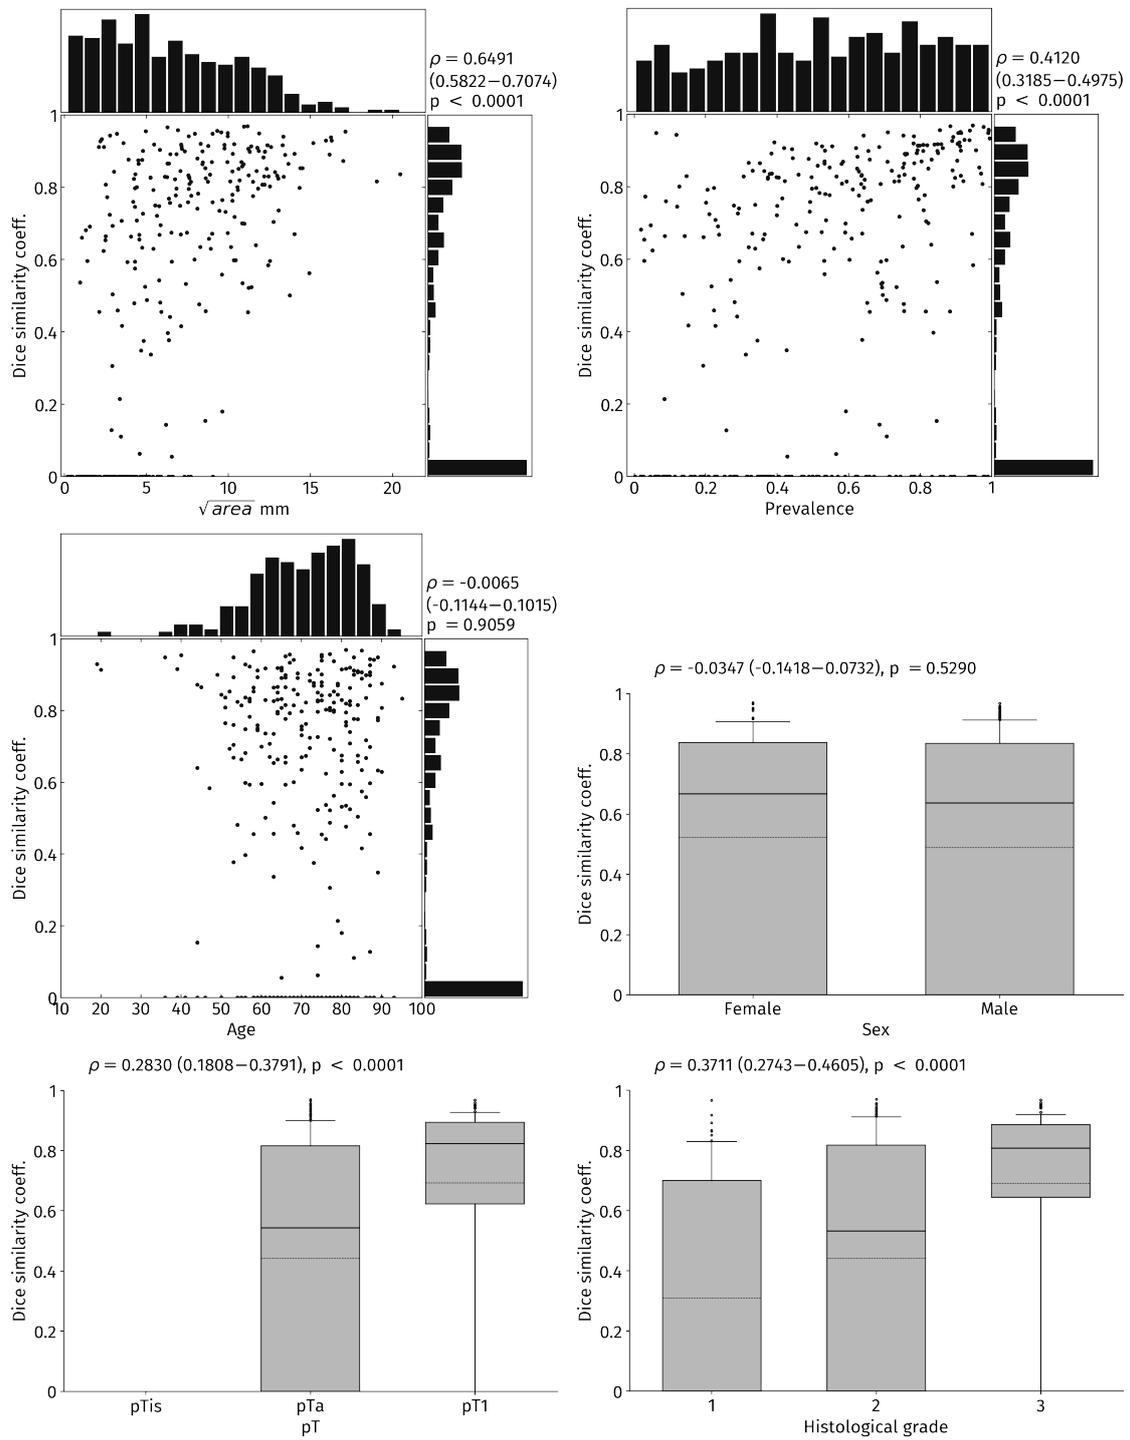

**Figure S16: Associations of primary analysis result in VUR1**

## 2.2 Per-scan comparison

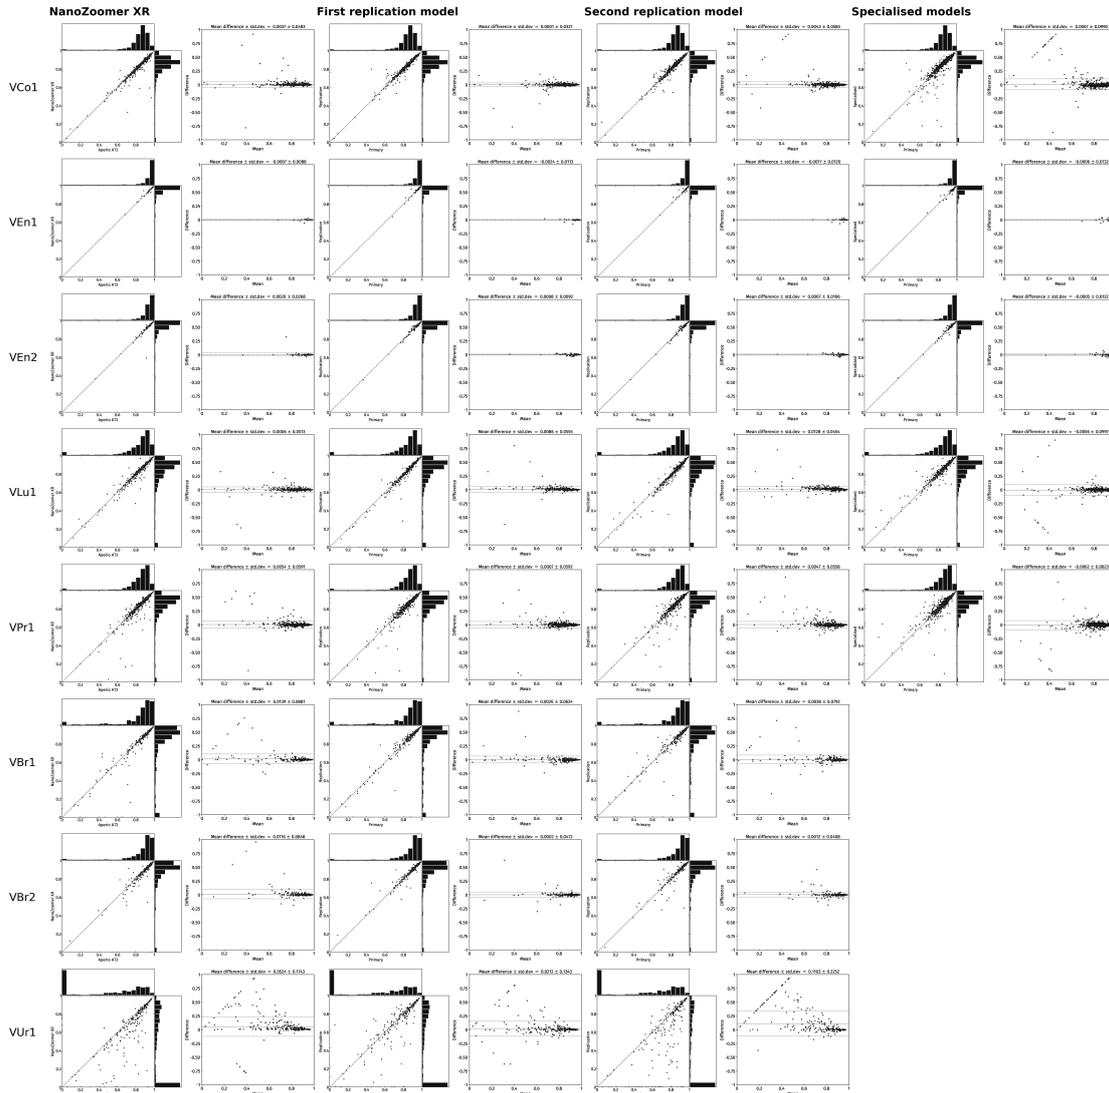

**Figure S17: Per scan comparison**

Per scan comparison viewed as a scatter plot (left) and mean difference plot (right) organised in columns for the primary model on Aperio AT2 vs the primary model on NanoZoomer XR, first replication model on Aperio AT2, second replication model on Aperio AT2, and the specialised models on Aperio AT2, respectively. Each scan result is the automatic vs manual segmentation measured with DSC.

### 2.3 Region areas

**Table S9: Performance in true positive regions**

Primary model evaluated on WSIs from Aperio AT2 in the validation cohorts

| Cohort | Images containing true positive regions<br>Count (proportion) | Dice similarity coefficient (%)<br>Mean (95% CI) |
|--------|---------------------------------------------------------------|--------------------------------------------------|
| VCo1   | 1058 (91.6%)                                                  | 86.10 (85.71 – 86.50)                            |
| VEn1   | 76 (98.7%)                                                    | 95.05 (93.82 – 96.27)                            |
| VEn2   | 150 (98.7%)                                                   | 93.18 (92.22 – 94.15)                            |
| VLu1   | 440 (84.3%)                                                   | 86.48 (85.75 – 87.22)                            |
| VPr1   | 731 (94.1%)                                                   | 87.76 (87.29 – 88.24)                            |
| VBr1   | 277 (89.4%)                                                   | 90.06 (89.26 – 90.86)                            |
| VBr2   | 295 (97.0%)                                                   | 90.71 (89.94 – 91.48)                            |
| VUr1   | 217 (65.4%)                                                   | 86.98 (86.09 – 87.87)                            |

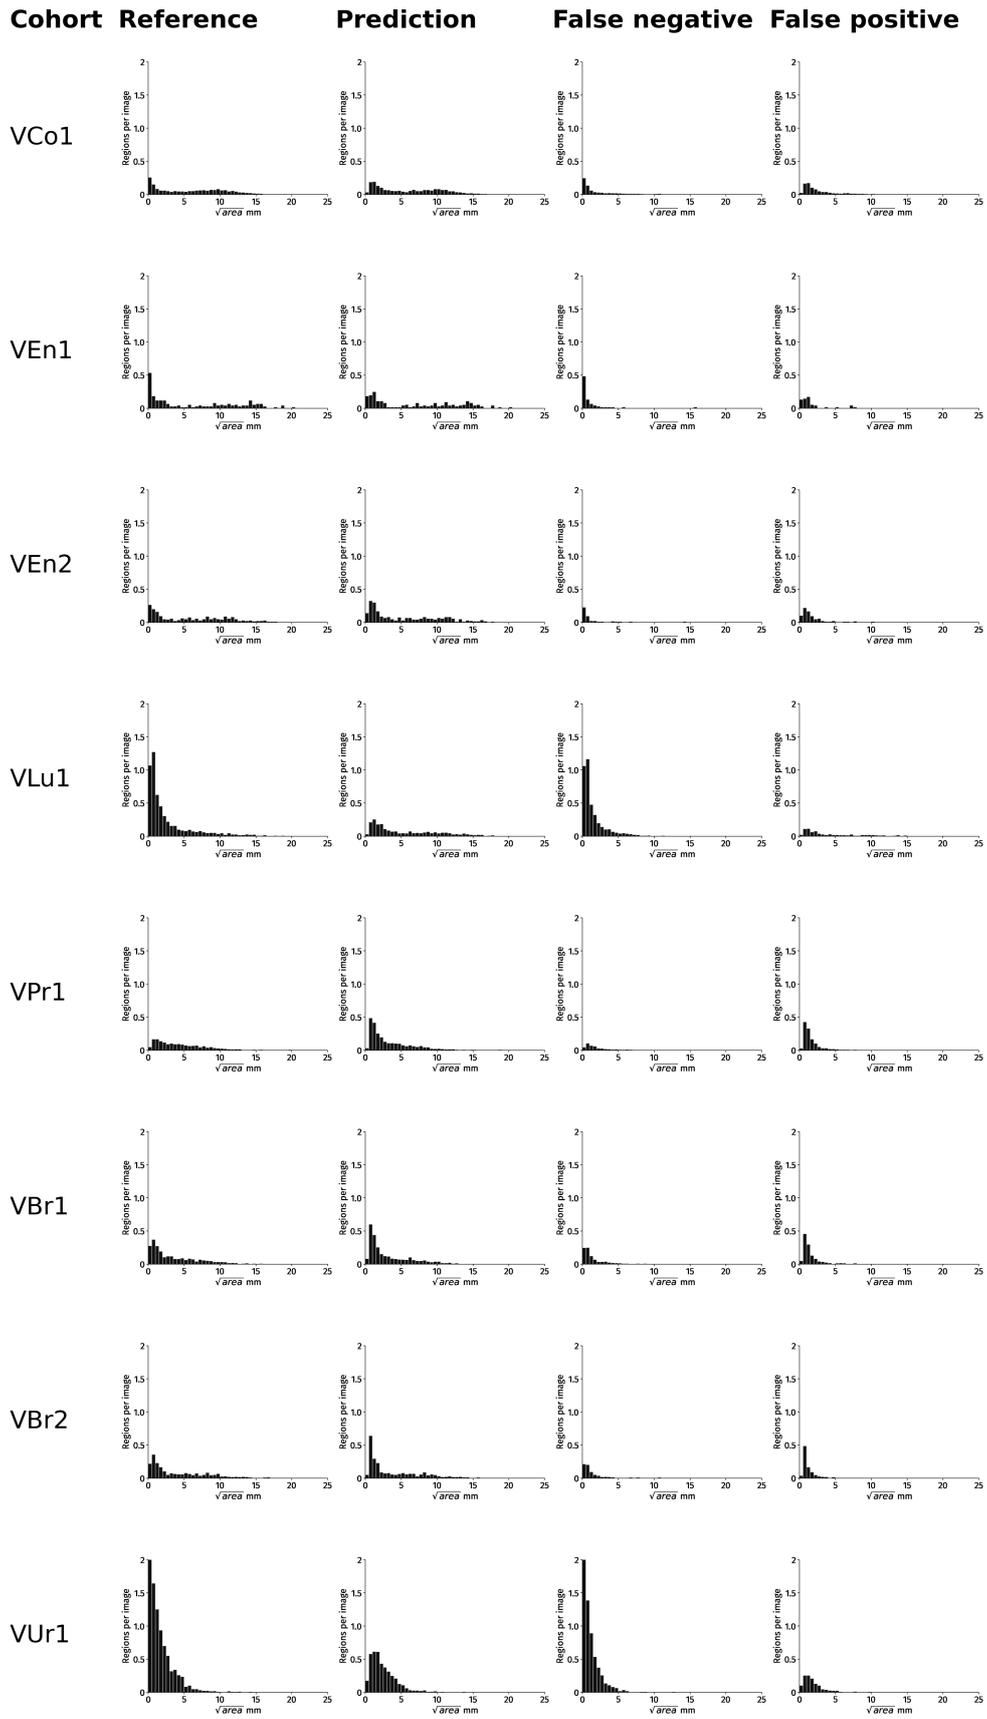

**Figure S18: Region areas in Aperio AT2 WSIs from the validation cohorts**  
 Reference regions are from the manual segmentation and predicted regions are from the automatic segmentation with the primary model.

**Table S10: Subgroup analyses in bladder cohorts**

| Cohort | Group             | All scans |                                                  | Scans with predictions |                                                  |
|--------|-------------------|-----------|--------------------------------------------------|------------------------|--------------------------------------------------|
|        |                   | Count     | Dice similarity coefficient (%)<br>Mean (95% CI) | Count                  | Dice similarity coefficient (%)<br>Mean (95% CI) |
| VUr1   | All scans         | 332       | 49.77 (45.64 – 53.90)                            | 224                    | 73.77 (71.16 – 76.39)                            |
|        | pT stage          |           |                                                  |                        |                                                  |
|        | pTa or pTis       | 256       | 43.99 (39.24 – 48.73)                            | 158                    | 71.27 (67.91 – 74.63)                            |
|        | pT1               | 76        | 69.27 (62.39 – 76.15)                            | 66                     | 79.76 (76.32 – 83.21)                            |
| BLCA   | All scans         | 431       | 84.49 (82.40 – 86.59)                            | 411                    | 88.61 (87.42 – 89.79)                            |
|        | pT stage          |           |                                                  |                        |                                                  |
|        | pT0               | 1         | 93.16                                            | 1                      | 93.16                                            |
|        | pT1               | 4         | 91.12 (80.31 – 01.93)                            | 4                      | 91.12 (80.31 – 01.93)                            |
|        | pT2               | 112       | 88.63 (85.86 – 91.39)                            | 110                    | 90.24 (88.60 – 91.87)                            |
|        | pT3               | 203       | 87.62 (85.21 – 90.04)                            | 199                    | 89.38 (87.66 – 91.11)                            |
|        | pT4               | 58        | 87.49 (81.89 – 93.08)                            | 56                     | 90.61 (87.01 – 94.21)                            |
|        | pTx               | 1         | 79.90                                            | 1                      | 79.90                                            |
|        | Missing           | 52        | 59.45 (49.74 – 69.17)                            | 40                     | 77.29 (73.04 – 81.55)                            |
|        | Fragmented tissue |           |                                                  |                        |                                                  |
|        | True              | 87        | 66.38 (59.91 – 72.86)                            | 75                     | 77.01 (73.41 – 80.60)                            |
|        | False             | 342       | 89.05 (87.27 – 90.84)                            | 334                    | 91.19 (90.15 – 92.22)                            |
|        | Missing           | 2         | 92.78 (87.98 – 97.58)                            | 2                      | 92.78 (87.98 – 97.58)                            |

## 2.4 Intra- and inter-observer variability

**Table S11: Intra- and inter-observer variability in VBr2**

*MP-1*: annotations by Manohar Pradhan in the first round. *MP-2*: annotations by Manohar Pradhan in the second round. *LV*: annotations by Ljiljana Vlatkovic. *Auto*: annotations by the primary automatic segmentation model presented in this study.

| Comparison   | Dice similarity coefficient (%) |                       |
|--------------|---------------------------------|-----------------------|
|              | Mean (95% CI)                   | Median (IQR)          |
| MP-2 vs MP-1 | 91.37 (90.20 – 92.54)           | 93.96 (90.19 – 96.85) |
| LV vs MP-1   | 74.25 (71.94 – 76.57)           | 79.55 (65.33 – 90.16) |
| Auto vs MP-1 | 88.16 (86.52 – 89.80)           | 92.45 (86.41 – 95.64) |
| LV vs MP-2   | 76.69 (74.39 – 78.99)           | 82.82 (67.94 – 91.40) |
| Auto vs MP-2 | 87.78 (86.05 – 89.51)           | 92.16 (86.37 – 95.54) |
| Auto vs LV   | 72.06 (69.63 – 74.48)           | 77.91 (62.76 – 88.36) |

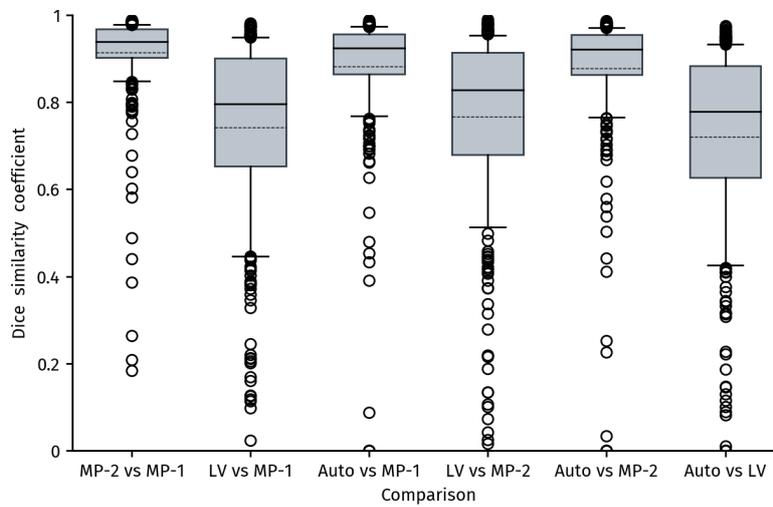

**Figure S19: Intra- and inter-observer variability in VBr2**

For each two observers that are compared, the plot summarises the Dice similarity coefficient with interquartile range (coloured box), mean value (perforated horizontal line), median value (solid horizontal line), the 10th and 90th percentile (whiskers), and outliers (circles). See Table S11 for label explanations.

## 2.5 Performance evaluation in five different scanners

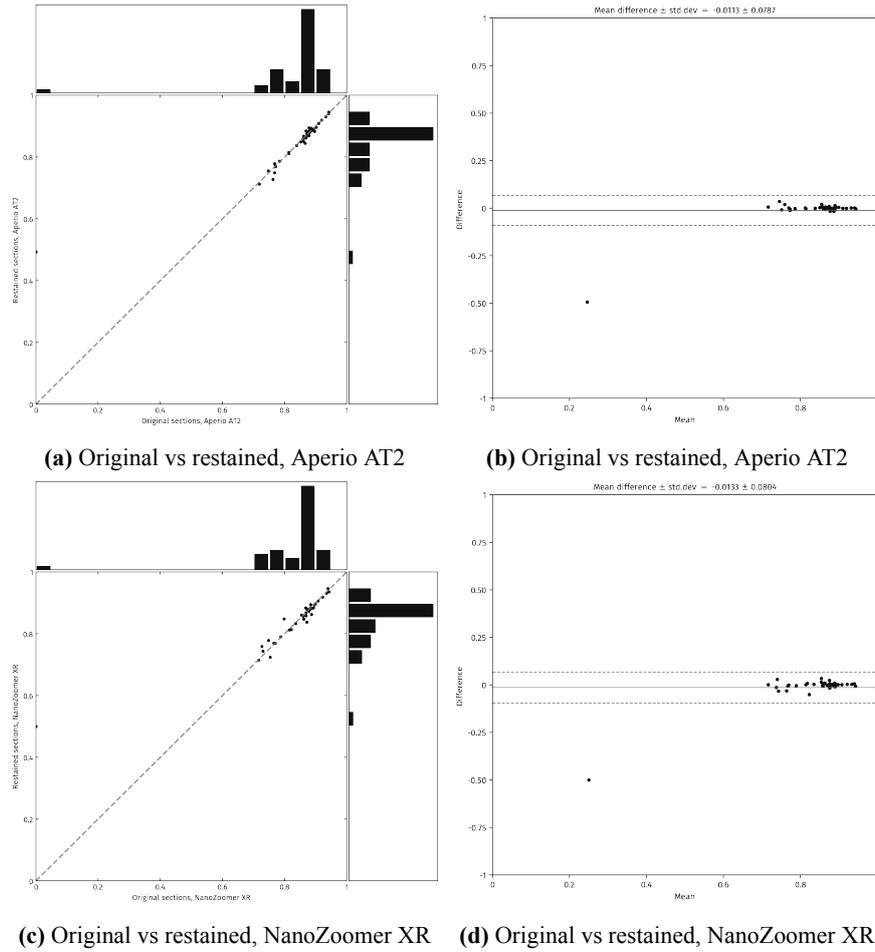

**Figure S20: Original vs retained mean difference**

Dice similarity coefficient of 39 tissue sections that were retained.

**Table S12: Primary model performance in VCo1 scanned on five different scanners**

Only slides that were successfully scanned on all five scanners were included

| Scanner          | Scans | Dice similarity coefficient (%)<br>Mean (95% CI) |
|------------------|-------|--------------------------------------------------|
| Aperio AT2       | 1 152 | 84.58 (83.90 – 85.26)                            |
| Aperio GT 450 DX | 1 152 | 82.85 (81.91 – 83.80)                            |
| KF-PRO-400       | 1 152 | 84.13 (83.36 – 84.90)                            |
| NanoZoomer XR    | 1 152 | 84.21 (83.51 – 84.92)                            |
| Pannoramic 1000  | 1 152 | 83.35 (82.51 – 84.18)                            |

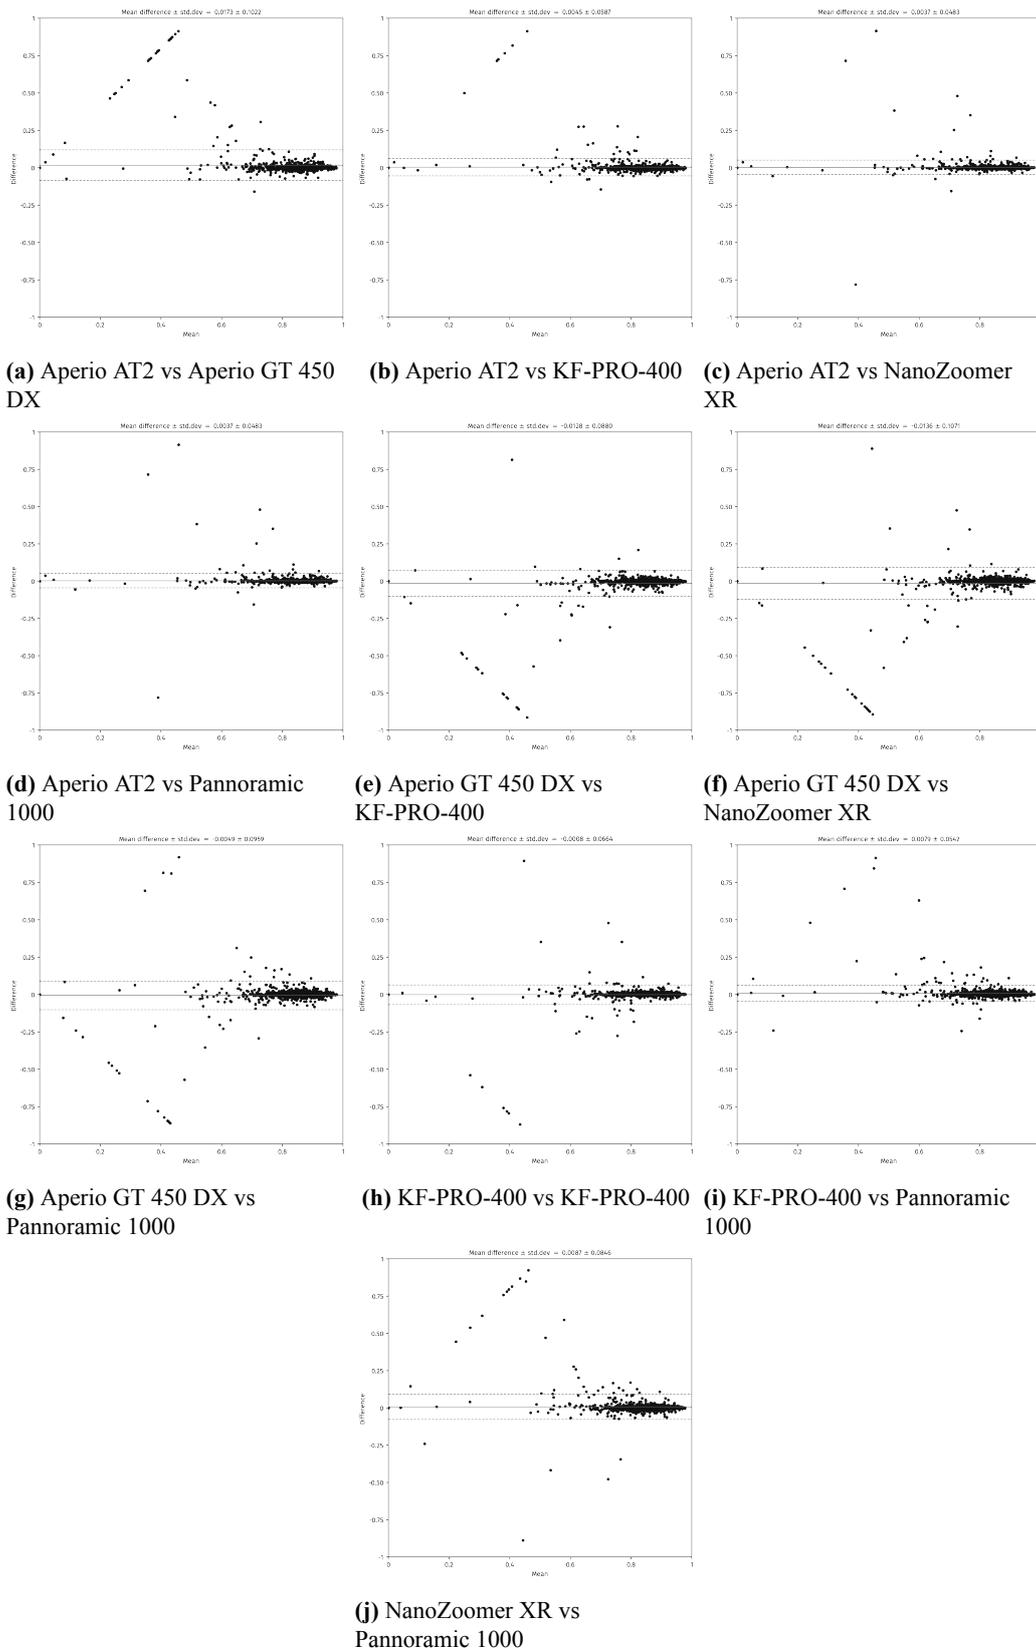

**Figure S21: Scanner vs scanner mean difference**

Dice similarity coefficient of 1 152 glass slides from VCo1 scanned with five different scanners. Each plot compares results from one scanner vs another, and the difference is computed as the Dice similarity coefficient of the scanner mentioned first minus the scanner mentioned last.

## 2.6 Comparison with MedSAM

**Table S13: MedSAM performance in validation datasets**

Dice similarity coefficient percent mean (95% CI) versus manual segmentation.

| Cohort | Method        | Aperio AT2            | NanoZoomer XR         |
|--------|---------------|-----------------------|-----------------------|
| VCo1   | Primary       | 84.54 (83.86 – 85.23) | 84.17 (83.46 – 84.88) |
|        | MedSAM-tumour | 79.38 (78.69 – 80.07) | 79.43 (78.72 – 80.13) |
|        | MedSAM-tissue | 48.23 (47.13 – 49.33) | 48.78 (47.72 – 49.84) |
|        | Tumour-bbox   | 73.78 (73.11 – 74.45) | 73.71 (73.03 – 74.39) |
| VEn1   | Primary       | 95.28 (94.20 – 96.36) | 95.35 (94.30 – 96.40) |
|        | MedSAM-tumour | 88.95 (86.34 – 91.56) | 89.75 (87.20 – 92.30) |
|        | MedSAM-tissue | 62.51 (57.25 – 67.76) | 61.50 (55.95 – 67.06) |
|        | Tumour-bbox   | 82.35 (79.39 – 85.31) | 82.29 (79.33 – 85.26) |
| VEn2   | Primary       | 93.40 (92.31 – 94.49) | 93.20 (92.03 – 94.37) |
|        | MedSAM-tumour | 86.56 (85.10 – 88.02) | 86.57 (85.14 – 87.99) |
|        | MedSAM-tissue | 53.12 (49.51 – 56.72) | 52.69 (49.04 – 56.35) |
|        | Tumour-bbox   | 78.49 (76.68 – 80.30) | 78.48 (76.67 – 80.28) |
| VLu1   | Primary       | 82.22 (80.54 – 83.91) | 82.16 (80.50 – 83.82) |
|        | MedSAM-tumour | 72.23 (70.75 – 73.71) | 72.32 (70.84 – 73.81) |
|        | MedSAM-tissue | 46.55 (44.57 – 48.52) | 46.79 (44.84 – 48.73) |
|        | Tumour-bbox   | 66.69 (65.28 – 68.11) | 66.64 (65.22 – 68.05) |
| VPr1   | Primary       | 84.36 (83.33 – 85.38) | 83.82 (82.72 – 84.92) |
|        | MedSAM-tumour | 65.77 (64.19 – 67.36) | 65.75 (64.17 – 67.34) |
|        | MedSAM-tissue | 27.78 (26.41 – 29.15) | 27.70 (26.36 – 29.05) |
|        | Tumour-bbox   | 60.09 (58.68 – 61.51) | 60.05 (58.63 – 61.47) |
| VBr1   | Primary       | 82.40 (79.94 – 84.86) | 81.01 (78.28 – 83.73) |
|        | MedSAM-tumour | 81.36 (79.49 – 83.22) | 81.16 (79.28 – 83.05) |
|        | MedSAM-tissue | 34.40 (32.08 – 36.72) | 36.19 (33.86 – 38.52) |
|        | Tumour-bbox   | 70.48 (68.70 – 72.26) | 71.29 (69.56 – 73.03) |
| VBr2   | Primary       | 88.16 (86.52 – 89.80) | 87.00 (85.07 – 88.92) |
|        | MedSAM-tumour | 82.54 (80.55 – 84.53) | 82.79 (80.84 – 84.75) |
|        | MedSAM-tissue | 42.49 (39.50 – 45.48) | 44.60 (41.66 – 47.55) |
|        | Tumour-bbox   | 72.93 (71.04 – 74.81) | 73.92 (72.09 – 75.75) |
| VUr1   | Primary       | 49.77 (45.64 – 53.90) | 44.53 (40.48 – 48.58) |
|        | MedSAM-tumour | 74.53 (72.27 – 76.78) | 74.28 (72.01 – 76.55) |
|        | MedSAM-tissue | 64.63 (61.77 – 67.49) | 64.58 (61.73 – 67.42) |
|        | Tumour-bbox   | 74.45 (72.28 – 76.62) | 74.45 (72.27 – 76.63) |

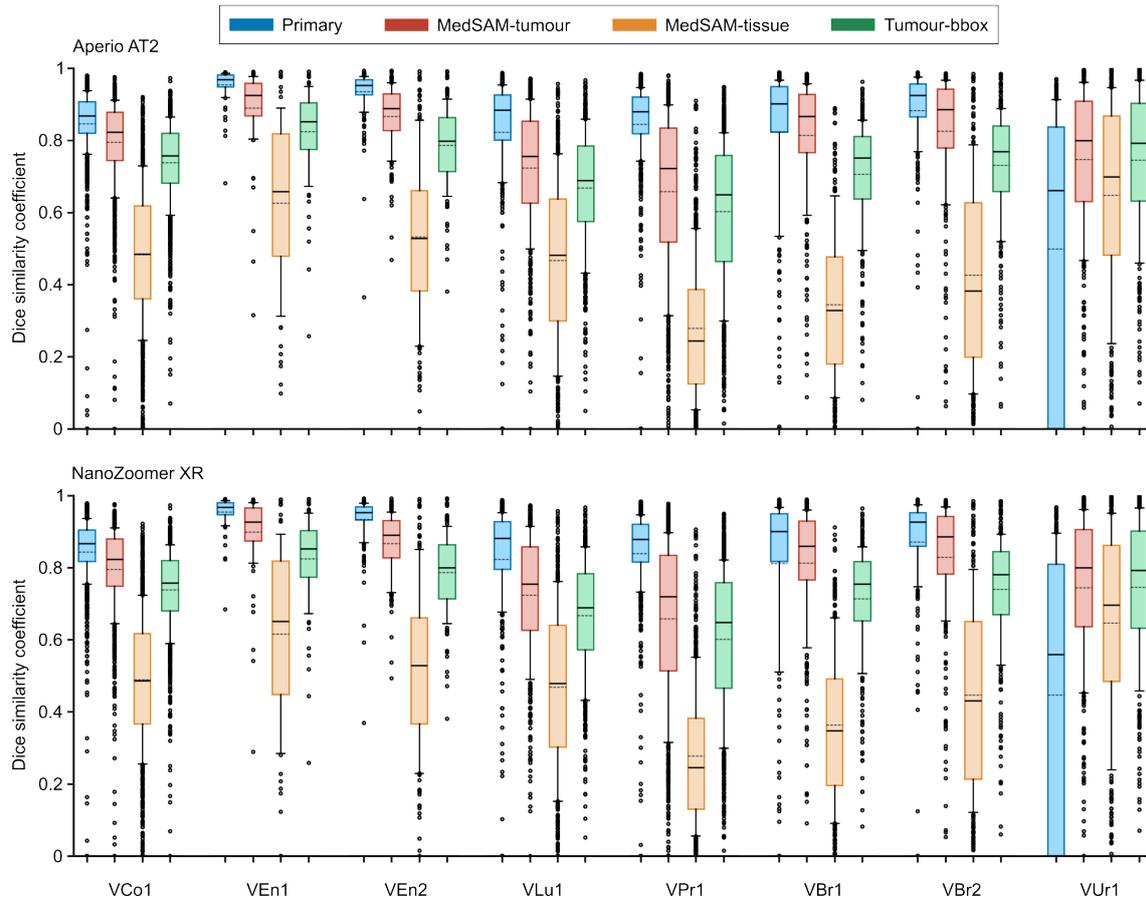

**Figure S22: MedSAM performance in validation datasets**

Segmentation performance in validation cohorts from Aperio AT2 (top) and NanoZoomer XR (bottom). Evaluated methods are MedSAM prompted by tumour bounding box (MedSAM-tumour), MedSAM prompted by tissue bounding box (MedSAM-tissue) and bounding boxes of manual annotations (Tumour-bbox). The result of the primary method presented in this study is included for reference (Primary). Summary statistics are given in Supplementary Table S13.

### 3 Segmentation network optimisation

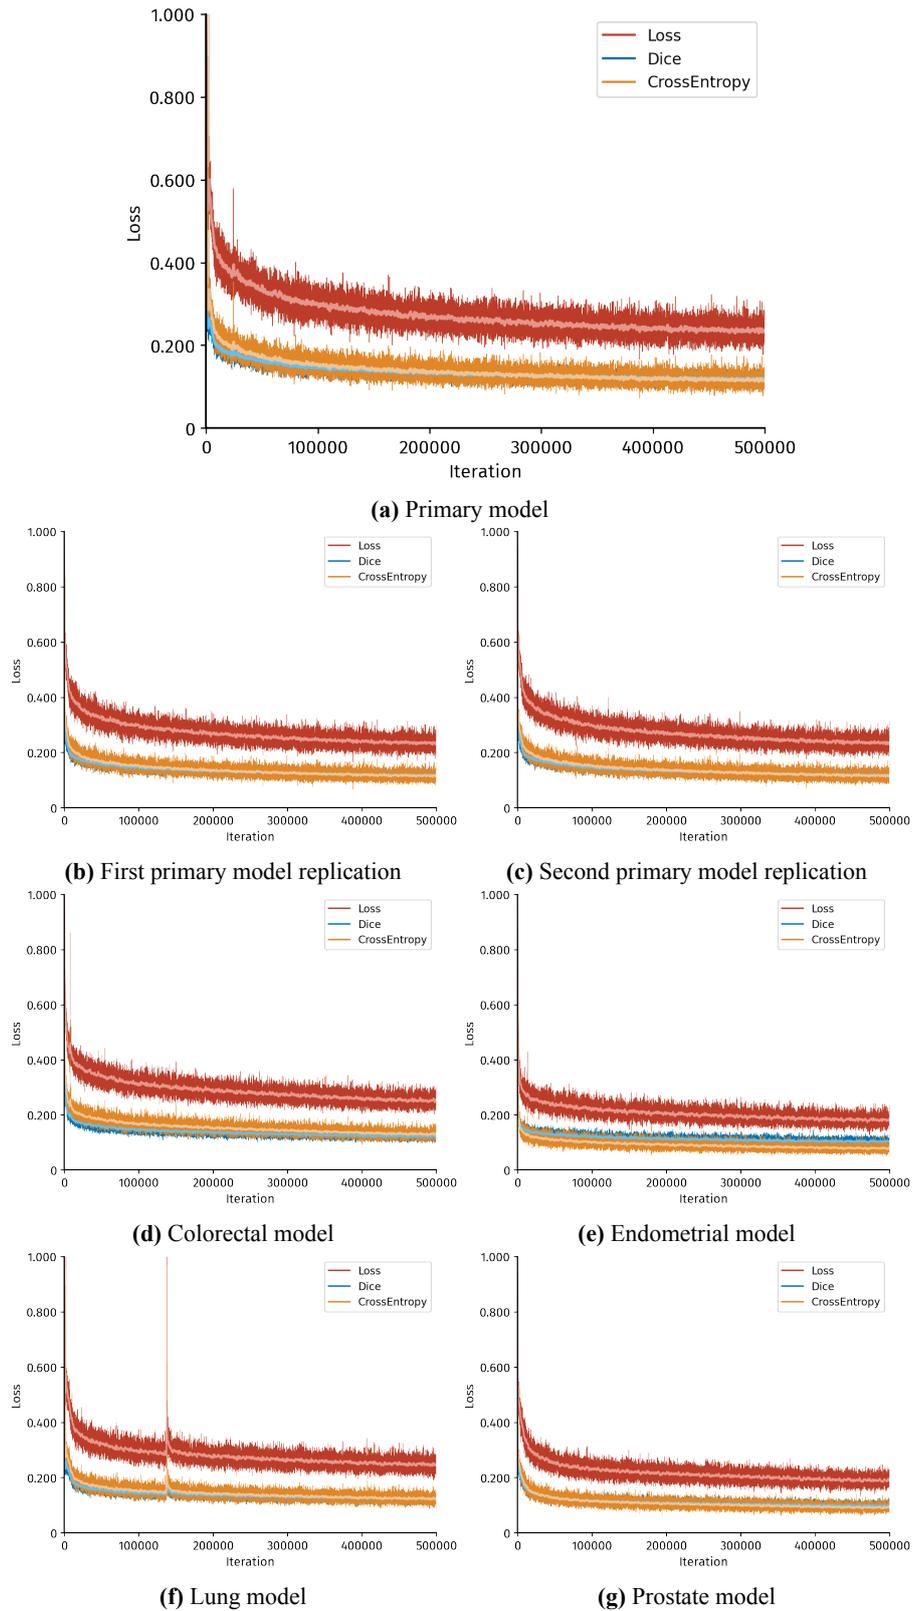

**Figure S23: Segmentation network optimisation loss curve**  
*Loss* is the sum of *Dice* loss and *CrossEntropy* loss. Values are averaged over 20 iterations.

## 4 TCGA cohorts

33 TCGA cohorts were downloaded from <https://www.cancer.gov/tcga> in December 2021. Only scans from so-called *diagnostic slides* were considered. LAML did not have diagnostic slides leaving the 32 cohorts. We only made use of BLCA, LUAD, LUSC and PRAD since these were the only one we had manually annotated at the time of conducting the study.

Since we segment the scans at resolution 1  $\mu\text{m}$  per pixel, we exclude all scans where the scan resolution information is not present. We note that for some scans there are an apparent disagreement between the magnification information present in the `PROPERTY_NAME_MPP_X` and `PROPERTY_NAME_MPP_Y` properties and the information from the `PROPERTY_NAME_OBJECTIVE_POWER` property (objective power at the lowest scan level, normally around 0.25  $\mu\text{m}$  per pixel for objective power 40). This might indicate that the actual scan resolution is different from what it is stated, but we use the magnification in the `PROPERTY_NAME_MPP_*` properties, and do not exclude any scans based on this apparent discrepancy.

We do not exclude any scans based on their appearance or quality, although we find scans with attributes such as pen markings, air bubbles, dust, tissue out of focus, different stain than H&E, etc.

All scans are stored in the `.svs` format and the openslide property `PROPERTY_NAME_VENDOR` for all scans is equal to Aperio. Based on visual appearance, we find it unlikely that all scans are in fact originally scanned with Aperio, but have not excluded any scans based on this.

Clinical data presented in Table S14 and Fig. S28 are from the TCGA Pan-Cancer Clinical Data Resource which publication should be consulted when interpreting the included variables and their values.<sup>1</sup>

### 4.1 Included scans

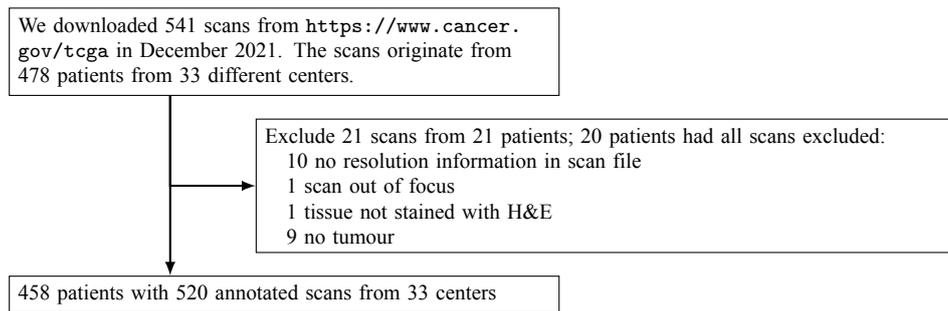

**Figure S24: Flow from downloaded scans to annotated scans for the LUAD cohort**

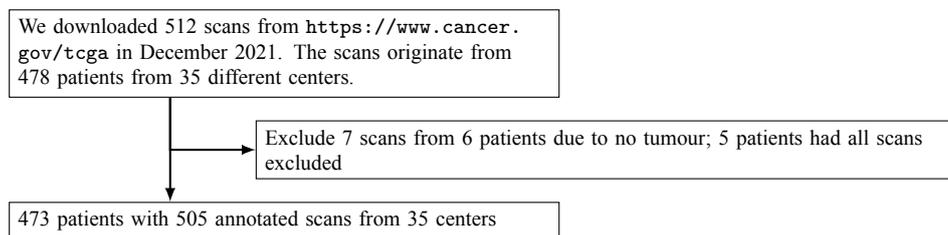

**Figure S25: Flow from downloaded scans to annotated scans for the LUSC cohort**

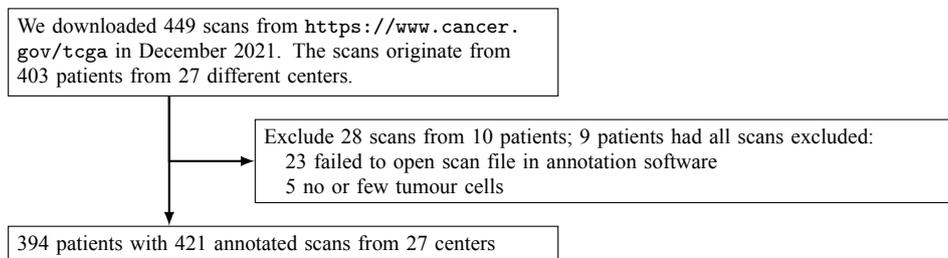

**Figure S26: Flow from downloaded scans to annotated scans for the PRAD cohort**

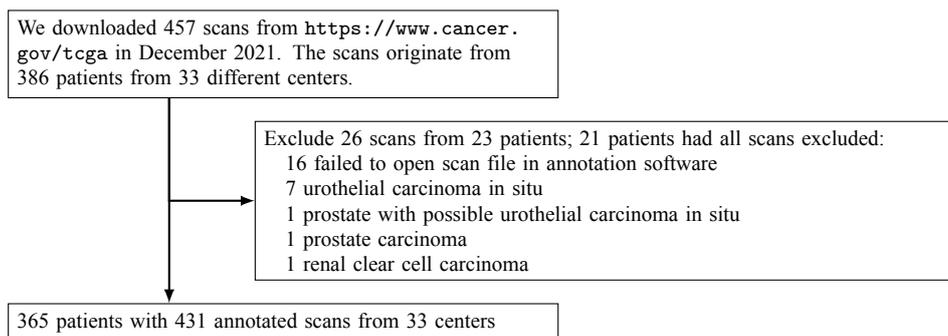

**Figure S27: Flow from downloaded scans to annotated scans for the BLCA cohort**

## 4.2 Baseline characteristics

**Table S14: Baseline characteristics for included TCGA cohorts**

Data are given as *median (interquartile range)* or *count (percentage)*. Time to *event* statistics are based only on patients with the respective event.

|                               | BLCA            | LUAD            | LUSC            | PRAD            |
|-------------------------------|-----------------|-----------------|-----------------|-----------------|
| Patient count                 | 365             | 458             | 473             | 394             |
| Age at diagnosis              |                 |                 |                 |                 |
| Years                         | 69 (60 – 76)    | 66 (59 – 73)    | 68 (62 – 74)    | 61 (56 – 66)    |
| Missing                       | 0               | 18 (4%)         | 9 (2%)          | 0               |
| Sex                           |                 |                 |                 |                 |
| Female                        | 91 (25%)        | 248 (54%)       | 119 (25%)       | 0               |
| Male                          | 274 (75%)       | 210 (46%)       | 354 (75%)       | 394 (100%)      |
| Cancer-specific death         |                 |                 |                 |                 |
| False                         | 242 (66%)       | 325 (71%)       | 341 (72%)       | 387 (98%)       |
| True                          | 110 (30%)       | 100 (22%)       | 83 (18%)        | 5 (1%)          |
| Missing                       | 13 (4%)         | 33 (7%)         | 49 (10%)        | 2 (1%)          |
| Time to cancer-specific death |                 |                 |                 |                 |
| Years                         | 1.1 (0.6 – 1.7) | 1.7 (0.9 – 2.7) | 1.7 (1.0 – 2.9) | 3.6 (2.2 – 5.1) |
| Missing                       | 1 (1%)          | 2 (2%)          | 2 (2%)          | 0               |
| Overall death                 |                 |                 |                 |                 |
| False                         | 202 (55%)       | 298 (65%)       | 271 (57%)       | 385 (98%)       |
| True                          | 163 (45%)       | 160 (35%)       | 202 (43%)       | 9 (2%)          |
| Time to overall death         |                 |                 |                 |                 |
| Years                         | 1.1 (0.6 – 1.7) | 1.7 (0.8 – 2.9) | 1.5 (0.8 – 3.1) | 3.6 (2.0 – 6.8) |
| Missing                       | 1 (1%)          | 3 (2%)          | 4 (2%)          | 0               |
| New tumour event              |                 |                 |                 |                 |
| False                         | 209 (57%)       | 272 (59%)       | 336 (71%)       | 322 (82%)       |
| True                          | 156 (43%)       | 186 (41%)       | 137 (29%)       | 72 (18%)        |
| Time to new tumour event      |                 |                 |                 |                 |
| Years                         | 0.8 (0.5 – 1.5) | 1.2 (0.7 – 1.9) | 1.2 (0.7 – 2.2) | 1.8 (0.9 – 3.0) |
| Missing                       | 0               | 2 (1%)          | 1 (1%)          | 0               |
| Follow-up time                |                 |                 |                 |                 |
| Years                         | 1.4 (0.9 – 2.5) | 1.8 (1.2 – 3.1) | 1.8 (0.9 – 3.5) | 2.8 (1.8 – 4.6) |
| Missing                       | 1 (<1%)         | 8 (2%)          | 6 (1%)          | 0               |
| pN stage                      |                 |                 |                 |                 |
| pN0                           | 207 (57%)       | 301 (66%)       | 302 (64%)       | 276 (70%)       |
| pN1                           | 40 (11%)        | 89 (19%)        | 125 (26%)       | 54 (14%)        |
| pN2                           | 71 (19%)        | 55 (12%)        | 36 (8%)         | 0               |
| pN3                           | 7 (2%)          | 2 (<1%)         | 5 (1%)          | 0               |
| pNx                           | 34 (9%)         | 10 (2%)         | 5 (1%)          | 0               |
| Missing                       | 6 (2%)          | 1 (<1%)         | 0               | 64 (16%)        |
| pT stage                      |                 |                 |                 |                 |
| pT0                           | 1 (<1%)         | 0               | 0               | 0               |
| pT1                           | 3 (1%)          | 157 (34%)       | 108 (23%)       | 0               |
| pT2                           | 108 (30%)       | 241 (53%)       | 280 (59%)       | 153 (39%)       |
| pT3                           | 174 (48%)       | 41 (9%)         | 64 (14%)        | 227 (58%)       |
| pT4                           | 51 (14%)        | 16 (3%)         | 21 (4%)         | 8 (2%)          |
| pTx                           | 1 (<1%)         | 3 (1%)          | 0               | 0               |
| Missing                       | 27 (7%)         | 0               | 0               | 6 (2%)          |
| Stage                         |                 |                 |                 |                 |
| I                             | 2 (1%)          | 250 (55%)       | 234 (49%)       | 0               |
| II                            | 115 (32%)       | 113 (25%)       | 152 (32%)       | 0               |
| III                           | 123 (34%)       | 63 (14%)        | 77 (16%)        | 0               |
| IV                            | 123 (34%)       | 25 (5%)         | 6 (1%)          | 0               |
| Missing                       | 2 (1%)          | 7 (2%)          | 4 (1%)          | 394 (100%)      |

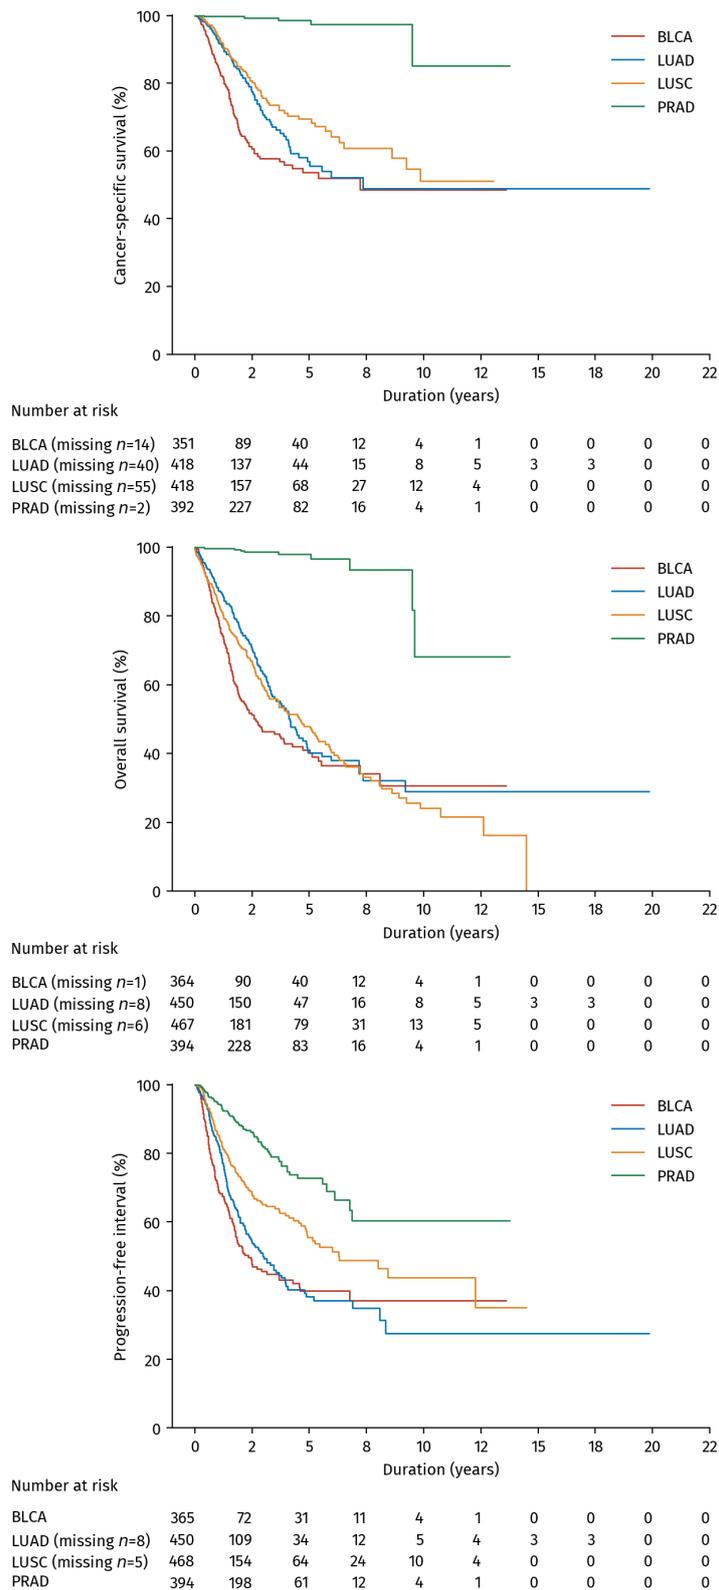

**Figure S28: Kaplan-Meier analysis for included TCGA materials**  
Duration is years since initial diagnosis.

## 5 Protocol amendment

A study protocol that was completed before the method validation is included in its entirety in section 6. It is included exactly how it existed at March 24, 2023, and any errors that were discovered after this date were corrected and presented in the current section rather than editing the protocol document itself.

### 5.1 Protocol section 1.1.4 DEn1 — Endometrial carcinoma

The first paragraph (lines 184 and 185) was left from a previous draft version and should be removed. This material is not part of the MoMaTEC study and the sentence at lines 188 and 189 should therefore be removed: *This material originates from the MoMaTEC (Molecular Markers in Treatment of Endometrial Cancer) trial (NCT number NCT00598845).*[8, 9]

### 5.2 Protocol section 1.2.8 VUr1 — Urothelial carcinoma

Earliest diagnosis date for patient inclusion should be corrected from 1992 to 2002. Specifically, included are all patients with non-muscle invasive urothelial carcinoma of the bladder and without upper urinary tract urothelial carcinoma with primary diagnosis date between 1.1.2002 and 1.1.2011 at Stavanger University Hospital, Norway.

### 5.3 Protocol Table 5 and protocol Fig. 18

Patients with small cell carcinoma were left out when summarising baseline characteristics. Corrected protocol table 5 is found in Table S15 and corrected protocol Fig. 18 is found in Fig. S29.

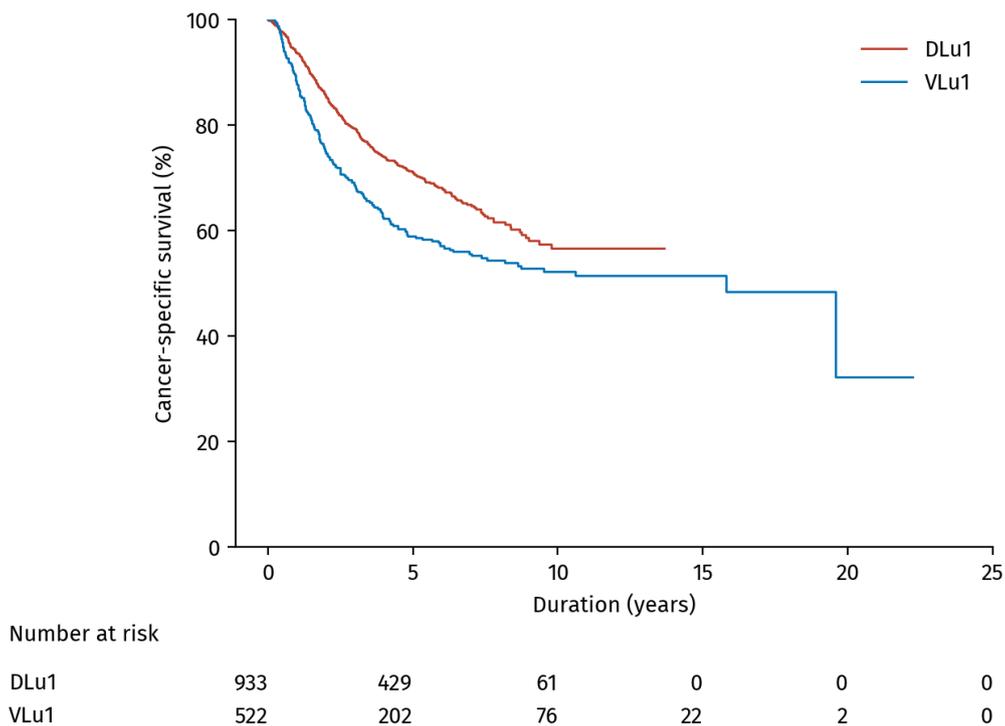

**Figure S29:** Kaplan-Meier analysis of survival in lung carcinoma materials. Duration is years since surgery for DLU1 and years since diagnosis for VLU1.

**Table S15:** Baseline characteristics in lung carcinoma cohorts. Starting point is at surgery for DLu1 and at diagnosis for VLu1.

|                                     | DLu1            | VLu1            |
|-------------------------------------|-----------------|-----------------|
| Patient count                       | 933             | 522             |
| Age                                 |                 |                 |
| Years                               | 68 (62 – 73)    | 68 (60 – 73)    |
| Sex                                 |                 |                 |
| Female                              | 465 (50%)       | 168 (32%)       |
| Male                                | 468 (50%)       | 354 (68%)       |
| Histological type                   |                 |                 |
| Adenocarcinoma                      | 521 (56%)       | 226 (43%)       |
| Adenosquamous carcinoma             | 16 (2%)         | 3 (1%)          |
| Bronchioloalveolar carcinoma        | 8 (1%)          | 0               |
| Carcinoid                           | 42 (5%)         | 0               |
| Large cell carcinoma                | 29 (3%)         | 0               |
| Large cell neuroendocrine carcinoma | 6 (1%)          | 0               |
| Salivary gland type lung carcinoma  | 5 (1%)          | 0               |
| Small cell carcinoma                | 11 (1%)         | 0               |
| Squamous cell carcinoma             | 287 (31%)       | 289 (55%)       |
| Undifferentiated carcinoma          | 4 (<1%)         | 3 (1%)          |
| Mixed                               | 2 (<1%)         | 0               |
| Other                               | 2 (<1%)         | 1 (<1%)         |
| Cancer-specific death               |                 |                 |
| False                               | 641 (69%)       | 316 (61%)       |
| True                                | 292 (31%)       | 206 (39%)       |
| Time to cancer-specific death       |                 |                 |
| Years                               | 2.2 (1.3 – 3.8) | 1.7 (0.9 – 3.2) |
| Follow-up time                      |                 |                 |
| Years                               | 4.6 (2.5 – 6.8) | 3.6 (1.4 – 7.4) |
| pN stage                            |                 |                 |
| pN0                                 | 676 (72%)       | 366 (70%)       |
| pN1                                 | 187 (20%)       | 102 (20%)       |
| pN2                                 | 70 (8%)         | 54 (10%)        |
| pT stage                            |                 |                 |
| pT1                                 | 328 (35%)       | 171 (33%)       |
| pT2                                 | 439 (47%)       | 196 (38%)       |
| pT3                                 | 137 (15%)       | 98 (19%)        |
| pT4                                 | 29 (3%)         | 57 (11%)        |
| Stage                               |                 |                 |
| I                                   | 511 (55%)       | 224 (43%)       |
| II                                  | 276 (30%)       | 170 (33%)       |
| III                                 | 135 (14%)       | 128 (25%)       |
| IV                                  | 11 (1%)         | 0               |

#### 5.4 Protocol Figs. 27, 28, 29, 30

A bug in the pixel counting script swapped counts for background and non-annotated foreground. This means that protocol Figs. 27 (b), 28 (b), 29 (b), 29 (c), 30 (b) and 30 (c) are wrong. The corrected Figs. S30 to S33 should replace the erroneous protocol Figs. 27, 28, 29 and 30, respectively.

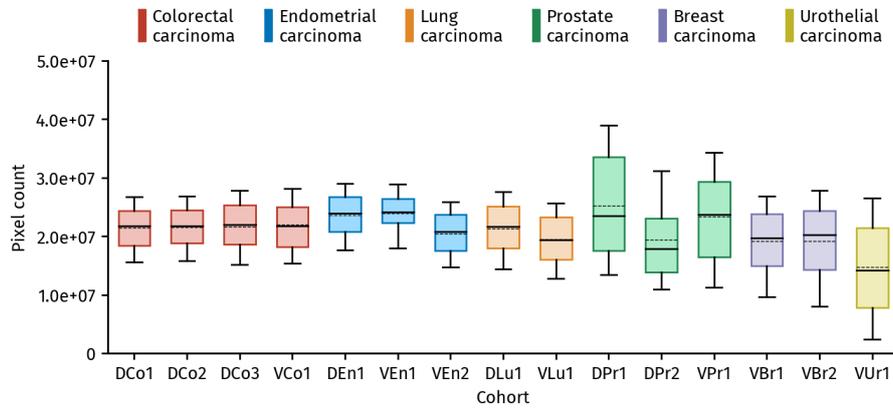

(a) Image area

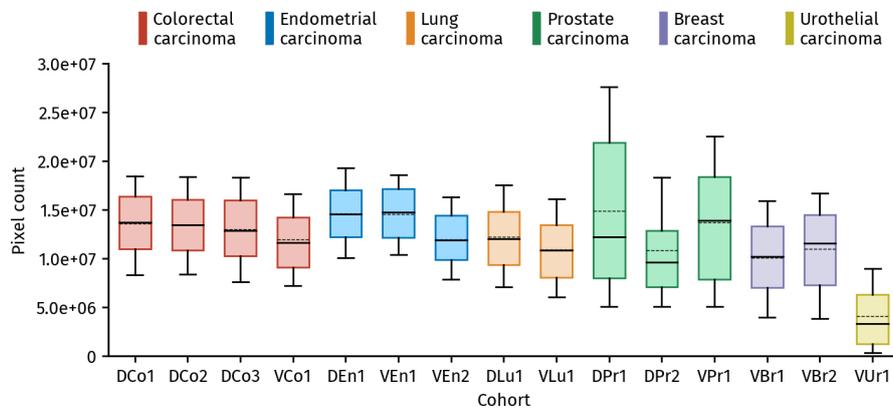

(b) Foreground area

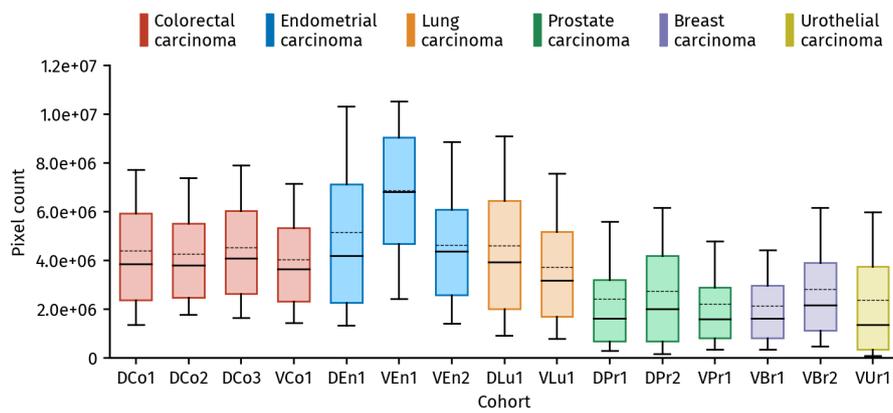

(c) Annotation area

**Figure S30:** Area in number of pixels at resolution 5  $\mu\text{m}$  per pixel in Aperio AP2 scans. “Foreground” is foreground without annotation and “Annotation” is foreground with annotation. Background exclusion masks are applied on all images. Note the difference in vertical axis range between subplots.

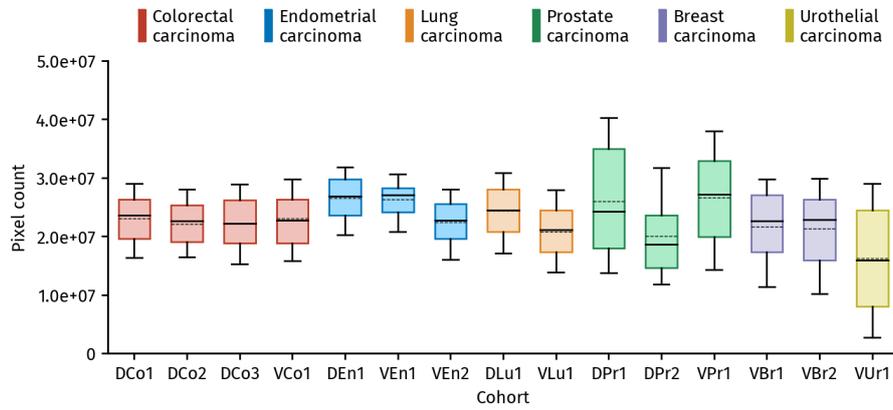

(a) Image area

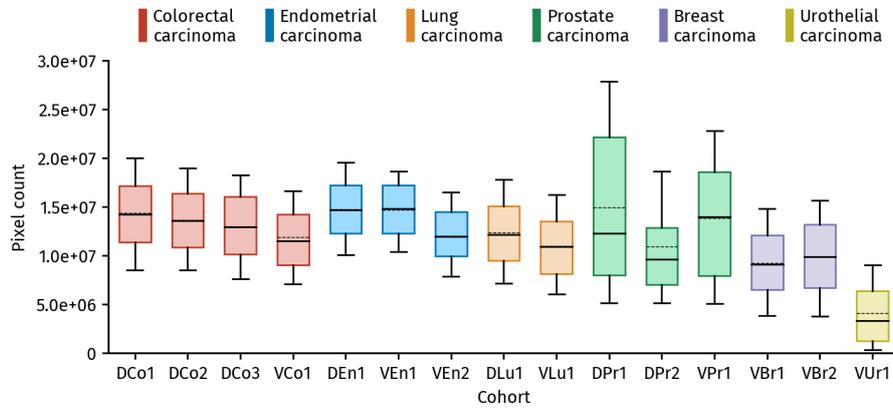

(b) Foreground area

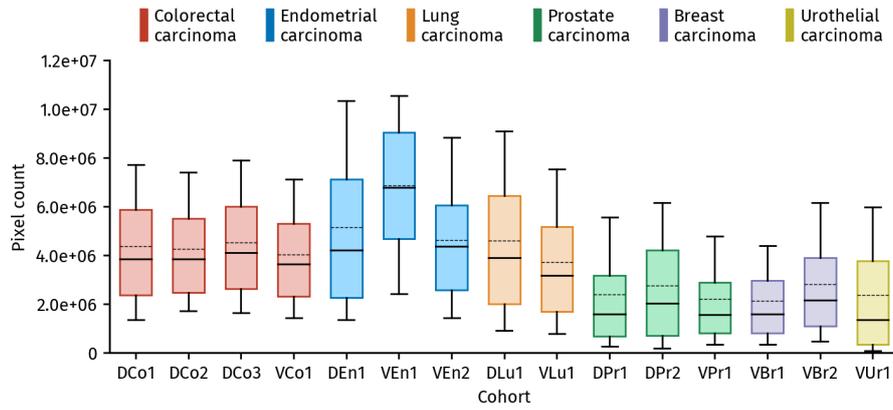

(c) Annotation area

**Figure S31:** Area in number of pixels at resolution 5  $\mu\text{m}$  per pixel in NanoZoomer XR scans. “Foreground” is foreground without annotation and “Annotation” is foreground with annotation. Background exclusion masks are applied on all images. Note the difference in vertical axis range between subplots.

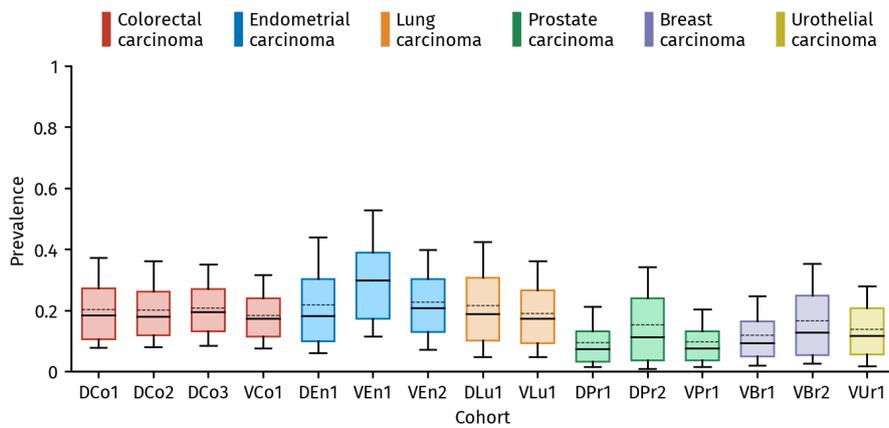

(a) Annotation prevalence in image

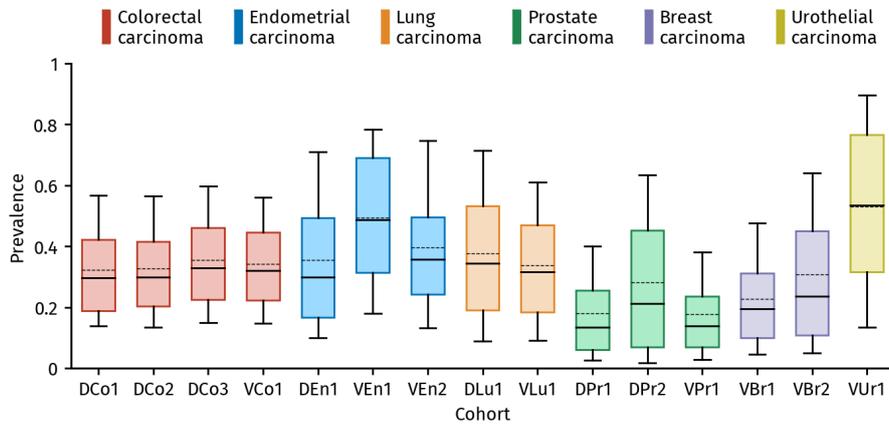

(b) Annotation prevalence in foreground

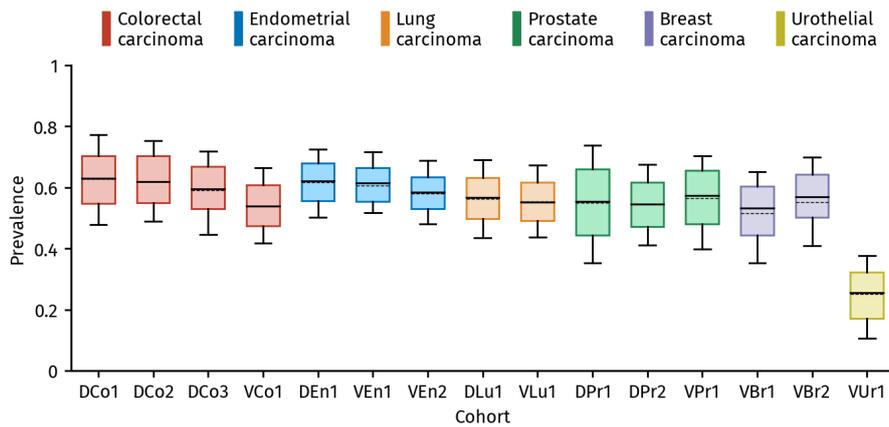

(c) Foreground prevalence in image

**Figure S32:** Prevalence at resolution 5  $\mu$ m per pixel in Aperio AT2 scans. “Foreground” is foreground without annotation and “Annotation” is foreground with annotation. Background exclusion masks are applied on all images.

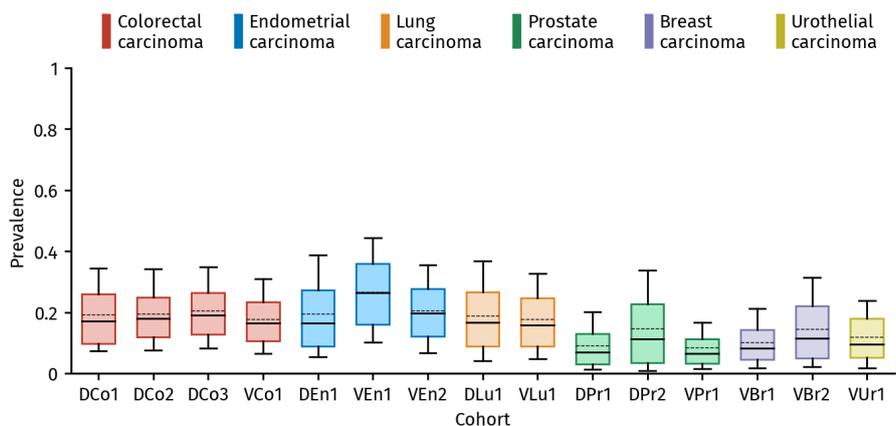

(a) Annotation prevalence in image

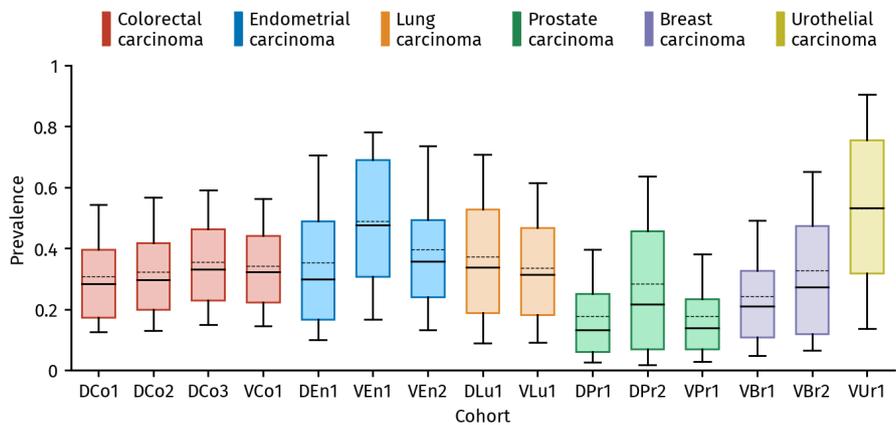

(b) Annotation prevalence in foreground

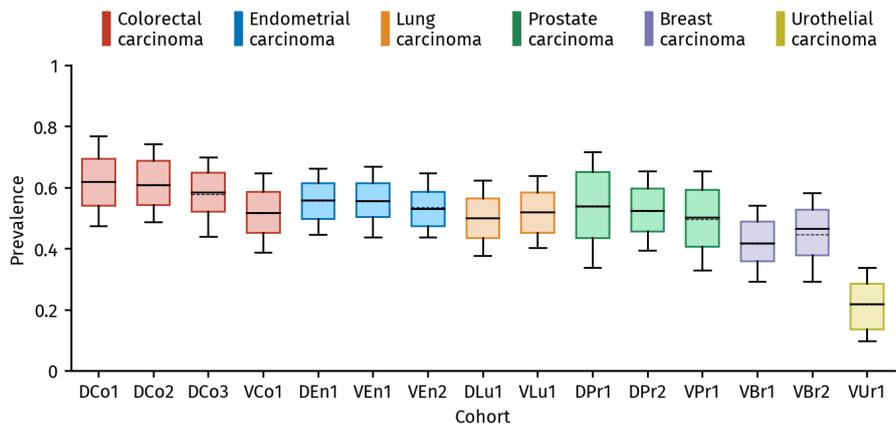

(c) Foreground prevalence in image

**Figure S33:** Prevalence at resolution 5  $\mu\text{m}$  per pixel in NanoZoomer XR scans. “Foreground” is foreground without annotation and “Annotation” is foreground with annotation. Background exclusion masks are applied on all images.

## References

1. Liu, J. *et al.* An integrated TCGA pan-cancer clinical data resource to drive high-quality survival outcome analytics. *Cell* **173**, 400–416 (2018).

## 6 Study protocol

# Protocol for external validation of a pan cancer deep learning method for automatic tumour segmentation in digital histology images

1 This protocol was last modified March 24, 2023, prior to all investigations that could reveal asso-  
2 ciations between the predicted and target segmentation masks in the method validation cohorts.  
3 At that time the method validation cohorts had been scanned, annotated and tiled; baseline char-  
4 acteristics, colour statistics and annotation statistics had been computed; the neural network part  
5 of all methods listed in the primary and secondary analyses had been applied on all tiles, but no  
6 further processing had been performed. All of the above interactions with the validation cohorts  
7 were performed blindly and did not inform choices made in the method development.

## 8 Contents

|    |                                                |           |
|----|------------------------------------------------|-----------|
| 9  | <b>1 Materials</b>                             | <b>1</b>  |
| 10 | 1.1 Materials for method development . . . . . | 2         |
| 11 | 1.1.1 DCo1 — Colorectal carcinoma . . . . .    | 2         |
| 12 | 1.1.2 DCo2 — Colorectal carcinoma . . . . .    | 3         |
| 13 | 1.1.3 DCo3 — Colorectal carcinoma . . . . .    | 4         |
| 14 | 1.1.4 DEn1 — Endometrial carcinoma . . . . .   | 5         |
| 15 | 1.1.5 DLu1 — Lung carcinoma . . . . .          | 7         |
| 16 | 1.1.6 DPr1 — Prostate carcinoma . . . . .      | 7         |
| 17 | 1.1.7 DPr2 — Prostate carcinoma . . . . .      | 8         |
| 18 | 1.2 Materials for method validation . . . . .  | 10        |
| 19 | 1.2.1 VCo1 — Colorectal carcinoma . . . . .    | 10        |
| 20 | 1.2.2 VEn1 — Endometrial carcinoma . . . . .   | 11        |
| 21 | 1.2.3 VEn2 — Endometrial carcinoma . . . . .   | 12        |
| 22 | 1.2.4 VLu1 — Lung carcinoma . . . . .          | 13        |
| 23 | 1.2.5 VPr1 — Prostate carcinoma . . . . .      | 13        |
| 24 | 1.2.6 VBr1 — Breast carcinoma . . . . .        | 14        |
| 25 | 1.2.7 VBr2 — Breast carcinoma . . . . .        | 15        |
| 26 | 1.2.8 VUr1 — Urothelial carcinoma . . . . .    | 16        |
| 27 | 1.3 Material analyses . . . . .                | 17        |
| 28 | 1.3.1 Baseline characteristics . . . . .       | 17        |
| 29 | 1.3.2 Survival characteristics . . . . .       | 23        |
| 30 | 1.3.3 Colour statistics . . . . .              | 29        |
| 31 | <b>2 Methods</b>                               | <b>33</b> |
| 32 | 2.1 Programming environment . . . . .          | 33        |
| 33 | 2.2 Method development . . . . .               | 33        |
| 34 | 2.2.1 Downsampling . . . . .                   | 34        |
| 35 | 2.2.2 Tiling . . . . .                         | 34        |
| 36 | 2.2.3 Dataset balancing . . . . .              | 36        |
| 37 | 2.2.4 Background segmentation . . . . .        | 36        |
| 38 | 2.2.5 Background tile exclusion . . . . .      | 43        |
| 39 | 2.2.6 Dataset augmentations . . . . .          | 45        |

|    |          |                                                                      |           |
|----|----------|----------------------------------------------------------------------|-----------|
| 40 | 2.2.7    | Image value standardisation . . . . .                                | 45        |
| 41 | 2.2.8    | Segmentation network . . . . .                                       | 49        |
| 42 | 2.2.9    | Network optimisation . . . . .                                       | 50        |
| 43 | 2.3      | Method application . . . . .                                         | 51        |
| 44 | 2.3.1    | Downsampling and tiling . . . . .                                    | 51        |
| 45 | 2.3.2    | Neural network . . . . .                                             | 51        |
| 46 | 2.3.3    | Reconstruction from tiles . . . . .                                  | 52        |
| 47 | 2.3.4    | Result post-processing . . . . .                                     | 53        |
| 48 | 2.4      | Performance evaluation . . . . .                                     | 54        |
| 49 | 2.4.1    | Overlap counting . . . . .                                           | 54        |
| 50 | <b>3</b> | <b>Analyses</b>                                                      | <b>57</b> |
| 51 | 3.1      | Primary analysis . . . . .                                           | 57        |
| 52 | 3.2      | Secondary analyses . . . . .                                         | 57        |
| 53 | 3.2.1    | Different performance evaluation metrics of primary result . . . . . | 57        |
| 54 | 3.2.2    | Primary result on scans from the NanoZoomer XR . . . . .             | 57        |
| 55 | 3.2.3    | Single cancer type training . . . . .                                | 57        |
| 56 | 3.2.4    | Primary analysis replication . . . . .                               | 58        |

57 **List of Figures**

|    |    |                                                                         |    |
|----|----|-------------------------------------------------------------------------|----|
| 58 | 1  | Acquisition overview DCo1 . . . . .                                     | 3  |
| 59 | 2  | Acquisition overview DCo2 . . . . .                                     | 3  |
| 60 | 3  | Acquisition overview DCo3 . . . . .                                     | 4  |
| 61 | 4  | Acquisition overview DEn1 . . . . .                                     | 6  |
| 62 | 5  | Acquisition overview DLu1 . . . . .                                     | 7  |
| 63 | 6  | Acquisition overview DPr1 . . . . .                                     | 8  |
| 64 | 7  | Acquisition overview DPr2 . . . . .                                     | 9  |
| 65 | 8  | Acquisition overview VCo1 . . . . .                                     | 11 |
| 66 | 9  | Acquisition overview VEn1 . . . . .                                     | 12 |
| 67 | 10 | Acquisition overview VEn2 . . . . .                                     | 12 |
| 68 | 11 | Acquisition overview VLu1 . . . . .                                     | 13 |
| 69 | 12 | Acquisition overview VPr1 . . . . .                                     | 14 |
| 70 | 13 | Acquisition overview VBr1 . . . . .                                     | 15 |
| 71 | 14 | Acquisition overview VBr2 . . . . .                                     | 15 |
| 72 | 15 | Acquisition overview VUr1 . . . . .                                     | 16 |
| 73 | 16 | Kaplan-Meier analysis in materials from colorectal carcinoma . . . . .  | 23 |
| 74 | 17 | Kaplan-Meier analysis in materials from endometrial carcinoma . . . . . | 24 |
| 75 | 18 | Kaplan-Meier analysis in materials from lung carcinoma . . . . .        | 25 |
| 76 | 19 | Kaplan-Meier analysis in materials from prostate carcinoma . . . . .    | 26 |
| 77 | 20 | Kaplan-Meier analysis in materials from urothelial carcinoma . . . . .  | 27 |
| 78 | 21 | Kaplan-Meier analysis in materials from urothelial carcinoma . . . . .  | 28 |
| 79 | 22 | Scan colour mean value Aperio AT2 . . . . .                             | 29 |
| 80 | 23 | Scan colour mean value NanoZoomer XR . . . . .                          | 30 |
| 81 | 24 | Scan colour standard deviation Aperio AT2 . . . . .                     | 31 |
| 82 | 25 | Scan colour standard deviation NanoZoomer XR . . . . .                  | 32 |
| 83 | 26 | Background exclusion example . . . . .                                  | 38 |
| 84 | 27 | Scan area Aperio AT2 . . . . .                                          | 39 |
| 85 | 28 | Scan area NanoZoomer XR . . . . .                                       | 40 |
| 86 | 29 | Scan content prevalence Aperio AT2 . . . . .                            | 41 |
| 87 | 30 | Scan content prevalence NanoZoomer XR . . . . .                         | 42 |
| 88 | 31 | Background exclusion statistics . . . . .                               | 44 |
| 89 | 32 | Tile colour mean value . . . . .                                        | 47 |
| 90 | 33 | Tile colour standard deviation . . . . .                                | 48 |
| 91 | 34 | Segmentation network architecture . . . . .                             | 49 |
| 92 | 35 | Step length schedule . . . . .                                          | 51 |
| 93 | 36 | Tiling example . . . . .                                                | 52 |
| 94 | 37 | Overlap weight tiles . . . . .                                          | 53 |

95 **List of Tables**

|     |    |                                                                            |    |
|-----|----|----------------------------------------------------------------------------|----|
| 96  | 1  | Data count in development cohorts . . . . .                                | 2  |
| 97  | 2  | Data count in validation cohorts . . . . .                                 | 10 |
| 98  | 3  | Baseline characteristics in materials from colorectal carcinoma . . . . .  | 17 |
| 99  | 4  | Baseline characteristics in materials from endometrial carcinoma . . . . . | 18 |
| 100 | 5  | Baseline characteristics in materials from lung carcinoma . . . . .        | 19 |
| 101 | 6  | Baseline characteristics in materials from prostate carcinoma . . . . .    | 20 |
| 102 | 7  | Baseline characteristics in materials from breast carcinoma . . . . .      | 21 |
| 103 | 8  | Baseline characteristics in materials from urothelial carcinoma . . . . .  | 22 |
| 104 | 9  | Python packages . . . . .                                                  | 33 |
| 105 | 10 | Annotated scan count after balancing . . . . .                             | 36 |
| 106 | 11 | Development set tile count . . . . .                                       | 43 |
| 107 | 12 | Colour statistics in tiles from development set . . . . .                  | 46 |
| 108 | 13 | Confusion matrix . . . . .                                                 | 55 |

# 109 1 Materials

110 Images analysed in this study are images of thin slices of resected solid tumours. Details about  
111 how these images are acquired follows below, before a per-cohort characterisation is presented.

112 The mass of interest is surgically removed from the patient and placed in containers with  
113 formalin for fixation. Pathologists examine the formalin-fixed specimen and regions of interest are  
114 cut into blocks and embedded in paraffin. The formalin-fixed paraffin-embedded (FFPE) blocks  
115 are sliced into thin tissue sections using a microtome and mounted on slides. Unless otherwise  
116 specified, the sections used in this study have thickness 3  $\mu\text{m}$ . The tissue section is then stained  
117 with conventional haematoxylin and eosin (H&E), prepared as a tissue slide and imaged with a  
118 microscope scanner to form a so-called whole slide image (WSI).

119 This scan is then examined by a pathologist, and the tumour area, if any, is delineated. When  
120 the tissue slide is scanned by multiple different scanners, the digital tumour annotation is usually  
121 created on a scan from one scanner and digitally transformed to match the corresponding scan from  
122 different scanners. In these cases the transferred tumour annotation is verified by a pathologist,  
123 who corrects the annotation when necessary. If the transfer fails, the destination scan is manually  
124 annotated. To transform the annotation from the source scan to the destination scan, we first  
125 downsample the scans by a factor of 32. Then an image registration from the source image  
126 to the destination image is computed using a scale-invariant feature transform (SIFT).[1] This  
127 transformation is then used to transfer the polygons of the source annotation to the destination  
128 image.

129 In some of the cohorts, FFPE blocks are received at the Institute for Cancer Genetics and Infor-  
130 matics (ICGI), Oslo University Hospital, Norway, and sectioned, stained, scanned, and annotated  
131 by laboratory technicians. For other cohorts, we receive H&E stained tissue slides which we scan.  
132 In the remaining cohorts we receive digital scan files. What kind of material we received for each  
133 particular cohort studied will be specified in the cohort description (section 1.1 and section 1.2).

134 In this study, we use two scanners; the Aperio AT2 (Leica Biosystems, Germany) and the  
135 NanoZoomer XR (Hamamatsu Photonics, Japan). Digital scan files are read using the *Python*  
136 interface of the *OpenSlide C* library version 3.4.1.[2]

137 All cohorts are presented in section 1.1 and section 1.2 for method development and valida-  
138 tion cohorts, respectively. Further descriptive analyses of the included materials are presented in  
139 section 1.3.

140 It should be noted that the materials were chiefly acquired for other projects, and not this seg-

141 mentation study. The exclusion reasons are therefore, in general, not consistent between materials.  
 142 Also, some exclusion reasons would perhaps not have been applied if the material were acquired  
 143 specifically for tumour segmentation.

144 Unless otherwise specified, all included scans in this study were manually annotated by pathol-  
 145 ogist Manohar Pradhan (MP) with over fifteen years of experience at the time the first cohorts in  
 146 this study were annotated.

## 147 1.1 Materials for method development

148 20 270 scans from two scanners and 4 305 patients from 7 different cohorts were used in developing  
 149 the tumour segmentation method; 3 from colorectal carcinoma, 1 from endometrial carcinoma, 1  
 150 from lung carcinoma and 2 from prostate carcinoma (protocol table 1).

**Protocol Table 1:** Number of patients, annotated scans and tiles in the development cohorts. Scans are from two different scanners. Tiles are produced at resolution 1  $\mu\text{m}$  per pixel and have a size of  $2048 \times 2048$  pixels.

| Cancer type           | Cohort | Patients | Scans      |               | Tiles      |               |
|-----------------------|--------|----------|------------|---------------|------------|---------------|
|                       |        |          | Aperio AT2 | NanoZoomer XR | Aperio AT2 | NanoZoomer XR |
| Colorectal carcinoma  | DCo1   | 206      | 206        | 206           | 28 911     | 30 552        |
|                       | DCo2   | 578      | 578        | 575           | 81 651     | 82 294        |
|                       | DCo3   | 765      | 765        | 764           | 108 429    | 109 720       |
|                       | Sum    | 1 549    | 1 549      | 1 545         | 218 991    | 222 566       |
| Endometrial carcinoma | DEn1   | 1 241    | 3 340      | 3 340         | 514 341    | 566 105       |
| Lung carcinoma        | DLu1   | 933      | 3 519      | 3 519         | 492 150    | 551 767       |
| Prostate carcinoma    | DPr1   | 328      | 976        | 976           | 158 001    | 163 527       |
|                       | DPr2   | 254      | 753        | 753           | 95 015     | 97 867        |
|                       | Sum    | 582      | 1 729      | 1 729         | 253 016    | 261 394       |
| Sum                   |        | 4 305    | 10 137     | 10 133        | 1 478 498  | 1 601 832     |

### 151 1.1.1 DCo1 — Colorectal carcinoma

152 224 patients with colonic adenocarcinoma and adjacent normal mucosa treated between 1988 and  
 153 2000 at Akershus University Hospital, Norway.[3, 4] Tissue blocks were received at ICGI, prepared  
 154 as tissue slides and scanned. After exclusions, (see protocol figure 1) 206 annotated scans remained  
 155 from both the Aperio AT2 the NanoZoomer XR scanner.

156 Scans from Aperio AT2 were manually annotated for tumour by a pathologist (MP), and these  
 157 tumour annotations were transferred to the corresponding NanoZoomer XR scans.

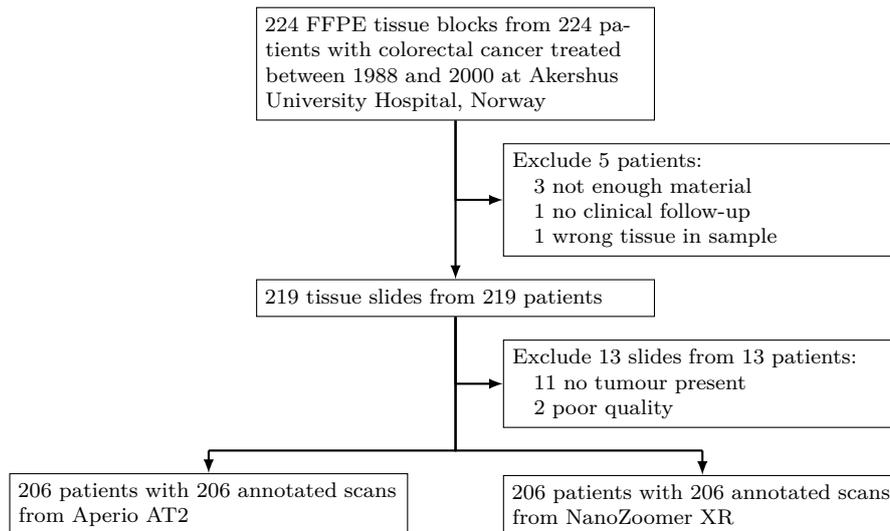

**Protocol Figure 1:** Flow from received blocks to annotated scans for the DCo1 cohort

158 **1.1.2 DCo2 — Colorectal carcinoma**

159 The material origin are patients with colorectal cancer treated between 1993 and 2003 at Aker  
 160 Hospital (now part of Oslo University Hospital), Norway. 578 patients with resected tissue  
 161 section and stages I, II, and III colorectal cancer that were analysed in previous studies were  
 162 included.[4, 5, 6] One tissue slide per patient was prepared at ICGI, and scanned with the Aperio  
 163 AT2 and NanoZoomer XR scanners. Three slides that had already been scanned with the Aperio  
 164 AT2 scanner could not be scanned with the NanoZoomer XR scanner because of damaged cover  
 165 glass. This resulted in 578 annotated scans from the Aperio AT2 scanner and 575 scans from the  
 166 NanoZoomer XR scanner (summarised in protocol figure 2).

167 Scans from Aperio AT2 were manually annotated for tumour by a pathologist (MP), and these  
 168 tumour annotations were transferred to the corresponding NanoZoomer XR scans.

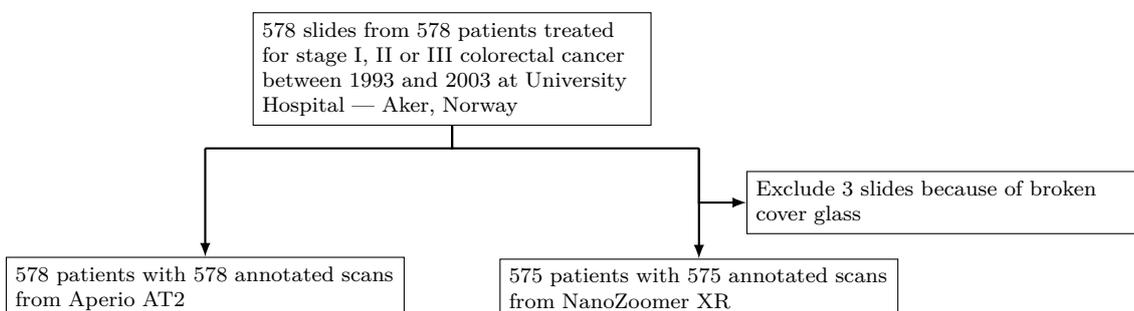

**Protocol Figure 2:** Flow from inclusions in previous studies (reference [5, 6]) to annotated scans for the DCo2 cohort

169 **1.1.3 DCo3 — Colorectal carcinoma**

170 2327 patients with histologically proven stage II or III colorectal cancer and resected primary tumour recruited from 151 hospitals in the United Kingdom between 2002 and 2004 for the *VICTOR*  
 171 trial and randomly assigned to receive either rofecoxib (1167 patients) or placebo (1160 patients). [7]  
 172 From 795 patients that we have included in a previous study, 795 H&E stained tissue sections were  
 173 obtained at ICGI. [4] Some tissue sections were sectioned from FFPE blocks at ICGI, and some  
 174 elsewhere. After exclusions as in reference [4] we had 768 scans from the Aperio AT2 scanner and  
 175 768 scans from the NanoZoomer XR scanner (see protocol figure 3). Two additional patients were  
 176 excluded since their slides were of poor quality, and the scans of the new sections did not have man-  
 177 ual annotations. One additional slide was also excluded because of no presence of tumour in the  
 178 tissue section. A final scan from the NanoZoomer XR scanner was excluded since the annotation  
 179 did not match the scan.  
 180

181 In this cohort, scans from NanoZoomer XR were manually annotated for tumour by a pathol-  
 182 ogist (MP) and these annotations were transferred to the corresponding Aperio AT2 scans.

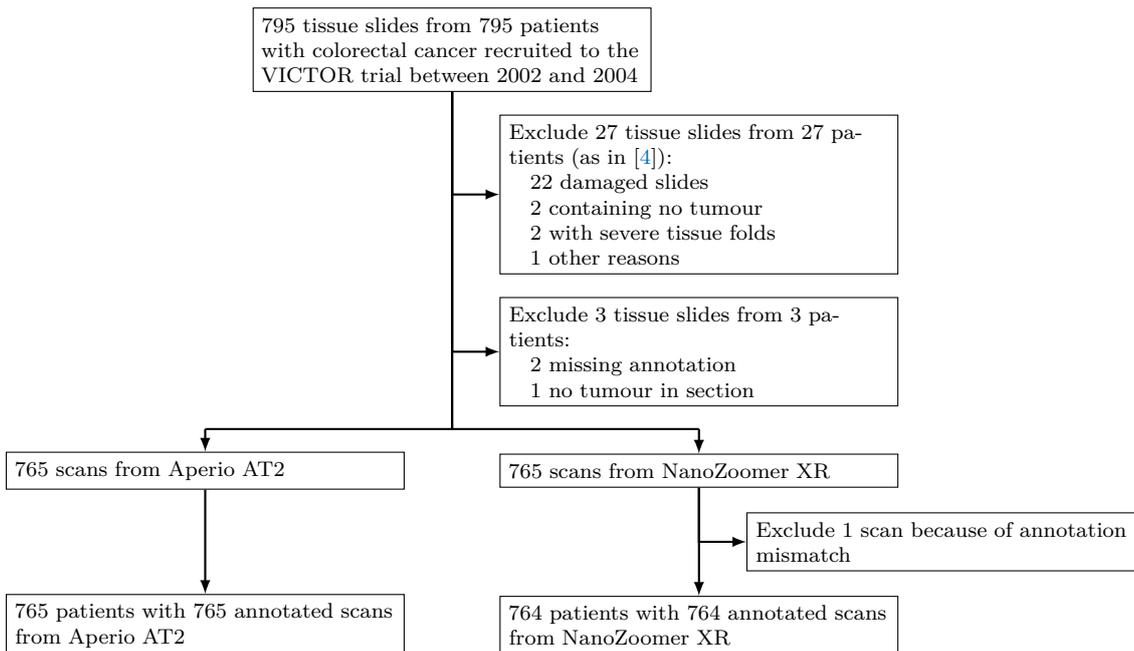

**Protocol Figure 3:** Flow from received slides to annotated scans for the DCo3 cohort

183 **1.1.4 DEn1 — Endometrial carcinoma**

184 We considered 1795 patients who underwent surgery for endometrial carcinoma between 2006 and  
185 2018 at Oslo University Hospital, Norway.

186 We considered 1795 patients referred to the Department of Gynecological Oncology at Oslo  
187 University Hospital (OUH), Norway, and diagnosed *or* operated for endometrial carcinoma at  
188 OUH between 2006 and 2017. This material originates from the MoMaTEC (Molecular Markers  
189 in Treatment of Endometrial Cancer) trial (NCT number NCT00598845).[8, 9]

190 Note that among the 1795 patients, 11 patients (with 28 FFPE tumour blocks) had neuroen-  
191 docrine tumours, which was removed from the World Health Organization classification of endome-  
192 trial carcinoma between the 2014 edition and the 2020 edition.[10, 11]

193 FFPE blocks were collected by ICGI and prepared as tissue slides. Large sections were split  
194 and placed on two slides. After exclusions (see protocol figure 4), there remained 1229 patients  
195 with 4760 FFPE tumour blocks. At most three FFPE blocks were randomly selected from each  
196 patient, except for patients with tumours with mixed histology where all blocks were selected. This  
197 reduced the number of included blocks to 3331. 11 sections from 11 blocks were too large for a  
198 single slide and were placed on two slides. With this we have 1241 patients and 3331 blocks with  
199 3340 annotated scans from Aperio AT2 and NanoZoomer XR.

200 After an update of the source of this material (after training but before validation), the following  
201 inconsistencies were noticed: 2 patients with 3 blocks each should have been excluded due to  
202 previous irradiation to a pelvic field including the uterus, 2 patients with 3 blocks each should  
203 have been excluded due to neoadjuvant treatment, 1 patient with 3 blocks was wrongly excluded  
204 due to complications after surgery. Protocol Figure 4 describe the material that was used in this  
205 study.

206 Scans from the NanoZoomer XR scanner were manually annotated for tumour by a pathologist  
207 (MP) and automatically transferred to the corresponding scans from the Aperio AT2 scanner.

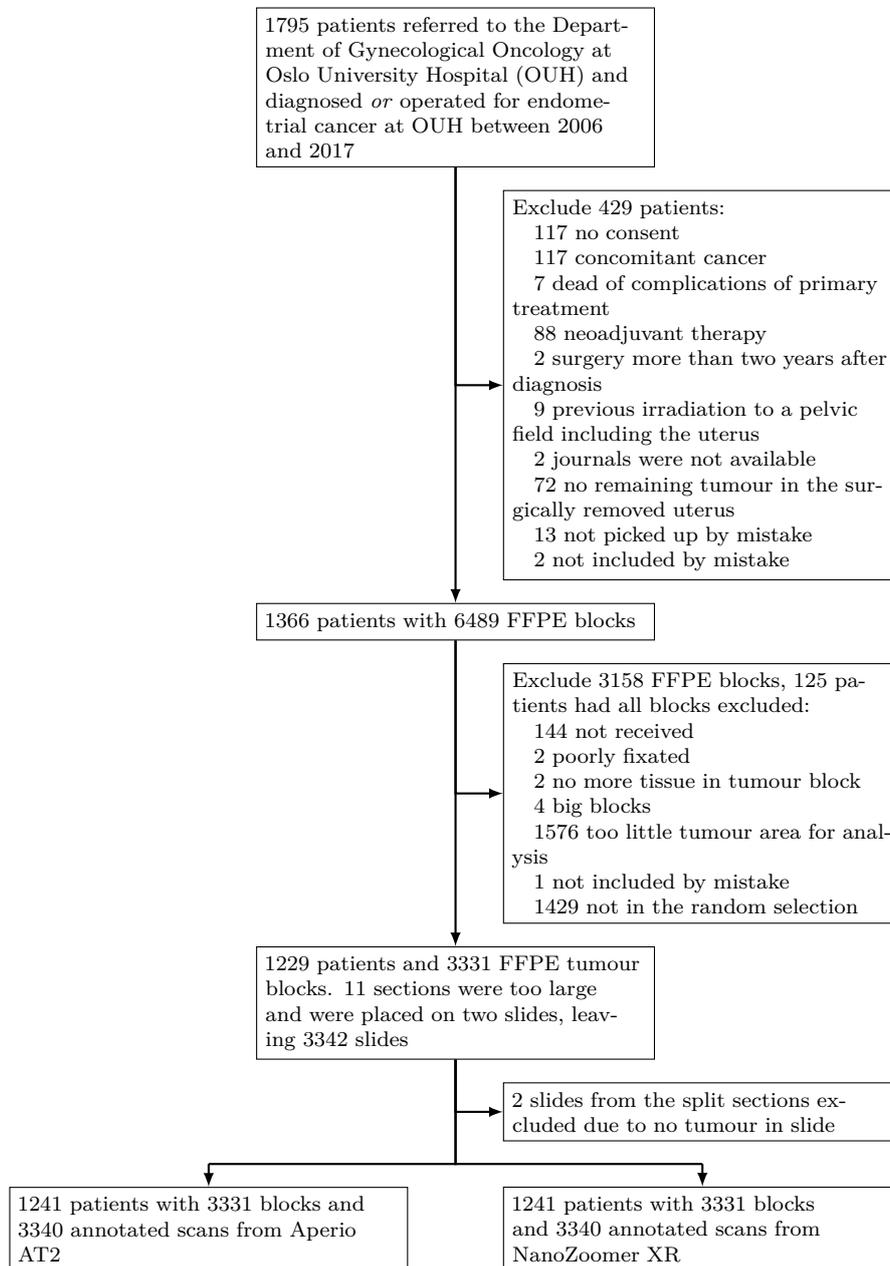

**Protocol Figure 4:** Flow from operated patients to annotated scans for the DEn1 cohort

208 **1.1.5 DLu1 — Lung carcinoma**

209 967 patients resected for primary lung cancer as part of primary treatment between March 2006  
210 and December 2018 at Oslo University Hospital, Norway. FFPE tissue blocks were requested from  
211 all but 5 excluded patients (see protocol figure 5) from pathology departments at Oslo University  
212 Hospital. 3519 H&E slides were successfully prepared at ICGI from 3519 FFPE tissue blocks from  
213 933 patients.

214 Scans from the NanoZoomer XR scanner were manually annotated by a pathologist (MP) and  
215 trained laboratory technician Jonathan Gullesen (JG). Annotations were verified and corrected if  
216 needed by a pathologist (MP). Large areas of fibrous tissue and necrosis were not included in the  
217 annotation. The manual annotations were automatically transferred to the corresponding Aperio  
218 AT2 scans.

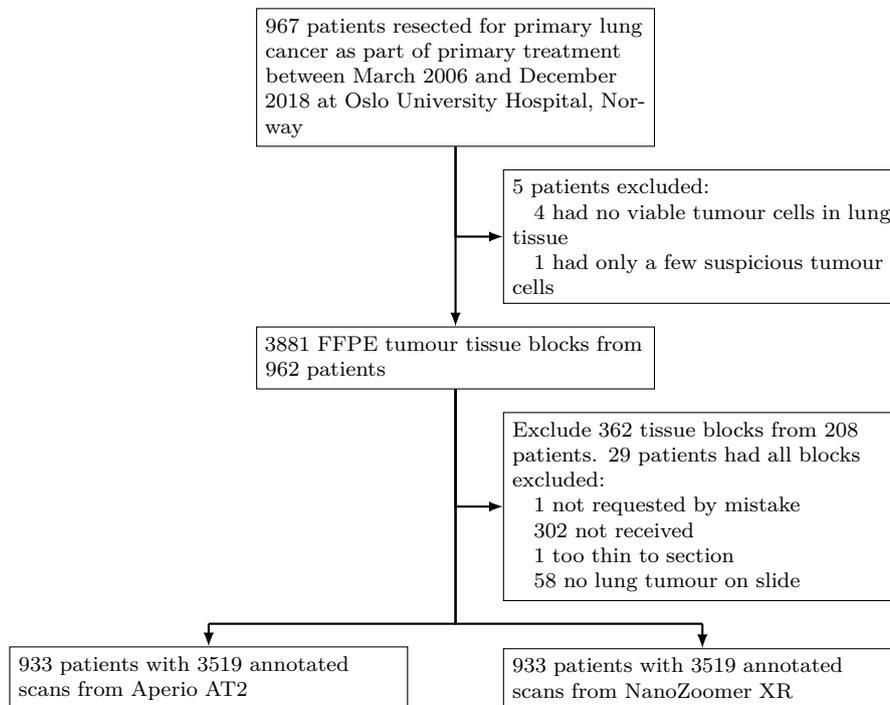

**Protocol Figure 5:** Flow from eligible patients to annotated scans for the DLu1 cohort

219 **1.1.6 DPr1 — Prostate carcinoma**

220 The cohort comprised 389 patients who underwent radical prostatectomy (RP) between 1999 and  
221 2010 at Vestfold Hospital Trust, Norway. 61 patients were excluded: 26 for missing FFPE blocks, 6  
222 for no tumour material and 29 patients for failing one or more FFPE block selection criteria. The

223 criteria were: one block with the highest Gleason score, a second block with the largest tumour  
 224 area, a third block selected randomly from the remaining blocks with a tumour area  $> 16 \text{ mm}^2$   
 225 on a diagnostic H&E section.[12] At scan preparation, 7 blocks were excluded, and a further slide  
 226 was excluded since this slide was missing when Aperio scanning was performed, leaving us with  
 227 976 annotated scans from both Aperio AT2 and NanoZoomer XR originating from 328 patients  
 228 (summarised in protocol figure 6).

229 Tumour areas in scans from Aperio AT2 were manually annotated by a pathologist (MP) and  
 230 large benign areas were avoided. These manual annotations were automatically transferred to  
 231 NanoZoomer XR scans.

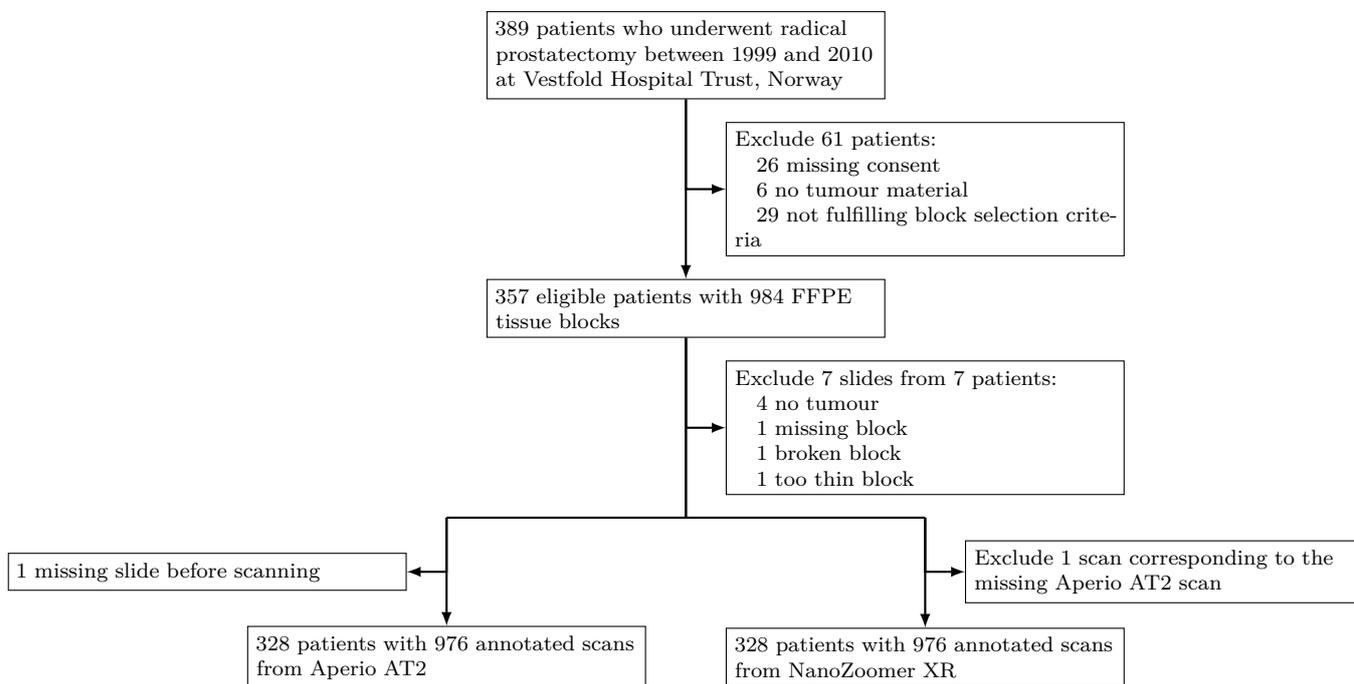

**Protocol Figure 6:** Flow from operated patients to annotated scans for the DPr1 cohort

### 232 1.1.7 DPr2 — Prostate carcinoma

233 The cohort originally comprised 317 patients who underwent RP between 1987 and 2005 at the  
 234 Norwegian Radium Hospital (now part of Oslo University Hospital), Norway. Inclusion criteria for  
 235 RP were preoperative absence of known metastases, age less than 75 years and life expectancy of  
 236 at least 10 years. Adjuvant therapy was started in cases with elevated PSA after surgery and/or  
 237 metastatic disease. All patients were operated by one surgeon (Håkon Wæhre).[13]

238 After exclusions (see protocol figure 7) there remained 307 eligible patients, of which 255 pa-  
 239 tients had three available tumour-containing blocks and were therefore included for further analyses.  
 240 The assessment was based on the highest Gleason sum and/or previously assessed non-diploid DNA  
 241 ploidy status, that had tumour areas measuring  $> 4 \text{ mm}^2$  on a diagnostic H&E section.[14] After  
 242 further exclusions, we had 753 annotated scans from 254 patients (245 patients with 3 scans each  
 243 and 9 patients with 2 scans each) from both the Aperio AT2 scanner and the NanoZoomer XR  
 244 scanner.

245 Tumour areas were manually annotated avoiding large benign areas. 50% of the Aperio AT2  
 246 scans were manually annotated by a pathologist (MP) and automatically transferred to the cor-  
 247 responding NanoZoomer XR scans. The other 50% of the NanoZoomer XR scans were manually  
 248 annotated by a laboratory technician (JG). Annotations were verified and corrected if needed by a  
 249 pathologist (MP). These annotations were automatically transferred to the corresponding Aperio  
 250 AT2 scans.

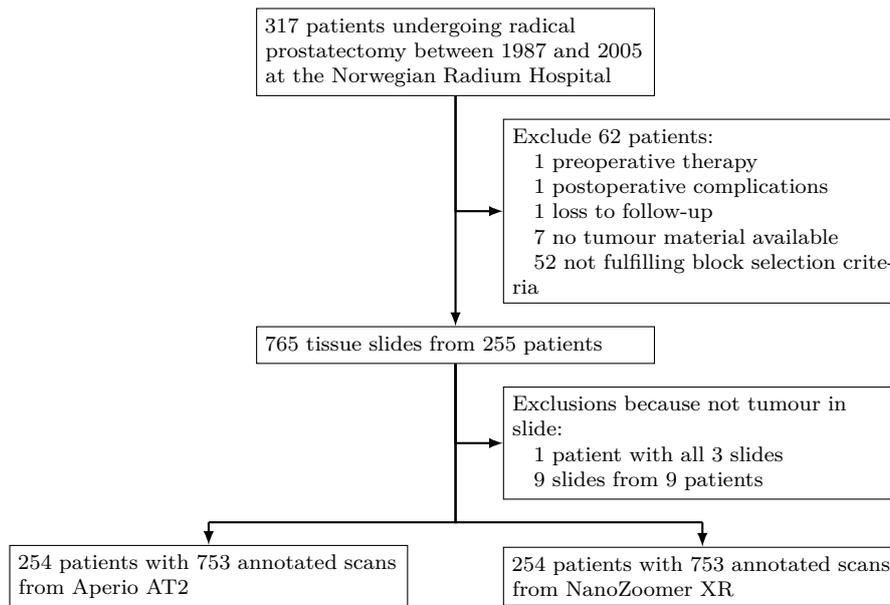

**Protocol Figure 7:** Flow from operated patients to annotated scans for the DPr2 cohort

251 **1.2 Materials for method validation**

252 7 258 scans from two scanners and 3 068 patients from 8 different cohorts were used in validating  
 253 the tumour segmentation method; 1 from colorectal carcinoma, 2 from endometrial carcinoma, 1  
 254 from lung carcinoma, 1 from prostate carcinoma, 1 from bladder carcinoma and 2 from breast  
 255 carcinoma (see protocol table 2).

256 All included scans from all validation cohorts were manually segmented prior to any investiga-  
 257 tion that could reveal correlations between predicted segmentation masks and manually segmented  
 258 target masks. All validation cohorts were primarily manually segmented for purposes other than  
 259 serving as validation cohorts for this project, and had already been manually segmented when  
 260 this project was initiated. These manual segmentations did not inform the development of the  
 261 presented segmentation method, nor did the development of the presented segmentation method  
 262 inform the manual segmentation.

**Protocol Table 2:** Number of patients, annotated scans and tiles in the validation cohorts. Scans are from two different scanners. Tiles are produced at resolution 1  $\mu\text{m}$  per pixel and have a size of 7 680  $\times$  7 680 pixels

| Cancer type           | Cohort | Patients | Scans      |               | Tiles      |               |
|-----------------------|--------|----------|------------|---------------|------------|---------------|
|                       |        |          | Aperio AT2 | NanoZoomer XR | Aperio AT2 | NanoZoomer XR |
| Colorectal carcinoma  | VCo1   | 1 132    | 1 155      | 1 155         | 17 686     | 18 635        |
| Endometrial carcinoma | VEn1   | 77       | 77         | 77            | 1 279      | 1 408         |
|                       | VEn2   | 132      | 152        | 152           | 2 179      | 2 383         |
|                       | Sum    | 209      | 229        | 229           | 3 458      | 3 791         |
| Lung carcinoma        | VLu1   | 522      | 522        | 522           | 7 100      | 7 649         |
| Prostate carcinoma    | VPr1   | 259      | 777        | 777           | 12 568     | 14 072        |
| Breast carcinoma      | VBr1   | 310      | 310        | 310           | 4 165      | 4 689         |
|                       | VBr2   | 304      | 304        | 304           | 4 098      | 4 576         |
|                       | Sum    | 614      | 614        | 614           | 8 263      | 9 265         |
| Urothelial carcinoma  | VUr1   | 332      | 332        | 332           | 3 446      | 3 814         |
| Sum                   |        | 3 068    | 3 629      | 3 629         | 52 521     | 57 226        |

263 **1.2.1 VCo1 — Colorectal carcinoma**

264 This cohort comprises participants in the QUASAR 2 (QUick And Simple And Reliable) trial  
 265 (ISRCTN registry number ISRCTN45133151). Between 2005 and 2010, 1952 eligible patients were  
 266 enrolled from 170 hospitals in seven countries (Australia, Austria, Czeck Republic, New Zealand,

267 Serbia, Slovenia, and the UK). The trial investigated the effect of bevacizumab on disease-free  
 268 survival after potentially curative surgery of primary tumour.[15] FFPE tissue blocks were collected  
 269 from 1 251 patients with either stage II or III colorectal cancer, of whom usable tissue blocks from  
 270 1 140 patients were received at ICGI.[4] After exclusions (see protocol figure 8) we had 1132 eligible  
 271 patients with 1155 annotated scans from the Aperio AT2 scanner and the NanoZoomer XR scanner.  
 272 Note that there were originally one section per patient, but some large sections had to be split  
 273 before scanning in order to fit the cover slip.

274 Scans from both Aperio AT2 and NanoZoomer XR were manually annotated for tumour by a  
 275 pathologist (MP).

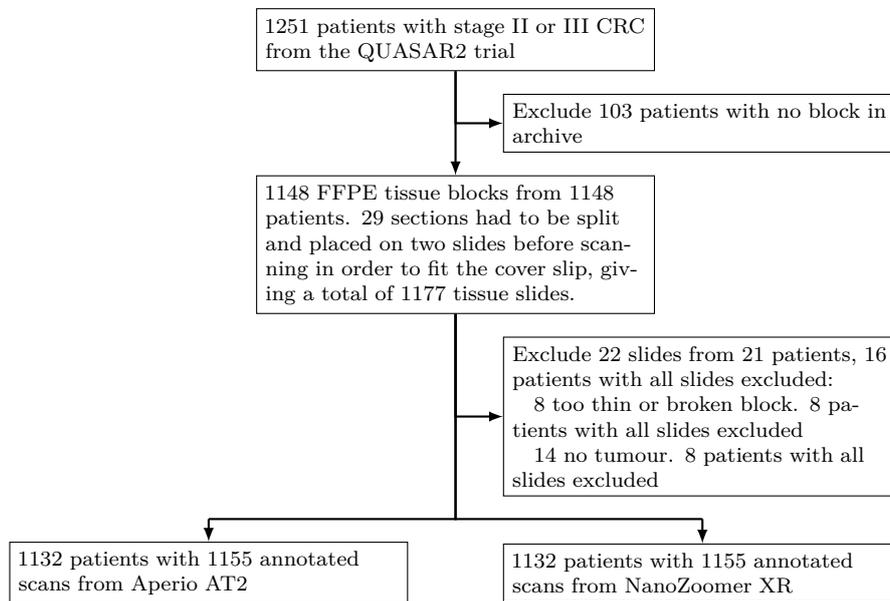

**Protocol Figure 8:** Flow from eligible patients to annotated scans for the VCo1 cohort

276 **1.2.2 VEn1 — Endometrial carcinoma**

277 95 blocks from 95 patients collected between 2001 and 2016 at Amsterdam Medical Center, The  
 278 Netherlands. Six patients were excluded for clinical reasons, after which a further twelve blocks were  
 279 excluded, leaving 77 patients with 77 annotated scans from both the Aperio AT2 and NanoZoomer  
 280 XR scanner (see protocol figure 9).

281 Scans from the NanoZoomer XR scanner were manually annotated by a pathologist (MP) and  
 282 transferred to the corresponding Aperio AT2 scans.

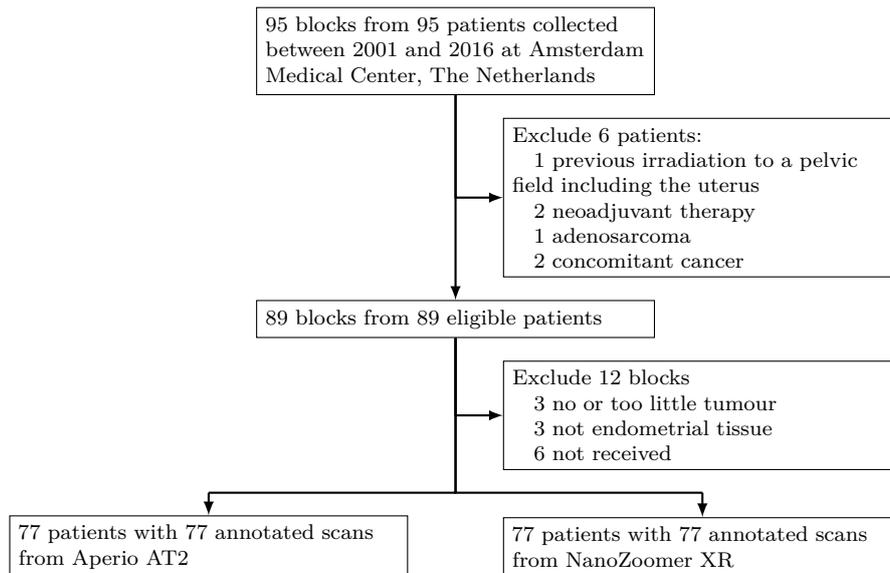

**Protocol Figure 9:** Flow from requested blocks to annotated scans for the VEN1 cohort

283 **1.2.3 VEn2 — Endometrial carcinoma**

284 177 blocks from 152 patients collected between 1999 and 2018 at Innsbruck Medical University,  
 285 Austria. 19 blocks were excluded for no or too little tumour in the received block. 6 blocks were  
 286 too thin to section. 14 patients had all blocks excluded for no or too little tumour, 4 patients had  
 287 all blocks excluded for too thin block, and one additional patient had one block excluded for both  
 288 reasons leaving no blocks left. This leaves 132 patients with 152 annotated scans from both the  
 289 Aperio AT2 and NanoZoomer XR scanner (see protocol figure 10).

290 Scans from the NanoZoomer XR scanner were manually annotated by a pathologist (MP) and  
 291 transferred to the corresponding Aperio AT2 scans.

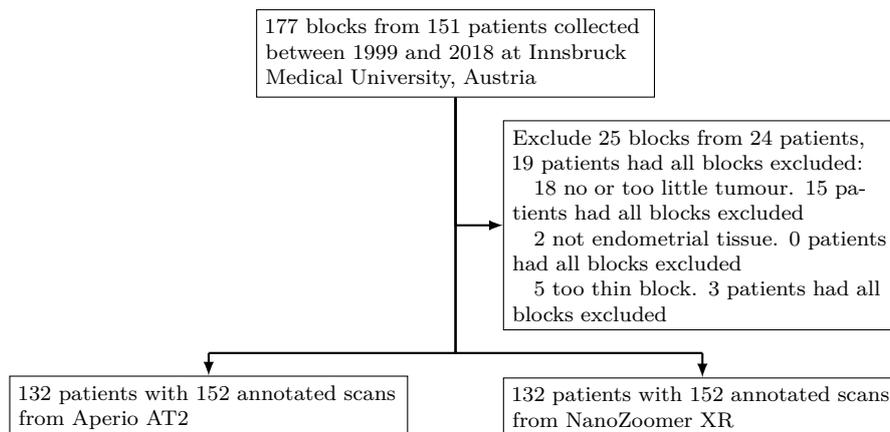

**Protocol Figure 10:** Flow from requested blocks to annotated scans for the VEN2 cohort

292 **1.2.4 VLu1 — Lung carcinoma**

293 A consecutive series of 633 patients with stage I to III non-small cell lung carcinoma (NSCLC)  
294 operated between 1990 and 2010 at the University Hospital of Northern Norway and Nordland  
295 Hospital, Norway.[16, 17] H&E stained tissue slides were received at ICGI for scanning, and after  
296 exclusions (see protocol figure 11) we had 522 eligible patients with 522 annotated scans from both  
297 the Aperio AT2 scanner and the NanoZoomer XR scanner.

298 NanoZoomer XR scans were manually annotated by a pathologist (MP), and they were auto-  
299 matically transferred to the corresponding Aperio AT2 scans. Large areas of fibrous tissue and  
300 necrosis were not annotated.

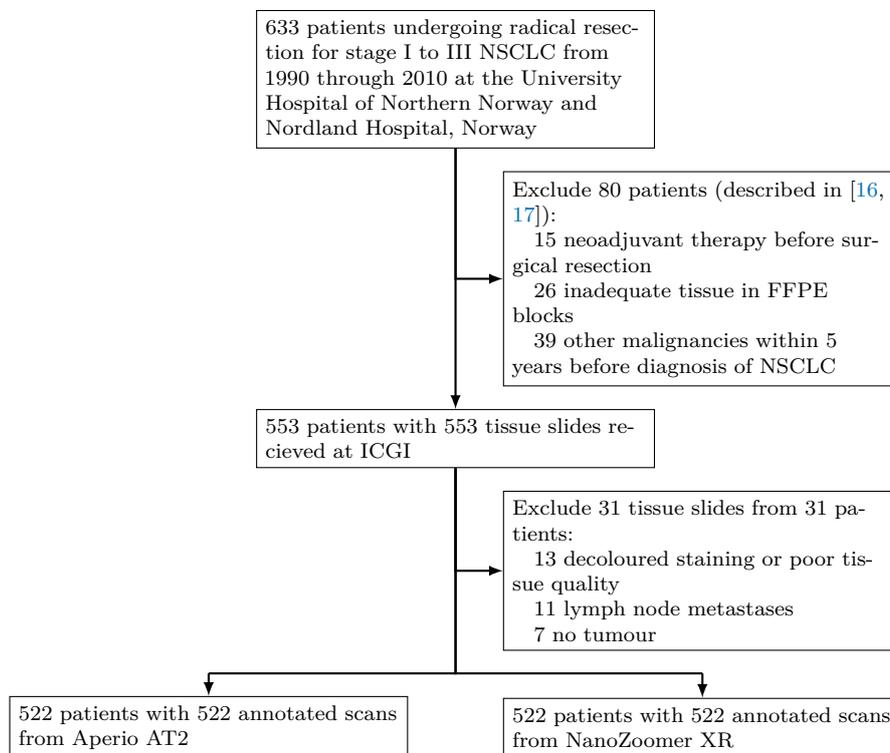

**Protocol Figure 11:** Flow from original study recruitment to annotated scans for the VLu1 cohort

301 **1.2.5 VPr1 — Prostate carcinoma**

302 The cohort comprised 287 patients who underwent RP between 2001 and 2006 at the Norwegian  
303 Radium Hospital (now a part of Oslo University Hospital), Norway. All patients were operated by  
304 one surgeon (Bjørn Brennhovd).[18]

305 After exclusions (see protocol figure 12), 259 eligible patients remained from which three blocks

306 were selected. The first and the second block represented the highest Gleason score and the largest  
307 tumour area, respectively. The third block was selected randomly from the remaining blocks with  
308 a tumour area  $> 5 \text{ mm}^2$  on a diagnostic H&E section.

309 We obtained three sections from all 259 eligible patients, resulting in 777 sections scanned on  
310 both the Aperio AT2 scanner and the NanoZoomer XR scanner.

311 The origin of the digital annotations are manual annotations made directly on the cover slip  
312 with a marker. These marked slides were scanned with a NanoZoomer HT (Hamamatsu Photonics,  
313 Japan) scanner. Digital annotations were generated on these scans by drawing inside the area  
314 delineated by the analog marker, this was done either manually or automatically. The resulting  
315 digital annotations were transferred to scans from the Aperio AT2 scanner before they were man-  
316 ually verified and potentially corrected by a pathologist (MP). Finally, the verified annotations  
317 were transferred to scans from the NanoZoomer XR scanner. Large areas of benign epithelium and  
318 stroma were not annotated.

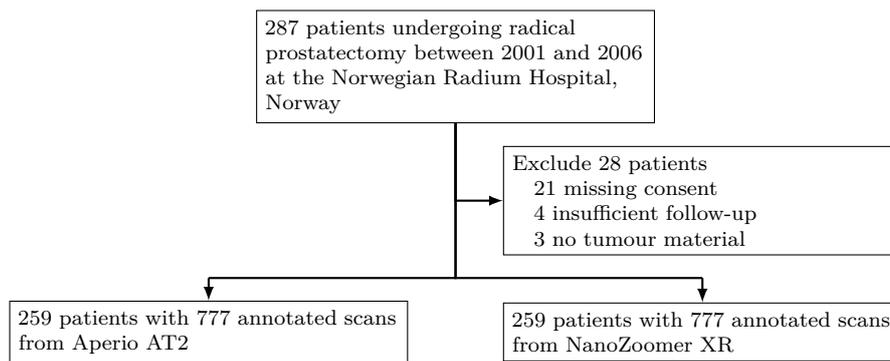

**Protocol Figure 12:** Flow from operated patients to annotated scans for the VPr1 cohort

### 319 1.2.6 VBr1 — Breast carcinoma

320 This cohort comprises 348 patients registered with breast cancer between 1990 and 1998 at Sta-  
321 vanger University Hospital, Norway.[19, 20, 21, 22] 320 H&E stained tissue sections prepared as  
322 slides from 320 patients were received at ICGI and scanned. After exclusions (see protocol fig-  
323 ure 13) we were left with 310 slides from 310 patients scanned on both the Aperio AT2 scanner  
324 and the NanoZoomer XR scanner.

325 Scans from the Aperio AT2 scanner were manually annotated by a pathologist (MP) and trans-  
326 ferred to the corresponding NanoZoomer XR scans. Both infiltrating tumour areas and intraductal  
327 carcinoma were annotated.

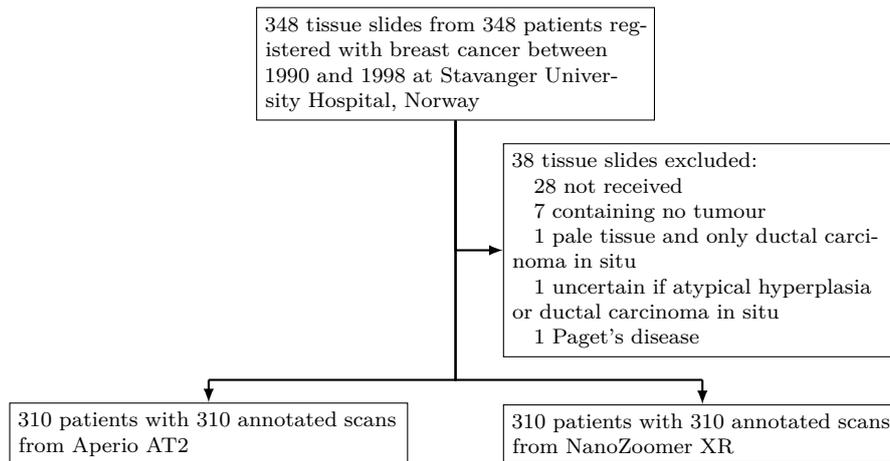

**Protocol Figure 13:** Flow from requested tissue slides to annotated scans for the VBr1 cohort

328 **1.2.7 VBr2 — Breast carcinoma**

329 This cohort comprises 339 patients registered with breast cancer between 2000 and 2004 at Sta-  
 330 vanger University Hospital, Norway.[23] 315 H&E stained tissue sections prepared as slides from  
 331 315 patients were received at ICGI and scanned. After exclusions (see protocol figure 14) we were  
 332 left with 304 slides from 304 patients scanned on both the Apero AT2 scanner and the NanoZoomer  
 333 XR scanner.

334 Scans from the Apero AT2 scanner were manually annotated by a pathologist (MP), and  
 335 annotations were transferred to the corresponding NanoZoomer XR scans. Both infiltrating tumour  
 336 areas and intraductal carcinoma were annotated.

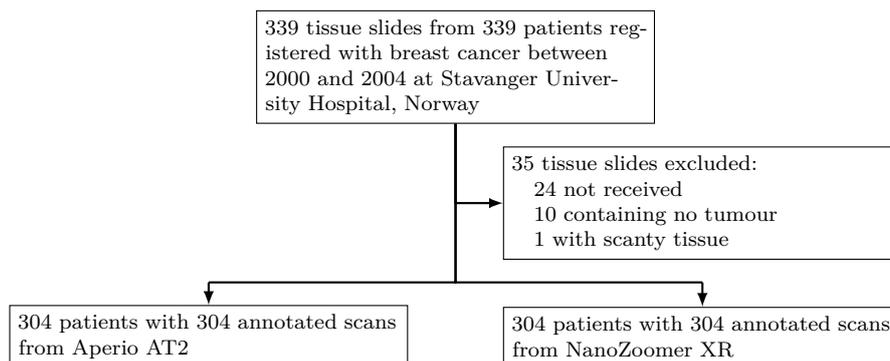

**Protocol Figure 14:** Flow from requested tissue slides to annotated scans for the VBr2 cohort

337 **1.2.8 VUr1 — Urothelial carcinoma**

338 357 patients diagnosed with urothelial carcinoma of the bladder between 1992 and 2010 at Stavanger  
339 University Hospital, Norway.[24, 25] From this, 333 slides from 333 patients were received at ICGI  
340 and scanned on the Aperio AT2 and the NanoZoomer XR scanner. 10 slides contained two parallel  
341 tissue sections, in which case only the best tissue section of the two parallels was scanned. One  
342 scan was excluded since it contained squamous epithelium and soft tissue but no tumour tissue,  
343 leaving us with 332 scans from 332 patients (see protocol figure 15).

344 All Aperio AT2 scans were manually annotated by a pathologist (MP), and the annotations  
345 were transferred to the NanoZoomer XR scanner. Urothelial tumours with or without infiltration  
346 were annotated.

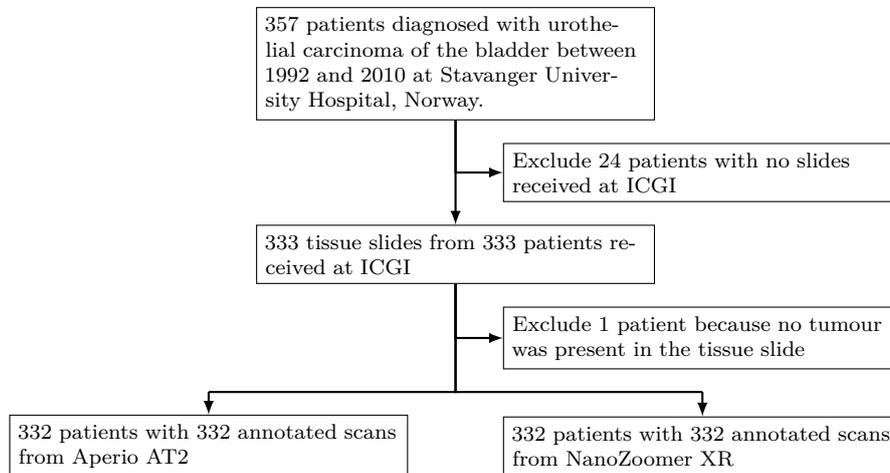

**Protocol Figure 15:** Flow from eligible patients to annotated scans for the VUr1 cohort

347 **1.3 Material analyses**

348 **1.3.1 Baseline characteristics**

349 Baseline characteristics for all cohorts grouped by cancer type are given in protocol tables 3 to 8.  
 350 Data are given as *median (interquartile range)* or *count (percentage)*. Time to *event* statistics are  
 351 based only on patients with the respective event. “Age” is age at a given starting point, which is  
 352 the same starting point as time to event durations and follow-up time durations starts from. This  
 353 starting point can vary between cohorts and will be specified.

**Protocol Table 3:** Baseline characteristics in colorectal carcinoma cohorts. Starting point is at randomisation for VCo1 and at surgery for the other cohorts.

|                               | DCo1            | DCo2            | DCo3            | VCo1            |
|-------------------------------|-----------------|-----------------|-----------------|-----------------|
| Patient count                 | 206             | 578             | 765             | 1132            |
| Age                           |                 |                 |                 |                 |
| Years                         | 71 (61 – 78)    | 73 (63 – 79)    | 64 (58 – 71)    | 65 (59 – 71)    |
| Missing                       | 2 (1%)          | 0               | 0               | 0               |
| Sex                           |                 |                 |                 |                 |
| Female                        | 106 (51%)       | 290 (50%)       | 270 (35%)       | 480 (42%)       |
| Male                          | 98 (48%)        | 288 (50%)       | 495 (65%)       | 652 (58%)       |
| Missing                       | 2 (1%)          | 0               | 0               | 0               |
| Cancer-specific death         |                 |                 |                 |                 |
| False                         | 144 (70%)       | 377 (65%)       | 645 (84%)       | 961 (85%)       |
| True                          | 60 (29%)        | 201 (35%)       | 120 (16%)       | 157 (14%)       |
| Missing                       | 2 (1%)          | 0               | 0               | 14 (1%)         |
| Time to cancer-specific death |                 |                 |                 |                 |
| Years                         | 0.7 (0.3 – 2.3) | 2.8 (1.7 – 5.1) | 3.0 (2.2 – 4.1) | 2.7 (1.7 – 3.6) |
| Follow-up time                |                 |                 |                 |                 |
| Years                         | 3.5 (1.0 – 5.0) | 6.6 (2.9 – 9.4) | 5.1 (4.1 – 5.8) | 4.6 (3.3 – 5.1) |
| Missing                       | 2 (1%)          | 0               | 0               | 0               |
| pT stage                      |                 |                 |                 |                 |
| pT1                           | 2 (1%)          | 27 (5%)         | 12 (2%)         | 18 (2%)         |
| pT2                           | 24 (12%)        | 103 (18%)       | 52 (7%)         | 71 (6%)         |
| pT3                           | 164 (80%)       | 414 (72%)       | 527 (69%)       | 588 (52%)       |
| pT4                           | 13 (6%)         | 34 (6%)         | 150 (20%)       | 404 (36%)       |
| Missing                       | 3 (1%)          | 0               | 24 (3%)         | 51 (5%)         |
| pN stage                      |                 |                 |                 |                 |
| pN0                           | 128 (62%)       | 388 (67%)       | 367 (48%)       | 406 (36%)       |
| pN1                           | 60 (29%)        | 152 (26%)       | 260 (34%)       | 515 (45%)       |
| pN2                           | 14 (7%)         | 37 (6%)         | 113 (15%)       | 185 (16%)       |
| Missing                       | 4 (2%)          | 1 (<1%)         | 25 (3%)         | 26 (2%)         |
| Stage                         |                 |                 |                 |                 |
| I                             | 8 (4%)          | 112 (19%)       | 0               | 0               |
| II                            | 99 (48%)        | 277 (48%)       | 379 (50%)       | 406 (36%)       |
| III                           | 52 (25%)        | 189 (33%)       | 386 (50%)       | 726 (64%)       |
| IV                            | 45 (22%)        | 0               | 0               | 0               |
| Missing                       | 2 (1%)          | 0               | 0               | 0               |
| Histological grade            |                 |                 |                 |                 |
| 1                             | 9 (4%)          | 58 (10%)        | 64 (8%)         | 46 (4%)         |
| 2                             | 173 (84%)       | 452 (78%)       | 608 (79%)       | 855 (76%)       |
| 3                             | 21 (10%)        | 63 (11%)        | 76 (10%)        | 173 (15%)       |
| Missing                       | 3 (1%)          | 5 (1%)          | 17 (2%)         | 58 (5%)         |

**Protocol Table 4:** Baseline characteristics in endometrial carcinoma cohorts. Starting point is at surgery.

|                                                        | DEn1             | VEn1            | VEn2            |
|--------------------------------------------------------|------------------|-----------------|-----------------|
| Patient count                                          | 1241             | 77              | 132             |
| Age                                                    |                  |                 |                 |
| Years                                                  | 68 (61 – 76)     | 67 (60 – 73)    | 68 (61 – 75)    |
| Missing                                                | 5 (<1%)          | 0               | 0               |
| Histological type                                      |                  |                 |                 |
| Adenosquamous carcinoma                                | 0                | 2 (3%)          | 0               |
| Carcinosarcoma                                         | 83 (7%)          | 17 (22%)        | 4 (3%)          |
| Clear cell carcinoma                                   | 35 (3%)          | 14 (18%)        | 4 (3%)          |
| Endometrioid carcinoma                                 | 825 (66%)        | 11 (14%)        | 98 (74%)        |
| Mucinous carcinoma                                     | 7 (1%)           | 0               | 0               |
| Neuroendocrine carcinoma                               | 11 (1%)          | 0               | 0               |
| Papillary serous carcinoma                             | 133 (11%)        | 31 (40%)        | 24 (18%)        |
| Squamous cell carcinoma                                | 0                | 2 (3%)          | 0               |
| Mixed with clear cell or papillary serous carcinoma    | 67 (5%)          | 0               | 0               |
| Mixed without clear cell or papillary serous carcinoma | 53 (4%)          | 0               | 0               |
| Undifferentiated carcinoma                             | 14 (1%)          | 0               | 2 (2%)          |
| Unclassifiable                                         | 9 (1%)           | 0               | 0               |
| Missing                                                | 4 (<1%)          | 0               | 0               |
| Cancer-specific death                                  |                  |                 |                 |
| False                                                  | 974 (78%)        | 56 (73%)        | 115 (87%)       |
| True                                                   | 263 (21%)        | 21 (27%)        | 17 (13%)        |
| Missing                                                | 4 (<1%)          | 0               | 0               |
| Time to cancer-specific death                          |                  |                 |                 |
| Years                                                  | 2.5 (1.4 – 4.2)  | 1.9 (1.3 – 3.4) | 3.7 (2.7 – 5.8) |
| Overall death                                          |                  |                 |                 |
| False                                                  | 756 (61%)        | 41 (53%)        | 94 (71%)        |
| True                                                   | 481 (39%)        | 36 (47%)        | 38 (29%)        |
| Missing                                                | 4 (<1%)          | 0               | 0               |
| Time to overall death                                  |                  |                 |                 |
| Years                                                  | 3.7 (1.8 – 6.7)  | 2.0 (1.3 – 3.4) | 5.0 (2.7 – 8.3) |
| Recurrence                                             |                  |                 |                 |
| False                                                  | 896 (72%)        | 54 (70%)        | 105 (80%)       |
| True                                                   | 341 (27%)        | 23 (30%)        | 27 (20%)        |
| Missing                                                | 4 (<1%)          | 0               | 0               |
| Time to recurrence                                     |                  |                 |                 |
| Years                                                  | 1.3 (0.7 – 2.4)  | 1.2 (1.0 – 1.5) | 1.2 (0.8 – 2.6) |
| Follow-up time                                         |                  |                 |                 |
| Years                                                  | 7.6 (5.0 – 11.8) | 3.6 (2.5 – 4.7) | 4.5 (2.0 – 8.4) |
| Missing                                                | 4 (<1%)          | 0               | 0               |
| FIGO stage                                             |                  |                 |                 |
| 1a                                                     | 548 (44%)        | 20 (26%)        | 48 (36%)        |
| 1b                                                     | 296 (24%)        | 12 (16%)        | 32 (24%)        |
| 2                                                      | 79 (6%)          | 14 (18%)        | 19 (14%)        |
| 3                                                      | 0                | 0               | 8 (6%)          |
| 3a                                                     | 28 (2%)          | 1 (1%)          | 0               |
| 3b                                                     | 12 (1%)          | 0               | 0               |
| 3c1                                                    | 106 (9%)         | 18 (23%)        | 15 (11%)        |
| 3c2                                                    | 72 (6%)          | 8 (10%)         | 9 (7%)          |
| 4                                                      | 0                | 0               | 1 (1%)          |
| 4a                                                     | 0                | 1 (1%)          | 0               |
| 4b                                                     | 96 (8%)          | 3 (4%)          | 0               |
| Missing                                                | 4 (<1%)          | 0               | 0               |
| Histological grade                                     |                  |                 |                 |
| 1                                                      | 467 (38%)        | 0               | 26 (20%)        |
| 2                                                      | 286 (23%)        | 1 (1%)          | 64 (48%)        |
| 3                                                      | 179 (14%)        | 75 (97%)        | 42 (32%)        |
| Missing                                                | 309 (25%)        | 1 (1%)          | 0               |

**Protocol Table 5:** Baseline characteristics in lung carcinoma cohorts. Starting point is at surgery for DLu1 and at diagnosis for VLu1.

|                                     | DLu1            | VLu1            |
|-------------------------------------|-----------------|-----------------|
| Patient count                       | 933             | 522             |
| Age                                 |                 |                 |
| Years                               | 68 (62 – 73)    | 68 (60 – 73)    |
| Missing                             | 11 (1%)         | 0               |
| Sex                                 |                 |                 |
| Female                              | 460 (49%)       | 168 (32%)       |
| Male                                | 462 (50%)       | 354 (68%)       |
| Missing                             | 11 (1%)         | 0               |
| Histological type                   |                 |                 |
| Adenocarcinoma                      | 521 (56%)       | 226 (43%)       |
| Adenosquamous carcinoma             | 16 (2%)         | 3 (1%)          |
| Bronchioloalveolar carcinoma        | 8 (1%)          | 0               |
| Carcinoid                           | 42 (5%)         | 0               |
| Large cell carcinoma                | 29 (3%)         | 0               |
| Large cell neuroendocrine carcinoma | 6 (1%)          | 0               |
| Salivary gland type lung carcinoma  | 5 (1%)          | 0               |
| Squamous cell carcinoma             | 287 (31%)       | 289 (55%)       |
| Undifferentiated carcinoma          | 4 (<1%)         | 3 (1%)          |
| Mixed                               | 2 (<1%)         | 0               |
| Other                               | 2 (<1%)         | 1 (<1%)         |
| Missing                             | 11 (1%)         | 0               |
| Cancer-specific death               |                 |                 |
| False                               | 635 (68%)       | 316 (61%)       |
| True                                | 287 (31%)       | 206 (39%)       |
| Missing                             | 11 (1%)         | 0               |
| Time to cancer-specific death       |                 |                 |
| Years                               | 2.2 (1.2 – 3.7) | 1.7 (0.9 – 3.2) |
| Follow-up time                      |                 |                 |
| Years                               | 4.6 (2.5 – 6.8) | 3.6 (1.4 – 7.4) |
| Missing                             | 11 (1%)         | 0               |
| pT stage                            |                 |                 |
| pT1                                 | 323 (35%)       | 171 (33%)       |
| pT2                                 | 433 (46%)       | 196 (38%)       |
| pT3                                 | 137 (15%)       | 98 (19%)        |
| pT4                                 | 29 (3%)         | 57 (11%)        |
| Missing                             | 11 (1%)         | 0               |
| pN stage                            |                 |                 |
| pN0                                 | 671 (72%)       | 366 (70%)       |
| pN1                                 | 184 (20%)       | 102 (20%)       |
| pN2                                 | 67 (7%)         | 54 (10%)        |
| Missing                             | 11 (1%)         | 0               |
| Stage                               |                 |                 |
| I                                   | 507 (54%)       | 224 (43%)       |
| II                                  | 273 (29%)       | 170 (33%)       |
| III                                 | 132 (14%)       | 128 (25%)       |
| IV                                  | 10 (1%)         | 0               |
| Missing                             | 11 (1%)         | 0               |

**Protocol Table 6:** Baseline characteristics in prostate carcinoma cohorts. Starting point is at surgery.

|                                | DPr1              | DPr2              | VPr1             |
|--------------------------------|-------------------|-------------------|------------------|
| Patient count                  | 328               | 254               | 259              |
| Age                            |                   |                   |                  |
| Years                          | 64 (61 – 68)      | 62 (58 – 67)      | 62 (59 – 66)     |
| Missing                        | 0                 | 1 (<1%)           | 0                |
| Overall death                  |                   |                   |                  |
| False                          | 257 (78%)         | 176 (69%)         | 200 (77%)        |
| True                           | 71 (22%)          | 77 (30%)          | 59 (23%)         |
| Missing                        | 0                 | 1 (<1%)           | 0                |
| Time to overall death          |                   |                   |                  |
| Years                          | 8.6 (6.3 – 12.3)  | 9.6 (5.7 – 12.8)  | 9.8 (7.2 – 13.5) |
| Biochemical recurrence         |                   |                   |                  |
| False                          | 215 (66%)         | 98 (39%)          | 188 (73%)        |
| True                           | 113 (34%)         | 155 (61%)         | 71 (27%)         |
| Missing                        | 0                 | 1 (<1%)           | 0                |
| Time to biochemical recurrence |                   |                   |                  |
| Years                          | 0.8 (0.0 – 3.9)   | 2.9 (1.5 – 5.3)   | 3.4 (1.2 – 5.6)  |
| Follow-up time                 |                   |                   |                  |
| Years                          | 11.0 (8.8 – 13.9) | 11.2 (7.7 – 14.4) | 9.6 (8.5 – 12.3) |
| Missing                        | 0                 | 1 (<1%)           | 0                |
| pT stage                       |                   |                   |                  |
| pT2                            | 178 (54%)         | 54 (21%)          | 159 (61%)        |
| pT3                            | 136 (41%)         | 168 (66%)         | 96 (37%)         |
| pT4                            | 0                 | 26 (10%)          | 2 (1%)           |
| pTx                            | 14 (4%)           | 4 (2%)            | 0                |
| Missing                        | 0                 | 2 (1%)            | 2 (1%)           |
| Gleason grade                  |                   |                   |                  |
| 2+3                            | 0                 | 0                 | 3 (1%)           |
| 3+3                            | 63 (19%)          | 11 (4%)           | 126 (49%)        |
| 3+4                            | 147 (45%)         | 92 (36%)          | 83 (32%)         |
| 3+5                            | 1 (<1%)           | 3 (1%)            | 0                |
| 4+3                            | 88 (27%)          | 77 (30%)          | 25 (10%)         |
| 4+4                            | 13 (4%)           | 41 (16%)          | 15 (6%)          |
| 4+5                            | 4 (1%)            | 26 (10%)          | 1 (<1%)          |
| 5+4                            | 1 (<1%)           | 3 (1%)            | 2 (1%)           |
| 5+5                            | 0                 | 0                 | 1 (<1%)          |
| Missing                        | 11 (3%)           | 1 (<1%)           | 3 (1%)           |

**Protocol Table 7:** Baseline characteristics in breast carcinoma cohorts. Starting point is at diagnosis.

|                                   | VBr1              | VBr2              |
|-----------------------------------|-------------------|-------------------|
| Patient count                     | 310               | 304               |
| Age                               |                   |                   |
| Years                             | 56 (50 – 64)      | 57 (47 – 64)      |
| Histological Type                 |                   |                   |
| Invasive ductal carcinoma         | 235 (76%)         | 284 (93%)         |
| Invasive lobular carcinoma        | 20 (6%)           | 6 (2%)            |
| Lobular carcinoma in situ         | 24 (8%)           | 0                 |
| Medullary carcinoma               | 5 (2%)            | 8 (3%)            |
| Tubular carcinoma                 | 12 (4%)           | 0                 |
| Other                             | 13 (4%)           | 6 (2%)            |
| Missing                           | 1 (<1%)           | 0                 |
| Distant metastases                |                   |                   |
| False                             | 255 (82%)         | 220 (72%)         |
| True                              | 55 (18%)          | 74 (24%)          |
| Missing                           | 0                 | 10 (3%)           |
| Time to distant metastases        |                   |                   |
| Years                             | 5.3 (2.6 – 11.7)  | 1.5 (0.7 – 3.3)   |
| Local recurrence                  |                   |                   |
| False                             | 279 (90%)         | 274 (90%)         |
| True                              | 31 (10%)          | 20 (7%)           |
| Missing                           | 0                 | 10 (3%)           |
| Time to local recurrence          |                   |                   |
| Years                             | 9.3 (4.3 – 16.5)  | 8.3 (2.8 – 13.3)  |
| Follow-up time distant metastases |                   |                   |
| Years                             | 14.9 (8.4 – 21.2) | 12.4 (4.0 – 15.2) |
| Missing                           | 0                 | 10 (3%)           |
| Follow-up time local recurrence   |                   |                   |
| Years                             | 13.3 (6.2 – 21.0) | 11.9 (3.8 – 15.1) |
| Missing                           | 0                 | 11 (4%)           |
| Oestrogen recetor (ER)            |                   |                   |
| Negative                          | 40 (13%)          | 153 (50%)         |
| Borderline                        | 11 (4%)           | 0                 |
| Positive                          | 258 (83%)         | 146 (48%)         |
| Missing                           | 1 (<1%)           | 5 (2%)            |
| Progesterone receptor (PR)        |                   |                   |
| Negative                          | 60 (19%)          | 166 (55%)         |
| Borderline                        | 55 (18%)          | 2 (1%)            |
| Positive                          | 194 (63%)         | 98 (32%)          |
| Missing                           | 1 (<1%)           | 38 (12%)          |
| Lymph node status                 |                   |                   |
| Negative                          | 310 (100%)        | 216 (71%)         |
| Positive                          | 0                 | 53 (17%)          |
| Missing                           | 0                 | 35 (12%)          |
| Nottingham prognostic index       |                   |                   |
| 3–5                               | 109 (35%)         | 39 (13%)          |
| 6–7                               | 134 (43%)         | 115 (38%)         |
| 8–9                               | 64 (21%)          | 134 (44%)         |
| Missing                           | 3 (1%)            | 16 (5%)           |

**Protocol Table 8:** Baseline characteristics in urothelial carcinoma cohort. Starting point is at diagnosis.

|                             | VUr1             |
|-----------------------------|------------------|
| Patient count               | 332              |
| Age                         |                  |
| Years                       | 72 (62 – 80)     |
| Missing                     | 2 (1%)           |
| Sex                         |                  |
| Female                      | 84 (25%)         |
| Male                        | 248 (75%)        |
| Recurrence                  |                  |
| False                       | 173 (52%)        |
| True                        | 159 (48%)        |
| Time to recurrence          |                  |
| Years                       | 1.2 (0.6 – 2.0)  |
| Stage progression           |                  |
| False                       | 307 (92%)        |
| True                        | 25 (8%)          |
| Time to stage progression   |                  |
| Years                       | 2.0 (0.7 – 3.0)  |
| Follow-up recurrence        |                  |
| Years                       | 5.8 (2.6 – 8.2)  |
| Follow-up stage progression |                  |
| Years                       | 7.2 (4.4 – 10.1) |
| pT stage                    |                  |
| pTa                         | 255 (77%)        |
| pTis                        | 1 (<1%)          |
| pT1                         | 76 (23%)         |
| Histological grade          |                  |
| 1                           | 65 (20%)         |
| 2                           | 155 (47%)        |
| 3                           | 111 (33%)        |
| Missing                     | 1 (<1%)          |
| Metastasis                  |                  |
| False                       | 321 (97%)        |
| True                        | 11 (3%)          |
| Multifocal                  |                  |
| False                       | 197 (59%)        |
| True                        | 107 (32%)        |
| Missing                     | 28 (8%)          |

354 1.3.2 Survival characteristics

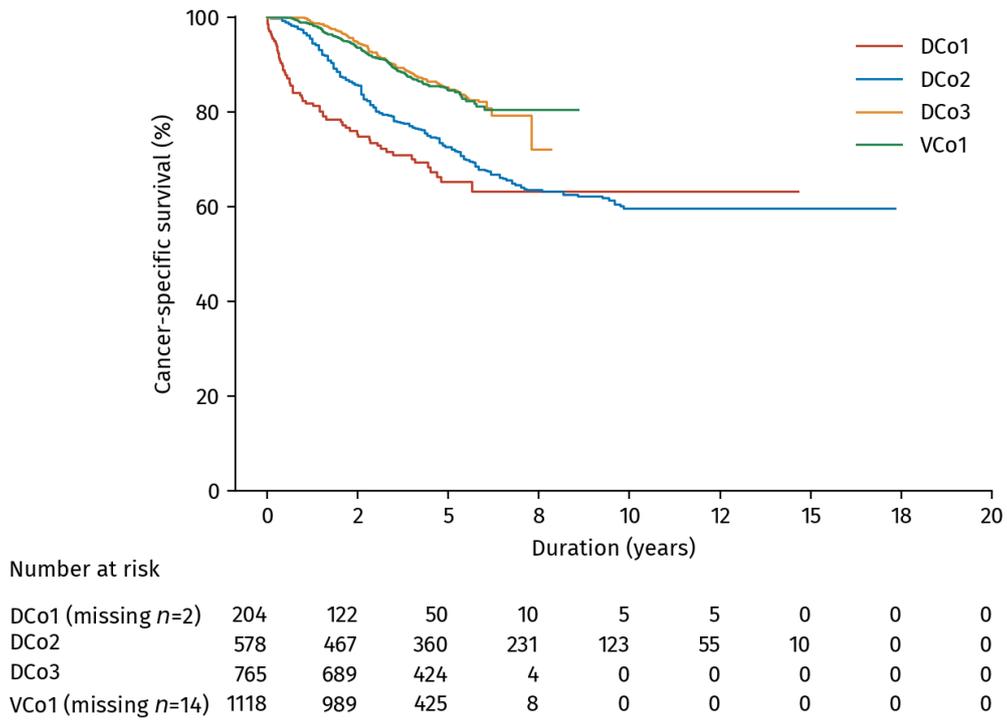

**Protocol Figure 16:** Kaplan-Meier analysis of survival in colorectal carcinoma materials. Duration is years since randomisation for VCo1 and years since surgery for the other cohorts.

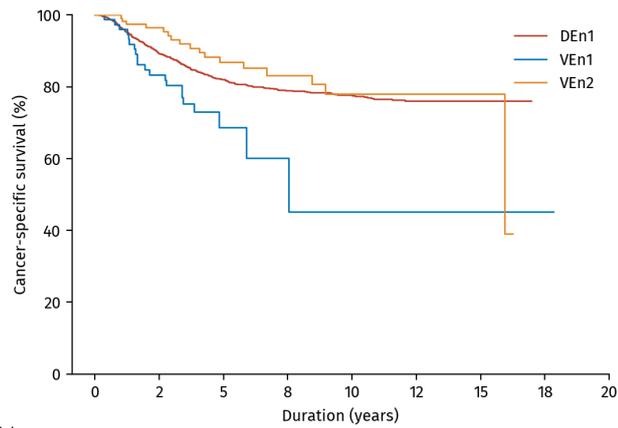

(a) Cancer-specific survival

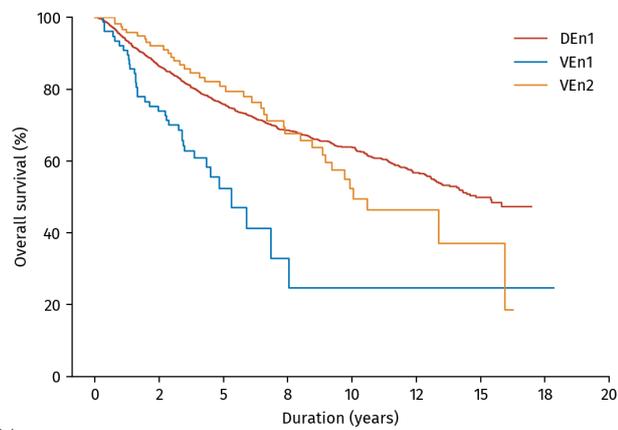

(b) Overall survival

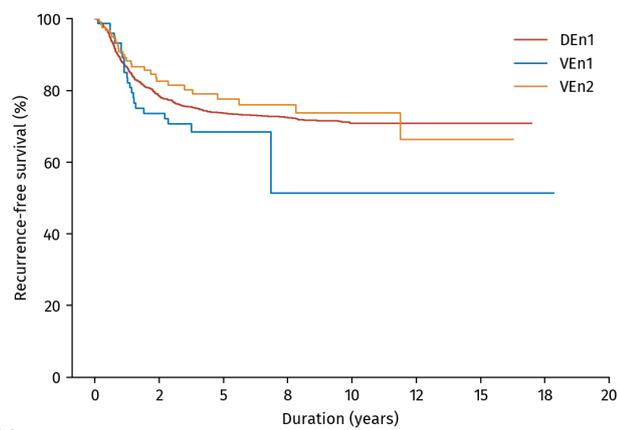

(c) Recurrence-free survival

**Protocol Figure 17:** Kaplan-Meier analysis of survival in endometrial carcinoma materials. Duration is years since surgery.

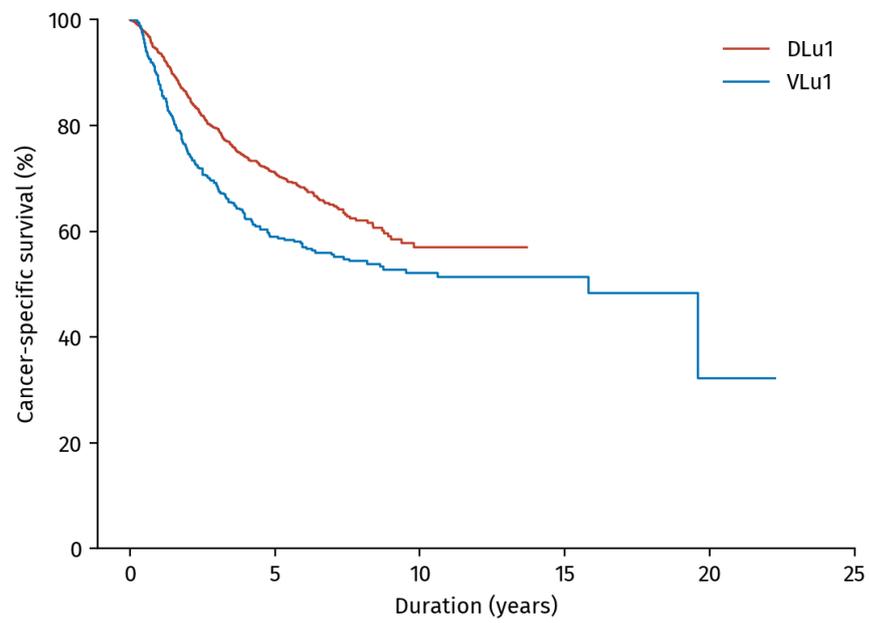

Number at risk

|                        |     |     |    |    |   |   |
|------------------------|-----|-----|----|----|---|---|
| DLu1 (missing $n=11$ ) | 922 | 424 | 60 | 0  | 0 | 0 |
| VLu1                   | 522 | 202 | 76 | 22 | 2 | 0 |

**Protocol Figure 18:** Kaplan-Meier analysis of survival in lung carcinoma materials. Duration is years since surgery for DLU1 and years since diagnosis for VLU1.

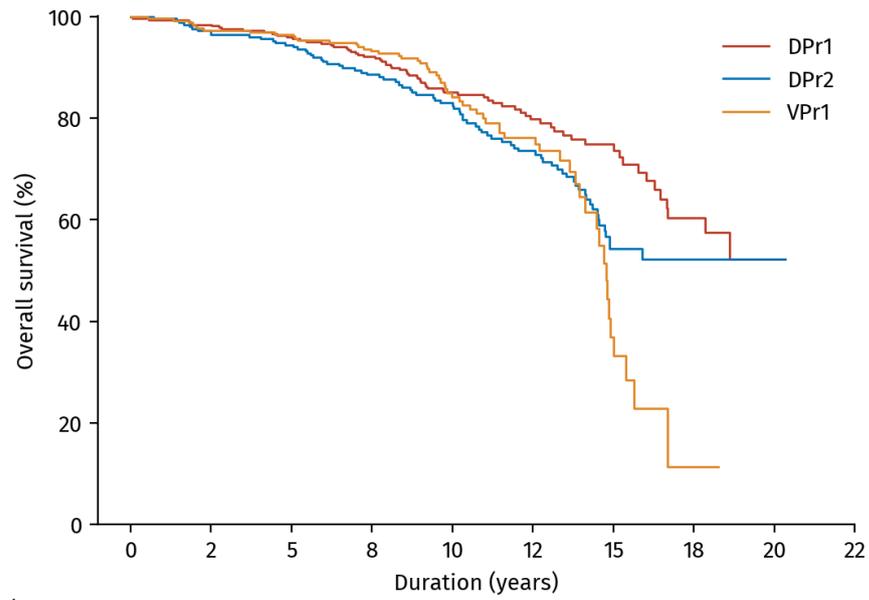

Number at risk

|                       |     |     |     |     |     |     |    |    |   |   |
|-----------------------|-----|-----|-----|-----|-----|-----|----|----|---|---|
| DPr1                  | 328 | 319 | 307 | 286 | 195 | 115 | 61 | 26 | 2 | 0 |
| DPr2 (missing $n=1$ ) | 253 | 244 | 233 | 192 | 150 | 108 | 45 | 12 | 1 | 0 |
| VPr1                  | 259 | 249 | 242 | 224 | 113 | 64  | 10 | 1  | 0 | 0 |

(a) Overall survival

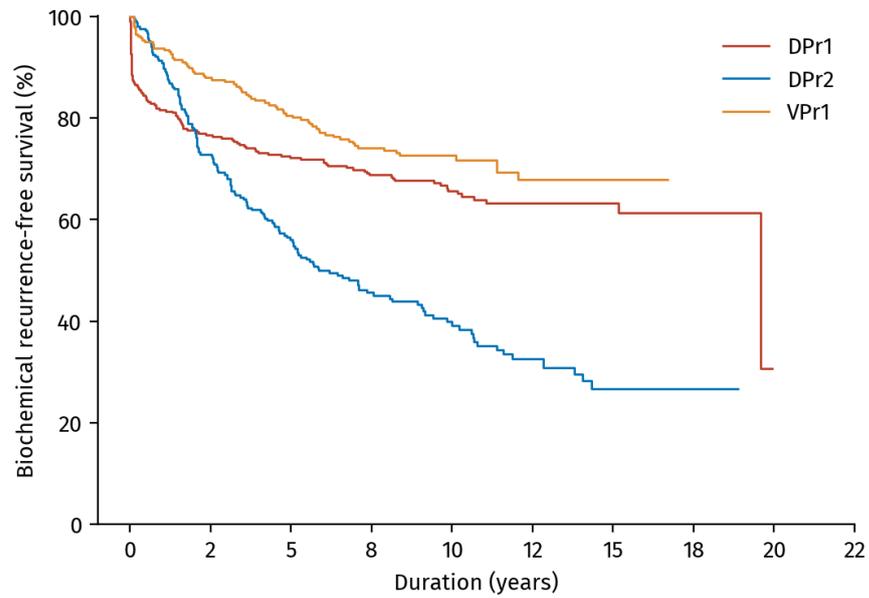

Number at risk

|                       |     |     |     |     |     |    |    |    |   |   |
|-----------------------|-----|-----|-----|-----|-----|----|----|----|---|---|
| DPr1                  | 328 | 245 | 220 | 195 | 119 | 69 | 37 | 14 | 0 | 0 |
| DPr2 (missing $n=1$ ) | 253 | 180 | 131 | 85  | 54  | 37 | 13 | 4  | 0 | 0 |
| VPr1                  | 259 | 218 | 193 | 165 | 80  | 40 | 4  | 0  | 0 | 0 |

(b) Biochemical recurrence-free survival

**Protocol Figure 19:** Kaplan-Meier analysis of survival in prostate carcinoma materials. Duration is years since surgery.

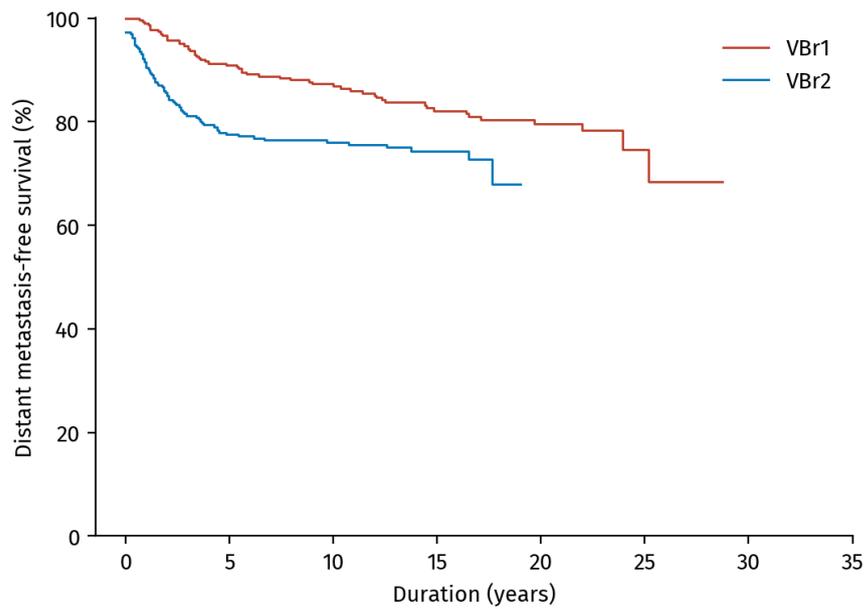

Number at risk

|                        |     |     |     |     |    |    |   |   |
|------------------------|-----|-----|-----|-----|----|----|---|---|
| VBr1                   | 310 | 261 | 206 | 154 | 94 | 14 | 0 | 0 |
| VBr2 (missing $n=10$ ) | 294 | 212 | 174 | 82  | 0  | 0  | 0 | 0 |

(a) Distant metastases-free survival

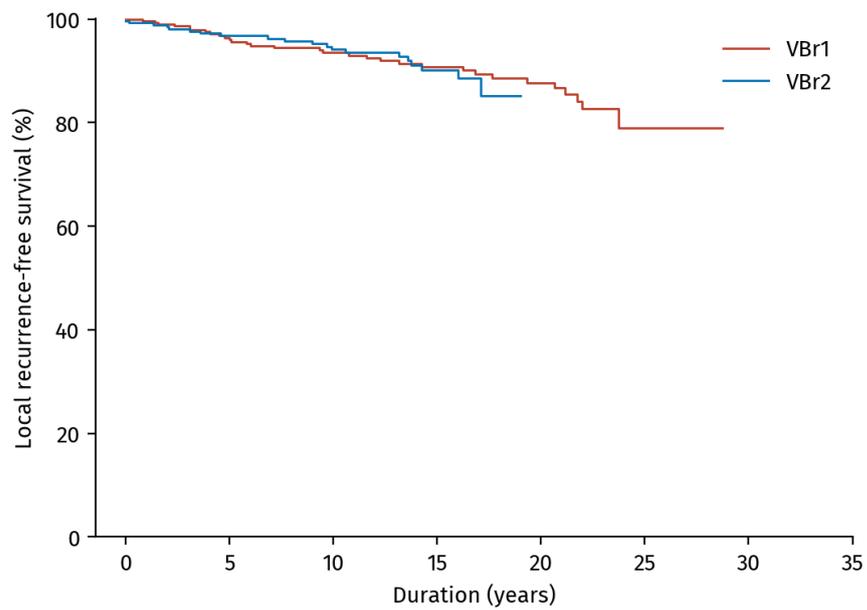

Number at risk

|                        |     |     |     |     |    |    |   |   |
|------------------------|-----|-----|-----|-----|----|----|---|---|
| VBr1                   | 310 | 252 | 195 | 144 | 89 | 13 | 0 | 0 |
| VBr2 (missing $n=11$ ) | 293 | 207 | 169 | 77  | 0  | 0  | 0 | 0 |

(b) Local recurrence-free survival

**Protocol Figure 20:** Kaplan-Meier analysis of survival in breast carcinoma materials. Duration is years since diagnosis. Note different follow-up times between the different event types.

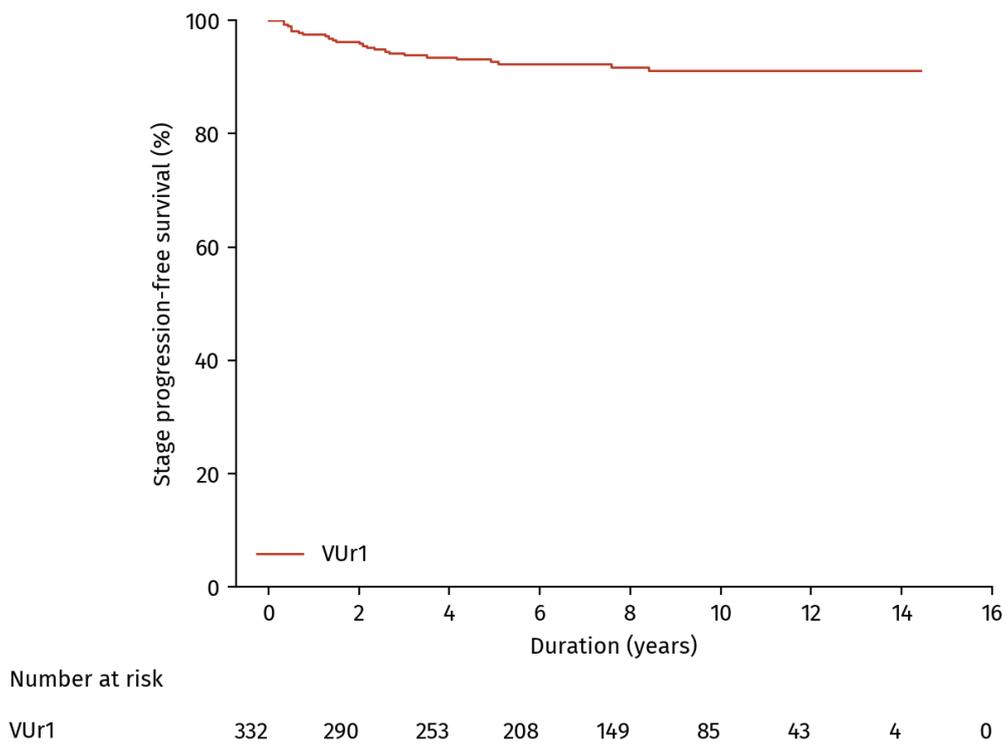

(a) Stage progression-free survival

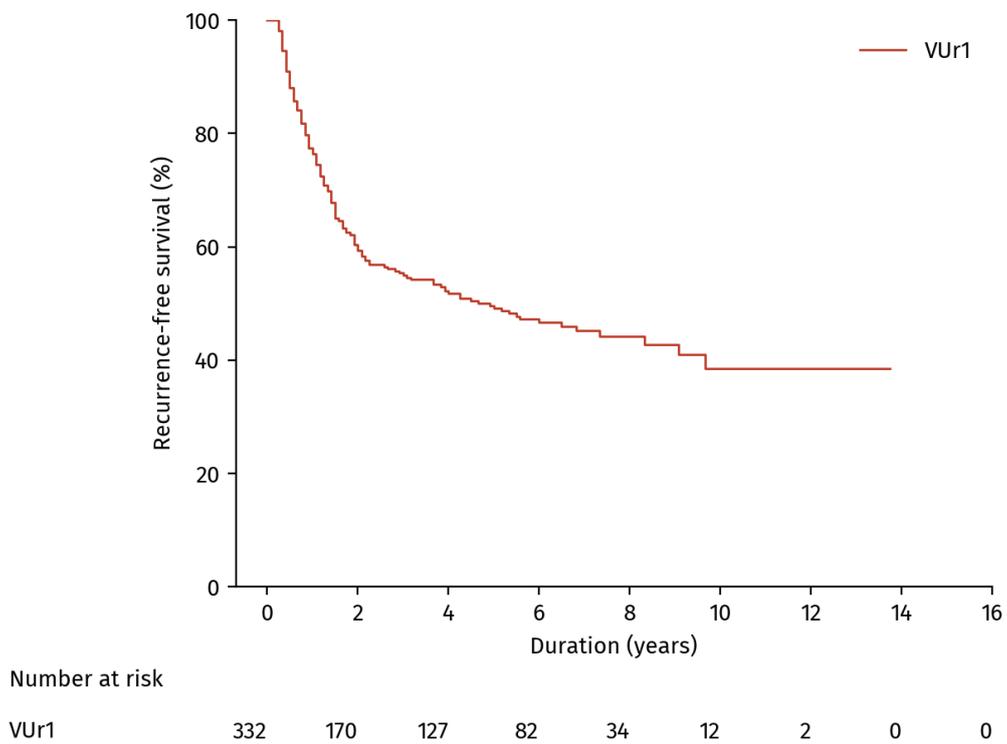

(b) Recurrence-free survival

**Protocol Figure 21:** Kaplan-Meier analysis of survival in urothelial carcinoma material. Duration is years since diagnosis. Note different follow-up times between the event types.

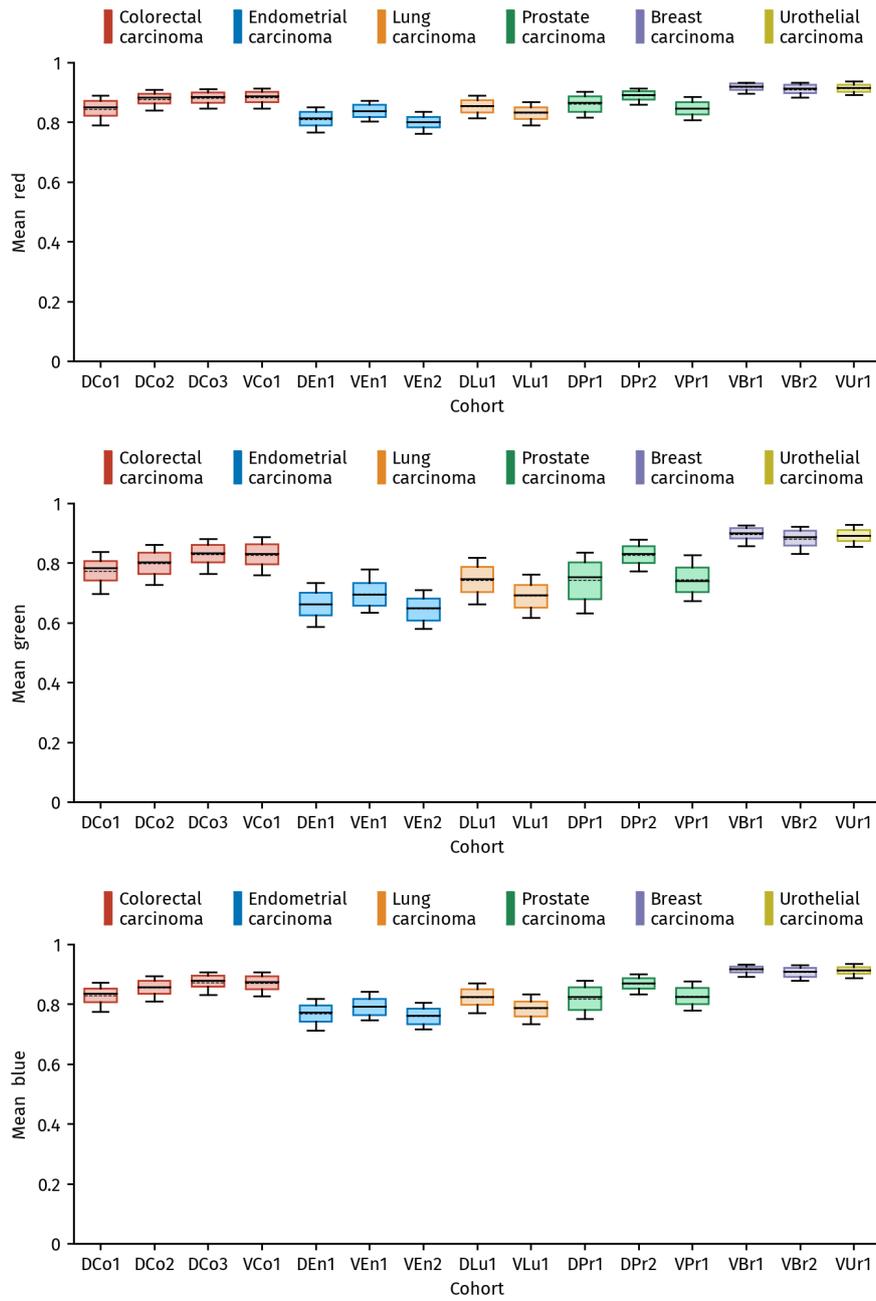

**Protocol Figure 22:** Colour channel mean value in full Aperio AT2 scans downsampled to 5  $\mu\text{m}$  per pixel

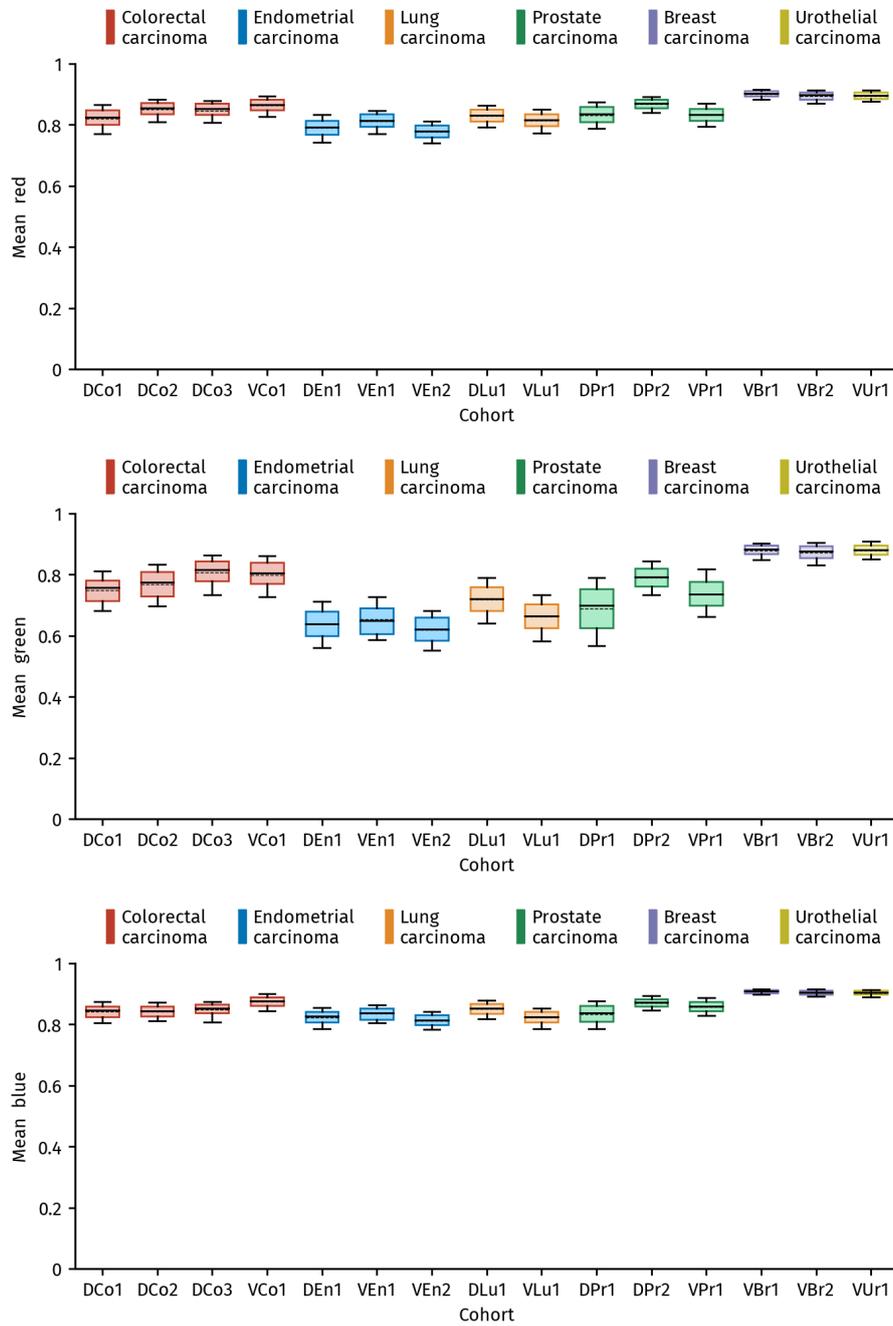

**Protocol Figure 23:** Colour channel mean value in full NanoZoomer XR scans downsampled to 5  $\mu\text{m}$  per pixel

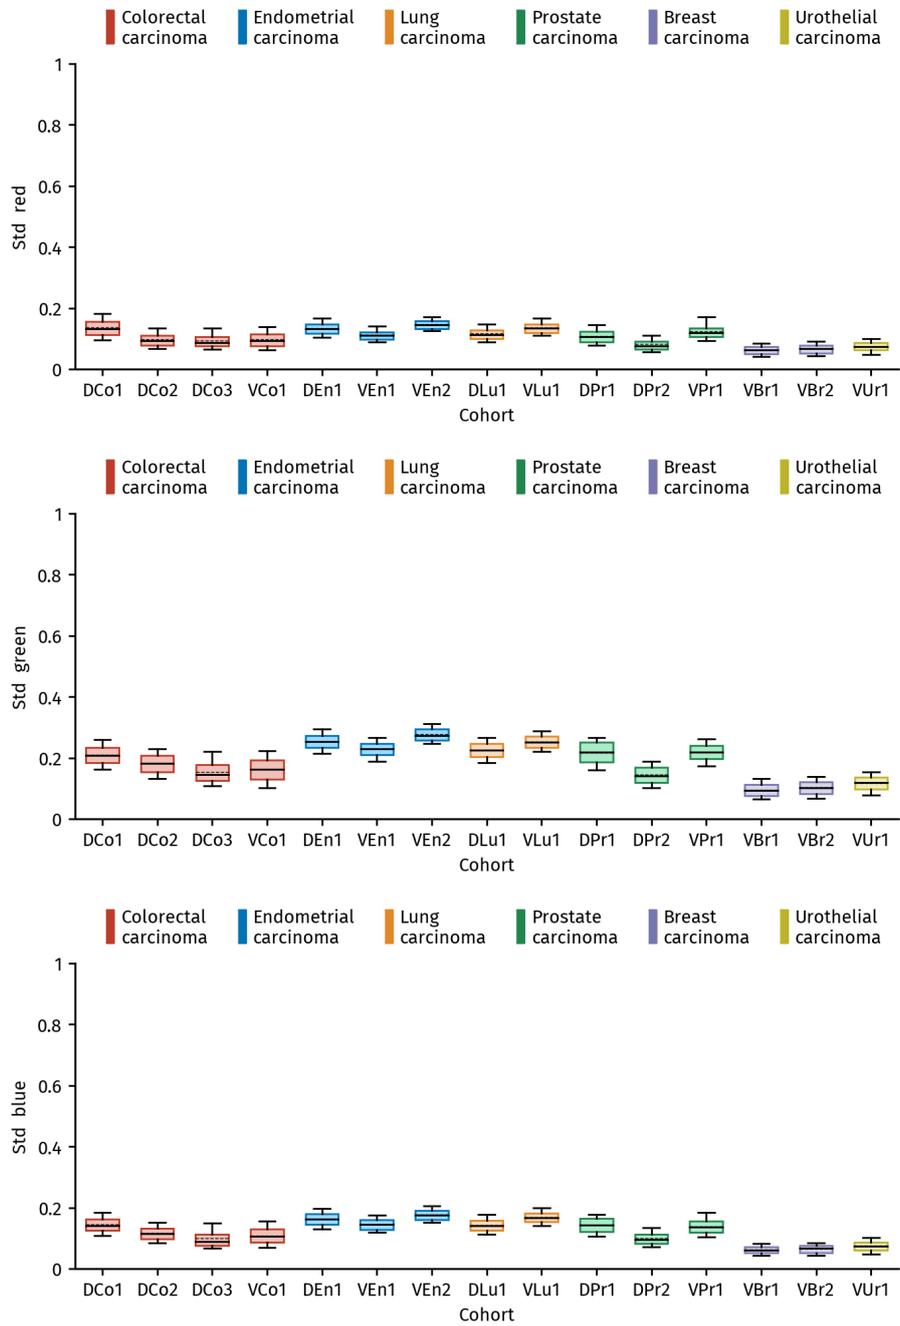

**Protocol Figure 24:** Colour channel standard deviation in full Aperio AT2 scans downscaled to 5  $\mu\text{m}$  per pixel

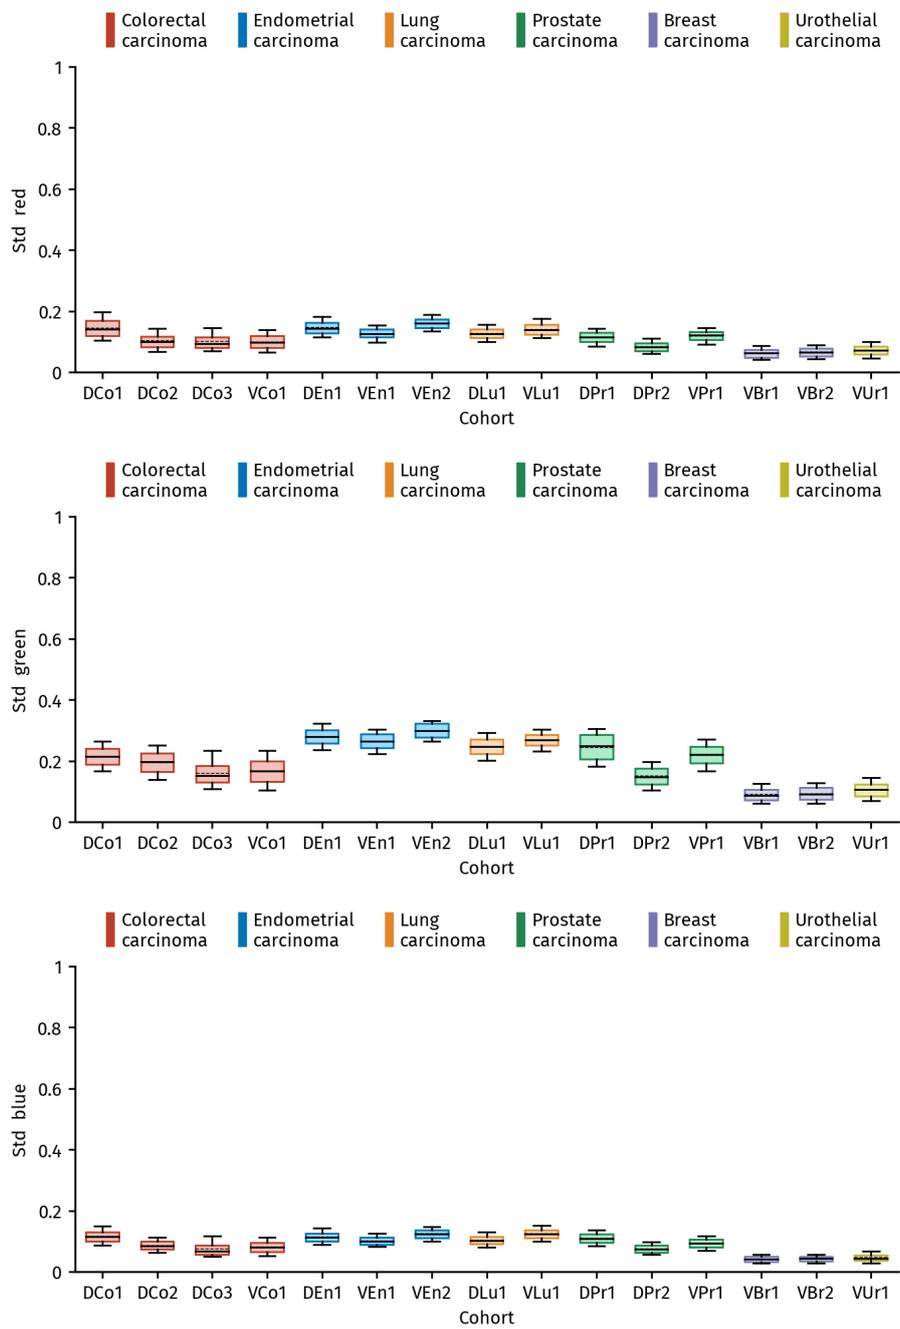

**Protocol Figure 25:** Colour channel standard deviation in full NanoZoomer XR scans downsampled to 5  $\mu\text{m}$  per pixel

## 356 2 Methods

357 This section give a detailed explanation of how the segmentation method was developed and how it  
358 is applied. The software and hardware development environment is described in section 2.1. Steps  
359 necessary for preparing the method are described in section 2.2 while the segmentation method  
360 itself is described in section 2.3. How we evaluate the performance of the segmentation result is  
361 explained in section 2.4.

### 362 2.1 Programming environment

363 Most programs used in this project are implemented in the *Python* programming language. For  
364 method validation, programs were run in a *Docker container* based on the  
365 `pytorch/pytorch:1.11.0-cuda11.3-cudnn8-runtime` image. The network optimisation was run  
366 in a Docker container based on the image `nvcr.io/nvidia/pytorch:22.02-py3`. Additional  
367 python packages used are listed in protocol table 9.

**Protocol Table 9:** Python packages and their versions

| Package                                  | Version  |
|------------------------------------------|----------|
| <code>alumentations</code>               | 1.1.0    |
| <code>matplotlib</code>                  | 3.5.1    |
| <code>opencv_python_headless</code>      | 4.5.5.64 |
| <code>openslide_python</code>            | 1.1.2    |
| <code>pandas</code>                      | 1.4.1    |
| <code>segmentation_models_pytorch</code> | 0.2.1    |
| <code>scikit-image</code>                | 0.19.2   |
| <code>timm</code>                        | 0.4.12   |
| <code>toml</code>                        | 0.10.2   |
| <code>torchinfo</code>                   | 1.6.3    |

368 Segmentation network processing was done on graphical processing units (GPUs). We used an  
369 Nvidia DGX machine with 8 A100 40 GB SXM GPUs, driver version 470.57.02 and CUDA version  
370 11.4 for the network optimisation. For the validation, we used computers with Nvidia Titan RTX  
371 24 GB GPU cards with driver version 465.19.01 and CUDA version 11.3.

### 372 2.2 Method development

373 The segmentation method use a convolutional neural network which needs to be optimised to this  
374 particular task of tumour segmentation. All necessary steps needed for preparation are described  
375 in this section and are summarised next:

- 376 1. Read input scans and downsample them to resolution 1  $\mu\text{m}$  per pixel (section 2.2.1)
- 377 2. Partition each scan into tiles with  $2048 \times 2048$  pixels (section 2.2.2)
- 378 3. Balance the development dataset (section 2.2.3)
- 379 4. Exclude background tiles (section 2.2.5)
- 380 5. Augment the development dataset (section 2.2.6)
- 381 6. Standardise input images (section 2.2.7)
- 382 7. Optimise the segmentation network (section 2.2.8)

### 383 2.2.1 Downsampling

384 Each scan used in this study is downsampled to a target resolution of 1  $\mu\text{m}$  per pixel (MPP). For  
385 reference, the highest resolution of many scans is labelled 40 $\times$  magnification which corresponds to  
386 about 0.25 MPP depending on the scanner vendor and model. As an example, we have scans from  
387 Aperio AT2 with a 40 $\times$  magnification with resolution 0.2530 MPP and scans from NanoZoomer  
388 XR with a 40 $\times$  magnification with resolution 0.2267 MPP (rounded to four decimal places).

389 The target downsampling factor is found by dividing the target MPP by the MPP at the highest  
390 resolution level of the scan (*level 0*). The level 0 MPP is accessed from the scan by `OpenSlide`  
391 using the `PROPERTY_NAME_MPP_X` and `PROPERTY_NAME_MPP_Y`. In case the directional level 0 MPP  
392 are different\*, the target downsampling factor will also be different in the two directions. If these  
393 two properties are not available in the scan, it is not included in the study.

394 For neural network optimisation and application, we read tile regions from the scan file one  
395 by one rather than the entire scan. Each tile is read from the scan at the pyramid level with a  
396 corresponding downsampling factor smaller than or equal to the target downsampling factor (or  
397 the smallest of the two directional target downsampling factors if they are different). Unless the  
398 target downsampling factor is equal to the reading downsampling factor, the size of the read tile  
399 will be larger than the target size. The enlarged tile is therefore downsampled to the target size  
400 so that the resulting resolution is equal to the target resolution. Downsampling to a target size  
401 (instead of to a target factor) also ensures that the resulting tile has the exact height and width  
402 we desire (and not e.g. off-by-one due to rounding). This final resizing is performed using `OpenCVs`  
403 `resize` function with the `INTER_AREA` interpolation option. This ensures that no upsampling is  
404 performed, but may result in tiles being read from the scan at different resolutions depending on  
405 the scanner model and settings.

406 For background exclusion, performance evaluation and display purposes, we use the downsam-  
407 pled scan as a single image, and in these cases the scan is downsampled to a resolution of 5 MPP  
408 (about 2 $\times$  magnification). Extracting the image from the scan file is done as for the tiles explained  
409 in the previous paragraph, with the exception that the target resolution is different and that the  
410 entire scan is read all at once in stead of in smaller regions.

### 411 2.2.2 Tiling

412 Since the downscaled scans are too large to process at a resolution of 1 MPP, they are partitioned  
413 into a set of tiles. The horizontal and vertical spatial dimensions are split in the same way, and  
414 the procedure for computing tile start and end coordinates is listed as python code in protocol  
415 listing 1.

416 The scan is partitioned into overlapping tiles if the scan dimension is not an integer multiple of  
417 the tile dimension and the minimum overlap is not specified to be 0. The amount of overlap is equal  
418 between all tile columns in the horizontal direction, except for between the rightmost tile columns  
419 which may overlap more, so that the rightmost tile column aligns with the right scan boundary.  
420 The same is true in the vertical direction where tile rows overlap with the same amount except  
421 perhaps for between the bottommost tile rows. With the procedure shown in protocol listing 1, we  
422 can also specify the minimum number of overlapping pixels along a dimension.

---

\*In this study, none of the included scans had different directional level 0 MPP

```

423
424 1 from typing import List, Tuple
425 2 import numpy as np
426 3
427 4
428 5 def find_overlap(full_size: int, part_size: int, min_overlap: int) -> Tuple[float, int]:
429 6     assert full_size > part_size, "The part is larger than the whole"
430 7     num_parts = int(np.ceil(full_size / part_size))
431 8     overlap = (part_size * num_parts - full_size) / (num_parts - 1)
432 9     if overlap < min_overlap:
433 10        assert part_size > min_overlap, "Part size must be greater than minimal overlap"
434 11        num_parts = int(np.ceil((full_size - min_overlap) / (part_size - min_overlap)))
435 12        overlap = (part_size * num_parts - full_size) / (num_parts - 1)
436 13    return overlap, num_parts
437 14
438 15
439 16 def partition(full_size: int, part_size: int, min_overlap: int) -> List[range]:
440 17     """
441 18     Divide a full line into parts where the line have size full_size and the parts have
442 19     size part_size (except when full_size < part_size).
443 20
444 21     Return a list of part start (inclusive) and stop (exclusive) points on the full line
445 22     """
446 23     ranges: List[range] = []
447 24     if full_size > part_size:
448 25         overlap, num_parts = find_overlap(full_size, part_size, min_overlap)
449 26         fractional_part = overlap - np.floor(overlap)
450 27         num_ceils = int(np.floor(num_parts * fractional_part))
451 28         for k in range(num_parts):
452 29             if k <= num_ceils:
453 30                 int_overlap = int(np.ceil(overlap))
454 31             else:
455 32                 int_overlap = int(np.floor(overlap))
456 33             if k == 0:
457 34                 start = 0
458 35             else:
459 36                 start = ranges[k - 1].stop - int_overlap
460 37             ranges.append(range(start, start + part_size))
461 38     else:
462 39         ranges.append(range(0, full_size))
463 40     return ranges

```

**Protocol Listing 1:** Divide with overlap

465 Tiles used for network optimisation have a target spatial dimension of  $2048 \times 2048$  pixels and  
466 are sampled from the scan with a minimum overlap of 0 pixels. Tiles used for network inference  
467 have a target spatial dimension of  $7680 \times 7680$  pixels with a minimum overlap of 1024 pixels.

468 Scan tiles are written as jpg files with 95% quality while annotation mask tiles are written as  
469 png files. Full scans at 5 MPP are written as png files.

470 **2.2.3 Dataset balancing**

471 The development set was balanced w.r.t. cancer type by oversampling the minority groups on a  
 472 tissue slide level. Tissue slides were selected multiple times at random without replacement so that  
 473 no slides were selected  $n + 1$  times before all slides had been selected  $n$  times. This resulted in 3 519  
 474 sections sampled from each cancer type (the same number of sections included in lung carcinoma,  
 475 which was the majority group). Counting scans from both scanners, the result was 7 030 scans from  
 476 colorectal carcinoma and 7 038 scans from each of the other cancer types. See protocol table 10  
 477 for an overview of the number of scans for each cohort. Note that since the selection was done  
 478 on a slide level, and cohorts DCo2 and DCo3 had fewer NanoZoomer XR scans than Aperio AT2,  
 479 there are slightly fewer scans from NanoZoomer XR than from Aperio AT2 in protocol table 10  
 480 for these two cohorts.

**Protocol Table 10:** Number of annotated scans in the training cohorts after balancing with oversampling

| Cancer type           | Cohort | Scans      |               |
|-----------------------|--------|------------|---------------|
|                       |        | Aperio AT2 | NanoZoomer XR |
| Colorectal carcinoma  | DCo1   | 471        | 471           |
|                       | DCo2   | 1 309      | 1 303         |
|                       | DCo3   | 1 739      | 1 737         |
|                       | Sum    | 3 519      | 3 511         |
| Endometrial carcinoma | DEn1   | 3 519      | 3 519         |
| Lung carcinoma        | DLu1   | 3 519      | 3 519         |
| Prostate carcinoma    | DPr1   | 1 981      | 1 981         |
|                       | DPr2   | 1 538      | 1 538         |
|                       | Sum    | 3 519      | 3 519         |
| Sum                   |        | 14 076     | 14 068        |

481 **2.2.4 Background segmentation**

482 A simple method is employed to segment the white background in an image from the rest. This  
 483 background mask is used to alter both predicted and reference segmentation masks. This is useful  
 484 when large background regions are inside the annotated region (one example being holes from  
 485 *tissue microarray* acquisition) without being manually annotated as background. These regions  
 486 are clearly not cancerous tissue, and should not be annotated as such neither by the reference nor  
 487 by the prediction.

488 Note that this segmentation is quite sensitive in that it will mark most tissue as foreground, also  
 489 adipose tissue that is often left out when applying threshold methods based on image brightness  
 490 or saturation or similar. But it may also include artefacts such as pen markings, air bubbles, dust,  
 491 glass cracks, etc. But since the mask is used to exclude white background tiles used in training, it  
 492 can be an advantage that foreground elements other than tissue is included. The method with the  
 493 stated parameter values assumes images of H&E-stained tissue with 5 MPP resolution.

494 Canny edge detection is performed on the input colour image, using the `OpenCV Canny`  
 495 implementation.[26] We use a  $3 \times 3$  *Sobel* filter for the gradient computation, and thresholds of  
 496 10 and 50 for the lower and upper thresholds in the hysteresis. This produce a mask with lots of  
 497 foreground pixels in regions with structure and lots of background pixels in homogeneous regions.

498 This foreground mask is refined by first removing small background regions. The mask first

499 undergoes morphological closing (`openCV morphologyEx`) with a square  $9 \times 9$  structure element  
500 before background regions with an area smaller than 10 000 pixels are filled in with the function  
501 `remove_small_holes` from the `scikit-image` python library. An area of 10 000 pixels at 5 MPP  
502 resolution corresponds to a square region of  $0.5 \text{ mm} \times 0.5 \text{ mm}$ .

503 Finally, small foreground regions are removed from the mask. Morphological opening is ap-  
504 plied on the mask using the `openCV morphologyEx` with the same  $9 \times 9$  structure element  
505 before foreground regions with an area smaller than 1 600 pixels are erased using the function  
506 `remove_small_objects` from the `scikit-image` python library. An area of 1 600 pixels corre-  
507 sponds to a square region of  $0.2 \text{ mm} \times 0.2 \text{ mm}$  at 5 MPP resolution.

508 This method is simple to implement, very robust, and quite fast, spending around one second  
509 per image on a single CPU core on consumer-grade hardware. An example of a downscaled scan  
510 from colorectal carcinoma scanned with Aperio AT2 and manually annotated is shown in protocol  
511 figure 26.

512 With this we can classify every pixel as either white background, foreground without annotation  
513 and foreground with annotation. This content classification is summarised for all scans in all  
514 cohorts used in this study in protocol figures 27 to 30.

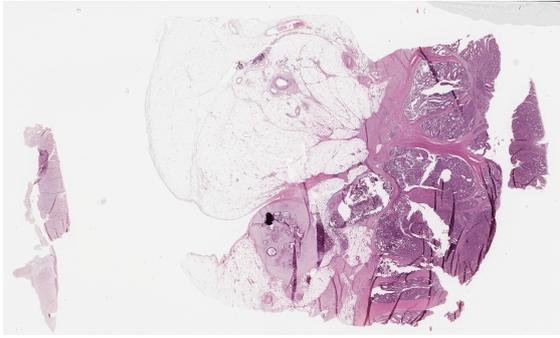

(a) Histology image

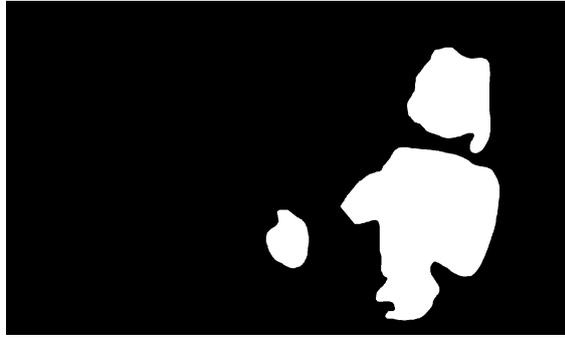

(b) Annotation mask without background segmentation

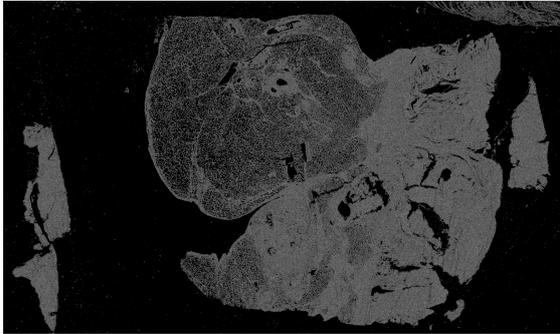

(c) Edges detected with the Canny method

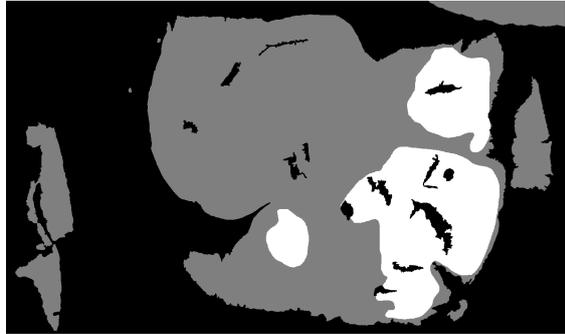

(d) Annotation and foreground mask

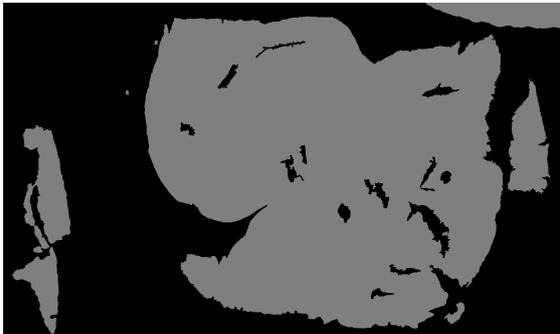

(e) Foreground mask

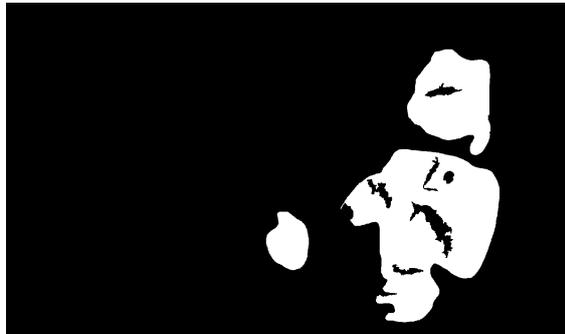

(f) Annotation mask after removing background

**Protocol Figure 26:** Scan and segmentation mask with background (black), foreground (gray) and tumour annotation (white)

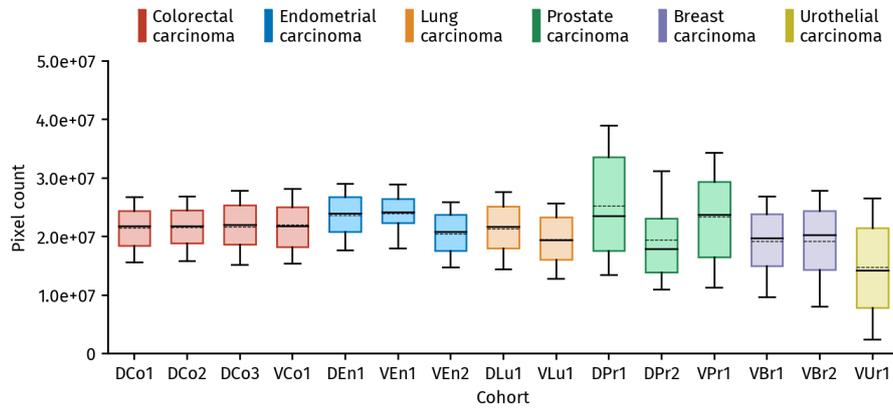

(a) Image area

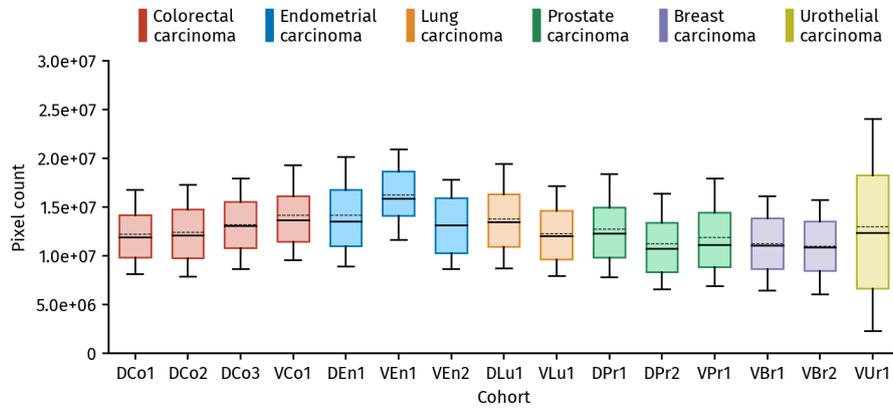

(b) Foreground area

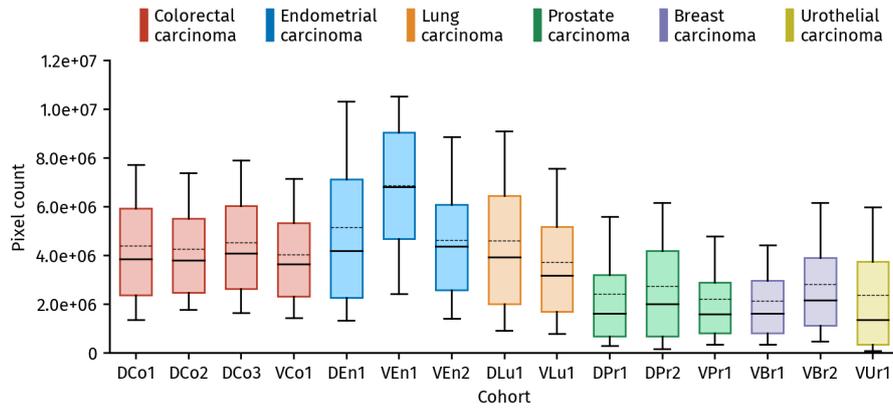

(c) Annotation area

**Protocol Figure 27:** Area in number of pixels at resolution 5  $\mu\text{m}$  per pixel in Aperio AP2 scans. “Foreground” is foreground without annotation and “Annotation” is foreground with annotation. Background exclusion masks are applied on all images. Note the difference in vertical axis range between subplots.

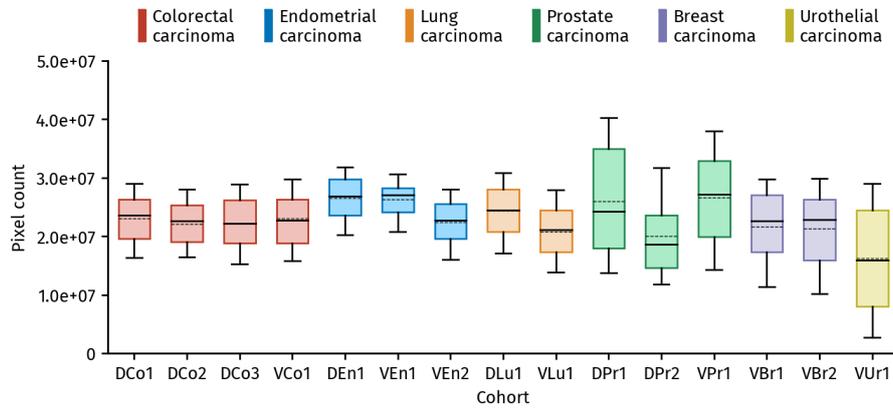

(a) Image area

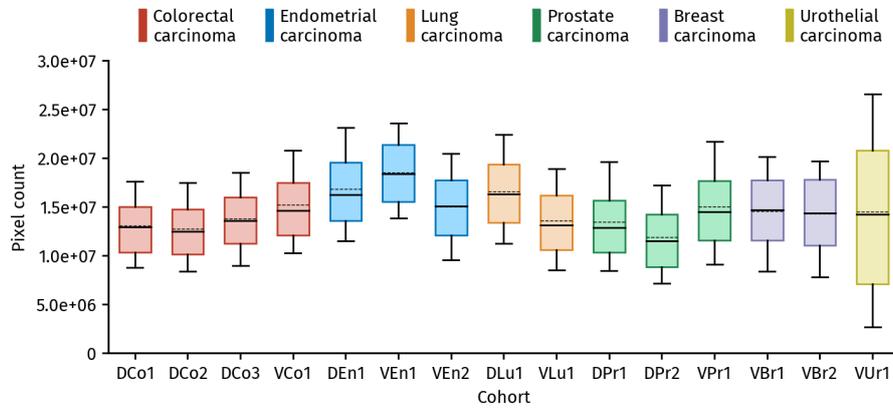

(b) Foreground area

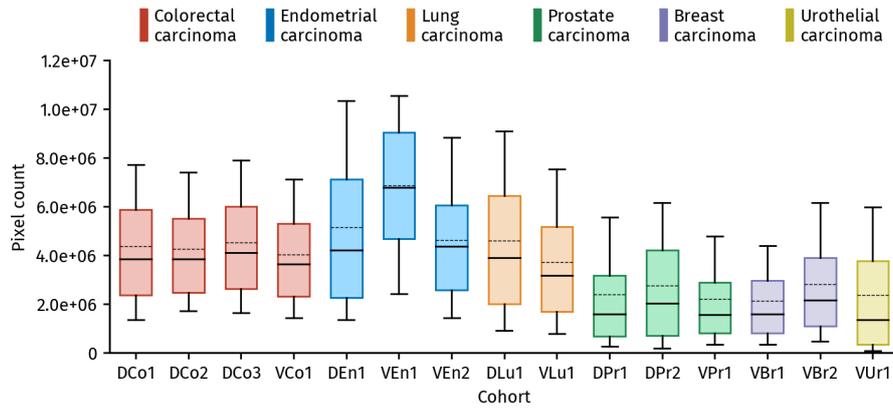

(c) Annotation area

**Protocol Figure 28:** Area in number of pixels at resolution  $5\mu\text{m}$  per pixel in NanoZoomer XR scans. “Foreground” is foreground without annotation and “Annotation” is foreground with annotation. Background exclusion masks are applied on all images. Note the difference in vertical axis range between subplots.

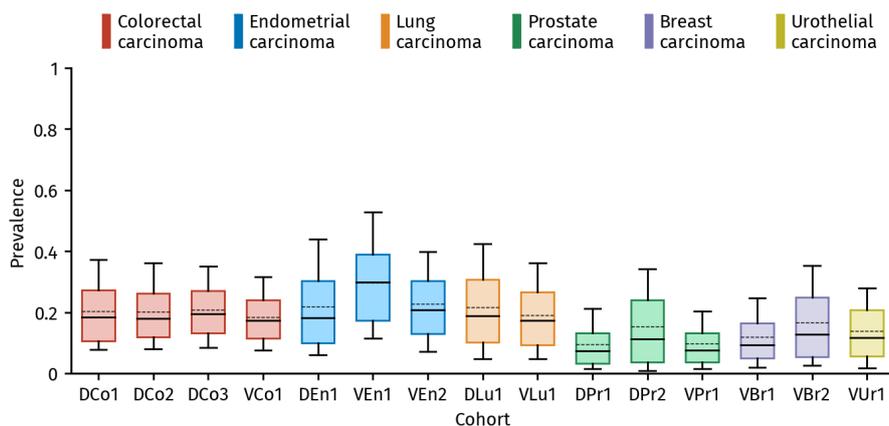

(a) Annotation prevalence in image

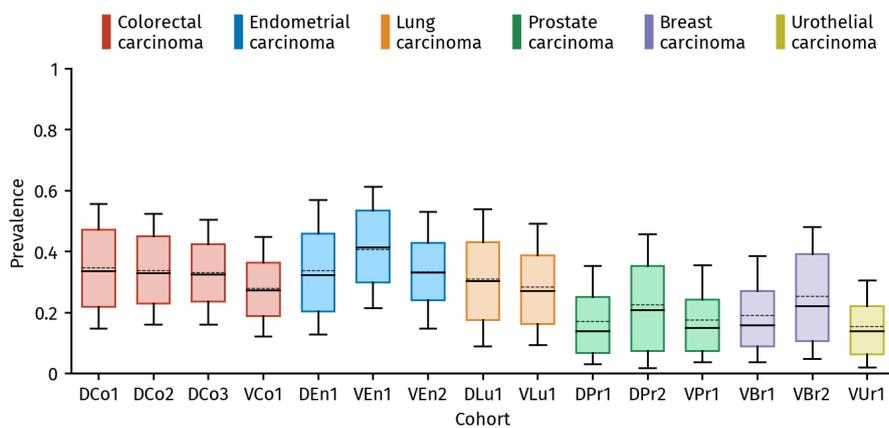

(b) Annotation prevalence in foreground

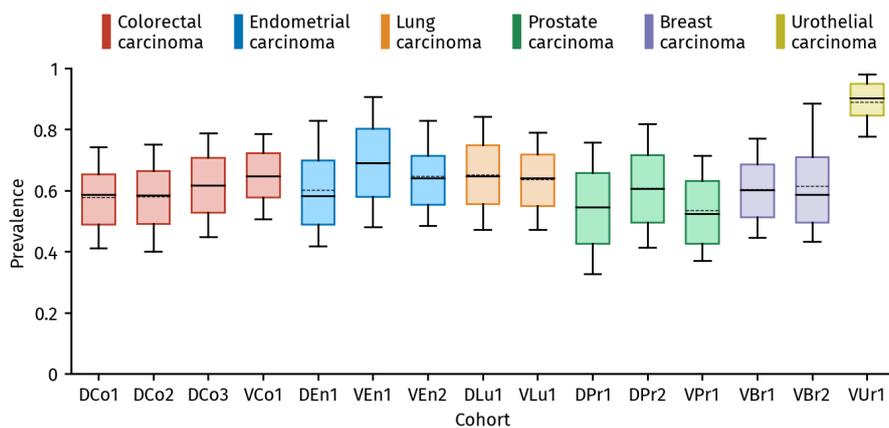

(c) Foreground prevalence in image

**Protocol Figure 29:** Prevalence at resolution 5  $\mu\text{m}$  per pixel in Aperio AT2 scans. “Foreground” is foreground without annotation and “Annotation” is foreground with annotation. Background exclusion masks are applied on all images.

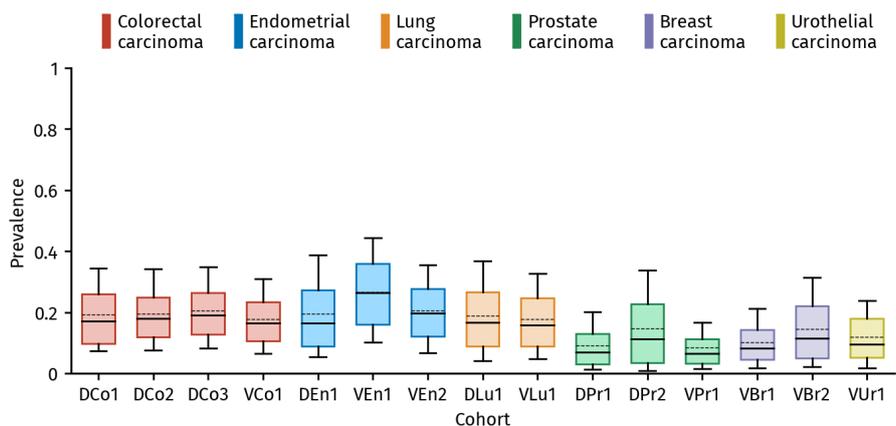

(a) Annotation prevalence in image

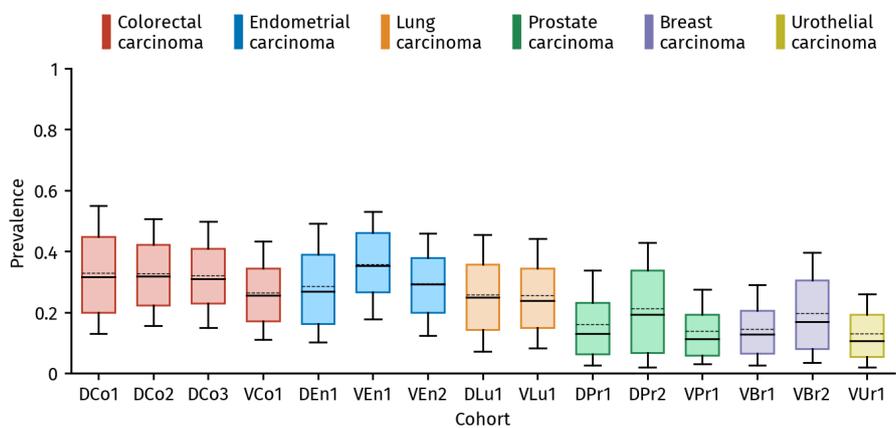

(b) Annotation prevalence in foreground

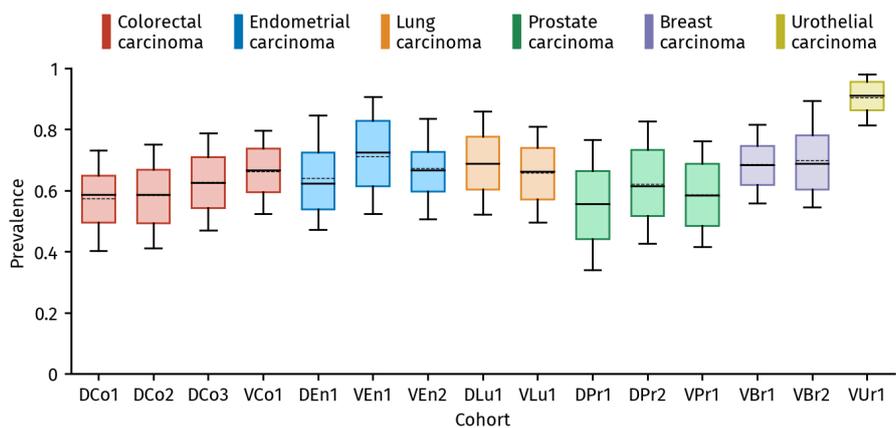

(c) Foreground prevalence in image

**Protocol Figure 30:** Prevalence at resolution  $5\mu\text{m}$  per pixel in NanoZoomer XR scans. “Foreground” is foreground without annotation and “Annotation” is foreground with annotation. Background exclusion masks are applied on all images.

515 **2.2.5 Background tile exclusion**

516 Tiles containing too much white background are removed from the development set. The back-  
 517 ground segmentation is performed on 5 MPP full images as described in section 2.2.4 and trans-  
 518 ferred to the 1 MPP tiles. Specifically, we include all tiles that contain some tumour annotated  
 519 regions, and for those that don't, we keep those with a background fraction smaller than 50%.

520 In total this reduces the number of unique tiles from 3 080 330 to 2 144 651 or from 4 233 081 to  
 521 2 902 032 non-unique tiles in the balanced dataset (see protocol table 11 and protocol figure 31).

**Protocol Table 11:** Number of unique tiles in development cohorts before and after background exclusion

| Cohort | Aperio AT2   |             |       | NanoZoomer XR |             |       | Both scanners |             |       |
|--------|--------------|-------------|-------|---------------|-------------|-------|---------------|-------------|-------|
|        | Tiles before | Tiles after | %     | Tiles before  | Tiles after | %     | Tiles before  | Tiles after | %     |
| DCo1   | 28 911       | 19 429      | 67.20 | 30 552        | 20 245      | 66.26 | 59 463        | 39 674      | 66.72 |
| DCo2   | 81 651       | 54 356      | 66.57 | 82 294        | 55 104      | 66.96 | 163 945       | 109 460     | 66.77 |
| DCo3   | 108 429      | 76 511      | 70.56 | 109 720       | 78 609      | 71.65 | 218 149       | 155 120     | 71.10 |
| DEn1   | 514 341      | 340 922     | 66.28 | 566 105       | 394 211     | 69.64 | 1 080 446     | 735 133     | 68.04 |
| DLu1   | 492 150      | 364 029     | 73.97 | 551 767       | 422 192     | 76.52 | 1 043 917     | 786 221     | 75.31 |
| DPr1   | 158 001      | 91 707      | 58.04 | 163 527       | 96 500      | 59.01 | 321 528       | 188 207     | 58.54 |
| DPr2   | 95 015       | 63 855      | 67.21 | 97 867        | 66 981      | 68.44 | 192 882       | 130 836     | 67.83 |
| Sum    | 1 478 498    | 1 010 809   | 68.37 | 1 601 832     | 1 133 842   | 70.78 | 3 080 330     | 2 144 651   | 69.62 |

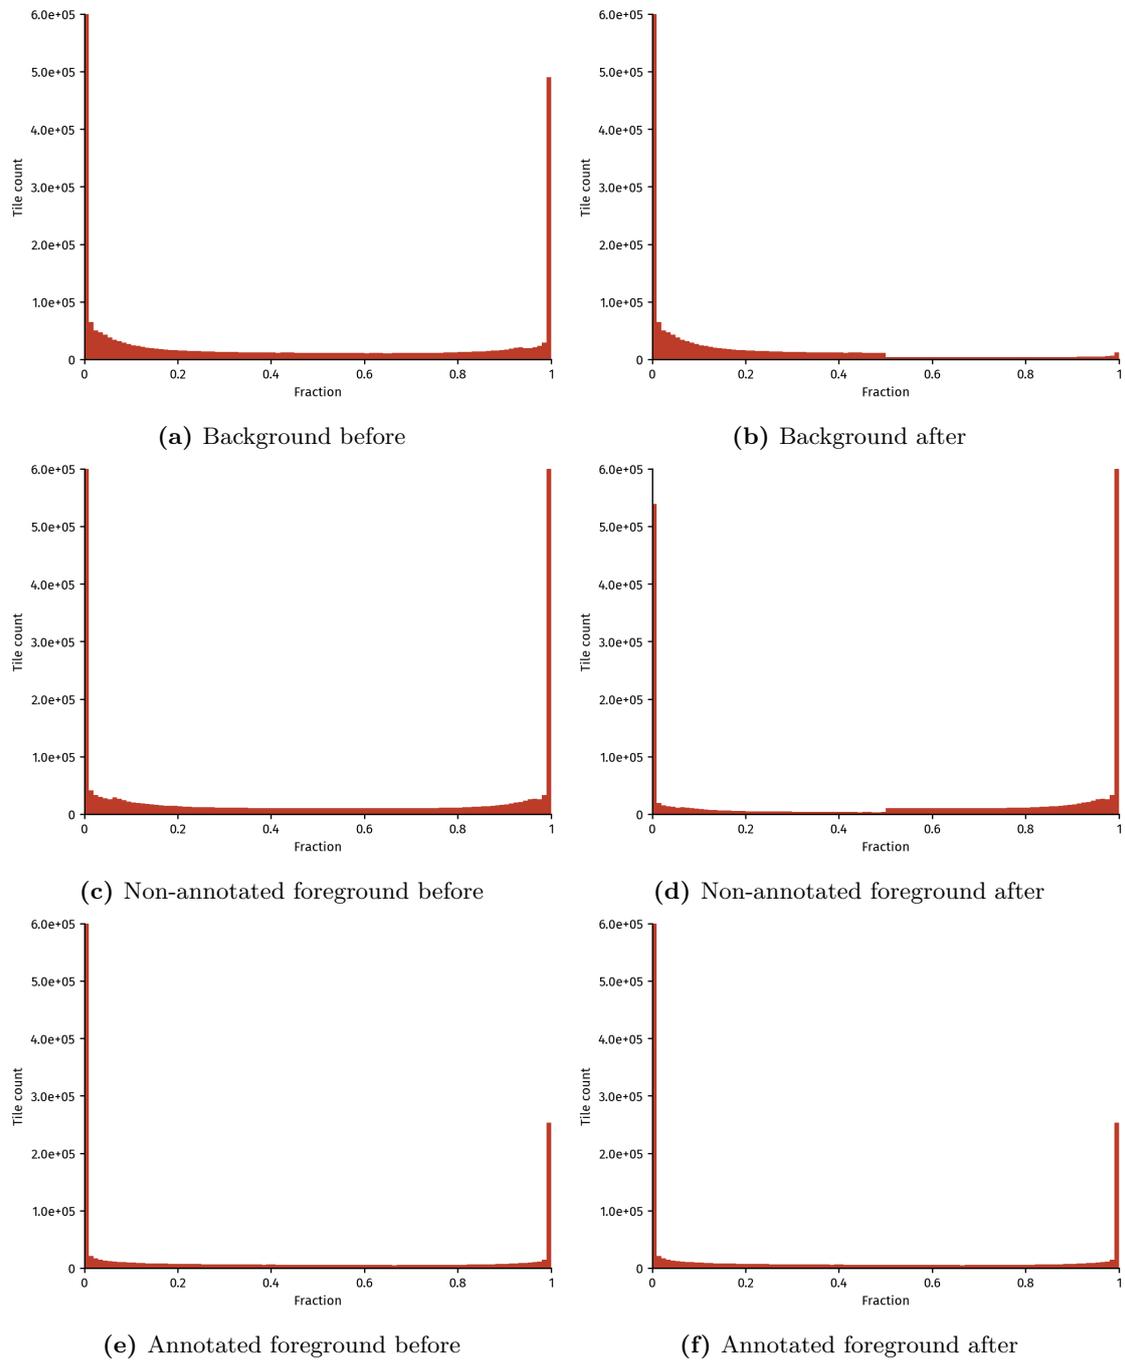

**Protocol Figure 31:** Distribution of number of tiles with a certain fraction of either background (top row) non-annotated foreground (middle row) and annotated foreground (bottom row) before (left column) and after (right column) background exclusion.

## 522 2.2.6 Dataset augmentations

523 Image tiles are read as *RGB* with 8 bits values per channel, cast to 32 bits floating point values,  
 524 and then preprocessed before they enter the segmentation network. We artificially augment the  
 525 training dataset by distorting images using the `albumentations` library.[27] The operations are  
 526 listed in protocol listing 2 in the order they are applied. Note that while the tiles are sampled at a  
 527 size of  $2048 \times 2048$  pixels, they are cropped to a size of  $1536 \times 1536$  pixels before they enter the  
 528 network.

529 Image distortions are only applied during network optimisation, and not when the fixed network  
 530 is applied.

```

531
532 1 HorizontalFlip(p=0.5)
533 2 RandomRotate90(p=0.5)
534 3 PadIfNeeded(min_height=1536, min_width=1536, border_mode=cv2.BORDER_CONSTANT, value=0)
535 4 RandomCrop(height=1536, width=1536)
536 5 RandomBrightnessContrast(
537 6     brightness_limit=[-0.2, 0.2], contrast_limit=[-0.2, 0.2], brightness_by_max=True, p=1
538 7 )
539 8 HueSaturationValue(
540 9     hue_shift_limit=[-26, 26], sat_shift_limit=[-26, 26], val_shift_limit=[-26, 26], p=1
541 10 )
542
  
```

**Protocol Listing 2:** Image distortions

## 543 2.2.7 Image value standardisation

544 Before the image enters the network, the image values are divided by 255 before the image is centred  
 545 around the development dataset mean value and scaled with the development dataset standard  
 546 deviation. This standardisation is applied both during network optimisation and inference.

547 The dataset mean value for an image channel is computed as

$$\begin{aligned}
 \mu &= \frac{1}{m} \sum_{i=1}^m \mu_i \\
 &= \frac{1}{m} \sum_{i=1}^m \frac{1}{n_i} \sum_{j=1}^{n_i} x_{ij}
 \end{aligned}$$

548 where  $x_{ij}$  is the value at pixel  $j$  in image  $i$  for the image channel and  $\mu_i$  is the mean value in image  
 549  $i$ .  $n_i$  is the number of pixels in image  $i$ , and  $m$  is the number of images in the dataset. Similarly,  
 550 the dataset variance for a single channel is estimated as

$$\begin{aligned}
 \sigma^2 &= \frac{1}{m} \sum_{i=1}^m \sigma_i^2 \\
 &= \frac{1}{m} \sum_{i=1}^m \frac{1}{n_i - 1} \sum_{j=1}^{n_i} (x_{ij} - \mu_i)^2.
 \end{aligned}$$

551 We use  $\sigma = \sqrt{\sigma^2}$  as the estimate for the dataset standard deviation. For both estimates  $\mu$  and  $\sigma$ ,  
 552 the final result is divided by 255 before it is applied.

553 When applied on all unique  $2048 \times 2048$ -sized tiles in the development dataset at resolution  
 554 1 MPP without distortions, we get the result shown in protocol table 12 and protocol figures 32

555 and 33. Colour mean and standard deviation distributions for the all scans at resolution 5 MPP  
556 are shown in protocol figures 22 to 25.

**Protocol Table 12:** Colour statistics for all unique tiles in the development set. Here, all 8-bit integer colour channel values are cast to 32 bit floating point values before the per-image statistics are computed. These values are then averaged over all tiles and the result is divided by 255.

| Colour channel | Mean value | Standard deviation |
|----------------|------------|--------------------|
| Red            | 0.8297992  | 0.1051075          |
| Green          | 0.7106879  | 0.1543867          |
| Blue           | 0.8241846  | 0.0991757          |

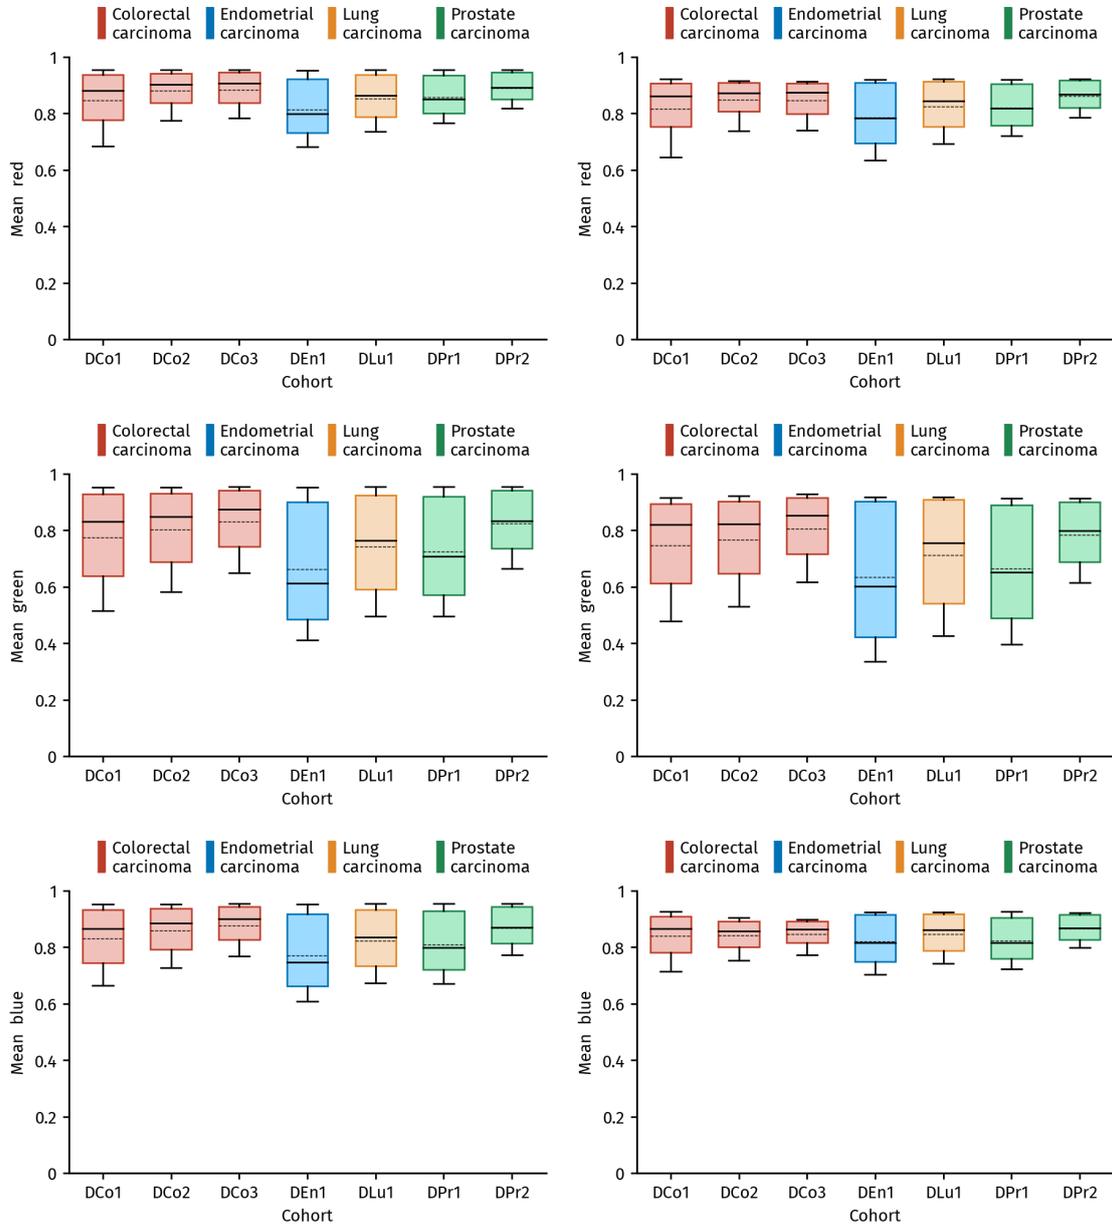

**Protocol Figure 32:** Colour channel mean value for all unique tiles in the development set. Tiles have resolution 1 MPP and a size of  $2048 \times 2048$  pixels. Aperio AT2 in the left column and NanoZoomer XR in the right column.

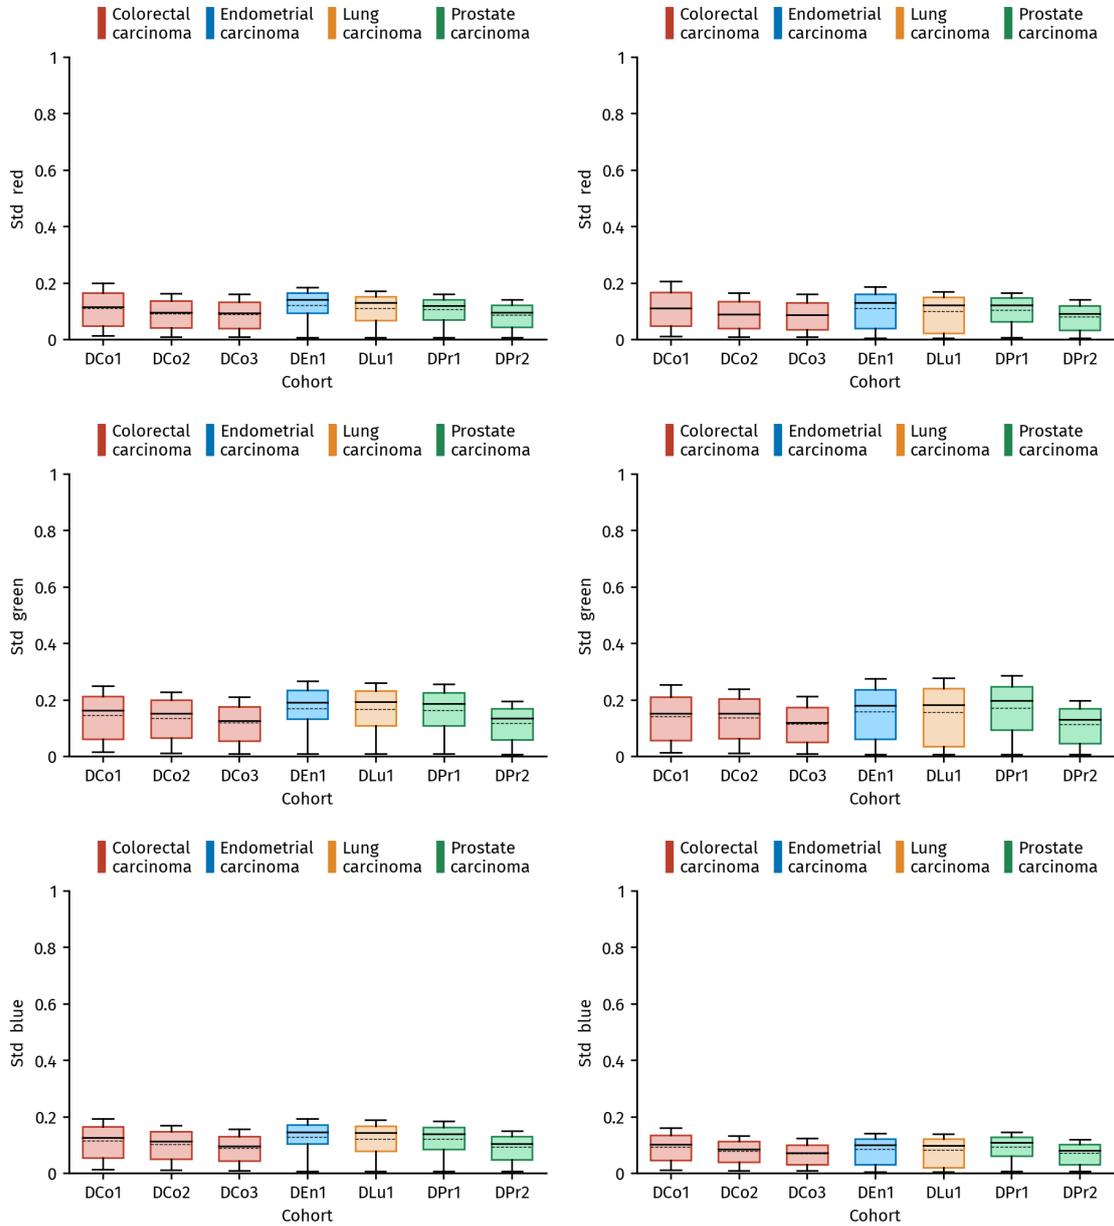

**Protocol Figure 33:** Colour channel standard deviation for all unique tiles in the development set. Tiles have resolution 1 MPP and a size of  $2048 \times 2048$  pixels. Aperio AT2 in the left column and NanoZoomer XR in the right column.



574 **2.2.9 Network optimisation**

575 Below we describe how the network was optimised, but in general we follow the procedure described  
 576 in by Brock and colleagues in their NFNNet paper, with some exceptions.[29] We do *not* use *Adaptive*  
 577 *Gradient Clipping* as we did not see any benefit for it in our case, perhaps because of our small  
 578 batch size (24 images). We also do not use moving averages of the model parameters.

579 The objective is to minimise the difference between the output of the segmentation network and  
 580 the reference segmentation by iteratively modifying the adjustable parameters of the segmentation  
 581 network. The difference to be minimised is captured by the loss function  $l = l_1 + l_2$ , where  $l_1$  is the  
 582 so-called *Dice-loss* (`DiceLoss` from `segmentation_models_pytorch` with `mode="multiclass"`),  
 583 and  $l_2$  is a so-called *top-90 Cross Entropy* loss function. The top-90 Cross Entropy at a particular  
 584 step is computed by first computing the per-pixel cross entropy for all pixels in the mini batch  
 585 of this step and then averaging the cross entropy value over pixels in the top 90 percentile. That  
 586 is, when computing the mean cross entropy, we are ignoring 10% of pixels with the lowest cross  
 587 entropy value.

588 We predict three classes, and the reference is segmented into background, non-annotated fore-  
 589 ground, and tumour-annotated foreground. We also experimented with using just two classes,  
 590 tumour-annotated foreground and everything else, but we did not notice any important difference  
 591 in performance.

592 The convolution weights in the encoder are initialised with *normal* initialisation while the biases  
 593 are initialised to zero.

$$X \sim \mathcal{N}(0, \sigma^2), \text{ where } \sigma = \sqrt{\frac{1}{c_i hw}}.$$

594 The convolution weights and biases used in the decoder and segmentation head are initialised with  
 595 *uniform* initialisation

$$X \sim \mathcal{U}(-a, a), \text{ where } a = \sqrt{\frac{1}{c_i hw}}.$$

596 In the above equations,  $c_i hw$  is the volume of the input feature maps in the convolutional layer  
 597 (number of input channels times the height times the width), often called *fan in*.[38]

598 At each iteration (or step), the adjustable network parameters are updated according to the  
 599 *Stochastic Gradient Descent* optimisation method with *Nesterov momentum* 0.9.[39] The optimisa-  
 600 tion is regularised with a *weight decay* value of  $2 \times 10^{-5}$  with the exceptions described by Brock  
 601 and colleagues.[29]

602 A batch of 24 images is randomly selected without replacement from the development dataset  
 603 and processed at each step. When the dataset is exhausted we say that an *epoch* is complete,  
 604 and the selection is reset. The whole batch is processed by the segmentation network before  
 605 the output is compared with the corresponding reference segmentation batch with the objec-  
 606 tive function. The batch of 24 is distributed on 8 GPUs with 3 tiles per GPU using `pytorchs`  
 607 `DistributedDataParallel`

608 The step length is initialised to  $1.0 \times 10^{-4}$  and incremented by  $1.0 \times 10^{-4}$  every 10th step until  
 609 step 1 000 when the step length has reached  $1.0 \times 10^{-2}$ . After this warm up period, the step length  
 610 follows a cosine annealing schedule until termination (see protocol figure 35).[40]

611 The optimisation is carried out for 500 000 steps (or 4.14 epochs) before termination. Since we  
 612 have 2 902 032 tiles in the dataset and 24 tiles per batch, we have 120 918 steps per epoch. The  
 613 model at step 500 000 is selected as the model used in the segmentation method.

614 We employ *Automatic mixed precision* both during optimisation of the network and when  
 615 applying it. This is provided by the `torch.cuda.amp` module in the `pytorch` python package.

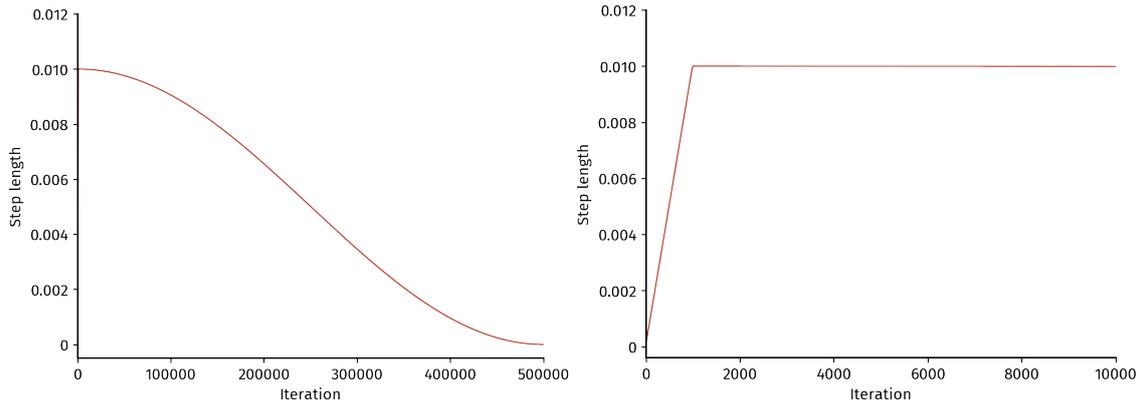

**Protocol Figure 35:** Step length with respect to optimisation iteration. Left panel shows all 500 000 steps while the right panel only shows the first 10 000 steps.

## 616 2.3 Method application

617 Application of the method on a single input scan can be summarised as

- 618 1. Read the input scan at 1 MPP resolution (section 2.3.1)
- 619 2. Partition the downsampled scan into overlapping tiles (section 2.3.1)
- 620 3. Apply the optimised segmentation network on each tile (section 2.3.2)
- 621 4. Construct a probability image from the segmentation network tiles (section 2.3.3)
- 622 5. Post-process to yield a final segmentation mask (section 2.3.4)

### 623 2.3.1 Downsampling and tiling

624 Scan reading and downsampling is done as described in section 2.2.1. Tiling is done as described  
 625 in section 2.2.2, with tile size of  $7\,680 \times 7\,680$  pixels with a minimum overlap of 1 024 pixels in each  
 626 direction (see example in protocol figure 36).

### 627 2.3.2 Neural network

628 Input images are processed with the optimised segmentation network after the following operations  
 629 are applied on the input image

- 630 1. Read image as RGB with 8-bit values in each channel
- 631 2. Zero-pad image so that both the image height and width are divisible by 16. This step is not  
 632 necessary for this particular setup since we have tiles with size  $7\,680 \times 7\,680$ , but is included  
 633 for making the method applicable in the general case with varying input sizes.
- 634 3. Scale image values to  $(0, 1)$  by dividing by 255
- 635 4. Subtract image by development dataset mean (protocol table 12)
- 636 5. Divide image by development dataset standard deviation (protocol table 12)

637 The resulting prediction from the segmentation network is an image with one channel per output  
 638 class, where only the channel corresponding to the tumour class is used further. Its values are  
 639 floats where pixel value 0 indicates negative prediction and 1 indicate positive prediction. The  
 640 image values are multiplied by 255 before the image is quantised to 8 bits. The padding (if any)  
 641 is removed before the prediction is written as a `png` image.

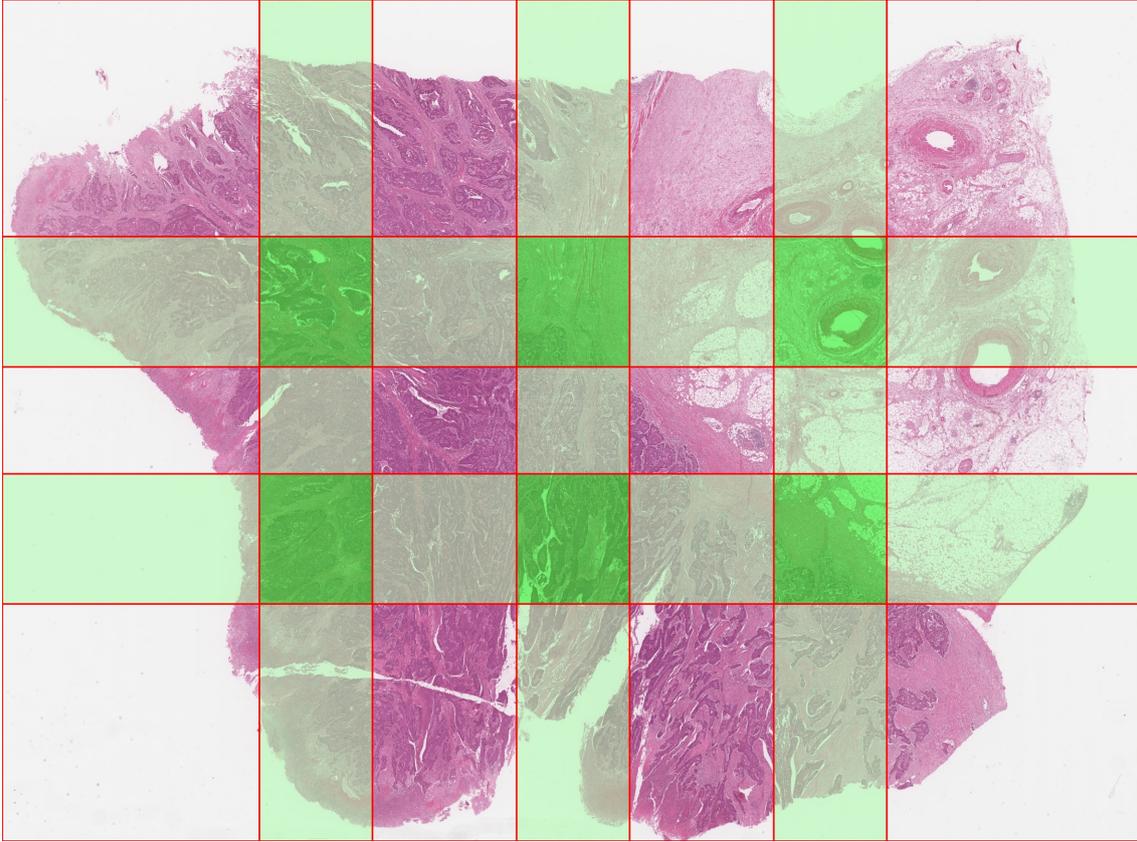

**Protocol Figure 36:** Tiling with size  $7680 \times 7680$  pixels and minimum overlap of 1024 pixels at resolution 1 MPP. Red shows the tile contour. Tile interiors are shown in green with opacity increasing with the number of overlapping tiles: transparent for no overlapping, light green for two overlapping, and darker green for four overlapping tiles.

### 642 2.3.3 Reconstruction from tiles

643 The final reconstructed image  $f$  is computed as  $f = \sum_i w_i g_i$  where  $f, w_i, g_i$  are  $m \times n$  matrices  
 644 and  $i$  iterate over all tiles.  $g_i$  represent a single tile output from the segmentation network, and  
 645 has the output tile value in the tile location and value zero everywhere else.  $w_i$  represent a single  
 646 weight tile which has values in the corresponding tile location and value zero everywhere else.  $w_i$   
 647 have values in  $[0, 1]$  and  $g_i$  have integer values in  $[0, 255]$  since they have been written as 8-bit `png`  
 648 files by the segmentation network. The values of  $f$  are quantised to integer values by rounding  
 649 with the tie-breaking rule of rounding half to even before  $f$  is written as `png`.

650 The weight tiles are constructed so that the sum weight image  $s = \sum_i w_i$  with shape  $m \times n$   
 651 will have value 1 in all pixels. In the rest of this explanation a *weight tile* and *image tile* will refer  
 652 only to the part of  $w_i$  and  $g_i$  that correspond to the location of each tile, respectively.

653 The tile weights are constructed in three phases, and an example result is shown in protocol  
 654 figure 37. First, initial weight tiles are computed for each image tile. These weight tiles are  
 655 weighted by distance in overlapping regions. A sum image the same size of  $f$  is constructed by  
 656 adding all initial weight tiles  $w$  at their locations within this sum image. Each initial weight tile  
 657 is normalised by dividing it by the tile cropped out from its location within the sum image. The  
 658 next two paragraphs explain the construction of the initial weight tiles.

659 An initial weight tile  $w$  is computed as the element-wise product of four side-specific weight  
 660 tiles:  $w_t$  weighting overlaps at the top of  $w$ ,  $w_b$  weighting overlaps at the bottom of  $w$ ,  $w_l$  weighting

661 overlaps at the left of  $w$  and  $w_r$ , weighting overlaps at the right of  $w$ .  
 662 In order to compute a side-specific weight tile, e.g.  $w_r$ , the smallest leftmost coordinate of all  
 663 overlapping tiles with a leftmost coordinate greater than the leftmost coordinate in  $w$  is recorded.  
 664 The region between this recorded coordinate and the rightmost coordinate of  $w$  defines the overlapping  
 665 area to the right in  $w$ . All pixels in  $w_r$ , to the left of this overlapping area are given value 1, and  
 666 all other pixels are giving a value decreasing linearly with the distance from the left overlapping  
 667 border:  $v = 1 - \frac{d}{1+l}$  where  $v$  is the result value,  $d$  is the distance from the left overlapping border,  
 668 and  $l$  is the length of the overlapping region. Both  $d$  and  $l$  are measured in pixels. The procedure  
 669 and weighting is similar for the other side-specific weight tiles.

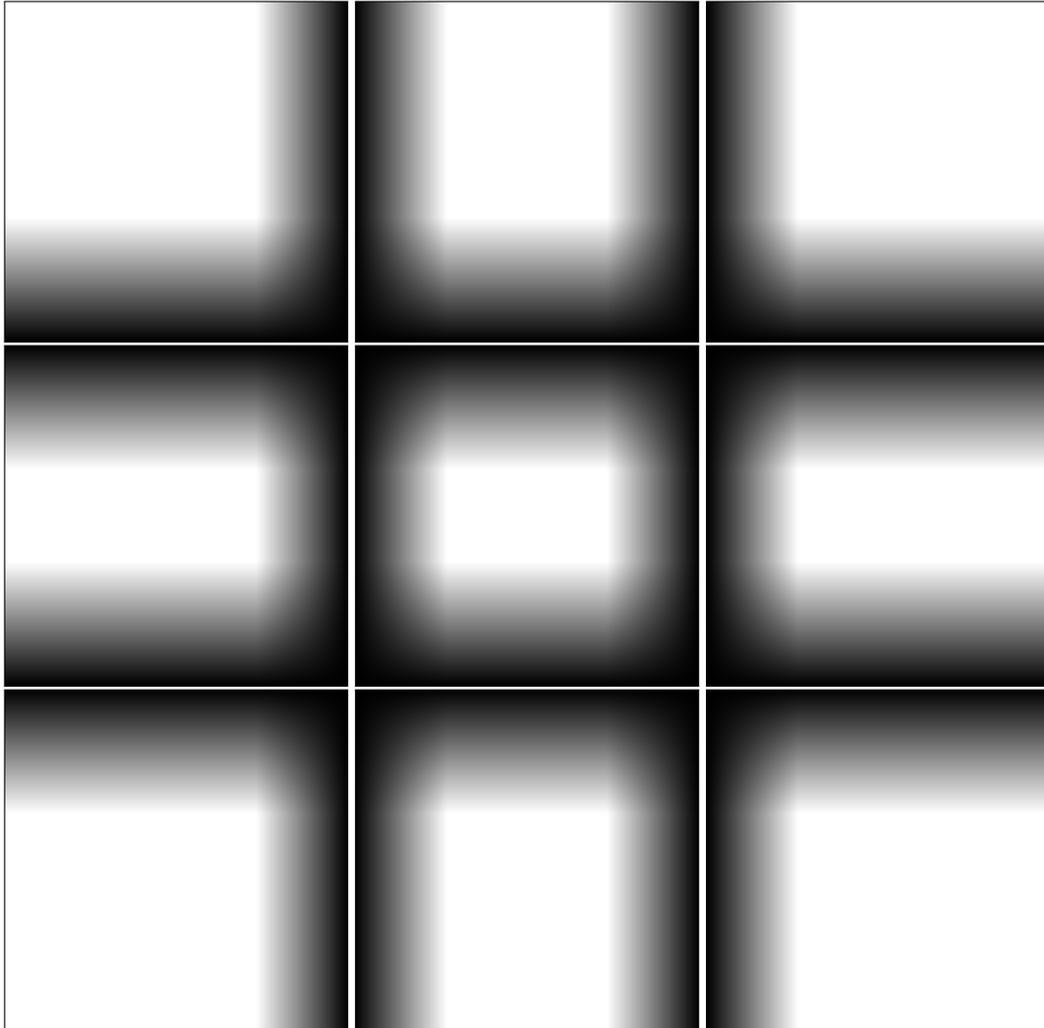

**Protocol Figure 37:** Weight tiles for merging overlapping tiles. The top left tile is overlapping with the tile to its right, the tile below, and to the tile in the middle. The centre tile is overlapping with all other tiles. The weight tile sub-images are arranged as their corresponding tiles. Note that frames are added in the above figure for clarity, but they are not present in the weight tiles.

#### 670 2.3.4 Result post-processing

671 Post-processing is used to transform the segmentation network output probability maps to binary  
 672 foreground and background masks. The process comprise three steps

- 673 1. Smooth the probability map
- 674 2. Binarise the smoothed probability map
- 675 3. Clean the binarised mask

676 The merged probability map from section 2.3.3 has the same size as the 1 MPP scan image  
677 they originate from. Before further post-processing, this probability map is downsampled by five  
678 times in both horizontal and vertical directions (corresponding to the scan image at 5 MPP).

679 We apply smoothing of the probability map both to get a smooth segmentation boundary in  
680 the final segmentation, and to reduce the impact of noise in the post-processing. For the sake  
681 of efficiency, the probability map is further downsampled before smoothing and upsampled again  
682 after smoothing is done. The downsampling factor is set to 0.2 for both the vertical and the  
683 horizontal direction unless the resulting image has an area less than  $10^6$ , in which case then the  
684 image is resized to have an area of  $10^6$ . This threshold is arbitrarily chosen as a safeguard against  
685 very small scans. Specifically, the new height and width is found by multiplication with a factor  
686  $\max\{0.2, \sqrt{10^6/(hw)}\}$  where  $hw$  is the area of the input. Then the resulting float value is floored  
687 to get an integer value. The image then undergoes median blurring with an aperture size of 9 using  
688 `OpenCVs medianBlur` function. Next, the result is further smoothed using `OpenCVs GaussianBlur`  
689 function with a kernel size of  $5 \times 5$ . Finally, the smoothed probability map is upsampled back to  
690 the original size corresponding to the 5 MPP scan image.

691 The smooth probability map is then dichotomised into foreground and background using a  
692 hysteresis threshold method. The lower threshold value is set to 85 (1/3 of 255) and the higher  
693 threshold value is set to 229 ( $\approx 90\%$  of 255).

694 Finally, foreground regions in the mask are pruned with the following procedure. For each  
695 connected foreground region in the foreground mask, collect the values the region cover in the  
696 smooth probability map. If the 95th percentile value of this collection is greater than 229, the  
697 corresponding region is kept as foreground, else it is labelled background.

698 All pixels not foreground in both the foreground mask from the probability map and the  
699 foreground mask from the scan image (section 2.2.4) are labelled as background. The resulting  
700 mask is further processed by removing small background regions and then small foreground regions  
701 as explained in section 2.2.4 for the foreground mask.

## 702 2.4 Performance evaluation

703 To measure the similarity between the reference and predicted segmentation, we use different  
704 metrics to highlight different similarities.

705 Since we employ the same background exclusion on both reference and prediction masks, it is  
706 of little interest to count true negative pixels in the white background area of a scan. We therefore  
707 excluded background in the performance evaluation. True negatives are therefore pixels that are  
708 marked as background in the prediction and neither as tumour nor background in the reference  
709 mask.

### 710 2.4.1 Overlap counting

711 For simple overlap comparison, we partition the pixels based on how they overlap in the reference  
712 and predicted segmentation:

**Protocol Table 13:** Confusion matrix

|           |            | Prediction |            |      |
|-----------|------------|------------|------------|------|
|           |            | Background | Foreground |      |
| Reference | Background | $TN$       | $FP$       | $RN$ |
|           | Foreground | $FN$       | $TP$       | $RP$ |
|           |            | $PN$       | $PP$       | $N$  |

$N$  = Pixel count in the image after excluding white background

$$RP = |\{x : x \text{ is foreground in reference}\}|$$

$$RN = |\{x : x \text{ is background in reference}\}|$$

$$PP = |\{x : x \text{ is foreground in prediction}\}|$$

$$PN = |\{x : x \text{ is background in prediction}\}|$$

$$TP = |\{x : x \text{ is foreground in reference and prediction}\}|$$

$$FN = |\{x : x \text{ is foreground in reference and background in prediction}\}|$$

$$FP = |\{x : x \text{ is background in reference and foreground in prediction}\}|$$

$$TN = |\{x : x \text{ is background in reference and prediction}\}|$$

713 These counts comprise a contingency table termed a *confusion matrix* (protocol table 13).

714 We can derive different metrics from the confusion matrix to measure different features of  
715 the segmentation result. Some common metrics that are used in this work are presented in the  
716 following.

717 True positive rate or sensitivity or recall measures the fraction of reference foreground pixels  
718 that are correctly marked as foreground

$$TPR = \frac{TP}{TP + FN} \quad (1)$$

719 False negative rate measures the fraction of reference foreground pixels that are wrongly marked  
720 as background

$$FNR = \frac{FN}{TP + FN} \quad (2)$$

721 True negative rate or specificity measures the fraction of reference background pixels that are  
722 correctly marked as background

$$TNR = \frac{TN}{TN + FP} \quad (3)$$

723 False positive rate measures the fraction of reference background pixels that are wrongly marked  
724 as foreground

$$FPR = \frac{FP}{TN + FP} \quad (4)$$

725 Positive predictive value or precision measures the fraction of predicted foreground pixels that are  
726 correctly marked as foreground

$$PPV = \frac{TP}{TP + FP} \quad (5)$$

727 Negative predictive value measures the fraction of predicted background pixels that are correctly  
728 marked as background

$$NPV = \frac{TN}{TN + FN} \quad (6)$$

729 Informedness

$$BIN = TPR + TNR - 1 \quad (7)$$

730 Markedness

$$BMA = PPV + NPV - 1 \quad (8)$$

731 Matthew's correlation coefficient is the geometric mean of informedness and markedness

$$MCC = \frac{TP \times TN - FN \times FP}{\sqrt{(TP + FN)(TP + FP)(TN + FN)(TN + FP)}} \quad (9)$$

732 Sørensen-Dice similarity coefficient or  $F_1$  score is the harmonic mean of the true positive rate and  
733 the positive predictive value

$$DSC = \frac{2TP}{2TP + FN + FP} \quad (10)$$

## 734 **3 Analyses**

### 735 **3.1 Primary analysis**

736 The primary analysis of this study is the performance assessment of an automatic method tasked  
737 to segment tumour regions from non-tumour regions in WSIs of H&E-stained tissue sections known  
738 to contain cancerous regions. The performance is evaluated against manual segmentations in the  
739 validation cohorts described in section 1.2 using only scans from the Aperio AT2 scanner.

740 The single segmentation method is as described in section 2 and developed using images from  
741 cohorts described in section 1.1.

742 The primary analysis of each validation cohort described in section 1.2 is the segmentation  
743 method's performance measured using the Dice similarity coefficient (eq. (10)) averaged over the  
744 images in the cohort with associated 95% confidence interval. The results will also be presented as  
745 a box plot showing mean value (which is the primary metric), median value, interquartile range,  
746 whiskers and outliers for each cohort.

### 747 **3.2 Secondary analyses**

#### 748 **3.2.1 Different performance evaluation metrics of primary result**

749 In the corresponding manner as done in the primary analysis for the Dice similarity coefficient,  
750 report the following segmentation performance evaluation metrics:

- 751 • Prevalence (amount of reference positive / total)
- 752 • Bias (amount of predicted positive / total)
- 753 • True positive rate (eq. (1))
- 754 • False negative rate (eq. (2))
- 755 • True negative rate (eq. (3))
- 756 • False positive rate (eq. (4))
- 757 • Positive predictive value (eq. (5))
- 758 • Negative predictive value (eq. (6))
- 759 • Informedness (eq. (7))
- 760 • Markedness (eq. (8))
- 761 • Matthews correlation coefficient (eq. (9))

#### 762 **3.2.2 Primary result on scans from the NanoZoomer XR**

763 Repeat the primary analysis and the analysis in section 3.2.1 but on scans from NanoZoomer XR  
764 instead of Aperio AT2.

#### 765 **3.2.3 Single cancer type training**

766 Repeat the primary analysis and the analysis in section 3.2.1 on methods that are developed exactly  
767 as the method analysed in the primary analysis except that the methods only have been trained  
768 on a subset of the original training set. The original training set is partitioned into one subset per  
769 cancer type, comprising scans only from that cancer type. Therefore, four segmentation methods  
770 are analysed, one for each of the cancer types

- 771 • Colorectal carcinoma
- 772 • Endometrial carcinoma

- 773       • Lung carcinoma  
774       • Prostate carcinoma

775 All four additional segmentation methods will be analysed on all validation cohorts.

### 776 **3.2.4 Primary analysis replication**

777 Repeat the primary analysis and the analysis in section [3.2.1](#) on methods trained exactly as the one  
778 in the primary analysis, except for different random seed which will affect the neural network pa-  
779 rameter initialisation and the image input pipeline. Both two additional methods will be analysed  
780 on all validation cohorts.

781 **References**

- 782 [1] David G Lowe. Object recognition from local scale-invariant features. In *Proceedings of the*  
783 *seventh IEEE international conference on computer vision*, volume 2, pages 1150–1157. Ieee,  
784 1999.
- 785 [2] Adam Goode, Benjamin Gilbert, Jan Harkes, Drazen Jukic, and Mahadev Satyanarayanan.  
786 Openslide: A vendor-neutral software foundation for digital pathology. *Journal of pathology*  
787 *informatics*, 4, 2013.
- 788 [3] J Bondi, A Husdal, G Bukholm, JM Nesland, A Bakka, and IRK Bukholm. Expression  
789 and gene amplification of primary (a, b1, d1, d3, and e) and secondary (c and h) cyclins in  
790 colon adenocarcinomas and correlation with patient outcome. *Journal of clinical pathology*,  
791 58(5):509–514, 2005.
- 792 [4] Ole-Johan Skrede, Sepp De Raedt, Andreas Kleppe, Tarjei S Hveem, Knut Liestøl, John  
793 Maddison, Hanne A Askautrud, Manohar Pradhan, John Arne Nesheim, Fritz Albrechtsen,  
794 et al. Deep learning for prediction of colorectal cancer outcome: a discovery and validation  
795 study. *The Lancet*, 395(10221):350–360, 2020.
- 796 [5] MA Merok, T Ahlquist, EC Røyrvik, KF Tufteland, M Hektoen, OH Sjo, T Mala, A Svindland,  
797 RA Lothe, and A Nesbakken. Microsatellite instability has a positive prognostic impact on  
798 stage ii colorectal cancer after complete resection: results from a large, consecutive norwegian  
799 series. *Annals of Oncology*, 24(5):1274–1282, 2013.
- 800 [6] TS Hveem, MA Merok, ME Pretorius, M Novelli, MS Bævre, OH Sjo, N Clinch, K Liestøl,  
801 A Svindland, RA Lothe, et al. Prognostic impact of genomic instability in colorectal cancer.  
802 *British journal of cancer*, 110(8):2159–2164, 2014.
- 803 [7] David J Kerr, Janet A Dunn, Michael J Langman, Justine L Smith, Rachel SJ Midgley,  
804 Andrew Stanley, Joanne C Stokes, Patrick Julier, Claire Iveson, Ravi Duvvuri, et al. Rofecoxib  
805 and cardiovascular adverse events in adjuvant treatment of colorectal cancer. *New England*  
806 *Journal of Medicine*, 357(4):360–369, 2007.
- 807 [8] Jone Trovik, Elisabeth Wik, Henrica MJ Werner, Camilla Krakstad, Harald Helland, Ingrid  
808 Vandenput, Tormund S Njølstad, Ingunn M Stefansson, Janusz Marcickiewicz, Solveig Tingul-  
809 stad, et al. Hormone receptor loss in endometrial carcinoma curettage predicts lymph node  
810 metastasis and poor outcome in prospective multicentre trial. *European journal of cancer*,  
811 49(16):3431–3441, 2013.
- 812 [9] Tarjei S Hveem, Tormund S Njølstad, Birgitte Nielsen, Rolf Anders Syvertsen, John Arne  
813 Nesheim, Marna L Kjæreng, Wanja Kildal, Manohar Pradhan, Janusz Marcickiewicz, Solveig  
814 Tingulstad, et al. Changes in chromatin structure in curettage specimens identifies high-risk  
815 patients in endometrial cancer. *Cancer Epidemiology and Prevention Biomarkers*, 26(1):61–67,  
816 2017.
- 817 [10] Robert J. Kurman, Maria Luisa Carcangiu, C. Simon Herrington, and Robert H. Young. *WHO*  
818 *Classification of Tumours of Female Reproductive Organs*. International Agency for Research  
819 on Cancer, Lyon, 4 edition, 2014.
- 820 [11] WHO Classification of Tumours Editorial Board. *WHO Classification of Tumours; Female*  
821 *Genital Tumours*. International Agency for Research on Cancer, Lyon, 5 edition, 2020.
- 822 [12] Jonathan I Epstein, Lars Egevad, Mahul B Amin, Brett Delahunt, John R Srigley, and Pe-  
823 ter A Humphrey. The 2014 international society of urological pathology (isup) consensus con-  
824 ference on gleason grading of prostatic carcinoma. *The American journal of surgical pathology*,  
825 40(2):244–252, 2016.

- 826 [13] Håkon Wæhre, Ljiljana Vlatkovic, Milada Cvancarova, Elisabeth Paus, Sophie D Fosså, and  
827 Håvard E Danielsen. Fifteen-year mortality after radical prostatectomy: Which factors are  
828 available for patient counselling? *Scandinavian Journal of Urology*, 48(2):123–130, 2014.
- 829 [14] Karolina Cyll, Elin Ersvær, Ljiljana Vlatkovic, Manohar Pradhan, Wanja Kildal, Marte Avran-  
830 den Kjær, Andreas Kleppe, Tarjei S Hveem, Birgitte Carlsen, Silje Gill, et al. Tumour hetero-  
831 geneity poses a significant challenge to cancer biomarker research. *British journal of cancer*,  
832 117(3):367–375, 2017.
- 833 [15] Rachel S Kerr, Sharon Love, Eva Segelov, Elaine Johnstone, Beverly Falcon, Peter Hewett,  
834 Andrew Weaver, David Church, Claire Scudder, Sarah Pearson, et al. Adjuvant capecitabine  
835 plus bevacizumab versus capecitabine alone in patients with colorectal cancer (quasar 2): an  
836 open-label, randomised phase 3 trial. *The Lancet Oncology*, 17(11):1543–1557, 2016.
- 837 [16] Sigurd M Hald, Mehrdad Rakaee, Inigo Martinez, Elin Richardsen, Samer Al-Saad, Erna-Elise  
838 Paulsen, Egil Støre Blix, Thomas Kilvaer, Sigve Andersen, Lill-Tove Busund, et al. Lag-3 in  
839 non-small-cell lung cancer: expression in primary tumors and metastatic lymph nodes is  
840 associated with improved survival. *Clinical lung cancer*, 19(3):249–259, 2018.
- 841 [17] Mehrdad Rakaee, Lill-Tove Rasmussen Busund, Simin Jamaly, Erna-Elise Paulsen, Elin  
842 Richardsen, Sigve Andersen, Samer Al-Saad, Roy M Bremnes, Tom Donnem, and Thomas K  
843 Kilvaer. Prognostic value of macrophage phenotypes in resectable non-small cell lung cancer  
844 assessed by multiplex immunohistochemistry. *Neoplasia*, 21(3):282–293, 2019.
- 845 [18] Karolina Cyll, Andreas Kleppe, Joakim Kalsnes, Ljiljana Vlatkovic, Manohar Pradhan, Wanja  
846 Kildal, Kari Anne R Tobin, Trine M Reine, Håkon Wæhre, Bjørn Brennhovd, et al. Pten and  
847 dna ploidy status by machine learning in prostate cancer. *Cancers*, 13(17):4291, 2021.
- 848 [19] Ivar Skaland, Emiel AM Janssen, Einar Gudlaugsson, Lydia Hui Ru Guo, and Jan Baak. The  
849 prognostic value of the proliferation marker phosphohistone h3 (pph3) in luminal, basal-like  
850 and triple negative phenotype invasive lymph node-negative breast cancer. *Analytical Cellular  
851 Pathology*, 31(4):261–271, 2009.
- 852 [20] Ivar Skaland, Emiel AM Janssen, Einar Gudlaugsson, Jan Klos, Kjell H Kjellevold, Håvard  
853 Søyland, and Jan Baak. Validating the prognostic value of proliferation measured by phospho-  
854 histone h3 (pph3) in invasive lymph node-negative breast cancer patients less than 71 years  
855 of age. *Breast cancer research and treatment*, 114(1):39–45, 2009.
- 856 [21] Kristin Jonsdottir, Hui Zhang, Darshni Jhagroe, Ivar Skaland, Aida Slewa, Benny Björkblom,  
857 Eleanor T Coffey, Einar Gudlaugsson, Rune Smaaland, Emiel AM Janssen, et al. The prog-  
858 nostic value of marcks-like 1 in lymph node-negative breast cancer. *Breast cancer research  
859 and treatment*, 135(2):381–390, 2012.
- 860 [22] Kristin Jonsdottir, Susanne R Janssen, Fabiana C Da Rosa, Einar Gudlaugsson, Ivar Skaland,  
861 Jan PA Baak, and Emiel AM Janssen. Validation of expression patterns for nine mirnas in  
862 204 lymph-node negative breast cancers. *PloS one*, 7(11):e48692, 2012.
- 863 [23] Nina Gran Egeland, Marie Austdal, Bianca van Diermen-Hidle, Emma Rewcastle, Einar G  
864 Gudlaugsson, Jan PA Baak, Ivar Skaland, Emiel AM Janssen, and Kristin Jonsdottir. Valid-  
865 ation study of marcksl1 as a prognostic factor in lymph node-negative breast cancer patients.  
866 *PloS one*, 14(3):e0212527, 2019.
- 867 [24] Vebjørn Kvikstad, Ok Målfrid Mangrud, Einar Gudlaugsson, Ingvild Dalen, Hans Espeland,  
868 Jan Baak, and Emiel AM Janssen. Prognostic value and reproducibility of different micro-  
869 scopic characteristics in the who grading systems for pta and pt1 urinary bladder urothelial  
870 carcinomas. *Diagnostic pathology*, 14(1):1–8, 2019.

- 871 [25] Melinda Lillesand, Vebjørn Kvikstad, Ok Målfrid Mangrud, Einar Gudlaugsson, Bianca van  
872 Diermen-Hidle, Ivar Skaland, Jan PA Baak, and Emiel AM Janssen. Mitotic activity index  
873 and cd25+ lymphocytes predict risk of stage progression in non-muscle invasive bladder cancer.  
874 *Plos one*, 15(6):e0233676, 2020.
- 875 [26] John Canny. A computational approach to edge detection. *IEEE Transactions on pattern  
876 analysis and machine intelligence*, pages 679–698, 1986.
- 877 [27] Alexander Buslaev, Vladimir I. Iglovikov, Eugene Khvedchenya, Alex Parinov, Mikhail  
878 Druzhinin, and Alexandr A. Kalinin. Albumentations: Fast and flexible image augmenta-  
879 tions. *Information*, 11(2), 2020.
- 880 [28] Adam Paszke, Sam Gross, Francisco Massa, Adam Lerer, James Bradbury, Gregory Chanan,  
881 Trevor Killeen, Zeming Lin, Natalia Gimelshein, Luca Antiga, Alban Desmaison, Andreas  
882 Kopf, Edward Yang, Zachary DeVito, Martin Raison, Alykhan Tejani, Sasank Chilamkurthy,  
883 Benoit Steiner, Lu Fang, Junjie Bai, and Soumith Chintala. Pytorch: An imperative style,  
884 high-performance deep learning library. In H. Wallach, H. Larochelle, A. Beygelzimer,  
885 F. d’Alché-Buc, E. Fox, and R. Garnett, editors, *Advances in Neural Information Process-  
886 ing Systems 32*, pages 8024–8035. Curran Associates, Inc., 2019.
- 887 [29] Andrew Brock, Soham De, Samuel L. Smith, and Karen Simonyan. High-performance large-  
888 scale image recognition without normalization. *arXiv preprint arXiv:2102.06171*, 2021.
- 889 [30] Andrew Brock, Soham De, and Samuel L. Smith. Characterizing signal propagation to close  
890 the performance gap in unnormalized resnets. In *9th International Conference on Learning  
891 Representations, ICLR*, 2021.
- 892 [31] Ross Wightman. Pytorch image models. [https://github.com/rwightman/  
893 pytorch-image-models](https://github.com/rwightman/pytorch-image-models), 2019.
- 894 [32] Jie Hu, Li Shen, and Gang Sun. Squeeze-and-excitation networks. In *Proceedings of the IEEE  
895 conference on computer vision and pattern recognition*, pages 7132–7141, 2018.
- 896 [33] Qilong Wang, Banggu Wu, Pengfei Zhu, Peihua Li, Wangmeng Zuo, and Qinghua Hu. Eca-  
897 net: Efficient channel attention for deep convolutional neural networks. In *2020 IEEE/CVF  
898 Conference on Computer Vision and Pattern Recognition (CVPR)*, pages 11531–11539, 2020.
- 899 [34] Dan Hendrycks and Kevin Gimpel. Gaussian error linear units (gelus). *arXiv preprint  
900 arXiv:1606.08415*, 2016.
- 901 [35] Liang-Chieh Chen, Yukun Zhu, George Papandreou, Florian Schroff, and Hartwig Adam.  
902 Encoder-decoder with atrous separable convolution for semantic image segmentation. In *Pro-  
903 ceedings of the European conference on computer vision (ECCV)*, pages 801–818, 2018.
- 904 [36] Pavel Yakubovskiy. Segmentation models pytorch. [https://github.com/qubvel/  
905 segmentation\\_models.pytorch](https://github.com/qubvel/segmentation_models.pytorch), 2020.
- 906 [37] Yuxin Wu and Kaiming He. Group normalization. In *Proceedings of the European conference  
907 on computer vision (ECCV)*, pages 3–19, 2018.
- 908 [38] Kaiming He, Xiangyu Zhang, Shaoqing Ren, and Jian Sun. Delving deep into rectifiers:  
909 Surpassing human-level performance on imagenet classification. In *Proceedings of the IEEE  
910 international conference on computer vision*, pages 1026–1034, 2015.
- 911 [39] Ilya Sutskever, James Martens, George Dahl, and Geoffrey Hinton. On the importance of ini-  
912 tialization and momentum in deep learning. In *International conference on machine learning*,  
913 pages 1139–1147. PMLR, 2013.
- 914 [40] Ilya Loshchilov and Frank Hutter. Sgdr: Stochastic gradient descent with warm restarts.  
915 *arXiv preprint arXiv:1608.03983*, 2016.
